# Supplementary material for: Multiple tests for restricted mean time lost with competing risks data
Source: arXiv:2409.07917 source file (2024-09-12)
Supplement: Supplementary file 1 [file supplement.pdf]

# Supplementary material to Multiple tests for the restricted mean time lost with competing risks data

Merle Munko<sup>1,\*</sup>, Dennis Dobler<sup>2,3</sup>, and Marc Ditzhaus<sup>1</sup>

<sup>1</sup> Otto-von-Guericke University Magdeburg; Magdeburg (Germany)

<sup>2</sup> TU Dortmund University; Dortmund (Germany)

<sup>3</sup> Research Center Trustworthy Data Science and Security, University Alliance Ruhr; Dortmund (Germany)

In this supplement, the theoretical proofs of all stated theorems can be found in Section A. In Section B, details on the simulations are given. This includes an explanation of the simulation settings in Section B.1 as well as additional figures and detailed tables of the simulation results in Section B.2 and B.3, respectively.

## Contents

|                                              |            |
|----------------------------------------------|------------|
| <b>List of Figures</b>                       | <b>1</b>   |
| <b>List of Tables</b>                        | <b>2</b>   |
| <b>A Proofs</b>                              | <b>6</b>   |
| <b>B Details on the Simulation Study</b>     | <b>19</b>  |
| B.1 Simulation Settings                      | 19         |
| B.2 Additional Figures of Simulation Results | 21         |
| B.3 Tables of Simulation Results             | 23         |
| <b>References</b>                            | <b>114</b> |

## List of Figures

|    |                                                                                                                  |    |
|----|------------------------------------------------------------------------------------------------------------------|----|
| S1 | Empirical powers for the 2-by-2 design across all scenarios under the alternative hypothesis.                    | 21 |
| S2 | Empirical powers for the Dunnett-type contrast hypotheses across all scenarios under the alternative hypothesis. | 22 |
| S3 | Empirical powers for the Tukey-type contrast hypotheses across all scenarios under the alternative hypothesis.   | 23 |

---

\*Corresponding author. Email address: merle.munko@ovgu.de

## List of Tables

|     |                                                                                                                                 |    |
|-----|---------------------------------------------------------------------------------------------------------------------------------|----|
| S1  | Rejection rates in percent for the 2-by-2 design with $\delta = 0.0$ and balanced large sample sizes. . . . .                   | 24 |
| S2  | Rejection rates in percent for the 2-by-2 design with $\delta = 0.0$ and balanced medium sample sizes. . . . .                  | 25 |
| S3  | Rejection rates in percent for the 2-by-2 design with $\delta = 0.0$ and balanced small sample sizes. . . . .                   | 26 |
| S4  | Rejection rates in percent for the 2-by-2 design with $\delta = 0.0$ and unbalanced large sample sizes. . . . .                 | 27 |
| S5  | Rejection rates in percent for the 2-by-2 design with $\delta = 0.0$ and unbalanced medium sample sizes. . . . .                | 28 |
| S6  | Rejection rates in percent for the 2-by-2 design with $\delta = 0.0$ and unbalanced small sample sizes. . . . .                 | 29 |
| S7  | Rejection rates in percent for the Dunnett-type contrast matrix with $\delta = 0.0$ and balanced large sample sizes. . . . .    | 30 |
| S8  | Rejection rates in percent for the Dunnett-type contrast matrix with $\delta = 0.0$ and balanced medium sample sizes. . . . .   | 31 |
| S9  | Rejection rates in percent for the Dunnett-type contrast matrix with $\delta = 0.0$ and balanced small sample sizes. . . . .    | 32 |
| S10 | Rejection rates in percent for the Dunnett-type contrast matrix with $\delta = 0.0$ and unbalanced large sample sizes. . . . .  | 33 |
| S11 | Rejection rates in percent for the Dunnett-type contrast matrix with $\delta = 0.0$ and unbalanced medium sample sizes. . . . . | 34 |
| S12 | Rejection rates in percent for the Dunnett-type contrast matrix with $\delta = 0.0$ and unbalanced small sample sizes. . . . .  | 35 |
| S13 | Rejection rates in percent for the Tukey-type contrast matrix with $\delta = 0.0$ and balanced large sample sizes. . . . .      | 36 |
| S14 | Rejection rates in percent for the Tukey-type contrast matrix with $\delta = 0.0$ and balanced medium sample sizes. . . . .     | 37 |
| S15 | Rejection rates in percent for the Tukey-type contrast matrix with $\delta = 0.0$ and balanced small sample sizes. . . . .      | 38 |
| S16 | Rejection rates in percent for the Tukey-type contrast matrix with $\delta = 0.0$ and unbalanced large sample sizes. . . . .    | 39 |
| S17 | Rejection rates in percent for the Tukey-type contrast matrix with $\delta = 0.0$ and unbalanced medium sample sizes. . . . .   | 40 |
| S18 | Rejection rates in percent for the Tukey-type contrast matrix with $\delta = 0.0$ and unbalanced small sample sizes. . . . .    | 41 |
| S19 | Rejection rates in percent for the 2-by-2 design with $\delta = 1.5$ and balanced large sample sizes. . . . .                   | 42 |
| S20 | Rejection rates in percent for the 2-by-2 design with $\delta = 1.5$ and balanced medium sample sizes. . . . .                  | 43 |
| S21 | Rejection rates in percent for the 2-by-2 design with $\delta = 1.5$ and balanced small sample sizes. . . . .                   | 44 |
| S22 | Rejection rates in percent for the 2-by-2 design with $\delta = 1.5$ and unbalanced large sample sizes. . . . .                 | 45 |

|     |                                                                                                                                              |    |
|-----|----------------------------------------------------------------------------------------------------------------------------------------------|----|
| S23 | Rejection rates in percent for the 2-by-2 design with $\delta = 1.5$ and unbalanced medium sample sizes. . . . .                             | 46 |
| S24 | Rejection rates in percent for the 2-by-2 design with $\delta = 1.5$ and unbalanced small sample sizes. . . . .                              | 47 |
| S25 | Rejection rates in percent for the Dunnett-type contrast matrix with $\delta = 1.5$ and balanced large sample sizes. . . . .                 | 48 |
| S26 | Rejection rates in percent for the Dunnett-type contrast matrix with $\delta = 1.5$ and balanced medium sample sizes. . . . .                | 49 |
| S27 | Rejection rates in percent for the Dunnett-type contrast matrix with $\delta = 1.5$ and balanced small sample sizes. . . . .                 | 50 |
| S28 | Rejection rates in percent for the Dunnett-type contrast matrix with $\delta = 1.5$ and unbalanced large sample sizes. . . . .               | 51 |
| S29 | Rejection rates in percent for the Dunnett-type contrast matrix with $\delta = 1.5$ and unbalanced medium sample sizes. . . . .              | 52 |
| S30 | Rejection rates in percent for the Dunnett-type contrast matrix with $\delta = 1.5$ and unbalanced small sample sizes. . . . .               | 53 |
| S31 | Rejection rates in percent for the Tukey-type contrast matrix with $\delta = 1.5$ and balanced large sample sizes. . . . .                   | 54 |
| S32 | Rejection rates in percent for the Tukey-type contrast matrix with $\delta = 1.5$ and balanced medium sample sizes. . . . .                  | 55 |
| S33 | Rejection rates in percent for the Tukey-type contrast matrix with $\delta = 1.5$ and balanced small sample sizes. . . . .                   | 56 |
| S34 | Rejection rates in percent for the Tukey-type contrast matrix with $\delta = 1.5$ and unbalanced large sample sizes. . . . .                 | 57 |
| S35 | Rejection rates in percent for the Tukey-type contrast matrix with $\delta = 1.5$ and unbalanced medium sample sizes. . . . .                | 58 |
| S36 | Rejection rates in percent for the Tukey-type contrast matrix with $\delta = 1.5$ and unbalanced small sample sizes. . . . .                 | 59 |
| S37 | Rejection rates in percent for the 2-by-2 design with $\delta = 1.5$ and balanced large sample sizes under equal censoring. . . . .          | 60 |
| S38 | Rejection rates in percent for the 2-by-2 design with $\delta = 1.5$ and balanced medium sample sizes under equal censoring. . . . .         | 61 |
| S39 | Rejection rates in percent for the 2-by-2 design with $\delta = 1.5$ and balanced small sample sizes under equal censoring. . . . .          | 62 |
| S40 | Rejection rates in percent for the 2-by-2 design with $\delta = 1.5$ and unbalanced large sample sizes under equal censoring. . . . .        | 63 |
| S41 | Rejection rates in percent for the 2-by-2 design with $\delta = 1.5$ and unbalanced medium sample sizes under equal censoring. . . . .       | 64 |
| S42 | Rejection rates in percent for the 2-by-2 design with $\delta = 1.5$ and unbalanced small sample sizes under equal censoring. . . . .        | 65 |
| S43 | Rejection rates in percent for the 2-by-2 design with $\delta = 1.5$ and balanced large sample sizes under unequal, high censoring. . . . .  | 66 |
| S44 | Rejection rates in percent for the 2-by-2 design with $\delta = 1.5$ and balanced medium sample sizes under unequal, high censoring. . . . . | 67 |
| S45 | Rejection rates in percent for the 2-by-2 design with $\delta = 1.5$ and balanced small sample sizes under unequal, high censoring. . . . .  | 68 |

|     |                                                                                                                                                               |    |
|-----|---------------------------------------------------------------------------------------------------------------------------------------------------------------|----|
| S46 | Rejection rates in percent for the 2-by-2 design with $\delta = 1.5$ and unbalanced large sample sizes under unequal, high censoring. . . . .                 | 69 |
| S47 | Rejection rates in percent for the 2-by-2 design with $\delta = 1.5$ and unbalanced medium sample sizes under unequal, high censoring. . . . .                | 70 |
| S48 | Rejection rates in percent for the 2-by-2 design with $\delta = 1.5$ and unbalanced small sample sizes under unequal, high censoring. . . . .                 | 71 |
| S49 | Rejection rates in percent for the 2-by-2 design with $\delta = 1.5$ and balanced large sample sizes under unequal, low censoring. . . . .                    | 72 |
| S50 | Rejection rates in percent for the 2-by-2 design with $\delta = 1.5$ and balanced medium sample sizes under unequal, low censoring. . . . .                   | 73 |
| S51 | Rejection rates in percent for the 2-by-2 design with $\delta = 1.5$ and balanced small sample sizes under unequal, low censoring. . . . .                    | 74 |
| S52 | Rejection rates in percent for the 2-by-2 design with $\delta = 1.5$ and unbalanced large sample sizes under unequal, low censoring. . . . .                  | 75 |
| S53 | Rejection rates in percent for the 2-by-2 design with $\delta = 1.5$ and unbalanced medium sample sizes under unequal, low censoring. . . . .                 | 76 |
| S54 | Rejection rates in percent for the 2-by-2 design with $\delta = 1.5$ and unbalanced small sample sizes under unequal, low censoring. . . . .                  | 77 |
| S55 | Rejection rates in percent for the Dunnett-type contrast matrix with $\delta = 1.5$ and balanced large sample sizes under equal censoring. . . . .            | 78 |
| S56 | Rejection rates in percent for the Dunnett-type contrast matrix with $\delta = 1.5$ and balanced medium sample sizes under equal censoring. . . . .           | 79 |
| S57 | Rejection rates in percent for the Dunnett-type contrast matrix with $\delta = 1.5$ and balanced small sample sizes under equal censoring. . . . .            | 80 |
| S58 | Rejection rates in percent for the Dunnett-type contrast matrix with $\delta = 1.5$ and unbalanced large sample sizes under equal censoring. . . . .          | 81 |
| S59 | Rejection rates in percent for the Dunnett-type contrast matrix with $\delta = 1.5$ and unbalanced medium sample sizes under equal censoring. . . . .         | 82 |
| S60 | Rejection rates in percent for the Dunnett-type contrast matrix with $\delta = 1.5$ and unbalanced small sample sizes under equal censoring. . . . .          | 83 |
| S61 | Rejection rates in percent for the Dunnett-type contrast matrix with $\delta = 1.5$ and balanced large sample sizes under unequal, high censoring. . . . .    | 84 |
| S62 | Rejection rates in percent for the Dunnett-type contrast matrix with $\delta = 1.5$ and balanced medium sample sizes under unequal, high censoring. . . . .   | 85 |
| S63 | Rejection rates in percent for the Dunnett-type contrast matrix with $\delta = 1.5$ and balanced small sample sizes under unequal, high censoring. . . . .    | 86 |
| S64 | Rejection rates in percent for the Dunnett-type contrast matrix with $\delta = 1.5$ and unbalanced large sample sizes under unequal, high censoring. . . . .  | 87 |
| S65 | Rejection rates in percent for the Dunnett-type contrast matrix with $\delta = 1.5$ and unbalanced medium sample sizes under unequal, high censoring. . . . . | 88 |
| S66 | Rejection rates in percent for the Dunnett-type contrast matrix with $\delta = 1.5$ and unbalanced small sample sizes under unequal, high censoring. . . . .  | 89 |
| S67 | Rejection rates in percent for the Dunnett-type contrast matrix with $\delta = 1.5$ and balanced large sample sizes under unequal, low censoring. . . . .     | 90 |
| S68 | Rejection rates in percent for the Dunnett-type contrast matrix with $\delta = 1.5$ and balanced medium sample sizes under unequal, low censoring. . . . .    | 91 |

|     |                                                                                                                                                              |     |
|-----|--------------------------------------------------------------------------------------------------------------------------------------------------------------|-----|
| S69 | Rejection rates in percent for the Dunnett-type contrast matrix with $\delta = 1.5$ and balanced small sample sizes under unequal, low censoring. . . . .    | 92  |
| S70 | Rejection rates in percent for the Dunnett-type contrast matrix with $\delta = 1.5$ and unbalanced large sample sizes under unequal, low censoring. . . . .  | 93  |
| S71 | Rejection rates in percent for the Dunnett-type contrast matrix with $\delta = 1.5$ and unbalanced medium sample sizes under unequal, low censoring. . . . . | 94  |
| S72 | Rejection rates in percent for the Dunnett-type contrast matrix with $\delta = 1.5$ and unbalanced small sample sizes under unequal, low censoring. . . . .  | 95  |
| S73 | Rejection rates in percent for the Tukey-type contrast matrix with $\delta = 1.5$ and balanced large sample sizes under equal censoring. . . . .             | 96  |
| S74 | Rejection rates in percent for the Tukey-type contrast matrix with $\delta = 1.5$ and balanced medium sample sizes under equal censoring. . . . .            | 97  |
| S75 | Rejection rates in percent for the Tukey-type contrast matrix with $\delta = 1.5$ and balanced small sample sizes under equal censoring. . . . .             | 98  |
| S76 | Rejection rates in percent for the Tukey-type contrast matrix with $\delta = 1.5$ and unbalanced large sample sizes under equal censoring. . . . .           | 99  |
| S77 | Rejection rates in percent for the Tukey-type contrast matrix with $\delta = 1.5$ and unbalanced medium sample sizes under equal censoring. . . . .          | 100 |
| S78 | Rejection rates in percent for the Tukey-type contrast matrix with $\delta = 1.5$ and unbalanced small sample sizes under equal censoring. . . . .           | 101 |
| S79 | Rejection rates in percent for the Tukey-type contrast matrix with $\delta = 1.5$ and balanced large sample sizes under unequal, high censoring. . . . .     | 102 |
| S80 | Rejection rates in percent for the Tukey-type contrast matrix with $\delta = 1.5$ and balanced medium sample sizes under unequal, high censoring. . . . .    | 103 |
| S81 | Rejection rates in percent for the Tukey-type contrast matrix with $\delta = 1.5$ and balanced small sample sizes under unequal, high censoring. . . . .     | 104 |
| S82 | Rejection rates in percent for the Tukey-type contrast matrix with $\delta = 1.5$ and unbalanced large sample sizes under unequal, high censoring. . . . .   | 105 |
| S83 | Rejection rates in percent for the Tukey-type contrast matrix with $\delta = 1.5$ and unbalanced medium sample sizes under unequal, high censoring. . . . .  | 106 |
| S84 | Rejection rates in percent for the Tukey-type contrast matrix with $\delta = 1.5$ and unbalanced small sample sizes under unequal, high censoring. . . . .   | 107 |
| S85 | Rejection rates in percent for the Tukey-type contrast matrix with $\delta = 1.5$ and balanced large sample sizes under unequal, low censoring. . . . .      | 108 |
| S86 | Rejection rates in percent for the Tukey-type contrast matrix with $\delta = 1.5$ and balanced medium sample sizes under unequal, low censoring. . . . .     | 109 |
| S87 | Rejection rates in percent for the Tukey-type contrast matrix with $\delta = 1.5$ and balanced small sample sizes under unequal, low censoring. . . . .      | 110 |
| S88 | Rejection rates in percent for the Tukey-type contrast matrix with $\delta = 1.5$ and unbalanced large sample sizes under unequal, low censoring. . . . .    | 111 |
| S89 | Rejection rates in percent for the Tukey-type contrast matrix with $\delta = 1.5$ and unbalanced medium sample sizes under unequal, low censoring. . . . .   | 112 |
| S90 | Rejection rates in percent for the Tukey-type contrast matrix with $\delta = 1.5$ and unbalanced small sample sizes under unequal, low censoring. . . . .    | 113 |

# A Proofs

## Proof of Theorem 1

Firstly, let  $i \in \{1, \dots, k\}$  be arbitrary but fixed. By Theorem 4.1 in [3], we have

$$n_i^{1/2} \left( \hat{A}_{i1} - A_{i1}, \dots, \hat{A}_{iM} - A_{iM} \right) \xrightarrow{d} (U_{i1}, \dots, U_{iM}) \quad (S1)$$

as  $n \rightarrow \infty$  on  $(D[0, \tau])^M$  equipped with the sup-norm, where  $U_{i1}, \dots, U_{iM}$  are centered Gaussian-martingales with

$$\begin{aligned} \text{Cov}(U_{im_1}(t), U_{im_1}(s)) &= \int_{[0, \min\{t, s\}]} \frac{1 - \Delta A_{im_1}}{y_i} dA_{im_1} =: \sigma_{im_1 m_1}(\min\{t, s\}), \\ \text{Cov}(U_{im_1}(t), U_{im_2}(s)) &= - \int_{[0, \min\{t, s\}]} \frac{\Delta A_{im_1}}{y_i} dA_{im_2} =: \sigma_{im_1 m_2}(\min\{t, s\}) \end{aligned}$$

and  $y_i(t) := P(X_{i1} \geq t)$  for all  $t, s \in [0, \tau]$ ;  $m_1, m_2 \in \{1, \dots, M\}$ ;  $m_1 \neq m_2$ . By [4], the limit  $(U_{i1}, \dots, U_{iM})$  is separable.

Let  $BV[0, \tau] \subset D[0, \tau]$  denote the set of all càdlàg functions on  $[0, \tau]$  of total variation bounded by a fixed and sufficiently large constant. Then, we consider the functional

$$\begin{aligned} \Phi : (BV[0, \tau])^M &\rightarrow \mathbb{R}^M, \\ (\Lambda_1, \dots, \Lambda_M) &\mapsto \left( \int_0^\tau \int_{[0, t]} \prod_{0 \leq x < u} \left\{ 1 - d \left( \sum_{\tilde{m}=1}^M \Lambda_{\tilde{m}} \right) (x) \right\} d\Lambda_m(u) dt \right)_{m \in \{1, \dots, M\}}. \end{aligned}$$

Here and throughout, we define the jump  $\Delta \Lambda(0)$  of a function  $\Lambda \in BV[0, \tau]$  at 0 as  $\Lambda(0)$ . Note that  $\Phi(A_{i1}, \dots, A_{iM}) = (\mu_{i1}, \dots, \mu_{iM})$  and  $\Phi(\hat{A}_{i1}, \dots, \hat{A}_{iM}) = (\hat{\mu}_{i1}, \dots, \hat{\mu}_{iM})$  holds. We aim to apply the delta-method. Therefore, we firstly show that  $\Phi$  is Hadamard-differentiable at  $(A_{i1}, \dots, A_{iM})$  with Hadamard-derivative  $\Phi'_{(A_{i1}, \dots, A_{iM})}$  at  $(\alpha_1, \dots, \alpha_M) \in (D[0, \tau])^M$  given by

$$\left( \int_0^\tau \left( \int_{[0, t]} \prod_{0 \leq x < u} (1 - dA_i(x)) d\alpha_m(u) - \int_{[0, t]} \prod_{0 \leq x < u} (1 - dA_i(x)) \int_{[0, u]} \frac{d \sum_{\tilde{m}=1}^M \alpha_{\tilde{m}}}{1 - \Delta A_i} dA_{im}(u) \right) dt \right)_{m \in \{1, \dots, M\}}.$$

Here, the integrals with respect to  $\alpha_m$  are defined via integration by parts because  $\alpha_m$  need not have finite variation. The same holds for other integrals of this kind below. In order to prove the Hadamard-differentiability, we consider the Wilcoxon functional and the product integral functional, that are

$$\begin{aligned} \Psi : \tilde{D}[0, \tau] \times BV[0, \tau] &\rightarrow D[0, \tau], \quad (A, B) \mapsto \int_{[0, \cdot]} A dB \\ \text{and } \phi : D[0, \tau] &\rightarrow \tilde{D}[0, \tau], \quad A \mapsto \prod_{0 \leq x < \cdot} (1 + dA(x)), \end{aligned}$$

where  $\tilde{D}[0, \tau]$  denotes the space of all left-continuous functions on  $[0, \tau]$  with existing limits from the right. Then, we can write

$$\Phi(\Lambda_1, \dots, \Lambda_M) = \left( \int_0^\tau \Psi \left( \phi \left( - \sum_{\tilde{m}=1}^M \Lambda_{\tilde{m}} \right), \Lambda_m \right) (t) dt \right)_{m \in \{1, \dots, M\}}$$

for  $\Lambda_1, \dots, \Lambda_M \in BV[0, \tau]$ . Applying the chain rule (Lemma 3.10.3 in [9]) yields

$$\Phi'_{(A_{i1}, \dots, A_{iM})}(\alpha_1, \dots, \alpha_M) = \left( \int_0^\tau \Psi'_{(\phi(-A_i), A_{im})} \left( \phi'_{-A_i} \left( - \sum_{\tilde{m}=1}^M \alpha_{\tilde{m}} \right), \alpha_m \right) (t) dt \right)_{m \in \{1, \dots, M\}}$$

for  $\alpha_1, \dots, \alpha_M \in D[0, \tau]$ . Note here that the final integral functional is linear, so it equals its Hadamard-derivative. Analogously to Lemma 3.10.18 and Lemma 3.10.32 in [9], one can show that

$$\Psi'_{(\phi(-A_i), A_{im})}(\alpha, \beta) = \int_{[0, \cdot]} S_{i-} d\beta + \int_{[0, \cdot]} \alpha dA_{im}, m \in \{1, \dots, M\}$$

and  $\phi'_{-A_i}(\beta) = S_{i-}(\cdot) \int_{[0, \cdot]} \frac{1}{1 - \Delta A_i} d\beta$

holds for all  $\alpha \in \tilde{D}[0, \tau], \beta \in D[0, \tau]$ . Thus, it follows that

$$\begin{aligned} & \Phi'_{(A_{i1}, \dots, A_{iM})}(\alpha_1, \dots, \alpha_M) \\ &= \left( \int_0^\tau \left( \int_{[0, t]} S_{i-} d\alpha_m - \int_{[0, t]} S_{i-}(s) \int_{[0, s]} \frac{d \sum_{\tilde{m}=1}^M \alpha_{\tilde{m}}}{1 - \Delta A_i} dA_{im}(s) \right) dt \right)_{m \in \{1, \dots, M\}} \\ &= \left( \int_0^\tau \left( \int_{[0, t]} S_{i-} d\alpha_m - \int_{[0, t]} \frac{\int_{(u, t]} S_{i-} dA_{im}}{1 - \Delta A_i(u)} d \sum_{\tilde{m}=1}^M \alpha_{\tilde{m}}(u) \right) dt \right)_{m \in \{1, \dots, M\}} \\ &= \left( \int_0^\tau \left( \int_{[0, t]} \frac{S_i}{1 - \Delta A_i} d\alpha_m - \int_{[0, t]} \frac{F_{im}(t) - F_{im}(u)}{1 - \Delta A_i(u)} d \sum_{\tilde{m}=1}^M \alpha_{\tilde{m}}(u) \right) dt \right)_{m \in \{1, \dots, M\}} \\ &= \left( \int_0^\tau \left( \int_{[0, t]} \frac{S_i(u) - F_{im}(t) + F_{im}(u)}{1 - \Delta A_i(u)} d\alpha_m(u) - \int_{[0, t]} \frac{F_{im}(t) - F_{im}(u)}{1 - \Delta A_i(u)} d \sum_{\tilde{m} \neq m} \alpha_{\tilde{m}}(u) \right) dt \right)_{m \in \{1, \dots, M\}} \\ &= \left( \int_0^\tau \left( \int_{[0, t]} \frac{1 - \sum_{\tilde{m} \neq m} F_{i\tilde{m}}(u) - F_{im}(t)}{1 - \Delta A_i(u)} d\alpha_m(u) - \int_{[0, t]} \frac{F_{im}(t) - F_{im}(u)}{1 - \Delta A_i(u)} d \sum_{\tilde{m} \neq m} \alpha_{\tilde{m}}(u) \right) dt \right)_{m \in \{1, \dots, M\}} \\ &= \left( \int_{[0, \tau]} \frac{(\tau - u) (1 - \sum_{\tilde{m} \neq m} F_{i\tilde{m}}(u)) - \int_u^\tau F_{im}(t) dt}{1 - \Delta A_i(u)} d\alpha_m(u) \right. \\ &\quad \left. + \int_{[0, \tau]} \frac{(\tau - u) F_{im}(u) - \int_u^\tau F_{im}(t) dt}{1 - \Delta A_i(u)} d \sum_{\tilde{m} \neq m} \alpha_{\tilde{m}}(u) \right)_{m \in \{1, \dots, M\}} \end{aligned}$$

for  $\alpha_1, \dots, \alpha_M \in D[0, \tau]$ , where here and throughout, we write  $\sum_{\tilde{m} \neq m}$  instead of  $\sum_{\tilde{m}=1, \tilde{m} \neq m}^M$  for the sake of brevity. Thus, an application of the delta-method (Theorem 3.10.4 in [9]) yields

$$\begin{aligned} n_i^{1/2}(\hat{\mu}_{im} - \mu_{im})_{m \in \{1, \dots, M\}} &\xrightarrow{d} \Phi'_{(A_{i1}, \dots, A_{iM})}(U_{i1}, \dots, U_{iM}) \\ &= \left( \int_{[0, \tau)} \frac{(\tau - u) \left(1 - \sum_{\tilde{m} \neq m} F_{i\tilde{m}}(u)\right) - \int_u^\tau F_{im}(t) dt}{1 - \Delta A_i(u)} dU_{im}(u) \right. \\ &\quad \left. + \int_{[0, \tau)} \frac{(\tau - u)F_{im}(u) - \int_u^\tau F_{im}(t) dt}{1 - \Delta A_i(u)} d \sum_{\tilde{m} \neq m} U_{i\tilde{m}}(u) \right)_{m \in \{1, \dots, M\}} \end{aligned}$$

as  $n \rightarrow \infty$ , where the limit is a centered  $M$ -dimensional random vector which follows a multivariate normal distribution. Its covariance matrix  $\Sigma_i := [\Sigma_{im_1 m_2}]_{m_1, m_2 \in \{1, \dots, M\}}$  has the following entries:  $\Sigma_{im_1 m_2}$  given by

$$\begin{aligned} &\int_{[0, \tau)} \frac{\left\{ (\tau - u) \left(1 - \sum_{\tilde{m} \neq m_1} F_{i\tilde{m}}(u)\right) - \int_u^\tau F_{im_1}(t) dt \right\} \left\{ (\tau - u) \left(1 - \sum_{\tilde{m} \neq m_2} F_{i\tilde{m}}(u)\right) - \int_u^\tau F_{im_2}(t) dt \right\}}{(1 - \Delta A_i(u))^2} d\sigma_{im_1 m_2}(u) \\ &+ \int_{[0, \tau)} \frac{\left\{ (\tau - u) \left(1 - \sum_{\tilde{m} \neq m_1} F_{i\tilde{m}}(u)\right) - \int_u^\tau F_{im_1}(t) dt \right\} \left\{ (\tau - u)F_{im_2}(u) - \int_u^\tau F_{im_2}(t) dt \right\}}{(1 - \Delta A_i(u))^2} d \sum_{\tilde{m} \neq m_2} \sigma_{im_1 \tilde{m}}(u) \\ &+ \int_{[0, \tau)} \frac{\left\{ (\tau - u) \left(1 - \sum_{\tilde{m} \neq m_2} F_{i\tilde{m}}(u)\right) - \int_u^\tau F_{im_2}(t) dt \right\} \left\{ (\tau - u)F_{im_1}(u) - \int_u^\tau F_{im_1}(t) dt \right\}}{(1 - \Delta A_i(u))^2} d \sum_{\tilde{m} \neq m_1} \sigma_{im_2 \tilde{m}}(u) \\ &+ \int_{[0, \tau)} \frac{\left\{ (\tau - u)F_{im_1}(u) - \int_u^\tau F_{im_1}(t) dt \right\} \left\{ (\tau - u)F_{im_2}(u) - \int_u^\tau F_{im_2}(t) dt \right\}}{(1 - \Delta A_i(u))^2} d \sum_{\tilde{m} \neq m_1} \sum_{\tilde{m} \neq m_2} \sigma_{i\tilde{m} \tilde{m}}(u) \end{aligned} \quad (S2)$$

for all  $m_1, m_2 \in \{1, \dots, M\}$ . Since  $i \in \{1, \dots, k\}$  was arbitrary and the groups are independent, the statement of the theorem follows with

$$\Sigma := \bigoplus_{i=1}^k (\kappa_i^{-1} \Sigma_i) \quad (S3)$$

by Assumption 1.

## Proof of Theorem 2

First of all, we investigate the covariance matrix estimator  $\hat{\Sigma}$ .

**Lemma S1.** *Under Assumption 1, we have  $\hat{\Sigma} \xrightarrow{P} \Sigma$  as  $n \rightarrow \infty$ , where here and throughout  $\xrightarrow{P}$  denotes convergence in outer probability.*



*Proof.* By (S1), Slutsky's lemma, and the continuous mapping theorem, we have

$$\sup_{t \in [0, \tau]} |\hat{A}_{im}(t) - A_{im}(t)| \xrightarrow{P} 0, i \in \{1, \dots, k\}, m \in \{1, \dots, M\}$$

as  $n \rightarrow \infty$ . Moreover, it holds

$$\sup_{t \in [0, \tau]} |\hat{\sigma}_{im_1 m_2}(t) - \sigma_{im_1 m_2}(t)| \xrightarrow{P} 0, i \in \{1, \dots, k\}, m_1, m_2 \in \{1, \dots, M\}$$

as  $n \rightarrow \infty$  by [3]. Note that  $\Delta A_i(u) \leq 1 - S_{i-}(\tau) < 1, i \in \{1, \dots, k\}$  holds for all  $u \in [0, \tau]$ . Hence, the covariance estimator  $\hat{\Sigma}_i$  is a continuous functional of  $\hat{A}_{im_1}$  and  $\hat{\sigma}_{im_1 m_2}, m_1, m_2 \in \{1, \dots, M\}$  for all  $i \in \{1, \dots, k\}$  and, thus, the consistency  $\hat{\Sigma} \xrightarrow{P} \Sigma$  as  $n \rightarrow \infty$  follows by Assumption 1.  $\square$

Furthermore, we need that  $\Sigma$  is positive definite. The following lemma ensures this under Assumption 2.

**Lemma S2.** *Under Assumptions 1 and 2,  $\Sigma$  is positive definite.*

*Proof.* Since  $\Sigma$  is positive definite whenever  $\Sigma_i$  is positive definite for all  $i \in \{1, \dots, k\}$ , we fix  $i \in \{1, \dots, k\}$ . Now, let  $\mathbf{a} = (a_1, \dots, a_M)^\top \in \mathbb{R}^M \setminus \{\mathbf{0}_M\}$  be arbitrary. We aim to show  $\mathbf{a}^\top \Sigma_i \mathbf{a} > 0$ . By the proof of Theorem 1, it holds that

$$\mathbf{a}^\top \Sigma_i \mathbf{a} = \text{Var} \left( \sum_{m=1}^M a_m \left( \int_{[0, \tau)} f_{im} dU_{im} + \int_{[0, \tau)} g_{im} d \sum_{\tilde{m} \neq m} U_{i\tilde{m}} \right) \right) = \text{Var} \left( \sum_{m=1}^M \int_{[0, \tau)} h_{im} dU_{im} \right)$$

with

$$\begin{aligned} f_{im}(u) &:= \frac{(\tau - u) (1 - \sum_{\tilde{m} \neq m} F_{i\tilde{m}}(u)) - \int_u^\tau F_{im}(t) dt}{1 - \Delta A_i(u)}, \\ g_{im}(u) &:= \frac{(\tau - u) F_{im}(u) - \int_u^\tau F_{im}(t) dt}{1 - \Delta A_i(u)} \\ \text{and } h_{im}(u) &:= a_m f_{im}(u) + \sum_{\tilde{m} \neq m} a_{\tilde{m}} g_{i\tilde{m}}(u) \end{aligned}$$

for all  $u \in [0, \tau)$ . We can calculate this variance further as

$$\begin{aligned} \mathbf{a}^\top \Sigma_i \mathbf{a} &= \sum_{m=1}^M \mathbb{E} \left( \left( \int_{[0, \tau)} h_{im} dU_{im} \right)^2 \right) + \sum_{m=1}^M \sum_{\tilde{m} \neq m} \mathbb{E} \left( \int_{[0, \tau)} h_{im} dU_{im} \int_{[0, \tau)} h_{i\tilde{m}} dU_{i\tilde{m}} \right) \\ &= \sum_{m=1}^M \int_{[0, \tau)} h_{im}^2 \frac{1 - \Delta A_{im}}{y_i} dA_{im} - \sum_{m=1}^M \sum_{\tilde{m} \neq m} \int_{[0, \tau)} h_{im} h_{i\tilde{m}} \frac{\Delta A_{im}}{y_i} dA_{i\tilde{m}} \\ &= \sum_{m=1}^M \int_{[0, \tau)} \frac{h_{im}^2}{y_i} dA_{im} - \sum_{m=1}^M \sum_{\tilde{m} \neq m} \int_{[0, \tau)} h_{im} h_{i\tilde{m}} \frac{\Delta A_{im}}{y_i} dA_{i\tilde{m}} \\ &= \sum_{m=1}^M \int_{[0, \tau)} \frac{h_{im}^2}{y_i} dA_{im}^c + \sum_{x \in \mathcal{D}_i} \frac{\sum_{m=1}^M h_{im}^2(x) \Delta A_{im}(x) - \left( \sum_{m=1}^M h_{im}(x) \Delta A_{im}(x) \right)^2}{y_i(x)} \quad (\text{S4}) \end{aligned}$$

where  $\mathcal{D}_i = \{x \in [0, \tau) : \Delta A_i(x) > 0\}$  is the set of discontinuity time points and

$$A_{im}^c(x) := A_{im}(x) - \sum_{y \leq x, y \in \mathcal{D}_i} \Delta A_{im}(y), m \in \{1, \dots, M\}$$

denotes the continuous part of  $A_{im}$  at  $x \in [0, \tau)$ . The Cauchy-Schwarz inequality yields

$$\left( \sum_{m=1}^M h_{im}(x) \Delta A_{im}(x) \right)^2 \leq \left( \sum_{m=1}^M h_{im}^2(x) \Delta A_{im}(x) \right) \left( \sum_{m=1}^M \Delta A_{im}(x) \right)$$

and, thus,

$$\sum_{m=1}^M h_{im}^2(x) \Delta A_{im}(x) - \left( \sum_{m=1}^M h_{im}(x) \Delta A_{im}(x) \right)^2 \geq \sum_{m=1}^M h_{im}^2(x) \Delta A_{im}(x) (1 - \Delta A_i(x)) \geq 0$$

for all  $x \in \mathcal{D}_i$ . Let  $m^* \in \{1, \dots, M\}$  be the index with  $|a_{m^*}| = \max\{|a_1|, \dots, |a_M|\} > 0$ . Then, it holds

$$\begin{aligned} |h_{im^*}(u)| &= \left| a_{m^*} f_{im^*}(u) + \sum_{\tilde{m} \neq m^*} a_{\tilde{m}} g_{i\tilde{m}}(u) \right| \geq |a_{m^*}| f_{im^*}(u) - \left| \sum_{\tilde{m} \neq m^*} a_{\tilde{m}} g_{i\tilde{m}}(u) \right| \\ &\geq |a_{m^*}| \left( f_{im^*}(u) + \sum_{\tilde{m} \neq m^*} g_{i\tilde{m}}(u) \right) = |a_{m^*}| \frac{\int_u^\tau S_i(t) dt}{1 - \Delta A_i(u)} \geq |a_{m^*}| (\tau - u) \frac{S_{i-}(\tau)}{1 - \Delta A_i(u)} > 0 \end{aligned}$$

for all  $u \in [0, \tau)$  since  $|f_{im^*}(u)| = f_{im^*}(u)$ ,  $|g_{i\tilde{m}}(u)| = -g_{i\tilde{m}}(u)$  and  $1 - \Delta A_i(u) \geq S_{i-}(\tau) > 0$  for all  $u \in [0, \tau)$ ;  $\tilde{m} \in \{1, \dots, M\}$ . Note that  $A_{im^*}(\tau) > 0$  due to Assumption 2. Hence, it follows that at least one of the summands in (S4) is strictly positive and, thus,  $\mathbf{a}^\top \Sigma_i \mathbf{a} > 0$ .  $\square$

For  $\Sigma$  positive definite, it holds that  $\text{rank}(\mathbf{H}\Sigma\mathbf{H}^\top) = \text{rank}(\mathbf{H})$ . Furthermore, the consistency of the covariance matrix estimator provides

$$P\left(\text{rank}(\mathbf{H}\hat{\Sigma}\mathbf{H}^\top) \neq \text{rank}(\mathbf{H})\right) \rightarrow 0 \quad (\text{S5})$$

as  $n \rightarrow \infty$ . Note that we use the regular probability  $P$  instead of the outer probability since  $\hat{\Sigma}$  is measurable. Hence, it follows that  $(\mathbf{H}\hat{\Sigma}\mathbf{H}^\top)^+ \xrightarrow{P} (\mathbf{H}\Sigma\mathbf{H}^\top)^+$  as  $n \rightarrow \infty$ . Theorem 1, Slutsky's lemma and Theorem 9.2.2 in [8] yield

$$\begin{aligned} W_n(\mathbf{H}, \mathbf{c}) &= n(\mathbf{H}\hat{\boldsymbol{\mu}} - \mathbf{c})^\top (\mathbf{H}\hat{\Sigma}\mathbf{H}^\top)^+ (\mathbf{H}\hat{\boldsymbol{\mu}} - \mathbf{c}) \\ &= (\mathbf{H}(n^{1/2}(\hat{\boldsymbol{\mu}} - \boldsymbol{\mu})))^\top (\mathbf{H}\hat{\Sigma}\mathbf{H}^\top)^+ \mathbf{H}(n^{1/2}(\hat{\boldsymbol{\mu}} - \boldsymbol{\mu})) \xrightarrow{d} \chi_{\text{rank}(\mathbf{H})}^2 \end{aligned}$$

as  $n \rightarrow \infty$  under the null hypothesis  $\mathcal{H}_0$  in (1).

### Proof of Theorem 3

In the following, we denote all permutation counterparts of the counting processes and estimators with a  $\pi$  in the superscript, e.g.,  $Y_i^\pi, N_{im}^\pi, \hat{A}_{im}^\pi, i \in \{1, \dots, k\}, m \in \{1, \dots, M\}$ , and all counterparts for the pooled sample with a subscript  $\bullet$  instead of  $i$ , e.g.,  $Y_\bullet := \sum_{i=1}^k Y_i, N_{\bullet m} := \sum_{i=1}^k N_{im}, \hat{A}_{\bullet m}(t) := \int_{[0,t]} Y_\bullet^{-1} dN_{\bullet m}, m \in \{1, \dots, M\}$  for all  $t \geq 0$ . Furthermore, set  $y_\bullet := \sum_{i=1}^k \kappa_i y_i, F_{\bullet m} := \sum_{i=1}^k \kappa_i F_{im}, A_{\bullet m}(t) := \int_{[0,t]} y_\bullet^{-1} dF_{\bullet m}, A_\bullet := \sum_{m=1}^M A_{\bullet m}$ ,

$$S_\bullet(t) := \prod_{x \leq t} \{1 - dA_\bullet(x)\}, \quad \sigma_{\bullet m \tilde{m}}(t) := \int_{[0,t]} (\mathbb{1}\{m = \tilde{m}\} - \Delta A_{\bullet m}) y_\bullet^{-1} dA_{\bullet \tilde{m}}$$

for all  $t \geq 0; m, \tilde{m} \in \{1, \dots, M\}$  and  $\boldsymbol{\mu}_\bullet := \mathbf{1}_k \otimes \left( \int_0^\tau F_{\bullet m}(t) dt \right)_{m \in \{1, \dots, M\}}$ .

**Lemma S3.** *Under Assumption 1, we have*

$$n^{1/2} (\hat{\boldsymbol{\mu}}^\pi - \boldsymbol{\mu}_\bullet) \xrightarrow{d^*} \mathbf{Z}^\pi \sim \mathcal{N}_{kM}(\mathbf{0}_{kM}, \boldsymbol{\Sigma}^\pi)$$

as  $n \rightarrow \infty$ . The definition of the covariance matrix  $\boldsymbol{\Sigma}^\pi$  is given at the end of the proof.

*Proof of Lemma S3.* Let us consider the class

$$\mathcal{F} := \{(x, d) \mapsto \mathbb{1}\{x \geq t\}, (x, d) \mapsto \mathbb{1}\{x \leq t, d = m\} \mid t \in [0, \tau], m \in \{1, \dots, M\}\}$$

with finite envelope function  $F \equiv 1$ . It can be shown that  $\mathcal{F}$  is  $P^{(X_{i1}, D_{i1})}$ -Donsker for all  $i = 1, \dots, k$ , e.g., by applying Theorem 2.6.8 in [9]. By Theorem 1 in [7], it follows that

$$n^{1/2} (n_i^{-1} (Y_i^\pi, N_{i1}^\pi, \dots, N_{iM}^\pi) - n^{-1} (Y_\bullet, N_{\bullet 1}, \dots, N_{\bullet M}))_{i \in \{1, \dots, k\}} \xrightarrow{d^*} (\bar{G}_i, G_{i1}, \dots, G_{iM})_{i \in \{1, \dots, k\}} \quad (\text{S6})$$

on  $(D[0, \tau])^{k(M+1)}$  as  $n \rightarrow \infty$ , where  $(\bar{G}_i, G_{i1}, \dots, G_{iM})_{i \in \{1, \dots, k\}}$  denotes a tight centered Gaussian process with covariance structure

$$\begin{aligned} \mathbb{E}(\bar{G}_i(t) \bar{G}_j(s)) &= (\kappa_i^{-1} \mathbb{1}\{i = j\} - 1) (y_\bullet(\max\{t, s\}) - y_\bullet(t) y_\bullet(s)), \\ \mathbb{E}(\bar{G}_i(t) G_{jm_1}(s)) &= (\kappa_i^{-1} \mathbb{1}\{i = j\} - 1) ((F_{\bullet m_1}(s) - F_{\bullet m_1-}(t)) \mathbb{1}\{s \geq t\} - y_\bullet(t) F_{\bullet m_1}(s)), \\ \mathbb{E}(G_{im_1}(t) G_{jm_2}(s)) &= (\kappa_i^{-1} \mathbb{1}\{i = j\} - 1) (F_{\bullet m_1}(\min\{t, s\}) \mathbb{1}\{m_1 = m_2\} - F_{\bullet m_1}(t) F_{\bullet m_2}(s)) \end{aligned}$$

at  $(t, s) \in [0, \tau]^2$  for all  $i, j \in \{1, \dots, k\}, m_1, m_2 \in \{1, \dots, M\}$ . By the conditional delta-method (Theorem 4 in [7]) and the uniform Hadamard-differentiability of the Wilcoxon functional (Example 1 in [7]), we get

$$\begin{aligned} n^{1/2} (\hat{A}_{im}^\pi - \hat{A}_{\bullet m})_{i \in \{1, \dots, k\}, m \in \{1, \dots, M\}} &\xrightarrow{d^*} \left( \int_{[0, \cdot]} y_\bullet^{-1} dG_{im} - \int_{[0, \cdot]} \bar{G}_i y_\bullet^{-2} dF_{\bullet m} \right)_{i \in \{1, \dots, k\}, m \in \{1, \dots, M\}} \\ &=: (U_{im}^\pi)_{i \in \{1, \dots, k\}, m \in \{1, \dots, M\}} \end{aligned}$$

on  $(D[0, \tau])^{kM}$  as  $n \rightarrow \infty$ . The limit variable  $(U_{im}^\pi)_{i \in \{1, \dots, k\}, m \in \{1, \dots, M\}}$  is a separable centered Gaussian process and the covariance structure can be calculated similarly as in [3] as

$$\begin{aligned} \mathbb{E}(U_{im_1}^\pi(t) U_{jm_2}^\pi(s)) &= (\kappa_i^{-1} \mathbb{1}\{i = j\} - 1) \int_{[0, \min\{t, s\}]} (\mathbb{1}\{m_1 = m_2\} - \Delta A_{\bullet m_1}) y_\bullet^{-1} dA_{\bullet m_2} \\ &=: \sigma_{ijm_1m_2}^\pi(\min\{t, s\}) \end{aligned}$$

for all  $i, j \in \{1, \dots, k\}, m_1, m_2 \in \{1, \dots, M\}$  and  $t, s \in [0, \tau]$ . Furthermore, we aim to apply the conditional delta-method with the function

$$(D[0, \tau])^{kM} \ni (\Lambda_{im})_{i \in \{1, \dots, k\}, m \in \{1, \dots, M\}} \mapsto (\Phi(\Lambda_{11}, \dots, \Lambda_{1M}), \dots, \Phi(\Lambda_{k1}, \dots, \Lambda_{kM})),$$

where  $\Phi$  is defined as in the proof of Theorem 2. To show the uniform Hadamard-differentiability of  $\Phi$  at  $(A_{\bullet 1}, \dots, A_{\bullet M})$ , we remind that  $\Phi$  is a composition of linear functionals, the Wilcoxon functional  $\Psi$  and the product integral functional  $\phi$ . Hence, the chain rule together with the examples in Section 4 of [7] implies that it remains to show that  $-\sum_{m=1}^M A_{\bullet m} : [0, \tau] \rightarrow \mathbb{R}$  is a càdlàg function of bounded variation with jumps contained in  $(-1, \infty)$ , which follows by Assumption 1. Thus, we receive

$$n^{1/2}(\hat{\boldsymbol{\mu}}^\pi - \boldsymbol{\mu}_\bullet) \xrightarrow{d^*} (\Phi'_{A_{\bullet 1}, \dots, A_{\bullet M}}(U_{11}^\pi, \dots, U_{1M}^\pi), \dots, \Phi'_{A_{\bullet 1}, \dots, A_{\bullet M}}(U_{k1}^\pi, \dots, U_{kM}^\pi)) =: \mathbf{Z}^\pi$$

as  $n \rightarrow \infty$ . The limit variable  $\mathbf{Z}^\pi$  is a centered normal variable with covariance matrix  $\Sigma^\pi$ , where the entries  $\Sigma_{im_1, jm_2}^\pi$  are given by

$$\begin{aligned} & \int_{[0, \tau]} \frac{\left\{ (\tau - u) \left( 1 - \sum_{\tilde{m} \neq m_1} F_{\bullet \tilde{m}}(u) \right) - \int_u^\tau F_{\bullet m_1}(t) dt \right\} \left\{ (\tau - u) \left( 1 - \sum_{\tilde{m} \neq m_2} F_{\bullet \tilde{m}}(u) \right) - \int_u^\tau F_{\bullet m_2}(t) dt \right\}}{(1 - \Delta A_\bullet(u))^2} d\sigma_{ijm_1m_2}^\pi(u) \\ & + \int_{[0, \tau]} \frac{\left\{ (\tau - u) \left( 1 - \sum_{\tilde{m} \neq m_1} F_{\bullet \tilde{m}}(u) \right) - \int_u^\tau F_{\bullet m_1}(t) dt \right\} \left\{ (\tau - u) F_{\bullet m_2}(u) - \int_u^\tau F_{\bullet m_2}(t) dt \right\}}{(1 - \Delta A_\bullet(u))^2} d \sum_{\tilde{m} \neq m_2} \sigma_{ijm_1\tilde{m}}^\pi(u) \\ & + \int_{[0, \tau]} \frac{\left\{ (\tau - u) \left( 1 - \sum_{\tilde{m} \neq m_2} F_{\bullet \tilde{m}}(u) \right) - \int_u^\tau F_{\bullet m_2}(t) dt \right\} \left\{ (\tau - u) F_{\bullet m_1}(u) - \int_u^\tau F_{\bullet m_1}(t) dt \right\}}{(1 - \Delta A_\bullet(u))^2} d \sum_{\tilde{m} \neq m_1} \sigma_{ijm_2\tilde{m}}^\pi(u) \\ & + \int_{[0, \tau]} \frac{\left\{ (\tau - u) F_{\bullet m_1}(u) - \int_u^\tau F_{\bullet m_1}(t) dt \right\} \left\{ (\tau - u) F_{\bullet m_2}(u) - \int_u^\tau F_{\bullet m_2}(t) dt \right\}}{(1 - \Delta A_\bullet(u))^2} d \sum_{\tilde{m} \neq m_1} \sum_{\tilde{m} \neq m_2} \sigma_{ij\tilde{m}\tilde{m}}^\pi(u) \end{aligned}$$

for all  $i, j \in \{1, \dots, k\}, m_1, m_2 \in \{1, \dots, M\}$ . □

Now, we turn to the permutation counterpart of the covariance matrix estimator.

**Lemma S4.** *Under Assumption 1, we have*

$$\hat{\Sigma}^\pi \xrightarrow{P} \tilde{\Sigma}^\pi := \bigoplus_{i=1}^k \kappa_i^{-1} (\tilde{\Sigma}_{m_1m_2}^\pi)_{m_1, m_2 \in \{1, \dots, M\}}$$

as  $n \rightarrow \infty$ , where  $\tilde{\Sigma}_{m_1m_2}^\pi$  is defined as in (S7) for all  $m_1, m_2 \in \{1, \dots, M\}$ .

*Proof of Lemma S4.* Due to the definition of  $\hat{\Sigma}^\pi$ , it remains to show  $\hat{\Sigma}_{im_1, im_2}^\pi \xrightarrow{P} \tilde{\Sigma}_{m_1m_2}^\pi, i \in \{1, \dots, k\}, m_1, m_2 \in \{1, \dots, M\}$ . Therefore, let  $i \in \{1, \dots, k\}$  be arbitrary but fixed. Then, (S6) implies

$$n^{1/2} (n_i^{-1} (Y_i^\pi, N_{i1}^\pi, \dots, N_{iM}^\pi) - n^{-1} (Y_\bullet, N_{\bullet 1}, \dots, N_{\bullet M})) \xrightarrow{d} (\bar{G}_i, G_{i1}, \dots, G_{iM})$$

on  $(D[0, \tau])^{M+1}$  as  $n \rightarrow \infty$  unconditionally by Lemma 1 of [7]. Hence, Slutsky's lemma provides

$$\sup_{t \in [0, \tau]} |n_i^{-1} Y_i^\pi(t) - n^{-1} Y_\bullet(t)| \xrightarrow{P} 0 \quad \text{and} \quad \sup_{t \in [0, \tau]} |n_i^{-1} N_{im}^\pi(t) - n^{-1} N_{\bullet m}(t)| \xrightarrow{P} 0, m \in \{1, \dots, M\}$$

as  $n \rightarrow \infty$ . By the definitions of  $Y_\bullet, N_{\bullet 1}, \dots, N_{\bullet M}$ , we further get

$$\begin{aligned} \sup_{t \in [0, \tau]} |n^{-1} Y_\bullet(t) - y_\bullet(t)| &= \sup_{t \in [0, \tau]} \left| \sum_{i=1}^k \left( \frac{n_i}{n} n_i^{-1} Y_i(t) - \kappa_i y_i(t) \right) \right| \xrightarrow{P} 0 \quad \text{and} \\ \sup_{t \in [0, \tau]} |n^{-1} N_{\bullet m}(t) - F_{\bullet m}(t)| &= \sup_{t \in [0, \tau]} \left| \sum_{i=1}^k \left( \frac{n_i}{n} n_i^{-1} N_{im}(t) - \kappa_i F_{im}(t) \right) \right| \xrightarrow{P} 0, m \in \{1, \dots, M\} \end{aligned}$$

as  $n \rightarrow \infty$  since  $\mathcal{F}$  in the proof of Lemma S3 is  $P^{(X_{i1}, D_{i1})}$ -Donsker. Thus, it follows

$$\sup_{t \in [0, \tau]} |n_i^{-1} Y_i^\pi(t) - y_\bullet(t)| \xrightarrow{P} 0 \quad \text{and} \quad \sup_{t \in [0, \tau]} |n_i^{-1} N_{im}^\pi(t) - F_{\bullet m}(t)| \xrightarrow{P} 0, m \in \{1, \dots, M\}$$

as  $n \rightarrow \infty$ . Since  $\hat{A}_{im}^\pi = \int_{[0, \cdot]} n_i(Y_i^\pi)^{-1} d(n_i^{-1} N_{im}^\pi)$ ,  $\hat{F}_{im}^\pi$  and  $\hat{\sigma}_{im\tilde{m}}^\pi$  are depending continuously on  $n_i^{-1}(Y_i^\pi, N_{i1}^\pi, \dots, N_{iM}^\pi)$ , we can conclude

$$\sup_{t \in [0, \tau]} |\hat{A}_{im}^\pi(t) - A_{\bullet m}(t)| \xrightarrow{P} 0, \sup_{t \in [0, \tau]} |\hat{F}_{im}^\pi(t) - F_{\bullet m}(t)| \xrightarrow{P} 0 \quad \text{and} \quad \sup_{t \in [0, \tau]} |\hat{\sigma}_{im\tilde{m}}^\pi(t) - \sigma_{\bullet m\tilde{m}}(t)| \xrightarrow{P} 0$$

as  $n \rightarrow \infty$  for all  $m, \tilde{m} \in \{1, \dots, M\}$ . Hence, we get

$$\begin{aligned} \hat{\Sigma}_{im_1, im_2}^\pi &\xrightarrow{P} \tilde{\Sigma}_{m_1 m_2}^\pi := \\ &\int_{[0, \tau]} \frac{\left\{ (\tau - u) \left( 1 - \sum_{\tilde{m} \neq m_1} F_{\bullet \tilde{m}}(u) \right) - \int_u^\tau F_{\bullet m_1}(t) dt \right\} \left\{ (\tau - u) \left( 1 - \sum_{\tilde{m} \neq m_2} F_{\bullet \tilde{m}}(u) \right) - \int_u^\tau F_{\bullet m_2}(t) dt \right\}}{(1 - \Delta A_\bullet(u))^2} d\sigma_{\bullet m_1 m_2}(u) \\ &+ \int_{[0, \tau]} \frac{\left\{ (\tau - u) \left( 1 - \sum_{\tilde{m} \neq m_1} F_{\bullet \tilde{m}}(u) \right) - \int_u^\tau F_{\bullet m_1}(t) dt \right\} \left\{ (\tau - u) F_{\bullet m_2}(u) - \int_u^\tau F_{\bullet m_2}(t) dt \right\}}{(1 - \Delta A_\bullet(u))^2} d \sum_{\tilde{m} \neq m_2} \sigma_{\bullet m_1 \tilde{m}}(u) \\ &+ \int_{[0, \tau]} \frac{\left\{ (\tau - u) \left( 1 - \sum_{\tilde{m} \neq m_2} F_{\bullet \tilde{m}}(u) \right) - \int_u^\tau F_{\bullet m_2}(t) dt \right\} \left\{ (\tau - u) F_{\bullet m_1}(u) - \int_u^\tau F_{\bullet m_1}(t) dt \right\}}{(1 - \Delta A_\bullet(u))^2} d \sum_{\tilde{m} \neq m_1} \sigma_{\bullet m_2 \tilde{m}}(u) \\ &+ \int_{[0, \tau]} \frac{\left\{ (\tau - u) F_{\bullet m_1}(u) - \int_u^\tau F_{\bullet m_1}(t) dt \right\} \left\{ (\tau - u) F_{\bullet m_2}(u) - \int_u^\tau F_{\bullet m_2}(t) dt \right\}}{(1 - \Delta A_\bullet(u))^2} d \sum_{\tilde{m} \neq m_1} \sum_{\tilde{m} \neq m_2} \sigma_{\bullet \tilde{m} \tilde{m}}(u) \end{aligned} \tag{S7}$$

as  $n \rightarrow \infty$ . □

As in the proof of Theorem 2, we need the positive definiteness of  $\tilde{\Sigma}^\pi$ , which is given by the following lemma.

**Lemma S5.** Under Assumptions 1 and 2,  $\tilde{\Sigma}^\pi$  is positive definite.

*Proof of Lemma S5.* The proof is similar to the proof of Lemma S2. Firstly note that  $\tilde{\Sigma}^\pi$  is positive definite if  $(\tilde{\Sigma}_{m_1 m_2}^\pi)_{m_1, m_2 \in \{1, \dots, M\}}$  is positive definite. Let  $\mathbf{a} = (a_1, \dots, a_M)^\top \in \mathbb{R}^M \setminus \{\mathbf{0}_M\}$  be arbitrary. With

$$\begin{aligned} f_m(u) &:= \frac{(\tau - u)(1 - \sum_{\tilde{m} \neq m} F_{\bullet, \tilde{m}}(u)) - \int_u^\tau F_{\bullet, m}(t) dt}{1 - \Delta A_{\bullet}(u)}, \\ g_m(u) &:= \frac{(\tau - u)F_{\bullet, m}(u) - \int_u^\tau F_{\bullet, m}(t) dt}{1 - \Delta A_{\bullet}(u)} \\ \text{and } h_m(u) &:= a_m f_m(u) + \sum_{\tilde{m} \neq m} a_{\tilde{m}} g_{\tilde{m}}(u) \end{aligned}$$

for all  $u \in [0, \tau)$ , we get

$$\mathbf{a}^\top (\tilde{\Sigma}_{m_1 m_2}^\pi)_{m_1, m_2 \in \{1, \dots, M\}} \mathbf{a} = \sum_{m=1}^M \int_{[0, \tau)} \frac{h_m^2}{y_{\bullet}} dA_{\bullet, m}^c \quad (\text{S8})$$

$$+ \sum_{x \in \mathcal{D}} \frac{\sum_{m=1}^M h_m^2(x) \Delta A_{\bullet, m}(x) - \left( \sum_{m=1}^M h_m(x) \Delta A_{\bullet, m}(x) \right)^2}{y_{\bullet}(x)} \quad (\text{S9})$$

analogously to the proof of Lemma S2, where  $\mathcal{D} := \{x \in [0, \tau) : \Delta A_{\bullet}(x) > 0\}$  and

$$A_{\bullet, m}^c(x) := A_{\bullet, m}(x) - \sum_{y \leq x, y \in \mathcal{D}} \Delta A_{\bullet, m}(y), m \in \{1, \dots, M\}$$

for all  $x \in [0, \tau)$ . The Cauchy-Schwarz inequality implies

$$\sum_{m=1}^M h_m^2(x) \Delta A_{\bullet, m}(x) - \left( \sum_{m=1}^M h_m(x) \Delta A_{\bullet, m}(x) \right)^2 \geq \sum_{m=1}^M h_m^2(x) \Delta A_{\bullet, m}(x) (1 - \Delta A_{\bullet}(x)) \geq 0$$

for all  $x \in \mathcal{D}$ . For  $m^* \in \{1, \dots, M\}$  with  $|a_{m^*}| = \max\{|a_1|, \dots, |a_M|\} > 0$ , it holds

$$\begin{aligned} |h_{m^*}(u)| &= \left| a_{m^*} f_{m^*}(u) + \sum_{\tilde{m} \neq m^*} a_{\tilde{m}} g_{\tilde{m}}(u) \right| \geq |a_{m^*}| f_{m^*}(u) - \left| \sum_{\tilde{m} \neq m^*} a_{\tilde{m}} g_{\tilde{m}}(u) \right| \\ &\geq |a_{m^*}| \left( f_{m^*}(u) + \sum_{\tilde{m} \neq m^*} g_{\tilde{m}}(u) \right) = |a_{m^*}| \frac{\sum_{i=1}^k \kappa_i \int_u^\tau S_i(t) dt}{1 - \Delta A_{\bullet}(u)} \\ &\geq |a_{m^*}| \frac{(\tau - u) \sum_{i=1}^k \kappa_i S_i(\tau)}{1 - \Delta A_{\bullet}(u)} > 0 \end{aligned}$$

for all  $u \in [0, \tau)$  since  $|f_{m^*}(u)| = f_{m^*}(u)$ ,  $|g_{\tilde{m}}(u)| = -g_{\tilde{m}}(u)$  and

$$\Delta A_{\bullet}(u) = \frac{\sum_{i=1}^k \kappa_i y_i(u) \Delta A_i(u)}{\sum_{i=1}^k \kappa_i y_i(u)} < 1$$

for all  $u \in [0, \tau)$ ;  $\tilde{m} \in \{1, \dots, M\}$ . Note that  $A_{\bullet, m^*}(\tau) > 0$  due to Assumption 2. Thus, at least one of the summands (S8) and (S9) is strictly positive.  $\square$

Note that  $\sigma_{ijm_1m_2}^\pi = (\kappa_i^{-1} \mathbb{1}\{i=j\} - 1) \sigma_{\bullet m_1m_2}$  for all  $i, j \in \{1, \dots, k\}, m_1, m_2 \in \{1, \dots, M\}$ . Hence, it holds  $\tilde{\Sigma}^\pi = \Sigma^\pi + (\mathbf{1}_k \mathbf{1}_k^\top) \otimes (\tilde{\Sigma}_{m_1m_2}^\pi)_{m_1, m_2 \in \{1, \dots, M\}}$  and, thus,  $\mathbf{H} \hat{\Sigma}^\pi \mathbf{H}^\top \xrightarrow{P} \mathbf{H} \tilde{\Sigma}^\pi \mathbf{H}^\top = \mathbf{H} \Sigma^\pi \mathbf{H}^\top$  as  $n \rightarrow \infty$  due to the contrast property of the hypothesis matrix  $\mathbf{H}$ . The positive definiteness of  $\tilde{\Sigma}^\pi$  ensures

$$\text{rank}(\mathbf{H} \Sigma^\pi \mathbf{H}^\top) = \text{rank}(\mathbf{H} \tilde{\Sigma}^\pi \mathbf{H}^\top) = \text{rank}(\mathbf{H}).$$

As in the proof of Theorem 2, we get  $(\mathbf{H} \hat{\Sigma}^\pi \mathbf{H}^\top)^+ \xrightarrow{P} (\mathbf{H} \Sigma^\pi \mathbf{H}^\top)^+$  as  $n \rightarrow \infty$ . Combining this with Lemma S3, Slutsky's lemma and Theorem 9.2.2 in [8] yields

$$\begin{aligned} W_n^\pi(\mathbf{H}) &= n(\mathbf{H} \hat{\boldsymbol{\mu}}^\pi)^\top \left( \mathbf{H} \hat{\Sigma}^\pi \mathbf{H}^\top \right)^+ (\mathbf{H} \hat{\boldsymbol{\mu}}^\pi) \\ &= \left( \mathbf{H}(n^{1/2}(\hat{\boldsymbol{\mu}}^\pi - \boldsymbol{\mu}_\bullet)) \right)^\top \left( \mathbf{H} \hat{\Sigma}^\pi \mathbf{H}^\top \right)^+ \left( \mathbf{H}(n^{1/2}(\hat{\boldsymbol{\mu}}^\pi - \boldsymbol{\mu}_\bullet)) \right) \\ &\xrightarrow{d^*} (\mathbf{H} \mathbf{Z}^\pi)^\top (\mathbf{H} \Sigma^\pi \mathbf{H}^\top)^+ (\mathbf{H} \mathbf{Z}^\pi) \sim \chi_{\text{rank}(\mathbf{H})}^2 \end{aligned}$$

as  $n \rightarrow \infty$ .

## Proof of Proposition 1

First of all, we aim to show  $q_{1-\alpha}^\pi \xrightarrow{P} \chi_{\text{rank}(\mathbf{H}), 1-\alpha}^2$  as  $n \rightarrow \infty$ . Therefore, we firstly state an in-probability version of Lemma S4 in the supplement of [5].

**Lemma S6.** *Let  $L \in \mathbb{N}$ ,  $F : \mathbb{R}^L \rightarrow [0, 1]$  be a continuous cumulative distribution function and  $(F_n)_{n \in \mathbb{N}}$  denote a sequence of maps taking values in the space of all cumulative distribution functions with*

$$F_n(\mathbf{t}) \xrightarrow{P} F(\mathbf{t}) \text{ as } n \rightarrow \infty \text{ for all } \mathbf{t} \in \mathbb{R}^L. \quad (\text{S10})$$

*Then, we have  $\sup_{\mathbf{t} \in \mathbb{R}^L} |F_n(\mathbf{t}) - F(\mathbf{t})| \xrightarrow{P} 0$  as  $n \rightarrow \infty$ .*

*Proof of Lemma S6.* To show this, we proceed similarly as in the proof of Lemma S4 in the supplement of [5]. Let  $f_{\mathbf{t}} : \mathbb{R}^L \rightarrow \mathbb{R}, f_{\mathbf{t}}(x_1, \dots, x_L) = \mathbb{1}\{x_1 \leq t_1, \dots, x_L \leq t_L\}$  for all  $\mathbf{t} = (t_1, \dots, t_L)^\top \in (\mathbb{R} \cup \{-\infty, \infty\})^L$ ,  $\mathbf{F} := \{f_{\mathbf{t}} \mid \mathbf{t} \in (\mathbb{R} \cup \{-\infty, \infty\})^L\}$  and  $\varepsilon > 0$  be arbitrary. Then, the bracketing number of  $\mathbf{F}$  is bounded by  $(m+1)^L$  for some  $m \in \mathbb{N}$  as shown in the proof of Lemma S4 in the supplement of [5]. As in the proof of Proposition 2.1 in [1], it holds

$$\sup_{\mathbf{w} \in \mathbb{R}^L} |F_n(\mathbf{w}) - F(\mathbf{w})| \leq 3 \max\{|F_n(\mathbf{w}) - F(\mathbf{w})|\} + 2\varepsilon,$$

where the maximum is taken over  $2(m+1)^L$  different values  $\mathbf{w} \in \mathbb{R}^L$ . Hence, we get

$$P^* \left( \sup_{\mathbf{w} \in \mathbb{R}^L} |F_n(\mathbf{w}) - F(\mathbf{w})| > 3\varepsilon \right) \leq P^* (\max\{|F_n(\mathbf{w}) - F(\mathbf{w})|\} > \varepsilon),$$

where  $P^*$  denotes the outer probability. The latter tends to 0 by assumption since the maximum is taken over a finite number of values  $\mathbf{w} \in \mathbb{R}^L$ .  $\square$

The following lemma can be used to show condition (S10) for a consistent resampling scheme. Here,  $\mathbf{X}_n$  represents the randomness of the data while  $\mathbf{Y}_n^{(1)}, \mathbf{Y}_n^{(2)}, \dots$  can be interpreted as the randomness of the resampling method.

**Lemma S7.** *Let  $\mathbf{X}_n : \Omega \rightarrow \chi_{1n}, \mathbf{Y}_n^{(1)} : \Omega_1 \rightarrow \chi_{2n}, \mathbf{Y}_n^{(2)} : \Omega_2 \rightarrow \chi_{2n}, \dots$  denote independent maps defined on probability spaces  $\Omega, \Omega_1, \Omega_2, \dots$  for  $n \in \mathbb{N}$ , where independence is understood in terms of a product probability space, cf. Section 2.3.1 in [10]. Furthermore, assume that  $\mathbf{Y}_n^{(1)}, \mathbf{Y}_n^{(2)}, \dots$  are identically distributed and  $\mathbf{W}_n : \chi_{1n} \times \chi_{2n} \rightarrow \mathbb{R}^L$  is a function for  $L, n \in \mathbb{N}$ . Suppose that  $F_n$  is the empirical distribution function of  $\mathbf{W}_n^{(b)} := \mathbf{W}_n(\mathbf{X}_n, \mathbf{Y}_n^{(b)})$ ,  $b \in \{1, \dots, B_n\}$  for  $B_n, n \in \mathbb{N}$  satisfying  $\mathbf{W}_n^{(1)} \xrightarrow{d^*} \mathbf{W} \sim F$  as  $n \rightarrow \infty$  conditionally on  $\mathbf{X}_n$ , where  $F : \mathbb{R}^L \rightarrow [0, 1]$  denotes a continuous cumulative distribution function. Then, (S10) is satisfied if  $B_n \rightarrow \infty$  as  $n \rightarrow \infty$ .*

*Proof of Lemma S7.* Let  $\mathbf{t} \in \mathbb{R}^L$  be arbitrary. Approximate  $f : \mathbb{R}^L \rightarrow \{0, 1\}, \mathbf{w} \mapsto \mathbb{1}\{\mathbf{w} \leq \mathbf{t}\}$  through sequences of Lipschitz functions  $(g_m)_{m \in \mathbb{N}}, (h_m)_{m \in \mathbb{N}}$  with  $1 \geq g_m \geq f \geq h_m \geq 0$  and  $\mathbb{E}[g_m(\mathbf{W}) - h_m(\mathbf{W})] \leq m^{-1}$  for all  $m \in \mathbb{N}$ , where  $\mathbf{x} \leq \mathbf{t}$  means that all components of  $\mathbf{x}$  are less than or equal to the corresponding values in the vector  $\mathbf{t}$ . Let  $\mathbb{E}_2^*$  denote the outer expectation with respect to the product space  $\times_{i=1}^\infty \Omega_i$ , cf. Section 1.2 in [10]. Then, it holds

$$\begin{aligned}
& |\mathbb{E}_2[f(\mathbf{W}_n^{(1)})^*] - \mathbb{E}[f(\mathbf{W})]| \\
& \leq \mathbb{E}_2[f(\mathbf{W}_n^{(1)})^*] - \mathbb{E}_2^*[f(\mathbf{W}_n^{(1)})] + |\mathbb{E}_2^*[f(\mathbf{W}_n^{(1)})] - \mathbb{E}[f(\mathbf{W})]| \\
& \leq \mathbb{E}_2[g_m(\mathbf{W}_n^{(1)})^*] - \mathbb{E}_2^*[h_m(\mathbf{W}_n^{(1)})] \\
& \quad + \max\{\mathbb{E}_2^*[g_m(\mathbf{W}_n^{(1)})] - \mathbb{E}[g_m(\mathbf{W})], \mathbb{E}[h_m(\mathbf{W})] - \mathbb{E}_2^*[h_m(\mathbf{W}_n^{(1)})]\} \\
& \quad + \mathbb{E}[g_m(\mathbf{W})] - \mathbb{E}[h_m(\mathbf{W})] \\
& \leq \mathbb{E}_2[g_m(\mathbf{W}_n^{(1)})^* - g_m(\mathbf{W}_n^{(1)})_*] + \mathbb{E}_2^*[g_m(\mathbf{W}_n^{(1)})] - \mathbb{E}_2^*[h_m(\mathbf{W}_n^{(1)})] \\
& \quad + \max\{\mathbb{E}_2^*[g_m(\mathbf{W}_n^{(1)})] - \mathbb{E}[g_m(\mathbf{W})], \mathbb{E}[h_m(\mathbf{W})] - \mathbb{E}_2^*[h_m(\mathbf{W}_n^{(1)})]\} + m^{-1} \\
& \xrightarrow{P} 0 + \mathbb{E}[g_m(\mathbf{W})] - \mathbb{E}[h_m(\mathbf{W})] + 0 + m^{-1} \leq 2m^{-1},
\end{aligned}$$

where here and throughout  $A^*$  and  $A_*$  denote the minimal measurable majorant and maximal measurable minorant, respectively, for a map  $A$  with respect to all probability spaces jointly. By choosing  $m$  sufficiently large, it follows

$$\mathbb{E}_2[f(\mathbf{W}_n^{(1)})^*] \xrightarrow{P} \mathbb{E}[f(\mathbf{W})] = F(\mathbf{t})$$

as  $n \rightarrow \infty$ . Analogously, one can show  $\mathbb{E}_2[f(\mathbf{W}_n^{(1)})_*] \xrightarrow{P} F(\mathbf{t})$  as  $n \rightarrow \infty$ . Since  $B_n \rightarrow \infty$  as



$n \rightarrow \infty$ , we have

$$\begin{aligned}
& \mathbb{E}_2 \left[ (|F_n(\mathbf{t}) - F(\mathbf{t})|^2)^* \right] \\
& \leq \mathbb{E}_2 \left[ (F_n^2(\mathbf{t}))^* \right] + 2\mathbb{E}_2 \left[ (-F_n(\mathbf{t}))^* \right] F(\mathbf{t}) + F^2(\mathbf{t}) \\
& \leq \frac{1}{B_n^2} \sum_{b_1, b_2=1}^{B_n} \mathbb{E}_2 \left[ (f(\mathbf{W}_n^{(b_1)}) f(\mathbf{W}_n^{(b_2)}))^* \right] + \frac{2}{B_n} \sum_{b=1}^{B_n} \mathbb{E}_2 \left[ (-f(\mathbf{W}_n^{(b)}))^* \right] F(\mathbf{t}) + F^2(\mathbf{t}) \\
& \leq \frac{1}{B_n} + \frac{1}{B_n^2} \sum_{b_1, b_2=1, b_1 \neq b_2}^{B_n} \mathbb{E}_2 \left[ f(\mathbf{W}_n^{(b_1)})^* \right] \mathbb{E}_2 \left[ f(\mathbf{W}_n^{(b_2)})^* \right] - 2\mathbb{E}_2 \left[ f(\mathbf{W}_n^{(1)})^* \right] F(\mathbf{t}) + F^2(\mathbf{t}) \\
& \leq \frac{1}{B_n} + \frac{B_n - 1}{B_n} \mathbb{E}_2 \left[ f(\mathbf{W}_n^{(1)})^* \right]^2 - 2\mathbb{E}_2 \left[ f(\mathbf{W}_n^{(1)})^* \right] F(\mathbf{t}) + F^2(\mathbf{t}) \\
& \xrightarrow{P} F^2(\mathbf{t}) - 2F(\mathbf{t})F(\mathbf{t}) + F^2(\mathbf{t}) = 0
\end{aligned}$$

as  $n \rightarrow \infty$ . Thus,  $\mathbb{E}^* \left[ |F_n(\mathbf{t}) - F(\mathbf{t})|^2 \right] \rightarrow 0$  as  $n \rightarrow \infty$  for all  $\mathbf{t} \in \mathbb{R}^L$  by the dominated convergence theorem (dominated by 1). Hence, (S10) in Lemma S8 follows.  $\square$

We apply both lemmas with  $F(\cdot) = \chi_{\text{rank}(\mathbf{H})}^2((-\infty, \cdot])$  and  $F_n$  being the empirical distribution function of the permutation counterparts of the Wald-type test statistic. Hence, we receive

$$\sup_{t \in \mathbb{R}} |F_n(t) - F(t)| \xrightarrow{P} 0$$

as  $n \rightarrow \infty$  by Theorem 3.

Moreover, the subsequence criterion (Lemma 1.9.2 (ii) in [10]) provides that every subsequence has a further subsequence such that  $\sup_{t \in \mathbb{R}} |F_n(t) - F(t)| \rightarrow 0$  holds outer almost surely along the latter subsequence. By proceeding as in the proof of Lemma S3 in the supplement of [5], we get  $q_{1-\alpha}^\pi \rightarrow \chi_{\text{rank}(\mathbf{H}), 1-\alpha}^2$  outer almost surely along the subsequence. Applying the subsequence criterion again yields  $q_{1-\alpha}^\pi \xrightarrow{P} \chi_{\text{rank}(\mathbf{H}), 1-\alpha}^2$  as  $n \rightarrow \infty$ .

By Slutsky's lemma and Theorem 2, it follows  $(W_n(\mathbf{H}, \mathbf{c}), q_{1-\alpha}^\pi) \xrightarrow{d} (W, \chi_{\text{rank}(\mathbf{H}), 1-\alpha}^2)$  as  $n \rightarrow \infty$  for  $W \sim \chi_{\text{rank}(\mathbf{H})}^2$ . By approximating the function  $f : \mathbb{R}^2 \rightarrow \{0, 1\}$ ,  $f(w, q) := \mathbb{1}\{w > q\}$  with sequences of Lipschitz functions  $(g_m)_{m \in \mathbb{N}}, (h_m)_{m \in \mathbb{N}}$  with  $1 \geq g_m \geq f \geq h_m \geq 0$  and

$$\mathbb{E} \left[ g_m(W, \chi_{\text{rank}(\mathbf{H}), 1-\alpha}^2) - h_m(W, \chi_{\text{rank}(\mathbf{H}), 1-\alpha}^2) \right] \leq m^{-1}$$

for all  $m \in \mathbb{N}$ , one can follow similarly as in the proof of Lemma S7 that

$$\mathbb{E}(\varphi^\pi) = \mathbb{E} \left[ f(W_n(\mathbf{H}, \mathbf{c}), q_{1-\alpha}^\pi) \right] \rightarrow \mathbb{E} \left[ f(W, \chi_{\text{rank}(\mathbf{H}), 1-\alpha}^2) \right] = P(W > \chi_{\text{rank}(\mathbf{H}), 1-\alpha}^2) = \alpha$$

holds as  $n \rightarrow \infty$ . Here, we can use the regular expectation  $\mathbb{E}$  instead of the outer expectation due to the measurability of  $W_n(\mathbf{H}, \mathbf{c})$  and  $q_{1-\alpha}^\pi$ .

## Proof of Theorem 4

By Slutsky's lemma, we combine Theorem 1 and Lemma S1 for Theorem 4. Since the map

$$\mathbb{R}^{kM} \times \mathbb{R}^{kM \times kM} \ni (\mathbf{m}, \mathbf{S}) \mapsto ((\mathbf{H}_\ell \mathbf{m})' (\mathbf{H}_\ell \mathbf{S} \mathbf{H}_\ell')^+ \mathbf{H}_\ell \mathbf{m})_{\ell \in \mathcal{T}} \in \mathbb{R}^{\mathcal{T}}$$

is continuous on  $\mathbb{R}^{kM} \times \{\Sigma\}$  due to Lemma S2, the statement follows by the continuous mapping theorem.

## Proof of Proposition 2

The following lemma is a version of Lemma S3 in [6] that helps to prove the convergence of the critical values.

**Lemma S8.** *Let  $L \in \mathbb{N}$  and  $\alpha \in (0, 1)$ . Moreover, let  $F_n$  denote a map taking values in the space of all cumulative distribution functions on  $\mathbb{R}^L$  and  $F_{n,\ell}, \ell \in \{1, \dots, L\}$  denote maps taking values in the space of all cumulative distribution functions on  $\mathbb{R}$  for all  $n \in \mathbb{N}$ . Additionally, let  $F : \mathbb{R}^L \rightarrow [0, 1]$  denote a continuous cumulative distribution function with marginal distribution functions  $F_1, \dots, F_L : \mathbb{R} \rightarrow [0, 1]$ , where  $F_\ell$  is strictly increasing on  $[F_\ell^{-1}(a), F_\ell^{-1}(b)]$ ,  $\ell \in \{1, \dots, L\}$  with*

$$0 < a < 1 - \alpha \leq 1 - \alpha/L < b < 1.$$

If (S10) and

$$F_{n,\ell}(t) \xrightarrow{P} F_\ell(t) \text{ as } n \rightarrow \infty \text{ for all } t \in \mathbb{R}; \ell \in \{1, \dots, L\} \quad (\text{S11})$$

hold, we have

$$F_{n,\ell}^{-1}(1 - \beta_n(\alpha)) \xrightarrow{P} F_\ell^{-1}(1 - \text{FWER}^{-1}(\alpha))$$

as  $n \rightarrow \infty$  for all  $\ell \in \{1, \dots, L\}$ , where

$$\text{FWER} : \mathbb{R} \rightarrow [0, 1], \quad \text{FWER}(\beta) := 1 - F((F_\ell^{-1}(1 - \beta))_{\ell \in \{1, \dots, L\}})$$

and  $\beta_n(\alpha) \in [0, 1]$  satisfying  $\beta_n(\alpha) \in [\text{FWER}_n^{-1}(\alpha) - \varepsilon_n, \text{FWER}_n^{-1}(\alpha + \varepsilon_n)]$  for all  $n \in \mathbb{N}$  with

$$\text{FWER}_n(\beta) := 1 - F_n((F_{n,\ell}^{-1}(1 - \beta))_{\ell \in \{1, \dots, L\}}) \quad \text{for all } \beta \in [0, 1]$$

and some null sequence  $(\varepsilon_n)_{n \in \mathbb{N}} \subset [0, \infty)$ .

The statement can be proved analogously to Lemma S3 in the supplement of [6]. However, we want to emphasize that all convergences stated there hold in outer probability. That is because

$$\sup_{\mathbf{t} \in \mathbb{R}^L} |F_n(\mathbf{t}) - F(\mathbf{t})| \xrightarrow{P} 0 \quad \text{as } n \rightarrow \infty$$

holds by Lemma S6 and there is an outer probability analogue of the subsequence criterion in Lemma 1.9.2 (ii) in [10].

**Remark 1.** If  $F_{n,1}, \dots, F_{n,L}$  are the marginal cumulative distribution functions of  $F_n$  in Lemma S8, (S11) is a direct consequence of (S10).

In order to prove Proposition 2, let  $F_n$  denote the empirical distribution function of

$$\left( (\mathbf{H}_\ell \hat{\Sigma}^{1/2} \mathbf{Y}^{(b)})^\top (\mathbf{H}_\ell \hat{\Sigma} \mathbf{H}_\ell^\top)^+ (\mathbf{H}_\ell \hat{\Sigma}^{1/2} \mathbf{Y}^{(b)}) \right)_{\ell \in \{1, \dots, L\}}, b \in \{1, \dots, B_n\},$$

$F_{n,\ell}(\cdot) = \chi_{\text{rank}(\mathbf{H}_\ell \hat{\Sigma} \mathbf{H}_\ell^\top)}^2((-\infty, \cdot])$  and  $F$  being the distribution function of  $(W_\ell)_{\ell \in \{1, \dots, L\}}$ . It should be noted that

$$\begin{aligned} \beta_n(\alpha) &:= \max \{ \beta \in \{0, 1/B_n, \dots, (B_n - 1)/B_n\} \mid \text{FWER}_n(\beta) \leq \alpha \} \\ &= \begin{cases} \text{FWER}_n^{-1}(\alpha + 1/B_n) - 1/B_n & \text{if } \alpha B_n \in \mathbb{N} \\ \text{FWER}_n^{-1}(\alpha) - 1/B_n & \text{if } \alpha B_n \notin \mathbb{N} \end{cases} \end{aligned}$$

suffices the conditions on  $\beta_n(\alpha)$  in Lemma S8 with  $\varepsilon_n = 1/B_n$  for all  $n \in \mathbb{N}$ . Due to Lemma S1, (S5) and Lemma S7, (S10) and (S11) hold. Thus, Lemma S8 provides

$$\chi_{\text{rank}(\mathbf{H}_\ell), 1-\beta_n(\alpha)}^2 \xrightarrow{P} \chi_{\text{rank}(\mathbf{H}_\ell), 1-\text{FWER}^{-1}(\alpha)}^2$$

as  $n \rightarrow \infty$  by (S5). Furthermore, it follows

$$(W_n(\mathbf{H}_\ell, \mathbf{c}_\ell), \chi_{\text{rank}(\mathbf{H}_\ell), 1-\beta_n(\alpha)}^2)_{\ell \in \mathcal{T}} \xrightarrow{d} (W_\ell, \chi_{\text{rank}(\mathbf{H}_\ell), 1-\text{FWER}^{-1}(\alpha)}^2)_{\ell \in \mathcal{T}}$$

as  $n \rightarrow \infty$  under  $\mathcal{H}_{0,\ell}, \ell \in \mathcal{T}$ , by Theorem 4 and Slutsky's lemma. Similarly as in the proof of Proposition 1, we approximate the function  $f : (w_\ell, q_\ell)_{\ell \in \mathcal{T}} \mapsto \max_{\ell \in \mathcal{T}} \mathbb{1}\{w_\ell > q_\ell\}$  through Lipschitz functions to obtain

$$\begin{aligned} \mathbb{E} \left( \max_{\ell \in \mathcal{T}} \varphi_\ell \right) &= \mathbb{E} \left( f \left( (W_n(\mathbf{H}_\ell, \mathbf{c}_\ell), \chi_{\text{rank}(\mathbf{H}_\ell), 1-\beta_n(\alpha)}^2)_{\ell \in \mathcal{T}} \right) \right) \\ &\rightarrow \mathbb{E} \left( f \left( (W_\ell, \chi_{\text{rank}(\mathbf{H}_\ell), 1-\text{FWER}^{-1}(\alpha)}^2)_{\ell \in \mathcal{T}} \right) \right) \\ &\leq 1 - F \left( \left( \chi_{\text{rank}(\mathbf{H}_\ell), 1-\text{FWER}^{-1}(\alpha)}^2 \right)_{\ell \in \{1, \dots, L\}} \right) \\ &= \text{FWER}(\text{FWER}^{-1}(\alpha)) = \alpha \end{aligned}$$

as  $n \rightarrow \infty$  holds under  $\mathcal{H}_{0,\ell}, \ell \in \mathcal{T}$ . Here, we can use the regular expectation  $\mathbb{E}$  instead of the outer expectation due to the measurability of  $W_n(\mathbf{H}_\ell, \mathbf{c}_\ell)$  and  $\chi_{\text{rank}(\mathbf{H}_\ell), 1-\beta_n(\alpha)}^2$ . The inequality is an equality if  $\mathcal{T} = \{1, \dots, L\}$ .

## B Details on the Simulation Study

### B.1 Simulation Settings

For the survival and censoring distributions, the same settings as in [5] are considered. Hence, the survival distributions are given by the following:

- Exponential distributions and early departures (*exp early*):  $T_{11}, T_{21}, T_{31} \sim \text{Exp}(0.2)$  and  $T_{41}$  with piece-wise constant hazard function  $t \mapsto \lambda_{\delta,1} \cdot \mathbb{1}\{t \leq 2\} + 0.2 \cdot \mathbb{1}\{t > 2\}$ ,
- exponential distributions and late departures (*exp late*):  $T_{11}, T_{21}, T_{31} \sim \text{Exp}(0.2)$  and  $T_{41}$  with piece-wise constant hazard function  $t \mapsto 0.2 \cdot \mathbb{1}\{t \leq 2\} + \lambda_{\delta,2} \cdot \mathbb{1}\{t > 2\}$ ,
- exponential distributions and proportional hazard alternative (*exp prop*):  $T_{11}, T_{21}, T_{31} \sim \text{Exp}(0.2)$  and  $T_{41} \sim \text{Exp}(\lambda_{\delta,3})$ ,
- lognormal distributions with scale alternatives (*logn*):  $T_{11}, T_{21}, T_{31} \sim \log N(2, 0.25)$  and  $T_{41} \sim \log N(\lambda_{\delta,4}, 0.25)$ ,
- exponential distributions and piece-wise exponential distributions (*pwExp*):  $T_{11}, T_{21}, T_{31} \sim \text{Exp}(0.2)$  and  $T_{41}$  with piece-wise constant hazard function  $t \mapsto 0.5 \cdot \mathbb{1}\{t \leq \lambda_{\delta,5}\} + 0.05 \cdot \mathbb{1}\{t > \lambda_{\delta,5}\}$ ,
- Weibull distributions and late departures (*Weib late*):  $T_{11}, T_{21}, T_{31} \sim \text{Weib}(3, 8)$  and  $T_{41} \sim \text{Weib}(3 \cdot \lambda_{\delta,6}, 8/\lambda_{\delta,6})$ ,
- Weibull distributions and proportional hazard alternative (*Weib prop*):  $T_{11}, T_{21}, T_{31} \sim \text{Weib}(3, 8)$  and  $T_{41} \sim \text{Weib}(3, \lambda_{\delta,7})$ ,
- Weibull distributions with crossing curves and scale alternatives (*Weib scale*):  $T_{11}, T_{21}, T_{31} \sim \text{Weib}(3, 8)$  and  $T_{41} \sim \text{Weib}(1.5, \lambda_{\delta,8})$ ,
- Weibull distributions with crossing curves and shape alternatives (*Weib shape*):  $T_{11}, T_{21}, T_{31} \sim \text{Weib}(3, 8)$  and  $T_{41} \sim \text{Weib}(\lambda_{\delta,9}, 14)$ .

The parameters  $\lambda_{\delta,1}, \dots, \lambda_{\delta,9}$  are determined as in [2] such that the restricted mean survival time difference equals  $\delta = \int_{[0,\tau]} S_1(t)dt - \int_{[0,\tau]} S_4(t)dt$ . As explained in Section 4.1, this results in RMTL differences of  $\mu_{4m} - \mu_{1m} = p_m \delta$  for all events  $m = 1, \dots, M$ .

The following three scenarios are chosen for the censoring times:

- Equally Weibull distributed censoring times (*equal*):  $C_{11}, C_{21}, C_{31}, C_{41} \sim \text{Weib}(3, 10)$ ,
- unequally Weibull distributed censoring times with high censoring rates (*unequal, high*):  $C_{11} \sim \text{Weib}(0.5, 15)$ ,  $C_{21} \sim \text{Weib}(0.5, 10)$ ,  $C_{31} \sim \text{Weib}(1, 8)$  and  $C_{41} \sim \text{Weib}(1, 10)$ ,
- unequally Weibull distributed censoring times with low censoring rates (*unequal, low*):  $C_{11} \sim \text{Weib}(1, 20)$ ,  $C_{21} \sim \text{Weib}(3, 10)$ ,  $C_{31} \sim \text{Weib}(1, 15)$  and  $C_{41} \sim \text{Weib}(3, 20)$ .

## B.2 Additional Figures of Simulation Results

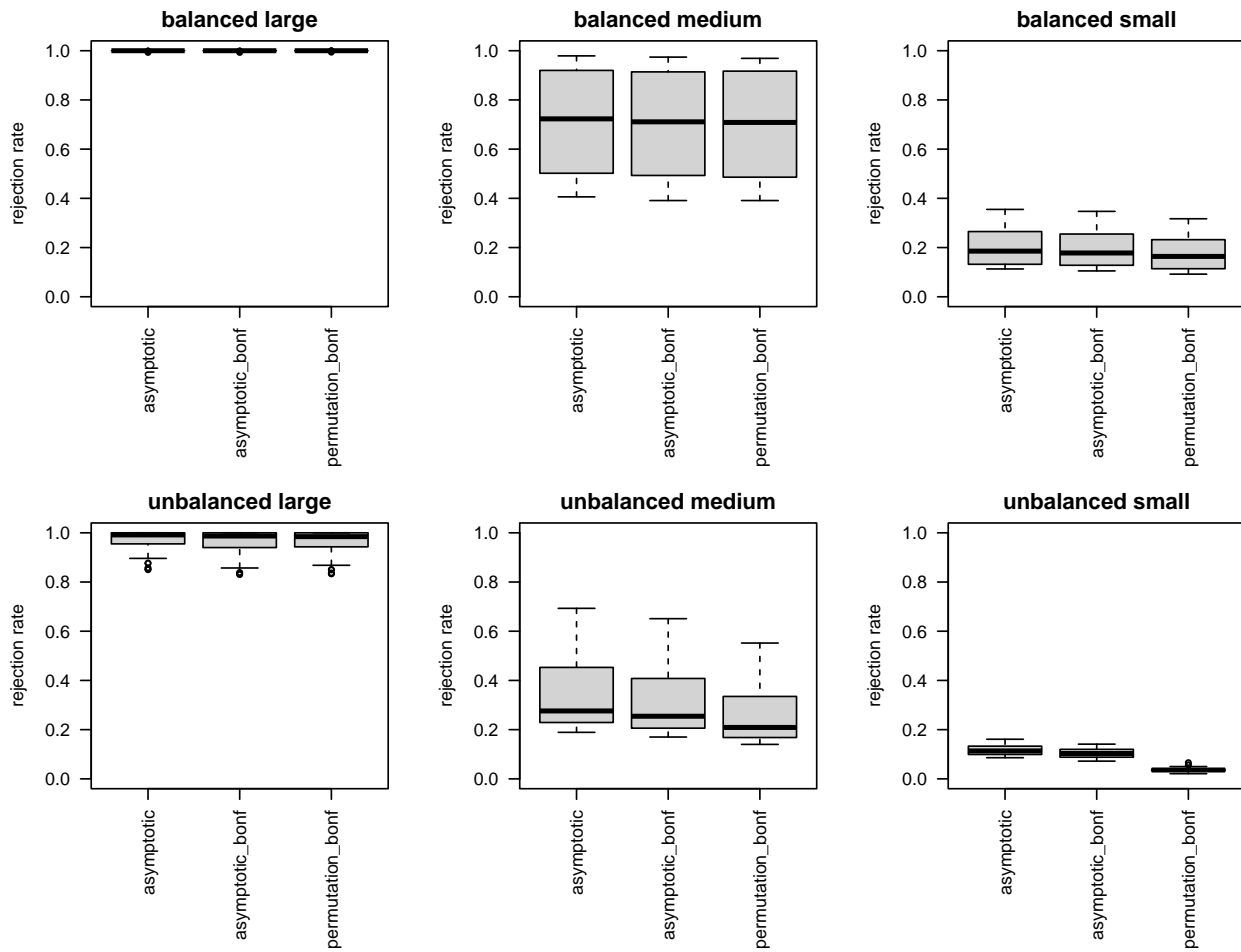

Figure S1: Empirical powers for the 2-by-2 design across all scenarios under the alternative hypothesis.

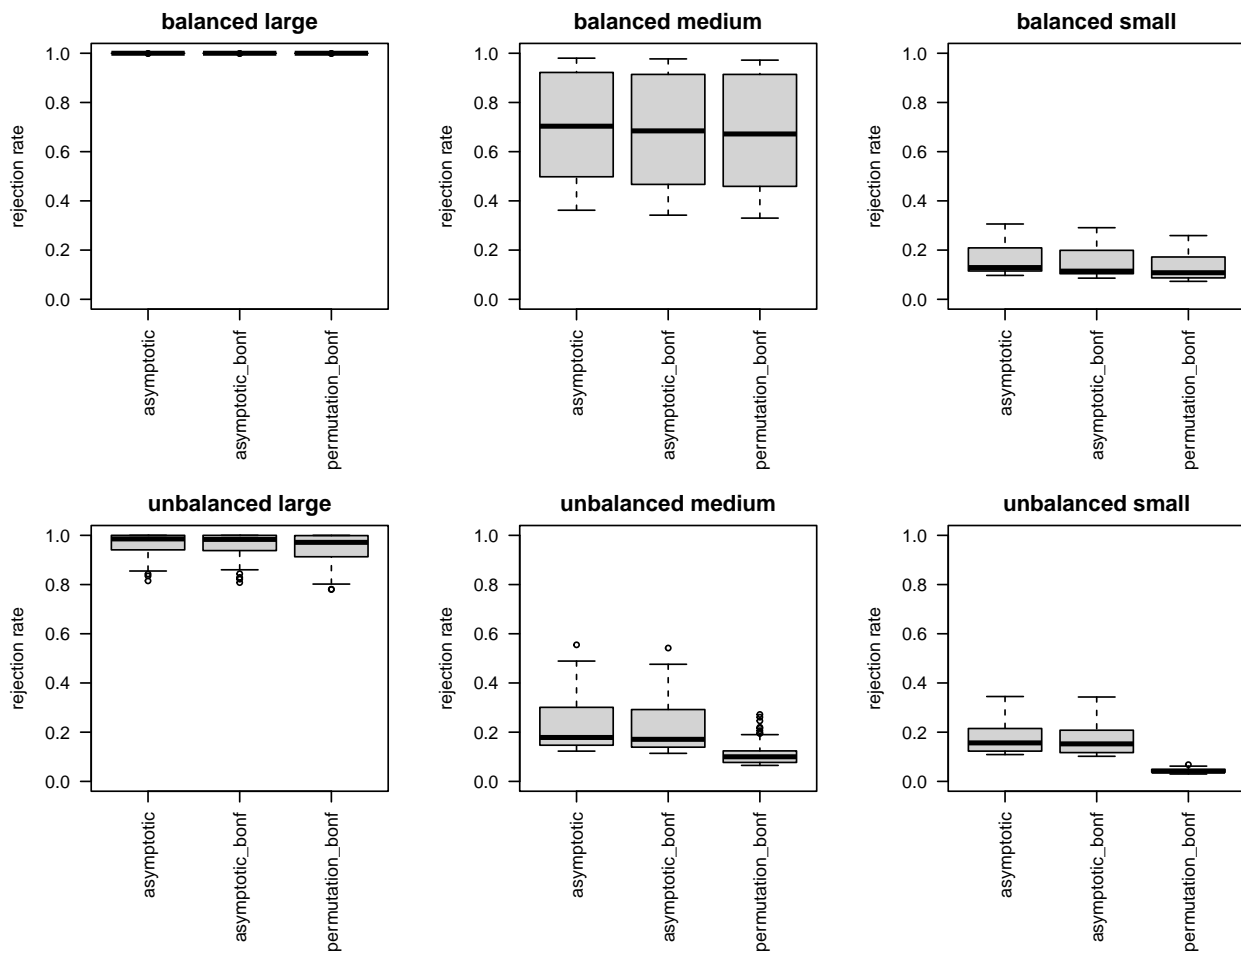

Figure S2: Empirical powers for the Dunnett-type contrast hypotheses across all scenarios under the alternative hypothesis.

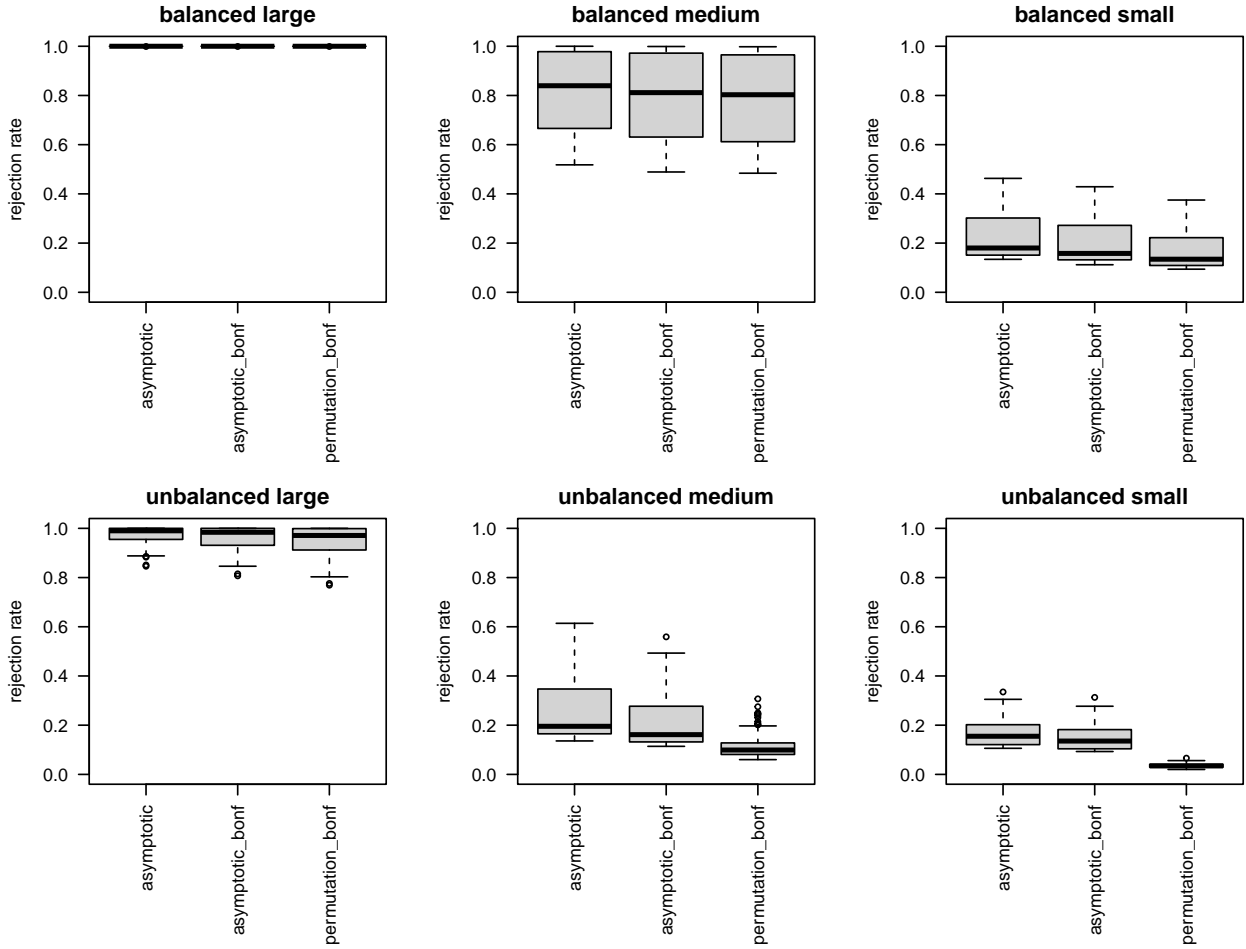

Figure S3: Empirical powers for the Tukey-type contrast hypotheses across all scenarios under the alternative hypothesis.

### B.3 Tables of Simulation Results

Tables S1–S36 contain the global rejection rates for all scenarios under the null and alternative hypothesis. For analyzing whether the false local hypotheses are rejected, Tables S37–S90 contain the rejection rates of all false hypotheses (under the alternative hypothesis). In detail, the following hypotheses are false under the alternative hypothesis:

- $\mathcal{H}_{0,1} = \mathcal{H}_{0,1}^A, \mathcal{H}_{0,2} = \mathcal{H}_{0,2}^A, \mathcal{H}_{0,3} = \mathcal{H}_{0,3}^A, \mathcal{H}_{0,4} = \mathcal{H}_{0,1}^B, \mathcal{H}_{0,5} = \mathcal{H}_{0,2}^B, \mathcal{H}_{0,6} = \mathcal{H}_{0,3}^B, \mathcal{H}_{0,7} = \mathcal{H}_{0,1}^{AB}, \mathcal{H}_{0,8} = \mathcal{H}_{0,2}^{AB}, \mathcal{H}_{0,9} = \mathcal{H}_{0,3}^{AB}$  for the 2-by-2 design,
- $\mathcal{H}_{0,7} : \mu_{11} = \mu_{41}, \mathcal{H}_{0,8} : \mu_{12} = \mu_{42}, \mathcal{H}_{0,9} : \mu_{13} = \mu_{43}$  for the Dunnett-type contrast matrix, and
- $\mathcal{H}_{0,7} : \mu_{11} = \mu_{41}, \mathcal{H}_{0,8} : \mu_{12} = \mu_{42}, \mathcal{H}_{0,9} : \mu_{13} = \mu_{43}, \mathcal{H}_{0,13} : \mu_{21} = \mu_{41}, \mathcal{H}_{0,14} : \mu_{22} = \mu_{42}, \mathcal{H}_{0,15} : \mu_{23} = \mu_{43}, \mathcal{H}_{0,16} : \mu_{31} = \mu_{41}, \mathcal{H}_{0,17} : \mu_{32} = \mu_{42}, \mathcal{H}_{0,18} : \mu_{33} = \mu_{43}$  for the Tukey-type contrast matrix.

Table S1: Rejection rates in percent for the 2-by-2 design with  $\delta = 0.0$  and balanced large sample sizes.

| Distribution          | Censoring distribution | asymptotic | asymptotic.bonf | permutation.bonf |
|-----------------------|------------------------|------------|-----------------|------------------|
| exp early continuous  | equal                  | <b>5.4</b> | <b>5.1</b>      | <b>4.9</b>       |
| exp early discrete    | equal                  | <b>6.1</b> | <b>5.7</b>      | <b>5.3</b>       |
| exp early continuous  | unequal, high          | <b>5.3</b> | <b>5.2</b>      | <b>5.3</b>       |
| exp early discrete    | unequal, high          | <b>5.7</b> | <b>5.2</b>      | <b>5.7</b>       |
| exp early continuous  | unequal, low           | <b>6.0</b> | <b>5.7</b>      | <b>5.9</b>       |
| exp early discrete    | unequal, low           | <b>6.1</b> | <b>5.8</b>      | <b>6.3</b>       |
| logn continuous       | equal                  | <b>4.7</b> | <b>4.5</b>      | <b>5.1</b>       |
| logn discrete         | equal                  | <b>4.8</b> | <b>4.6</b>      | <b>5.6</b>       |
| logn continuous       | unequal, high          | <b>4.3</b> | <b>4.2</b>      | <b>4.5</b>       |
| logn discrete         | unequal, high          | <b>4.1</b> | <b>4.0</b>      | <b>4.4</b>       |
| logn continuous       | unequal, low           | <b>4.5</b> | <b>4.4</b>      | <b>5.5</b>       |
| logn discrete         | unequal, low           | <b>4.7</b> | <b>4.7</b>      | <b>5.0</b>       |
| pwExp continuous      | equal                  | <b>5.8</b> | <b>5.5</b>      | <b>5.9</b>       |
| pwExp discrete        | equal                  | <b>5.7</b> | <b>5.6</b>      | <b>6.0</b>       |
| pwExp continuous      | unequal, high          | <b>6.0</b> | <b>5.9</b>      | <b>6.3</b>       |
| pwExp discrete        | unequal, high          | <b>5.3</b> | <b>5.2</b>      | <b>6.2</b>       |
| pwExp continuous      | unequal, low           | <b>5.7</b> | <b>5.4</b>      | <b>5.5</b>       |
| pwExp discrete        | unequal, low           | <b>5.9</b> | <b>5.5</b>      | <b>5.7</b>       |
| Weib prop continuous  | equal                  | <b>4.9</b> | <b>4.6</b>      | <b>5.5</b>       |
| Weib prop discrete    | equal                  | <b>5.1</b> | <b>4.7</b>      | <b>4.7</b>       |
| Weib prop continuous  | unequal, high          | <b>5.3</b> | <b>5.2</b>      | <b>5.3</b>       |
| Weib prop discrete    | unequal, high          | <b>5.7</b> | <b>5.5</b>      | <b>5.8</b>       |
| Weib prop continuous  | unequal, low           | <b>4.4</b> | <b>4.4</b>      | <b>5.1</b>       |
| Weib prop discrete    | unequal, low           | <b>5.1</b> | <b>4.9</b>      | <b>5.2</b>       |
| Weib scale continuous | equal                  | <b>4.3</b> | <b>4.1</b>      | <b>4.9</b>       |
| Weib scale discrete   | equal                  | <b>4.7</b> | <b>4.6</b>      | <b>5.0</b>       |
| Weib scale continuous | unequal, high          | <b>5.6</b> | <b>5.6</b>      | <b>5.5</b>       |
| Weib scale discrete   | unequal, high          | <b>6.1</b> | <b>5.8</b>      | <b>5.8</b>       |
| Weib scale continuous | unequal, low           | <b>4.6</b> | <b>4.5</b>      | <b>4.8</b>       |
| Weib scale discrete   | unequal, low           | <b>4.6</b> | <b>4.5</b>      | <b>4.7</b>       |
| Weib shape continuous | equal                  | <b>4.5</b> | <b>4.1</b>      | <b>4.4</b>       |
| Weib shape discrete   | equal                  | <b>4.9</b> | <b>4.7</b>      | <b>4.3</b>       |
| Weib shape continuous | unequal, high          | <b>6.1</b> | <b>5.6</b>      | <b>6.2</b>       |
| Weib shape discrete   | unequal, high          | <b>5.9</b> | <b>5.7</b>      | <b>5.7</b>       |
| Weib shape continuous | unequal, low           | <b>5.0</b> | <b>4.4</b>      | <b>4.8</b>       |
| Weib shape discrete   | unequal, low           | <b>5.1</b> | <b>4.9</b>      | <b>4.6</b>       |

All values in the binomial interval  $[3.7, 6.4]$  are printed in bold type.



Table S2: Rejection rates in percent for the 2-by-2 design with  $\delta = 0.0$  and balanced medium sample sizes.

| Distribution          | Censoring distribution | asymptotic | asymptotic.bonf | permutation.bonf |
|-----------------------|------------------------|------------|-----------------|------------------|
| exp early continuous  | equal                  | <b>4.9</b> | <b>4.8</b>      | <b>4.8</b>       |
| exp early discrete    | equal                  | <b>5.0</b> | <b>4.7</b>      | <b>4.8</b>       |
| exp early continuous  | unequal, high          | <b>5.2</b> | <b>5.1</b>      | <b>5.5</b>       |
| exp early discrete    | unequal, high          | <b>5.2</b> | <b>5.0</b>      | <b>4.8</b>       |
| exp early continuous  | unequal, low           | <b>4.7</b> | <b>4.6</b>      | <b>5.1</b>       |
| exp early discrete    | unequal, low           | <b>5.3</b> | <b>5.0</b>      | <b>5.4</b>       |
| logn continuous       | equal                  | <b>5.5</b> | <b>5.4</b>      | <b>5.8</b>       |
| logn discrete         | equal                  | <b>4.8</b> | <b>4.8</b>      | <b>5.0</b>       |
| logn continuous       | unequal, high          | <b>4.1</b> | <b>3.8</b>      | <b>4.9</b>       |
| logn discrete         | unequal, high          | <b>5.0</b> | <b>4.9</b>      | <b>5.4</b>       |
| logn continuous       | unequal, low           | <b>4.4</b> | <b>4.3</b>      | <b>4.3</b>       |
| logn discrete         | unequal, low           | <b>4.0</b> | <b>3.7</b>      | <b>4.3</b>       |
| pwExp continuous      | equal                  | <b>5.3</b> | <b>4.8</b>      | <b>4.9</b>       |
| pwExp discrete        | equal                  | <b>5.0</b> | <b>5.0</b>      | <b>4.4</b>       |
| pwExp continuous      | unequal, high          | <b>4.3</b> | <b>4.3</b>      | <b>4.7</b>       |
| pwExp discrete        | unequal, high          | <b>4.4</b> | <b>4.2</b>      | <b>4.7</b>       |
| pwExp continuous      | unequal, low           | <b>5.3</b> | <b>4.9</b>      | <b>5.4</b>       |
| pwExp discrete        | unequal, low           | <b>5.0</b> | <b>4.7</b>      | <b>4.6</b>       |
| Weib prop continuous  | equal                  | <b>5.0</b> | <b>5.0</b>      | <b>5.1</b>       |
| Weib prop discrete    | equal                  | <b>5.5</b> | <b>4.9</b>      | <b>5.3</b>       |
| Weib prop continuous  | unequal, high          | <b>4.6</b> | <b>4.3</b>      | <b>5.0</b>       |
| Weib prop discrete    | unequal, high          | <b>5.2</b> | <b>5.2</b>      | <b>4.6</b>       |
| Weib prop continuous  | unequal, low           | <b>5.4</b> | <b>5.0</b>      | <b>5.6</b>       |
| Weib prop discrete    | unequal, low           | <b>5.1</b> | <b>4.9</b>      | <b>5.1</b>       |
| Weib scale continuous | equal                  | <b>6.0</b> | <b>5.5</b>      | <b>5.5</b>       |
| Weib scale discrete   | equal                  | <b>5.1</b> | <b>4.9</b>      | <b>5.1</b>       |
| Weib scale continuous | unequal, high          | <b>5.5</b> | <b>5.3</b>      | <b>5.0</b>       |
| Weib scale discrete   | unequal, high          | <b>5.7</b> | <b>5.6</b>      | <b>5.8</b>       |
| Weib scale continuous | unequal, low           | <b>5.1</b> | <b>5.1</b>      | <b>5.6</b>       |
| Weib scale discrete   | unequal, low           | <b>4.9</b> | <b>4.8</b>      | <b>5.0</b>       |
| Weib shape continuous | equal                  | <b>5.8</b> | <b>5.8</b>      | <b>5.6</b>       |
| Weib shape discrete   | equal                  | <b>5.5</b> | <b>5.3</b>      | <b>5.3</b>       |
| Weib shape continuous | unequal, high          | <b>5.5</b> | <b>5.4</b>      | <b>5.4</b>       |
| Weib shape discrete   | unequal, high          | <b>5.1</b> | <b>4.9</b>      | <b>4.9</b>       |
| Weib shape continuous | unequal, low           | <b>5.2</b> | <b>5.1</b>      | <b>5.5</b>       |
| Weib shape discrete   | unequal, low           | <b>4.9</b> | <b>4.7</b>      | <b>5.0</b>       |

All values in the binomial interval  $[3.7, 6.4]$  are printed in bold type.

Table S3: Rejection rates in percent for the 2-by-2 design with  $\delta = 0.0$  and balanced small sample sizes.

| Distribution          | Censoring distribution | asymptotic | asymptotic_bonf | permutation_bonf |
|-----------------------|------------------------|------------|-----------------|------------------|
| exp early continuous  | equal                  | <b>5.4</b> | <b>5.1</b>      | <b>4.8</b>       |
| exp early discrete    | equal                  | <b>5.5</b> | <b>5.3</b>      | <b>4.6</b>       |
| exp early continuous  | unequal, high          | <b>5.4</b> | <b>5.3</b>      | <b>4.2</b>       |
| exp early discrete    | unequal, high          | <b>6.0</b> | <b>6.0</b>      | <b>4.7</b>       |
| exp early continuous  | unequal, low           | <b>6.0</b> | <b>5.4</b>      | <b>5.2</b>       |
| exp early discrete    | unequal, low           | <b>6.1</b> | <b>6.0</b>      | <b>4.9</b>       |
| logn continuous       | equal                  | <b>5.9</b> | <b>5.5</b>      | <b>5.8</b>       |
| logn discrete         | equal                  | <b>6.4</b> | <b>6.1</b>      | <b>6.2</b>       |
| logn continuous       | unequal, high          | <b>6.2</b> | <b>6.0</b>      | <b>4.8</b>       |
| logn discrete         | unequal, high          | <b>5.9</b> | <b>5.7</b>      | <b>4.7</b>       |
| logn continuous       | unequal, low           | <b>6.0</b> | <b>5.9</b>      | <b>5.5</b>       |
| logn discrete         | unequal, low           | <b>6.0</b> | <b>5.9</b>      | <b>5.5</b>       |
| pwExp continuous      | equal                  | <b>5.7</b> | <b>5.4</b>      | <b>4.3</b>       |
| pwExp discrete        | equal                  | <b>5.2</b> | <b>5.0</b>      | <b>4.2</b>       |
| pwExp continuous      | unequal, high          | <b>5.1</b> | <b>4.8</b>      | <b>4.4</b>       |
| pwExp discrete        | unequal, high          | <b>4.9</b> | <b>4.5</b>      | <b>4.0</b>       |
| pwExp continuous      | unequal, low           | <b>5.4</b> | <b>4.9</b>      | <b>4.5</b>       |
| pwExp discrete        | unequal, low           | <b>5.6</b> | <b>5.5</b>      | <b>4.5</b>       |
| Weib prop continuous  | equal                  | <b>6.1</b> | <b>5.9</b>      | <b>5.7</b>       |
| Weib prop discrete    | equal                  | <b>5.8</b> | <b>5.6</b>      | <b>4.7</b>       |
| Weib prop continuous  | unequal, high          | <b>6.3</b> | <b>6.0</b>      | <b>5.6</b>       |
| Weib prop discrete    | unequal, high          | <b>6.5</b> | <b>6.1</b>      | <b>4.7</b>       |
| Weib prop continuous  | unequal, low           | <b>7.2</b> | <b>6.8</b>      | <b>5.9</b>       |
| Weib prop discrete    | unequal, low           | <b>5.9</b> | <b>5.7</b>      | <b>5.8</b>       |
| Weib scale continuous | equal                  | <b>6.9</b> | <b>6.9</b>      | <b>6.5</b>       |
| Weib scale discrete   | equal                  | <b>5.5</b> | <b>5.4</b>      | <b>5.7</b>       |
| Weib scale continuous | unequal, high          | <b>7.1</b> | <b>6.4</b>      | <b>5.3</b>       |
| Weib scale discrete   | unequal, high          | <b>6.2</b> | <b>6.2</b>      | <b>5.3</b>       |
| Weib scale continuous | unequal, low           | <b>6.4</b> | <b>6.3</b>      | <b>6.6</b>       |
| Weib scale discrete   | unequal, low           | <b>6.2</b> | <b>5.9</b>      | <b>6.0</b>       |
| Weib shape continuous | equal                  | <b>6.5</b> | <b>6.3</b>      | <b>6.4</b>       |
| Weib shape discrete   | equal                  | <b>6.3</b> | <b>6.0</b>      | <b>5.7</b>       |
| Weib shape continuous | unequal, high          | <b>6.4</b> | <b>6.4</b>      | <b>6.0</b>       |
| Weib shape discrete   | unequal, high          | <b>6.9</b> | <b>6.8</b>      | <b>5.4</b>       |
| Weib shape continuous | unequal, low           | <b>6.5</b> | <b>6.4</b>      | <b>6.5</b>       |
| Weib shape discrete   | unequal, low           | <b>6.2</b> | <b>6.2</b>      | <b>5.6</b>       |

All values in the binomial interval  $[3.7, 6.4]$  are printed in bold type.

Table S4: Rejection rates in percent for the 2-by-2 design with  $\delta = 0.0$  and unbalanced large sample sizes.

| Distribution          | Censoring distribution | asymptotic | asymptotic.bonf | permutation.bonf |
|-----------------------|------------------------|------------|-----------------|------------------|
| exp early continuous  | equal                  | <b>4.3</b> | <b>4.0</b>      | <b>4.2</b>       |
| exp early discrete    | equal                  | <b>5.1</b> | <b>4.8</b>      | <b>4.6</b>       |
| exp early continuous  | unequal, high          | <b>5.4</b> | <b>4.6</b>      | <b>4.7</b>       |
| exp early discrete    | unequal, high          | <b>5.6</b> | <b>5.0</b>      | <b>4.9</b>       |
| exp early continuous  | unequal, low           | <b>5.3</b> | <b>4.9</b>      | <b>5.3</b>       |
| exp early discrete    | unequal, low           | <b>5.3</b> | <b>5.0</b>      | <b>5.5</b>       |
| logn continuous       | equal                  | <b>4.9</b> | <b>4.3</b>      | <b>4.3</b>       |
| logn discrete         | equal                  | <b>5.0</b> | <b>4.8</b>      | <b>4.6</b>       |
| logn continuous       | unequal, high          | <b>5.1</b> | <b>4.5</b>      | <b>5.0</b>       |
| logn discrete         | unequal, high          | <b>4.9</b> | <b>4.4</b>      | <b>5.5</b>       |
| logn continuous       | unequal, low           | <b>5.1</b> | <b>4.8</b>      | <b>4.6</b>       |
| logn discrete         | unequal, low           | <b>5.0</b> | <b>4.8</b>      | <b>4.5</b>       |
| pwExp continuous      | equal                  | <b>5.7</b> | <b>5.1</b>      | <b>4.7</b>       |
| pwExp discrete        | equal                  | <b>5.5</b> | <b>4.8</b>      | <b>4.7</b>       |
| pwExp continuous      | unequal, high          | <b>3.8</b> | <b>3.7</b>      | <b>4.1</b>       |
| pwExp discrete        | unequal, high          | <b>4.1</b> | <b>3.6</b>      | <b>4.4</b>       |
| pwExp continuous      | unequal, low           | <b>5.6</b> | <b>4.8</b>      | <b>4.5</b>       |
| pwExp discrete        | unequal, low           | <b>5.5</b> | <b>4.9</b>      | <b>4.5</b>       |
| Weib prop continuous  | equal                  | <b>5.2</b> | <b>4.8</b>      | <b>4.7</b>       |
| Weib prop discrete    | equal                  | <b>5.5</b> | <b>5.1</b>      | <b>4.7</b>       |
| Weib prop continuous  | unequal, high          | <b>4.8</b> | <b>4.5</b>      | <b>4.6</b>       |
| Weib prop discrete    | unequal, high          | <b>6.1</b> | <b>5.8</b>      | <b>4.6</b>       |
| Weib prop continuous  | unequal, low           | <b>5.0</b> | <b>4.5</b>      | <b>4.4</b>       |
| Weib prop discrete    | unequal, low           | <b>4.6</b> | <b>4.6</b>      | <b>4.7</b>       |
| Weib scale continuous | equal                  | <b>4.8</b> | <b>4.7</b>      | <b>4.4</b>       |
| Weib scale discrete   | equal                  | <b>4.8</b> | <b>4.3</b>      | <b>4.7</b>       |
| Weib scale continuous | unequal, high          | <b>5.0</b> | <b>4.6</b>      | <b>4.9</b>       |
| Weib scale discrete   | unequal, high          | <b>4.6</b> | <b>4.3</b>      | <b>3.7</b>       |
| Weib scale continuous | unequal, low           | <b>4.3</b> | <b>4.1</b>      | <b>4.0</b>       |
| Weib scale discrete   | unequal, low           | <b>4.3</b> | <b>4.2</b>      | <b>4.1</b>       |
| Weib shape continuous | equal                  | <b>5.1</b> | <b>4.4</b>      | <b>4.4</b>       |
| Weib shape discrete   | equal                  | <b>5.0</b> | <b>4.4</b>      | <b>4.3</b>       |
| Weib shape continuous | unequal, high          | <b>5.3</b> | <b>4.3</b>      | <b>4.7</b>       |
| Weib shape discrete   | unequal, high          | <b>4.9</b> | <b>4.6</b>      | <b>4.0</b>       |
| Weib shape continuous | unequal, low           | <b>4.4</b> | <b>4.2</b>      | <b>4.2</b>       |
| Weib shape discrete   | unequal, low           | <b>4.2</b> | <b>4.1</b>      | <b>4.1</b>       |

All values in the binomial interval  $[3.7, 6.4]$  are printed in bold type.

Table S5: Rejection rates in percent for the 2-by-2 design with  $\delta = 0.0$  and unbalanced medium sample sizes.

| Distribution          | Censoring distribution | asymptotic | asymptotic.bonf | permutation.bonf |
|-----------------------|------------------------|------------|-----------------|------------------|
| exp early continuous  | equal                  | 6.6        | <b>5.9</b>      | <b>5.4</b>       |
| exp early discrete    | equal                  | <b>6.2</b> | <b>6.0</b>      | <b>5.4</b>       |
| exp early continuous  | unequal, high          | <b>5.5</b> | <b>5.4</b>      | <b>4.7</b>       |
| exp early discrete    | unequal, high          | <b>6.0</b> | <b>5.6</b>      | <b>4.5</b>       |
| exp early continuous  | unequal, low           | <b>5.9</b> | <b>5.3</b>      | <b>4.4</b>       |
| exp early discrete    | unequal, low           | <b>5.7</b> | <b>5.5</b>      | <b>5.0</b>       |
| logn continuous       | equal                  | 8.1        | 7.7             | <b>5.8</b>       |
| logn discrete         | equal                  | 7.3        | 7.0             | <b>5.7</b>       |
| logn continuous       | unequal, high          | 7.8        | 7.6             | <b>5.4</b>       |
| logn discrete         | unequal, high          | 7.4        | 6.6             | <b>4.8</b>       |
| logn continuous       | unequal, low           | 6.9        | 6.5             | <b>4.8</b>       |
| logn discrete         | unequal, low           | <b>6.3</b> | <b>6.0</b>      | <b>4.0</b>       |
| pwExp continuous      | equal                  | <b>5.3</b> | <b>4.9</b>      | <b>4.5</b>       |
| pwExp discrete        | equal                  | <b>5.4</b> | <b>5.0</b>      | <b>4.6</b>       |
| pwExp continuous      | unequal, high          | <b>5.4</b> | <b>5.2</b>      | <b>4.4</b>       |
| pwExp discrete        | unequal, high          | <b>5.0</b> | <b>4.7</b>      | <b>4.0</b>       |
| pwExp continuous      | unequal, low           | <b>5.7</b> | <b>4.8</b>      | <b>4.6</b>       |
| pwExp discrete        | unequal, low           | <b>6.0</b> | <b>5.5</b>      | <b>4.9</b>       |
| Weib prop continuous  | equal                  | <b>5.3</b> | <b>4.8</b>      | <b>4.3</b>       |
| Weib prop discrete    | equal                  | <b>5.5</b> | <b>5.5</b>      | <b>4.5</b>       |
| Weib prop continuous  | unequal, high          | 7.5        | 6.7             | <b>5.0</b>       |
| Weib prop discrete    | unequal, high          | 7.2        | 6.5             | <b>4.7</b>       |
| Weib prop continuous  | unequal, low           | <b>5.9</b> | <b>5.4</b>      | <b>3.8</b>       |
| Weib prop discrete    | unequal, low           | <b>6.2</b> | <b>6.1</b>      | <b>4.1</b>       |
| Weib scale continuous | equal                  | 7.0        | <b>6.3</b>      | <b>5.1</b>       |
| Weib scale discrete   | equal                  | 7.5        | 7.3             | <b>5.9</b>       |
| Weib scale continuous | unequal, high          | 8.4        | 8.1             | <b>5.5</b>       |
| Weib scale discrete   | unequal, high          | 8.2        | 7.7             | <b>5.3</b>       |
| Weib scale continuous | unequal, low           | 6.7        | <b>6.4</b>      | <b>5.0</b>       |
| Weib scale discrete   | unequal, low           | 7.5        | 7.0             | <b>5.8</b>       |
| Weib shape continuous | equal                  | 7.7        | 6.7             | <b>5.5</b>       |
| Weib shape discrete   | equal                  | 8.4        | 7.1             | <b>6.0</b>       |
| Weib shape continuous | unequal, high          | 7.8        | 7.3             | <b>4.2</b>       |
| Weib shape discrete   | unequal, high          | 7.9        | 7.6             | <b>5.5</b>       |
| Weib shape continuous | unequal, low           | 7.6        | 6.9             | <b>5.3</b>       |
| Weib shape discrete   | unequal, low           | 7.8        | 7.6             | <b>5.9</b>       |

All values in the binomial interval  $[3.7, 6.4]$  are printed in bold type.

Table S6: Rejection rates in percent for the 2-by-2 design with  $\delta = 0.0$  and unbalanced small sample sizes.

| Distribution          | Censoring distribution | asymptotic | asymptotic.bonf | permutation.bonf |
|-----------------------|------------------------|------------|-----------------|------------------|
| exp early continuous  | equal                  | 12.4       | 11.0            | <b>5.5</b>       |
| exp early discrete    | equal                  | 12.7       | 12.2            | <b>5.7</b>       |
| exp early continuous  | unequal, high          | 12.4       | 11.2            | <b>3.8</b>       |
| exp early discrete    | unequal, high          | 10.9       | 10.2            | <b>3.9</b>       |
| exp early continuous  | unequal, low           | 11.1       | 10.5            | <b>4.4</b>       |
| exp early discrete    | unequal, low           | 11.5       | 10.8            | <b>4.3</b>       |
| logn continuous       | equal                  | 15.1       | 14.3            | <b>6.1</b>       |
| logn discrete         | equal                  | 14.9       | 14.3            | <b>5.5</b>       |
| logn continuous       | unequal, high          | 17.2       | 16.0            | <b>4.9</b>       |
| logn discrete         | unequal, high          | 16.6       | 15.8            | <b>5.8</b>       |
| logn continuous       | unequal, low           | 11.7       | 11.5            | <b>4.3</b>       |
| logn discrete         | unequal, low           | 11.7       | 11.4            | <b>3.9</b>       |
| pwExp continuous      | equal                  | 10.9       | 10.0            | <b>4.7</b>       |
| pwExp discrete        | equal                  | 11.5       | 10.8            | <b>5.4</b>       |
| pwExp continuous      | unequal, high          | 12.2       | 11.4            | <b>3.5</b>       |
| pwExp discrete        | unequal, high          | 12.2       | 11.8            | <b>4.4</b>       |
| pwExp continuous      | unequal, low           | 10.4       | 9.8             | <b>5.0</b>       |
| pwExp discrete        | unequal, low           | 10.7       | 9.9             | <b>4.7</b>       |
| Weib prop continuous  | equal                  | 13.5       | 11.9            | <b>5.1</b>       |
| Weib prop discrete    | equal                  | 13.8       | 13.1            | <b>4.9</b>       |
| Weib prop continuous  | unequal, high          | 17.8       | 16.8            | <b>5.1</b>       |
| Weib prop discrete    | unequal, high          | 16.8       | 15.7            | <b>4.8</b>       |
| Weib prop continuous  | unequal, low           | 10.1       | 9.1             | 2.6              |
| Weib prop discrete    | unequal, low           | 10.5       | 9.7             | 3.4              |
| Weib scale continuous | equal                  | 19.8       | 18.6            | 8.0              |
| Weib scale discrete   | equal                  | 20.2       | 18.9            | 7.0              |
| Weib scale continuous | unequal, high          | 19.2       | 17.8            | <b>6.4</b>       |
| Weib scale discrete   | unequal, high          | 19.6       | 18.0            | <b>6.1</b>       |
| Weib scale continuous | unequal, low           | 14.8       | 14.3            | <b>5.5</b>       |
| Weib scale discrete   | unequal, low           | 14.6       | 14.0            | <b>5.6</b>       |
| Weib shape continuous | equal                  | 23.3       | 21.7            | 10.0             |
| Weib shape discrete   | equal                  | 22.8       | 21.1            | 9.2              |
| Weib shape continuous | unequal, high          | 21.6       | 19.8            | 6.7              |
| Weib shape discrete   | unequal, high          | 21.3       | 19.4            | 6.5              |
| Weib shape continuous | unequal, low           | 19.0       | 18.1            | 7.5              |
| Weib shape discrete   | unequal, low           | 18.8       | 17.6            | 7.1              |

All values in the binomial interval  $[3.7, 6.4]$  are printed in bold type.

Table S7: Rejection rates in percent for the Dunnett-type contrast matrix with  $\delta = 0.0$  and balanced large sample sizes.

| Distribution          | Censoring distribution | asymptotic | asymptotic_bonf | permutation_bonf |
|-----------------------|------------------------|------------|-----------------|------------------|
| exp early continuous  | equal                  | <b>5.7</b> | <b>5.1</b>      | <b>5.1</b>       |
| exp early discrete    | equal                  | <b>5.3</b> | <b>4.8</b>      | <b>5.0</b>       |
| exp early continuous  | unequal, high          | <b>5.5</b> | <b>5.1</b>      | <b>5.1</b>       |
| exp early discrete    | unequal, high          | <b>5.8</b> | <b>5.4</b>      | <b>5.3</b>       |
| exp early continuous  | unequal, low           | <b>5.5</b> | <b>5.0</b>      | <b>5.5</b>       |
| exp early discrete    | unequal, low           | <b>5.6</b> | <b>4.7</b>      | <b>5.0</b>       |
| logn continuous       | equal                  | <b>4.4</b> | <b>4.1</b>      | <b>3.9</b>       |
| logn discrete         | equal                  | <b>5.1</b> | <b>4.5</b>      | <b>4.3</b>       |
| logn continuous       | unequal, high          | <b>4.9</b> | <b>4.5</b>      | <b>4.6</b>       |
| logn discrete         | unequal, high          | <b>4.8</b> | <b>4.4</b>      | <b>4.3</b>       |
| logn continuous       | unequal, low           | <b>4.6</b> | <b>4.0</b>      | <b>4.8</b>       |
| logn discrete         | unequal, low           | <b>4.9</b> | <b>4.3</b>      | <b>4.9</b>       |
| pwExp continuous      | equal                  | <b>5.5</b> | <b>5.0</b>      | <b>5.6</b>       |
| pwExp discrete        | equal                  | <b>5.3</b> | <b>4.8</b>      | <b>5.2</b>       |
| pwExp continuous      | unequal, high          | <b>5.1</b> | <b>4.6</b>      | <b>4.6</b>       |
| pwExp discrete        | unequal, high          | <b>4.9</b> | <b>4.5</b>      | <b>5.0</b>       |
| pwExp continuous      | unequal, low           | <b>4.7</b> | <b>4.4</b>      | <b>5.0</b>       |
| pwExp discrete        | unequal, low           | <b>5.2</b> | <b>4.8</b>      | <b>4.9</b>       |
| Weib prop continuous  | equal                  | <b>5.1</b> | <b>4.6</b>      | <b>4.9</b>       |
| Weib prop discrete    | equal                  | <b>4.3</b> | <b>4.1</b>      | <b>4.8</b>       |
| Weib prop continuous  | unequal, high          | <b>5.3</b> | <b>5.2</b>      | <b>5.3</b>       |
| Weib prop discrete    | unequal, high          | <b>5.8</b> | <b>5.4</b>      | <b>5.9</b>       |
| Weib prop continuous  | unequal, low           | <b>5.2</b> | <b>4.9</b>      | <b>4.3</b>       |
| Weib prop discrete    | unequal, low           | <b>5.3</b> | <b>4.7</b>      | <b>4.8</b>       |
| Weib scale continuous | equal                  | <b>4.9</b> | <b>4.6</b>      | <b>4.7</b>       |
| Weib scale discrete   | equal                  | <b>4.4</b> | <b>3.8</b>      | <b>4.2</b>       |
| Weib scale continuous | unequal, high          | <b>4.8</b> | <b>4.7</b>      | <b>4.6</b>       |
| Weib scale discrete   | unequal, high          | <b>5.6</b> | <b>5.4</b>      | <b>5.3</b>       |
| Weib scale continuous | unequal, low           | <b>5.0</b> | <b>4.8</b>      | <b>4.5</b>       |
| Weib scale discrete   | unequal, low           | <b>5.2</b> | <b>4.5</b>      | <b>4.7</b>       |
| Weib shape continuous | equal                  | <b>5.1</b> | <b>4.8</b>      | <b>4.7</b>       |
| Weib shape discrete   | equal                  | <b>4.5</b> | <b>3.8</b>      | <b>4.5</b>       |
| Weib shape continuous | unequal, high          | <b>5.1</b> | <b>4.9</b>      | <b>5.2</b>       |
| Weib shape discrete   | unequal, high          | <b>5.3</b> | <b>4.9</b>      | <b>5.2</b>       |
| Weib shape continuous | unequal, low           | <b>5.2</b> | <b>5.0</b>      | <b>5.1</b>       |
| Weib shape discrete   | unequal, low           | <b>5.3</b> | <b>4.6</b>      | <b>5.0</b>       |

All values in the binomial interval  $[3.7, 6.4]$  are printed in bold type.

Table S8: Rejection rates in percent for the Dunnett-type contrast matrix with  $\delta = 0.0$  and balanced medium sample sizes.

| Distribution          | Censoring distribution | asymptotic | asymptotic.bonf | permutation.bonf |
|-----------------------|------------------------|------------|-----------------|------------------|
| exp early continuous  | equal                  | <b>5.6</b> | <b>4.7</b>      | <b>4.6</b>       |
| exp early discrete    | equal                  | <b>5.3</b> | <b>4.9</b>      | <b>5.3</b>       |
| exp early continuous  | unequal, high          | 6.6        | <b>5.6</b>      | <b>5.4</b>       |
| exp early discrete    | unequal, high          | <b>5.1</b> | <b>4.7</b>      | <b>5.5</b>       |
| exp early continuous  | unequal, low           | <b>5.8</b> | <b>5.2</b>      | <b>6.2</b>       |
| exp early discrete    | unequal, low           | <b>6.1</b> | <b>5.3</b>      | <b>6.2</b>       |
| logn continuous       | equal                  | <b>4.5</b> | <b>3.9</b>      | <b>4.0</b>       |
| logn discrete         | equal                  | <b>5.4</b> | <b>4.8</b>      | <b>5.2</b>       |
| logn continuous       | unequal, high          | <b>4.5</b> | <b>4.1</b>      | <b>4.0</b>       |
| logn discrete         | unequal, high          | <b>5.1</b> | <b>4.8</b>      | <b>4.7</b>       |
| logn continuous       | unequal, low           | <b>4.9</b> | <b>4.2</b>      | <b>4.5</b>       |
| logn discrete         | unequal, low           | <b>5.5</b> | <b>5.1</b>      | <b>5.3</b>       |
| pwExp continuous      | equal                  | <b>6.1</b> | <b>5.3</b>      | <b>5.6</b>       |
| pwExp discrete        | equal                  | 6.5        | <b>5.6</b>      | <b>5.7</b>       |
| pwExp continuous      | unequal, high          | <b>5.5</b> | <b>4.6</b>      | <b>5.1</b>       |
| pwExp discrete        | unequal, high          | <b>6.4</b> | <b>5.4</b>      | <b>4.9</b>       |
| pwExp continuous      | unequal, low           | 7.4        | <b>6.1</b>      | <b>5.9</b>       |
| pwExp discrete        | unequal, low           | 6.9        | <b>6.4</b>      | <b>6.2</b>       |
| Weib prop continuous  | equal                  | <b>5.0</b> | <b>4.4</b>      | <b>5.1</b>       |
| Weib prop discrete    | equal                  | <b>4.8</b> | <b>4.4</b>      | <b>5.5</b>       |
| Weib prop continuous  | unequal, high          | <b>4.8</b> | <b>4.0</b>      | <b>4.2</b>       |
| Weib prop discrete    | unequal, high          | <b>5.0</b> | <b>4.2</b>      | <b>3.9</b>       |
| Weib prop continuous  | unequal, low           | <b>5.1</b> | <b>4.6</b>      | <b>5.0</b>       |
| Weib prop discrete    | unequal, low           | <b>4.8</b> | <b>4.0</b>      | <b>4.7</b>       |
| Weib scale continuous | equal                  | <b>5.3</b> | <b>4.7</b>      | <b>5.0</b>       |
| Weib scale discrete   | equal                  | <b>4.8</b> | <b>4.3</b>      | <b>5.1</b>       |
| Weib scale continuous | unequal, high          | <b>5.0</b> | <b>4.4</b>      | <b>4.4</b>       |
| Weib scale discrete   | unequal, high          | <b>5.6</b> | <b>5.0</b>      | <b>4.8</b>       |
| Weib scale continuous | unequal, low           | <b>5.5</b> | <b>4.8</b>      | <b>4.8</b>       |
| Weib scale discrete   | unequal, low           | <b>4.7</b> | <b>4.3</b>      | <b>5.3</b>       |
| Weib shape continuous | equal                  | <b>5.4</b> | <b>4.7</b>      | <b>5.1</b>       |
| Weib shape discrete   | equal                  | <b>4.6</b> | <b>4.1</b>      | <b>5.1</b>       |
| Weib shape continuous | unequal, high          | <b>5.1</b> | <b>4.6</b>      | <b>5.2</b>       |
| Weib shape discrete   | unequal, high          | <b>5.2</b> | <b>4.9</b>      | <b>5.0</b>       |
| Weib shape continuous | unequal, low           | <b>5.5</b> | <b>4.9</b>      | <b>5.2</b>       |
| Weib shape discrete   | unequal, low           | <b>4.6</b> | <b>4.4</b>      | <b>4.8</b>       |

All values in the binomial interval  $[3.7, 6.4]$  are printed in bold type.

Table S9: Rejection rates in percent for the Dunnett-type contrast matrix with  $\delta = 0.0$  and balanced small sample sizes.

| Distribution          | Censoring distribution | asymptotic | asymptotic_bonf | permutation_bonf |
|-----------------------|------------------------|------------|-----------------|------------------|
| exp early continuous  | equal                  | <b>5.6</b> | <b>5.2</b>      | <b>4.7</b>       |
| exp early discrete    | equal                  | <b>5.5</b> | <b>5.1</b>      | <b>4.8</b>       |
| exp early continuous  | unequal, high          | <b>6.4</b> | <b>6.2</b>      | <b>4.7</b>       |
| exp early discrete    | unequal, high          | 7.0        | <b>6.2</b>      | <b>4.9</b>       |
| exp early continuous  | unequal, low           | <b>5.4</b> | <b>4.6</b>      | <b>4.2</b>       |
| exp early discrete    | unequal, low           | <b>5.1</b> | <b>4.5</b>      | <b>4.0</b>       |
| logn continuous       | equal                  | <b>5.5</b> | <b>4.8</b>      | <b>4.0</b>       |
| logn discrete         | equal                  | <b>4.9</b> | <b>4.3</b>      | 3.5              |
| logn continuous       | unequal, high          | 7.0        | 6.6             | <b>5.7</b>       |
| logn discrete         | unequal, high          | 7.3        | 6.7             | <b>6.1</b>       |
| logn continuous       | unequal, low           | <b>5.4</b> | <b>4.5</b>      | <b>4.1</b>       |
| logn discrete         | unequal, low           | <b>4.5</b> | <b>4.0</b>      | <b>3.7</b>       |
| pwExp continuous      | equal                  | 6.6        | <b>5.5</b>      | <b>4.9</b>       |
| pwExp discrete        | equal                  | <b>6.2</b> | <b>5.2</b>      | <b>4.8</b>       |
| pwExp continuous      | unequal, high          | <b>6.4</b> | <b>5.2</b>      | <b>3.9</b>       |
| pwExp discrete        | unequal, high          | <b>6.4</b> | <b>5.4</b>      | <b>4.1</b>       |
| pwExp continuous      | unequal, low           | 6.7        | <b>5.8</b>      | <b>5.4</b>       |
| pwExp discrete        | unequal, low           | <b>6.3</b> | <b>5.6</b>      | <b>4.7</b>       |
| Weib prop continuous  | equal                  | 7.3        | 6.6             | 6.5              |
| Weib prop discrete    | equal                  | 6.7        | <b>5.7</b>      | <b>5.2</b>       |
| Weib prop continuous  | unequal, high          | 6.6        | <b>5.9</b>      | <b>4.6</b>       |
| Weib prop discrete    | unequal, high          | <b>6.1</b> | <b>5.7</b>      | <b>5.2</b>       |
| Weib prop continuous  | unequal, low           | 6.9        | 6.5             | <b>5.9</b>       |
| Weib prop discrete    | unequal, low           | 7.0        | <b>6.3</b>      | <b>5.7</b>       |
| Weib scale continuous | equal                  | 7.6        | 7.1             | 6.7              |
| Weib scale discrete   | equal                  | 6.7        | <b>6.0</b>      | <b>5.4</b>       |
| Weib scale continuous | unequal, high          | 6.7        | <b>6.1</b>      | <b>4.5</b>       |
| Weib scale discrete   | unequal, high          | <b>5.9</b> | <b>5.4</b>      | <b>4.6</b>       |
| Weib scale continuous | unequal, low           | 7.0        | 6.5             | <b>6.2</b>       |
| Weib scale discrete   | unequal, low           | 6.9        | <b>6.1</b>      | <b>5.5</b>       |
| Weib shape continuous | equal                  | 7.5        | 6.9             | 6.5              |
| Weib shape discrete   | equal                  | 6.5        | <b>6.0</b>      | <b>5.7</b>       |
| Weib shape continuous | unequal, high          | 6.9        | <b>6.4</b>      | <b>5.3</b>       |
| Weib shape discrete   | unequal, high          | 6.7        | <b>6.2</b>      | <b>5.5</b>       |
| Weib shape continuous | unequal, low           | 6.8        | 6.5             | <b>6.4</b>       |
| Weib shape discrete   | unequal, low           | <b>6.3</b> | <b>5.6</b>      | <b>5.6</b>       |

All values in the binomial interval  $[3.7, 6.4]$  are printed in bold type.



Table S10: Rejection rates in percent for the Dunnett-type contrast matrix with  $\delta = 0.0$  and unbalanced large sample sizes.

| Distribution          | Censoring distribution | asymptotic | asymptotic.bonf | permutation.bonf |
|-----------------------|------------------------|------------|-----------------|------------------|
| exp early continuous  | equal                  | <b>5.5</b> | <b>5.4</b>      | <b>5.3</b>       |
| exp early discrete    | equal                  | <b>5.7</b> | <b>5.5</b>      | <b>5.6</b>       |
| exp early continuous  | unequal, high          | <b>4.8</b> | <b>4.7</b>      | <b>4.4</b>       |
| exp early discrete    | unequal, high          | <b>5.6</b> | <b>5.2</b>      | <b>5.6</b>       |
| exp early continuous  | unequal, low           | <b>6.2</b> | <b>5.6</b>      | <b>5.5</b>       |
| exp early discrete    | unequal, low           | <b>6.3</b> | <b>6.0</b>      | <b>6.2</b>       |
| logn continuous       | equal                  | 7.9        | 7.6             | 6.6              |
| logn discrete         | equal                  | 6.7        | 6.6             | 6.8              |
| logn continuous       | unequal, high          | 7.3        | 7.0             | <b>6.2</b>       |
| logn discrete         | unequal, high          | 7.3        | 7.1             | <b>5.4</b>       |
| logn continuous       | unequal, low           | 7.1        | 6.9             | <b>6.0</b>       |
| logn discrete         | unequal, low           | 6.6        | 6.5             | <b>5.6</b>       |
| pwExp continuous      | equal                  | <b>5.8</b> | <b>5.4</b>      | <b>5.2</b>       |
| pwExp discrete        | equal                  | <b>5.4</b> | <b>5.1</b>      | <b>5.4</b>       |
| pwExp continuous      | unequal, high          | <b>5.1</b> | <b>5.0</b>      | <b>5.2</b>       |
| pwExp discrete        | unequal, high          | <b>5.7</b> | <b>5.7</b>      | <b>5.8</b>       |
| pwExp continuous      | unequal, low           | <b>6.1</b> | <b>5.9</b>      | <b>5.4</b>       |
| pwExp discrete        | unequal, low           | <b>6.0</b> | <b>5.8</b>      | <b>5.6</b>       |
| Weib prop continuous  | equal                  | <b>6.0</b> | <b>5.7</b>      | <b>5.6</b>       |
| Weib prop discrete    | equal                  | <b>6.0</b> | <b>5.8</b>      | <b>5.7</b>       |
| Weib prop continuous  | unequal, high          | <b>4.9</b> | <b>4.5</b>      | <b>5.1</b>       |
| Weib prop discrete    | unequal, high          | <b>5.9</b> | <b>5.6</b>      | <b>5.0</b>       |
| Weib prop continuous  | unequal, low           | <b>5.1</b> | <b>4.9</b>      | <b>4.7</b>       |
| Weib prop discrete    | unequal, low           | <b>6.0</b> | <b>5.5</b>      | <b>5.6</b>       |
| Weib scale continuous | equal                  | <b>5.5</b> | <b>5.2</b>      | <b>4.9</b>       |
| Weib scale discrete   | equal                  | <b>5.9</b> | <b>5.7</b>      | <b>5.9</b>       |
| Weib scale continuous | unequal, high          | <b>4.7</b> | <b>4.5</b>      | <b>4.1</b>       |
| Weib scale discrete   | unequal, high          | <b>5.5</b> | <b>5.3</b>      | <b>4.8</b>       |
| Weib scale continuous | unequal, low           | <b>5.0</b> | <b>4.8</b>      | <b>4.9</b>       |
| Weib scale discrete   | unequal, low           | <b>5.8</b> | <b>5.5</b>      | <b>5.0</b>       |
| Weib shape continuous | equal                  | <b>5.7</b> | <b>5.3</b>      | <b>5.8</b>       |
| Weib shape discrete   | equal                  | <b>6.1</b> | <b>5.9</b>      | <b>6.0</b>       |
| Weib shape continuous | unequal, high          | <b>5.3</b> | <b>5.1</b>      | <b>5.1</b>       |
| Weib shape discrete   | unequal, high          | <b>6.0</b> | <b>5.8</b>      | <b>5.2</b>       |
| Weib shape continuous | unequal, low           | <b>5.1</b> | <b>5.0</b>      | <b>4.7</b>       |
| Weib shape discrete   | unequal, low           | <b>6.1</b> | <b>5.8</b>      | <b>5.5</b>       |

All values in the binomial interval  $[3.7, 6.4]$  are printed in bold type.

Table S11: Rejection rates in percent for the Dunnett-type contrast matrix with  $\delta = 0.0$  and unbalanced medium sample sizes.

| Distribution          | Censoring distribution | asymptotic | asymptotic.bonf | permutation.bonf |
|-----------------------|------------------------|------------|-----------------|------------------|
| exp early continuous  | equal                  | 8.0        | 7.8             | <b>6.1</b>       |
| exp early discrete    | equal                  | 7.7        | 7.2             | <b>6.2</b>       |
| exp early continuous  | unequal, high          | 7.9        | 7.6             | <b>5.3</b>       |
| exp early discrete    | unequal, high          | 9.0        | 8.5             | 7.1              |
| exp early continuous  | unequal, low           | 7.5        | 7.4             | <b>5.9</b>       |
| exp early discrete    | unequal, low           | 8.0        | 7.6             | <b>6.1</b>       |
| logn continuous       | equal                  | 10.2       | 9.5             | <b>5.9</b>       |
| logn discrete         | equal                  | 9.3        | 9.0             | <b>5.1</b>       |
| logn continuous       | unequal, high          | 9.4        | 9.1             | <b>4.6</b>       |
| logn discrete         | unequal, high          | 10.7       | 10.4            | <b>4.9</b>       |
| logn continuous       | unequal, low           | 9.0        | 8.8             | <b>5.1</b>       |
| logn discrete         | unequal, low           | 9.2        | 9.0             | <b>4.7</b>       |
| pwExp continuous      | equal                  | 6.7        | 6.7             | <b>4.7</b>       |
| pwExp discrete        | equal                  | 6.7        | <b>6.2</b>      | <b>5.2</b>       |
| pwExp continuous      | unequal, high          | <b>6.0</b> | <b>5.7</b>      | <b>5.0</b>       |
| pwExp discrete        | unequal, high          | 6.7        | 6.5             | <b>5.0</b>       |
| pwExp continuous      | unequal, low           | <b>6.4</b> | <b>6.0</b>      | <b>5.1</b>       |
| pwExp discrete        | unequal, low           | <b>6.4</b> | <b>6.0</b>      | <b>5.2</b>       |
| Weib prop continuous  | equal                  | 8.4        | 7.9             | <b>5.3</b>       |
| Weib prop discrete    | equal                  | 7.8        | 7.3             | <b>5.0</b>       |
| Weib prop continuous  | unequal, high          | 11.6       | 11.1            | 6.9              |
| Weib prop discrete    | unequal, high          | 11.7       | 11.6            | <b>6.4</b>       |
| Weib prop continuous  | unequal, low           | 7.8        | 7.6             | <b>5.1</b>       |
| Weib prop discrete    | unequal, low           | 7.9        | 7.8             | <b>5.8</b>       |
| Weib scale continuous | equal                  | 9.1        | 8.5             | <b>5.9</b>       |
| Weib scale discrete   | equal                  | 9.7        | 9.1             | <b>5.7</b>       |
| Weib scale continuous | unequal, high          | 11.7       | 10.9            | 7.8              |
| Weib scale discrete   | unequal, high          | 12.0       | 11.9            | 6.8              |
| Weib scale continuous | unequal, low           | 9.4        | 9.2             | <b>5.8</b>       |
| Weib scale discrete   | unequal, low           | 8.9        | 8.8             | 6.6              |
| Weib shape continuous | equal                  | 10.4       | 10.0            | <b>6.3</b>       |
| Weib shape discrete   | equal                  | 10.1       | 9.7             | <b>5.6</b>       |
| Weib shape continuous | unequal, high          | 11.1       | 10.6            | 7.3              |
| Weib shape discrete   | unequal, high          | 13.2       | 13.2            | 6.8              |
| Weib shape continuous | unequal, low           | 9.8        | 9.7             | <b>6.4</b>       |
| Weib shape discrete   | unequal, low           | 9.4        | 9.2             | <b>6.3</b>       |

All values in the binomial interval  $[3.7, 6.4]$  are printed in bold type.

Table S12: Rejection rates in percent for the Dunnett-type contrast matrix with  $\delta = 0.0$  and unbalanced small sample sizes.

| Distribution          | Censoring distribution | asymptotic  | asymptotic.bonf | permutation.bonf |
|-----------------------|------------------------|-------------|-----------------|------------------|
| exp early continuous  | equal                  | 17.6        | 17.0            | <b>6.3</b>       |
| exp early discrete    | equal                  | 18.3        | 18.0            | 6.8              |
| exp early continuous  | unequal, high          | 21.6        | 21.2            | <b>6.2</b>       |
| exp early discrete    | unequal, high          | 22.9        | 22.4            | <b>5.4</b>       |
| exp early continuous  | unequal, low           | 16.5        | 16.0            | <b>4.3</b>       |
| exp early discrete    | unequal, low           | 17.6        | 17.1            | <b>4.1</b>       |
| logn continuous       | equal                  | 28.3        | 28.1            | <b>5.4</b>       |
| logn discrete         | equal                  | <b>31.7</b> | <b>31.3</b>     | <b>4.8</b>       |
| logn continuous       | unequal, high          | <b>43.9</b> | <b>43.6</b>     | <b>6.2</b>       |
| logn discrete         | unequal, high          | <b>47.4</b> | <b>46.9</b>     | <b>6.4</b>       |
| logn continuous       | unequal, low           | 24.0        | 23.4            | <b>4.1</b>       |
| logn discrete         | unequal, low           | 26.3        | 25.5            | <b>4.7</b>       |
| pwExp continuous      | equal                  | 16.7        | 16.4            | <b>5.3</b>       |
| pwExp discrete        | equal                  | 16.6        | 16.4            | <b>4.7</b>       |
| pwExp continuous      | unequal, high          | 20.0        | 19.7            | <b>5.2</b>       |
| pwExp discrete        | unequal, high          | 23.3        | 23.0            | <b>4.7</b>       |
| pwExp continuous      | unequal, low           | 16.5        | 16.2            | <b>4.6</b>       |
| pwExp discrete        | unequal, low           | 16.7        | 16.4            | <b>4.3</b>       |
| Weib prop continuous  | equal                  | 23.5        | 23.3            | <b>6.1</b>       |
| Weib prop discrete    | equal                  | 27.4        | 27.2            | <b>6.0</b>       |
| Weib prop continuous  | unequal, high          | <b>38.8</b> | <b>38.4</b>     | <b>5.1</b>       |
| Weib prop discrete    | unequal, high          | <b>43.8</b> | <b>43.4</b>     | <b>6.4</b>       |
| Weib prop continuous  | unequal, low           | 21.5        | 21.0            | <b>4.1</b>       |
| Weib prop discrete    | unequal, low           | 23.7        | 23.2            | <b>4.2</b>       |
| Weib scale continuous | equal                  | <b>31.5</b> | <b>31.2</b>     | 8.8              |
| Weib scale discrete   | equal                  | <b>34.2</b> | <b>34.2</b>     | 8.1              |
| Weib scale continuous | unequal, high          | <b>45.7</b> | <b>45.4</b>     | 6.7              |
| Weib scale discrete   | unequal, high          | <b>51.4</b> | <b>51.0</b>     | 7.1              |
| Weib scale continuous | unequal, low           | 29.0        | 28.7            | <b>6.1</b>       |
| Weib scale discrete   | unequal, low           | <b>32.0</b> | <b>31.7</b>     | <b>5.6</b>       |
| Weib shape continuous | equal                  | <b>35.8</b> | <b>35.6</b>     | 9.3              |
| Weib shape discrete   | equal                  | <b>39.4</b> | <b>39.2</b>     | 9.2              |
| Weib shape continuous | unequal, high          | <b>47.2</b> | <b>47.1</b>     | 6.8              |
| Weib shape discrete   | unequal, high          | <b>54.9</b> | <b>54.6</b>     | 7.5              |
| Weib shape continuous | unequal, low           | <b>34.5</b> | <b>34.0</b>     | 7.7              |
| Weib shape discrete   | unequal, low           | <b>37.3</b> | <b>37.2</b>     | <b>6.4</b>       |

All values in the binomial interval  $[3.7, 6.4]$  are printed in bold type.

Table S13: Rejection rates in percent for the Tukey-type contrast matrix with  $\delta = 0.0$  and balanced large sample sizes.

| Distribution          | Censoring distribution | asymptotic | asymptotic.bonf | permutation.bonf |
|-----------------------|------------------------|------------|-----------------|------------------|
| exp early continuous  | equal                  | <b>5.5</b> | <b>4.4</b>      | <b>5.0</b>       |
| exp early discrete    | equal                  | <b>5.3</b> | <b>4.9</b>      | <b>5.2</b>       |
| exp early continuous  | unequal, high          | <b>6.0</b> | <b>5.6</b>      | <b>4.8</b>       |
| exp early discrete    | unequal, high          | <b>5.3</b> | <b>4.5</b>      | <b>4.4</b>       |
| exp early continuous  | unequal, low           | <b>4.9</b> | <b>3.8</b>      | <b>4.1</b>       |
| exp early discrete    | unequal, low           | <b>5.0</b> | <b>3.9</b>      | <b>4.6</b>       |
| logn continuous       | equal                  | <b>5.2</b> | <b>4.6</b>      | <b>4.9</b>       |
| logn discrete         | equal                  | <b>5.3</b> | <b>4.3</b>      | <b>4.6</b>       |
| logn continuous       | unequal, high          | <b>4.8</b> | <b>3.7</b>      | <b>4.2</b>       |
| logn discrete         | unequal, high          | <b>4.5</b> | <b>3.8</b>      | <b>4.3</b>       |
| logn continuous       | unequal, low           | <b>5.2</b> | <b>4.7</b>      | <b>4.9</b>       |
| logn discrete         | unequal, low           | <b>5.4</b> | <b>4.5</b>      | <b>5.0</b>       |
| pwExp continuous      | equal                  | <b>5.9</b> | <b>5.4</b>      | <b>5.7</b>       |
| pwExp discrete        | equal                  | <b>6.1</b> | <b>5.2</b>      | <b>5.9</b>       |
| pwExp continuous      | unequal, high          | <b>5.7</b> | <b>5.0</b>      | <b>4.4</b>       |
| pwExp discrete        | unequal, high          | <b>5.8</b> | <b>5.1</b>      | <b>4.5</b>       |
| pwExp continuous      | unequal, low           | <b>5.7</b> | <b>5.1</b>      | <b>5.4</b>       |
| pwExp discrete        | unequal, low           | <b>5.5</b> | <b>5.3</b>      | <b>4.9</b>       |
| Weib prop continuous  | equal                  | <b>4.3</b> | <b>3.9</b>      | <b>3.4</b>       |
| Weib prop discrete    | equal                  | <b>5.1</b> | <b>4.4</b>      | <b>4.2</b>       |
| Weib prop continuous  | unequal, high          | <b>6.6</b> | <b>5.6</b>      | <b>5.5</b>       |
| Weib prop discrete    | unequal, high          | <b>6.5</b> | <b>6.0</b>      | <b>5.9</b>       |
| Weib prop continuous  | unequal, low           | <b>5.7</b> | <b>5.2</b>      | <b>4.6</b>       |
| Weib prop discrete    | unequal, low           | <b>6.1</b> | <b>4.9</b>      | <b>5.3</b>       |
| Weib scale continuous | equal                  | <b>4.3</b> | <b>3.8</b>      | <b>4.5</b>       |
| Weib scale discrete   | equal                  | <b>4.8</b> | <b>4.4</b>      | <b>4.3</b>       |
| Weib scale continuous | unequal, high          | <b>5.9</b> | <b>5.1</b>      | <b>5.7</b>       |
| Weib scale discrete   | unequal, high          | <b>6.4</b> | <b>5.8</b>      | <b>6.4</b>       |
| Weib scale continuous | unequal, low           | <b>6.1</b> | <b>5.1</b>      | <b>5.0</b>       |
| Weib scale discrete   | unequal, low           | <b>5.6</b> | <b>5.0</b>      | <b>5.3</b>       |
| Weib shape continuous | equal                  | <b>4.3</b> | <b>3.8</b>      | <b>4.4</b>       |
| Weib shape discrete   | equal                  | <b>5.0</b> | <b>4.5</b>      | <b>4.4</b>       |
| Weib shape continuous | unequal, high          | <b>5.7</b> | <b>5.1</b>      | <b>4.9</b>       |
| Weib shape discrete   | unequal, high          | <b>6.3</b> | <b>5.6</b>      | <b>5.5</b>       |
| Weib shape continuous | unequal, low           | <b>5.7</b> | <b>4.9</b>      | <b>4.9</b>       |
| Weib shape discrete   | unequal, low           | <b>6.0</b> | <b>5.0</b>      | <b>5.0</b>       |

All values in the binomial interval  $[3.7, 6.4]$  are printed in bold type.

Table S14: Rejection rates in percent for the Tukey-type contrast matrix with  $\delta = 0.0$  and balanced medium sample sizes.

| Distribution          | Censoring distribution | asymptotic | asymptotic.bonf | permutation.bonf |
|-----------------------|------------------------|------------|-----------------|------------------|
| exp early continuous  | equal                  | <b>4.5</b> | 3.1             | <b>4.2</b>       |
| exp early discrete    | equal                  | <b>5.2</b> | <b>4.2</b>      | <b>4.0</b>       |
| exp early continuous  | unequal, high          | <b>5.5</b> | <b>4.5</b>      | <b>5.0</b>       |
| exp early discrete    | unequal, high          | <b>5.5</b> | <b>4.7</b>      | <b>4.9</b>       |
| exp early continuous  | unequal, low           | <b>5.7</b> | <b>4.8</b>      | <b>5.0</b>       |
| exp early discrete    | unequal, low           | <b>5.9</b> | <b>5.4</b>      | <b>5.2</b>       |
| logn continuous       | equal                  | <b>4.9</b> | <b>4.5</b>      | <b>5.2</b>       |
| logn discrete         | equal                  | <b>5.4</b> | <b>4.8</b>      | <b>5.9</b>       |
| logn continuous       | unequal, high          | <b>4.1</b> | 3.2             | <b>4.1</b>       |
| logn discrete         | unequal, high          | <b>4.3</b> | <b>3.9</b>      | <b>4.5</b>       |
| logn continuous       | unequal, low           | <b>4.7</b> | <b>4.1</b>      | <b>4.7</b>       |
| logn discrete         | unequal, low           | <b>4.8</b> | <b>3.9</b>      | <b>4.3</b>       |
| pwExp continuous      | equal                  | <b>5.5</b> | <b>4.8</b>      | <b>4.1</b>       |
| pwExp discrete        | equal                  | <b>5.9</b> | <b>5.3</b>      | <b>4.3</b>       |
| pwExp continuous      | unequal, high          | <b>4.6</b> | <b>4.2</b>      | <b>4.2</b>       |
| pwExp discrete        | unequal, high          | <b>4.3</b> | 3.3             | 3.4              |
| pwExp continuous      | unequal, low           | <b>6.3</b> | <b>4.9</b>      | <b>4.9</b>       |
| pwExp discrete        | unequal, low           | <b>6.6</b> | <b>5.5</b>      | <b>4.8</b>       |
| Weib prop continuous  | equal                  | <b>6.0</b> | <b>5.3</b>      | <b>5.4</b>       |
| Weib prop discrete    | equal                  | <b>5.4</b> | <b>4.4</b>      | <b>4.9</b>       |
| Weib prop continuous  | unequal, high          | <b>4.9</b> | <b>4.3</b>      | <b>4.2</b>       |
| Weib prop discrete    | unequal, high          | <b>4.3</b> | 3.6             | <b>4.1</b>       |
| Weib prop continuous  | unequal, low           | <b>5.2</b> | <b>4.3</b>      | <b>4.6</b>       |
| Weib prop discrete    | unequal, low           | <b>5.5</b> | <b>4.5</b>      | <b>5.0</b>       |
| Weib scale continuous | equal                  | <b>6.2</b> | <b>5.5</b>      | <b>4.8</b>       |
| Weib scale discrete   | equal                  | <b>5.4</b> | <b>4.6</b>      | <b>5.0</b>       |
| Weib scale continuous | unequal, high          | <b>5.1</b> | <b>4.2</b>      | <b>3.9</b>       |
| Weib scale discrete   | unequal, high          | <b>4.1</b> | 3.5             | <b>4.5</b>       |
| Weib scale continuous | unequal, low           | <b>5.3</b> | <b>4.1</b>      | <b>5.0</b>       |
| Weib scale discrete   | unequal, low           | <b>5.5</b> | <b>4.5</b>      | <b>5.1</b>       |
| Weib shape continuous | equal                  | <b>6.1</b> | <b>5.4</b>      | <b>5.0</b>       |
| Weib shape discrete   | equal                  | <b>5.9</b> | <b>5.2</b>      | <b>5.7</b>       |
| Weib shape continuous | unequal, high          | <b>5.5</b> | <b>4.7</b>      | <b>4.5</b>       |
| Weib shape discrete   | unequal, high          | <b>5.1</b> | <b>4.3</b>      | <b>4.6</b>       |
| Weib shape continuous | unequal, low           | <b>5.3</b> | <b>4.5</b>      | <b>5.7</b>       |
| Weib shape discrete   | unequal, low           | <b>5.6</b> | <b>4.8</b>      | <b>5.4</b>       |

All values in the binomial interval  $[3.7, 6.4]$  are printed in bold type.

Table S15: Rejection rates in percent for the Tukey-type contrast matrix with  $\delta = 0.0$  and balanced small sample sizes.

| Distribution          | Censoring distribution | asymptotic | asymptotic_bonf | permutation_bonf |
|-----------------------|------------------------|------------|-----------------|------------------|
| exp early continuous  | equal                  | <b>6.3</b> | <b>5.3</b>      | <b>4.2</b>       |
| exp early discrete    | equal                  | <b>6.1</b> | <b>5.5</b>      | <b>4.4</b>       |
| exp early continuous  | unequal, high          | 6.9        | <b>6.0</b>      | <b>5.0</b>       |
| exp early discrete    | unequal, high          | 6.9        | <b>5.7</b>      | <b>4.5</b>       |
| exp early continuous  | unequal, low           | <b>6.3</b> | <b>5.9</b>      | <b>4.2</b>       |
| exp early discrete    | unequal, low           | <b>6.4</b> | <b>5.7</b>      | <b>4.7</b>       |
| logn continuous       | equal                  | <b>6.2</b> | <b>5.5</b>      | <b>5.1</b>       |
| logn discrete         | equal                  | <b>6.0</b> | <b>5.3</b>      | <b>4.8</b>       |
| logn continuous       | unequal, high          | 7.5        | 6.8             | <b>5.4</b>       |
| logn discrete         | unequal, high          | 7.3        | 6.8             | <b>6.2</b>       |
| logn continuous       | unequal, low           | <b>6.3</b> | <b>5.7</b>      | <b>4.4</b>       |
| logn discrete         | unequal, low           | <b>6.1</b> | <b>5.3</b>      | <b>4.2</b>       |
| pwExp continuous      | equal                  | <b>4.4</b> | 3.6             | 3.1              |
| pwExp discrete        | equal                  | <b>4.6</b> | <b>3.9</b>      | <b>3.8</b>       |
| pwExp continuous      | unequal, high          | <b>6.3</b> | <b>5.3</b>      | <b>3.8</b>       |
| pwExp discrete        | unequal, high          | <b>6.0</b> | <b>4.9</b>      | <b>4.2</b>       |
| pwExp continuous      | unequal, low           | <b>5.5</b> | <b>5.0</b>      | <b>4.0</b>       |
| pwExp discrete        | unequal, low           | <b>5.4</b> | <b>4.6</b>      | <b>4.1</b>       |
| Weib prop continuous  | equal                  | 6.7        | <b>5.8</b>      | <b>5.3</b>       |
| Weib prop discrete    | equal                  | <b>5.7</b> | <b>5.0</b>      | <b>5.1</b>       |
| Weib prop continuous  | unequal, high          | 6.8        | <b>5.7</b>      | <b>4.4</b>       |
| Weib prop discrete    | unequal, high          | <b>6.2</b> | <b>5.7</b>      | <b>4.1</b>       |
| Weib prop continuous  | unequal, low           | 6.6        | <b>6.0</b>      | <b>5.1</b>       |
| Weib prop discrete    | unequal, low           | 6.9        | <b>5.8</b>      | <b>4.9</b>       |
| Weib scale continuous | equal                  | 7.0        | <b>6.4</b>      | <b>5.8</b>       |
| Weib scale discrete   | equal                  | <b>5.7</b> | <b>4.9</b>      | <b>4.6</b>       |
| Weib scale continuous | unequal, high          | 6.5        | <b>5.5</b>      | <b>4.3</b>       |
| Weib scale discrete   | unequal, high          | <b>6.1</b> | <b>5.2</b>      | <b>3.7</b>       |
| Weib scale continuous | unequal, low           | 7.0        | <b>5.7</b>      | <b>5.1</b>       |
| Weib scale discrete   | unequal, low           | <b>6.0</b> | <b>5.2</b>      | <b>4.8</b>       |
| Weib shape continuous | equal                  | 6.7        | <b>5.6</b>      | <b>5.3</b>       |
| Weib shape discrete   | equal                  | <b>5.6</b> | <b>4.7</b>      | <b>4.5</b>       |
| Weib shape continuous | unequal, high          | <b>6.4</b> | <b>5.2</b>      | <b>4.2</b>       |
| Weib shape discrete   | unequal, high          | <b>6.4</b> | <b>5.3</b>      | <b>4.7</b>       |
| Weib shape continuous | unequal, low           | 6.5        | <b>5.8</b>      | <b>5.2</b>       |
| Weib shape discrete   | unequal, low           | <b>5.8</b> | <b>4.9</b>      | <b>4.8</b>       |

All values in the binomial interval  $[3.7, 6.4]$  are printed in bold type.

Table S16: Rejection rates in percent for the Tukey-type contrast matrix with  $\delta = 0.0$  and unbalanced large sample sizes.

| Distribution          | Censoring distribution | asymptotic | asymptotic.bonf | permutation.bonf |
|-----------------------|------------------------|------------|-----------------|------------------|
| exp early continuous  | equal                  | <b>5.5</b> | <b>4.9</b>      | <b>4.5</b>       |
| exp early discrete    | equal                  | <b>5.9</b> | <b>5.2</b>      | <b>5.0</b>       |
| exp early continuous  | unequal, high          | <b>5.0</b> | <b>4.4</b>      | <b>4.0</b>       |
| exp early discrete    | unequal, high          | <b>5.4</b> | <b>4.8</b>      | <b>4.8</b>       |
| exp early continuous  | unequal, low           | <b>5.7</b> | <b>5.4</b>      | <b>5.5</b>       |
| exp early discrete    | unequal, low           | <b>6.0</b> | <b>4.9</b>      | <b>5.4</b>       |
| logn continuous       | equal                  | 6.8        | <b>5.5</b>      | <b>5.3</b>       |
| logn discrete         | equal                  | <b>6.4</b> | <b>5.6</b>      | <b>4.9</b>       |
| logn continuous       | unequal, high          | 6.7        | <b>5.2</b>      | <b>4.3</b>       |
| logn discrete         | unequal, high          | <b>5.7</b> | <b>4.7</b>      | <b>4.7</b>       |
| logn continuous       | unequal, low           | 7.2        | <b>5.6</b>      | <b>6.0</b>       |
| logn discrete         | unequal, low           | <b>6.3</b> | <b>5.6</b>      | <b>5.0</b>       |
| pwExp continuous      | equal                  | <b>5.2</b> | <b>4.4</b>      | <b>4.7</b>       |
| pwExp discrete        | equal                  | <b>5.0</b> | <b>4.4</b>      | <b>4.6</b>       |
| pwExp continuous      | unequal, high          | <b>5.6</b> | <b>4.3</b>      | <b>4.7</b>       |
| pwExp discrete        | unequal, high          | <b>5.8</b> | <b>5.0</b>      | <b>5.3</b>       |
| pwExp continuous      | unequal, low           | <b>5.5</b> | <b>4.0</b>      | <b>4.3</b>       |
| pwExp discrete        | unequal, low           | <b>4.9</b> | <b>4.2</b>      | <b>4.4</b>       |
| Weib prop continuous  | equal                  | <b>5.5</b> | <b>4.2</b>      | <b>4.1</b>       |
| Weib prop discrete    | equal                  | <b>6.0</b> | <b>5.1</b>      | <b>5.4</b>       |
| Weib prop continuous  | unequal, high          | <b>4.5</b> | <b>4.0</b>      | <b>4.4</b>       |
| Weib prop discrete    | unequal, high          | <b>5.2</b> | <b>4.2</b>      | <b>4.4</b>       |
| Weib prop continuous  | unequal, low           | <b>5.5</b> | <b>4.0</b>      | <b>3.4</b>       |
| Weib prop discrete    | unequal, low           | <b>4.8</b> | <b>4.0</b>      | <b>4.1</b>       |
| Weib scale continuous | equal                  | <b>5.2</b> | <b>3.8</b>      | <b>3.6</b>       |
| Weib scale discrete   | equal                  | <b>6.0</b> | <b>5.2</b>      | <b>4.6</b>       |
| Weib scale continuous | unequal, high          | <b>4.4</b> | <b>4.0</b>      | <b>3.2</b>       |
| Weib scale discrete   | unequal, high          | <b>4.7</b> | <b>3.8</b>      | <b>3.6</b>       |
| Weib scale continuous | unequal, low           | <b>5.1</b> | <b>4.0</b>      | <b>4.4</b>       |
| Weib scale discrete   | unequal, low           | <b>5.0</b> | <b>4.1</b>      | <b>3.9</b>       |
| Weib shape continuous | equal                  | <b>5.4</b> | <b>4.1</b>      | <b>3.7</b>       |
| Weib shape discrete   | equal                  | <b>6.4</b> | <b>5.3</b>      | <b>5.1</b>       |
| Weib shape continuous | unequal, high          | <b>5.0</b> | <b>4.5</b>      | <b>4.0</b>       |
| Weib shape discrete   | unequal, high          | <b>4.9</b> | <b>4.0</b>      | <b>4.3</b>       |
| Weib shape continuous | unequal, low           | <b>4.9</b> | <b>4.0</b>      | <b>4.0</b>       |
| Weib shape discrete   | unequal, low           | <b>5.0</b> | <b>4.2</b>      | <b>4.1</b>       |

All values in the binomial interval  $[3.7, 6.4]$  are printed in bold type.

Table S17: Rejection rates in percent for the Tukey-type contrast matrix with  $\delta = 0.0$  and unbalanced medium sample sizes.

| Distribution          | Censoring distribution | asymptotic | asymptotic.bonf | permutation.bonf |
|-----------------------|------------------------|------------|-----------------|------------------|
| exp early continuous  | equal                  | 7.0        | 6.6             | <b>5.1</b>       |
| exp early discrete    | equal                  | 6.8        | <b>6.0</b>      | <b>4.5</b>       |
| exp early continuous  | unequal, high          | 7.6        | 6.9             | <b>4.8</b>       |
| exp early discrete    | unequal, high          | 8.7        | 7.8             | <b>5.3</b>       |
| exp early continuous  | unequal, low           | 6.9        | <b>6.1</b>      | <b>5.1</b>       |
| exp early discrete    | unequal, low           | 7.1        | <b>6.3</b>      | <b>5.9</b>       |
| logn continuous       | equal                  | 9.7        | 8.5             | <b>5.6</b>       |
| logn discrete         | equal                  | 9.7        | 8.7             | <b>4.6</b>       |
| logn continuous       | unequal, high          | 9.1        | 8.3             | <b>3.7</b>       |
| logn discrete         | unequal, high          | 10.6       | 9.2             | <b>4.3</b>       |
| logn continuous       | unequal, low           | 9.0        | 8.3             | <b>4.8</b>       |
| logn discrete         | unequal, low           | 9.7        | 8.5             | <b>4.4</b>       |
| pwExp continuous      | equal                  | 7.5        | <b>6.0</b>      | <b>4.8</b>       |
| pwExp discrete        | equal                  | 8.0        | 6.5             | <b>4.5</b>       |
| pwExp continuous      | unequal, high          | <b>6.4</b> | <b>5.5</b>      | 3.4              |
| pwExp discrete        | unequal, high          | 6.8        | <b>5.7</b>      | 3.5              |
| pwExp continuous      | unequal, low           | 7.5        | <b>6.3</b>      | <b>4.7</b>       |
| pwExp discrete        | unequal, low           | 7.4        | <b>6.2</b>      | <b>4.9</b>       |
| Weib prop continuous  | equal                  | 7.7        | 6.7             | <b>3.8</b>       |
| Weib prop discrete    | equal                  | 7.4        | 6.5             | <b>4.1</b>       |
| Weib prop continuous  | unequal, high          | 10.6       | 9.3             | <b>5.4</b>       |
| Weib prop discrete    | unequal, high          | 11.1       | 9.4             | <b>5.4</b>       |
| Weib prop continuous  | unequal, low           | 8.0        | <b>6.4</b>      | <b>3.8</b>       |
| Weib prop discrete    | unequal, low           | 7.9        | 7.2             | <b>3.8</b>       |
| Weib scale continuous | equal                  | 9.3        | 7.6             | <b>4.8</b>       |
| Weib scale discrete   | equal                  | 8.8        | 8.1             | <b>5.9</b>       |
| Weib scale continuous | unequal, high          | 10.7       | 9.7             | <b>5.8</b>       |
| Weib scale discrete   | unequal, high          | 11.9       | 10.9            | <b>6.0</b>       |
| Weib scale continuous | unequal, low           | 9.3        | 7.4             | <b>4.5</b>       |
| Weib scale discrete   | unequal, low           | 9.8        | 9.0             | <b>4.5</b>       |
| Weib shape continuous | equal                  | 9.9        | 8.5             | <b>5.5</b>       |
| Weib shape discrete   | equal                  | 9.4        | 8.5             | <b>5.8</b>       |
| Weib shape continuous | unequal, high          | 10.5       | 9.3             | <b>5.5</b>       |
| Weib shape discrete   | unequal, high          | 11.6       | 11.1            | <b>5.8</b>       |
| Weib shape continuous | unequal, low           | 10.0       | 8.1             | <b>4.6</b>       |
| Weib shape discrete   | unequal, low           | 10.7       | 9.2             | <b>5.1</b>       |

All values in the binomial interval  $[3.7, 6.4]$  are printed in bold type.



Table S18: Rejection rates in percent for the Tukey-type contrast matrix with  $\delta = 0.0$  and unbalanced small sample sizes.

| Distribution          | Censoring distribution | asymptotic  | asymptotic.bonf | permutation.bonf |
|-----------------------|------------------------|-------------|-----------------|------------------|
| exp early continuous  | equal                  | 16.9        | 16.0            | <b>4.6</b>       |
| exp early discrete    | equal                  | 18.2        | 16.4            | <b>5.2</b>       |
| exp early continuous  | unequal, high          | 20.8        | 19.3            | <b>5.4</b>       |
| exp early discrete    | unequal, high          | 22.8        | 21.9            | <b>4.7</b>       |
| exp early continuous  | unequal, low           | 15.8        | 14.6            | <b>3.7</b>       |
| exp early discrete    | unequal, low           | 16.4        | 15.3            | 2.8              |
| logn continuous       | equal                  | 27.9        | 26.5            | <b>5.3</b>       |
| logn discrete         | equal                  | <b>30.3</b> | 29.7            | <b>5.3</b>       |
| logn continuous       | unequal, high          | <b>43.1</b> | <b>41.4</b>     | <b>5.8</b>       |
| logn discrete         | unequal, high          | <b>46.3</b> | <b>43.9</b>     | <b>5.2</b>       |
| logn continuous       | unequal, low           | 23.9        | 21.7            | <b>3.7</b>       |
| logn discrete         | unequal, low           | 25.9        | 23.4            | <b>4.1</b>       |
| pwExp continuous      | equal                  | 16.5        | 14.8            | <b>4.6</b>       |
| pwExp discrete        | equal                  | 16.4        | 15.3            | <b>4.8</b>       |
| pwExp continuous      | unequal, high          | 20.8        | 19.6            | <b>4.9</b>       |
| pwExp discrete        | unequal, high          | 22.9        | 22.4            | <b>4.8</b>       |
| pwExp continuous      | unequal, low           | 16.3        | 15.1            | <b>4.1</b>       |
| pwExp discrete        | unequal, low           | 16.8        | 15.1            | <b>4.4</b>       |
| Weib prop continuous  | equal                  | 23.0        | 22.3            | <b>4.7</b>       |
| Weib prop discrete    | equal                  | 26.7        | 25.7            | <b>4.7</b>       |
| Weib prop continuous  | unequal, high          | <b>37.9</b> | <b>35.8</b>     | <b>5.8</b>       |
| Weib prop discrete    | unequal, high          | <b>42.4</b> | <b>40.8</b>     | <b>5.6</b>       |
| Weib prop continuous  | unequal, low           | 21.1        | 19.1            | 2.8              |
| Weib prop discrete    | unequal, low           | 22.4        | 21.0            | <b>3.9</b>       |
| Weib scale continuous | equal                  | <b>31.1</b> | <b>30.4</b>     | 7.9              |
| Weib scale discrete   | equal                  | <b>34.4</b> | <b>33.1</b>     | 7.0              |
| Weib scale continuous | unequal, high          | <b>44.1</b> | <b>42.1</b>     | 7.3              |
| Weib scale discrete   | unequal, high          | <b>49.8</b> | <b>48.1</b>     | 6.6              |
| Weib scale continuous | unequal, low           | 27.6        | 25.8            | <b>5.7</b>       |
| Weib scale discrete   | unequal, low           | <b>30.8</b> | 29.0            | <b>6.1</b>       |
| Weib shape continuous | equal                  | <b>35.9</b> | <b>35.1</b>     | 9.5              |
| Weib shape discrete   | equal                  | <b>39.1</b> | <b>38.1</b>     | 8.7              |
| Weib shape continuous | unequal, high          | <b>46.3</b> | <b>44.7</b>     | 7.5              |
| Weib shape discrete   | unequal, high          | <b>53.6</b> | <b>52.0</b>     | 6.8              |
| Weib shape continuous | unequal, low           | <b>33.7</b> | <b>32.2</b>     | 7.6              |
| Weib shape discrete   | unequal, low           | <b>35.9</b> | <b>34.3</b>     | 7.7              |

All values in the binomial interval  $[3.7, 6.4]$  are printed in bold type.

Table S19: Rejection rates in percent for the 2-by-2 design with  $\delta = 1.5$  and balanced large sample sizes.

| Distribution          | Censoring distribution | asymptotic | asymptotic_bonf | permutation_bonf |
|-----------------------|------------------------|------------|-----------------|------------------|
| exp early continuous  | equal                  | 100.0      | 100.0           | 100.0            |
| exp early discrete    | equal                  | 100.0      | 100.0           | 100.0            |
| exp early continuous  | unequal, high          | 99.8       | 99.8            | 99.9             |
| exp early discrete    | unequal, high          | 99.8       | 99.8            | 99.9             |
| exp early continuous  | unequal, low           | 100.0      | 100.0           | 100.0            |
| exp early discrete    | unequal, low           | 100.0      | 100.0           | 100.0            |
| exp late continuous   | equal                  | 100.0      | 100.0           | 100.0            |
| exp late discrete     | equal                  | 100.0      | 100.0           | 100.0            |
| exp late continuous   | unequal, high          | 100.0      | 100.0           | 100.0            |
| exp late discrete     | unequal, high          | 99.9       | 99.9            | 99.9             |
| exp late continuous   | unequal, low           | 100.0      | 100.0           | 100.0            |
| exp late discrete     | unequal, low           | 100.0      | 100.0           | 100.0            |
| exp prop continuous   | equal                  | 100.0      | 100.0           | 100.0            |
| exp prop discrete     | equal                  | 100.0      | 100.0           | 100.0            |
| exp prop continuous   | unequal, high          | 100.0      | 100.0           | 99.9             |
| exp prop discrete     | unequal, high          | 100.0      | 100.0           | 100.0            |
| exp prop continuous   | unequal, low           | 100.0      | 100.0           | 100.0            |
| exp prop discrete     | unequal, low           | 100.0      | 100.0           | 100.0            |
| logn continuous       | equal                  | 100.0      | 100.0           | 100.0            |
| logn discrete         | equal                  | 100.0      | 100.0           | 100.0            |
| logn continuous       | unequal, high          | 100.0      | 100.0           | 100.0            |
| logn discrete         | unequal, high          | 100.0      | 100.0           | 100.0            |
| logn continuous       | unequal, low           | 100.0      | 100.0           | 100.0            |
| logn discrete         | unequal, low           | 100.0      | 100.0           | 100.0            |
| pwExp continuous      | equal                  | 100.0      | 100.0           | 100.0            |
| pwExp discrete        | equal                  | 100.0      | 100.0           | 100.0            |
| pwExp continuous      | unequal, high          | 99.3       | 99.3            | 99.4             |
| pwExp discrete        | unequal, high          | 100.0      | 100.0           | 100.0            |
| pwExp continuous      | unequal, low           | 100.0      | 100.0           | 100.0            |
| pwExp discrete        | unequal, low           | 100.0      | 100.0           | 100.0            |
| Weib late continuous  | equal                  | 100.0      | 100.0           | 100.0            |
| Weib late discrete    | equal                  | 100.0      | 100.0           | 100.0            |
| Weib late continuous  | unequal, high          | 100.0      | 100.0           | 100.0            |
| Weib late discrete    | unequal, high          | 100.0      | 100.0           | 100.0            |
| Weib late continuous  | unequal, low           | 100.0      | 100.0           | 100.0            |
| Weib late discrete    | unequal, low           | 100.0      | 100.0           | 100.0            |
| Weib prop continuous  | equal                  | 100.0      | 100.0           | 100.0            |
| Weib prop discrete    | equal                  | 100.0      | 100.0           | 100.0            |
| Weib prop continuous  | unequal, high          | 100.0      | 100.0           | 100.0            |
| Weib prop discrete    | unequal, high          | 100.0      | 100.0           | 100.0            |
| Weib prop continuous  | unequal, low           | 100.0      | 100.0           | 100.0            |
| Weib prop discrete    | unequal, low           | 100.0      | 100.0           | 100.0            |
| Weib scale continuous | equal                  | 100.0      | 100.0           | 100.0            |
| Weib scale discrete   | equal                  | 100.0      | 100.0           | 100.0            |
| Weib scale continuous | unequal, high          | 100.0      | 100.0           | 100.0            |
| Weib scale discrete   | unequal, high          | 100.0      | 100.0           | 100.0            |
| Weib scale continuous | unequal, low           | 100.0      | 100.0           | 100.0            |
| Weib scale discrete   | unequal, low           | 100.0      | 100.0           | 100.0            |
| Weib shape continuous | equal                  | 100.0      | 100.0           | 100.0            |
| Weib shape discrete   | equal                  | 100.0      | 100.0           | 100.0            |
| Weib shape continuous | unequal, high          | 100.0      | 100.0           | 100.0            |
| Weib shape discrete   | unequal, high          | 100.0      | 100.0           | 100.0            |
| Weib shape continuous | unequal, low           | 100.0      | 100.0           | 100.0            |
| Weib shape discrete   | unequal, low           | 100.0      | 100.0           | 100.0            |

Table S20: Rejection rates in percent for the 2-by-2 design with  $\delta = 1.5$  and balanced medium sample sizes.

| Distribution          | Censoring distribution | asymptotic | asymptotic_bonf | permutation_bonf |
|-----------------------|------------------------|------------|-----------------|------------------|
| exp early continuous  | equal                  | 49.4       | 48.5            | 48.0             |
| exp early discrete    | equal                  | 55.1       | 53.7            | 56.5             |
| exp early continuous  | unequal, high          | 40.6       | 39.1            | 39.2             |
| exp early discrete    | unequal, high          | 42.6       | 41.7            | 42.6             |
| exp early continuous  | unequal, low           | 46.4       | 45.6            | 46.6             |
| exp early discrete    | unequal, low           | 52.9       | 52.0            | 51.3             |
| exp late continuous   | equal                  | 52.2       | 50.6            | 51.0             |
| exp late discrete     | equal                  | 59.0       | 56.2            | 58.0             |
| exp late continuous   | unequal, high          | 41.9       | 40.0            | 39.2             |
| exp late discrete     | unequal, high          | 45.1       | 43.1            | 43.3             |
| exp late continuous   | unequal, low           | 50.8       | 49.7            | 48.0             |
| exp late discrete     | unequal, low           | 55.1       | 54.2            | 53.9             |
| exp prop continuous   | equal                  | 50.2       | 49.3            | 48.7             |
| exp prop discrete     | equal                  | 54.8       | 53.5            | 53.8             |
| exp prop continuous   | unequal, high          | 40.9       | 39.5            | 39.3             |
| exp prop discrete     | unequal, high          | 44.2       | 42.8            | 44.3             |
| exp prop continuous   | unequal, low           | 49.3       | 48.3            | 48.6             |
| exp prop discrete     | unequal, low           | 52.6       | 51.4            | 51.4             |
| logn continuous       | equal                  | 94.2       | 93.8            | 93.7             |
| logn discrete         | equal                  | 97.9       | 97.4            | 96.7             |
| logn continuous       | unequal, high          | 73.5       | 72.2            | 71.6             |
| logn discrete         | unequal, high          | 80.8       | 80.0            | 79.1             |
| logn continuous       | unequal, low           | 92.2       | 91.9            | 91.7             |
| logn discrete         | unequal, low           | 97.1       | 97.0            | 96.5             |
| pwExp continuous      | equal                  | 48.3       | 47.2            | 45.6             |
| pwExp discrete        | equal                  | 56.0       | 54.6            | 54.4             |
| pwExp continuous      | unequal, high          | 40.8       | 39.3            | 39.1             |
| pwExp discrete        | unequal, high          | 43.9       | 42.9            | 41.7             |
| pwExp continuous      | unequal, low           | 47.2       | 45.9            | 46.2             |
| pwExp discrete        | unequal, low           | 52.4       | 51.1            | 50.9             |
| Weib late continuous  | equal                  | 94.8       | 94.4            | 94.1             |
| Weib late discrete    | equal                  | 97.0       | 96.7            | 96.3             |
| Weib late continuous  | unequal, high          | 77.4       | 77.0            | 75.2             |
| Weib late discrete    | unequal, high          | 81.7       | 80.9            | 81.8             |
| Weib late continuous  | unequal, low           | 94.5       | 94.3            | 94.3             |
| Weib late discrete    | unequal, low           | 97.4       | 97.1            | 96.4             |
| Weib prop continuous  | equal                  | 93.1       | 92.8            | 92.4             |
| Weib prop discrete    | equal                  | 96.7       | 96.5            | 95.9             |
| Weib prop continuous  | unequal, high          | 76.0       | 74.9            | 74.4             |
| Weib prop discrete    | unequal, high          | 82.3       | 81.4            | 81.1             |
| Weib prop continuous  | unequal, low           | 92.8       | 92.2            | 92.9             |
| Weib prop discrete    | unequal, low           | 96.6       | 96.5            | 96.9             |
| Weib scale continuous | equal                  | 87.2       | 86.6            | 86.8             |
| Weib scale discrete   | equal                  | 92.3       | 91.4            | 92.0             |
| Weib scale continuous | unequal, high          | 70.1       | 69.1            | 68.5             |
| Weib scale discrete   | unequal, high          | 76.3       | 75.5            | 76.3             |
| Weib scale continuous | unequal, low           | 86.9       | 86.3            | 87.1             |
| Weib scale discrete   | unequal, low           | 92.0       | 91.8            | 91.7             |
| Weib shape continuous | equal                  | 78.8       | 77.5            | 79.1             |
| Weib shape discrete   | equal                  | 85.5       | 85.0            | 85.1             |
| Weib shape continuous | unequal, high          | 65.0       | 63.4            | 62.7             |
| Weib shape discrete   | unequal, high          | 71.1       | 70.0            | 70.1             |
| Weib shape continuous | unequal, low           | 77.7       | 76.9            | 77.1             |
| Weib shape discrete   | unequal, low           | 85.4       | 84.7            | 85.6             |

Table S21: Rejection rates in percent for the 2-by-2 design with  $\delta = 1.5$  and balanced small sample sizes.

| Distribution          | Censoring distribution | asymptotic | asymptotic_bonf | permutation_bonf |
|-----------------------|------------------------|------------|-----------------|------------------|
| exp early continuous  | equal                  | 13.0       | 12.1            | 11.8             |
| exp early discrete    | equal                  | 12.3       | 12.1            | 10.7             |
| exp early continuous  | unequal, high          | 12.4       | 11.8            | 10.0             |
| exp early discrete    | unequal, high          | 11.3       | 10.5            | 9.3              |
| exp early continuous  | unequal, low           | 12.9       | 12.2            | 11.3             |
| exp early discrete    | unequal, low           | 13.9       | 13.1            | 11.3             |
| exp late continuous   | equal                  | 14.1       | 13.3            | 12.5             |
| exp late discrete     | equal                  | 14.5       | 14.0            | 14.2             |
| exp late continuous   | unequal, high          | 13.2       | 12.8            | 10.8             |
| exp late discrete     | unequal, high          | 13.2       | 12.2            | 10.3             |
| exp late continuous   | unequal, low           | 13.8       | 12.9            | 12.3             |
| exp late discrete     | unequal, low           | 15.0       | 13.9            | 13.7             |
| exp prop continuous   | equal                  | 12.7       | 12.2            | 10.6             |
| exp prop discrete     | equal                  | 13.2       | 12.8            | 12.0             |
| exp prop continuous   | unequal, high          | 11.8       | 11.4            | 9.2              |
| exp prop discrete     | unequal, high          | 12.3       | 12.3            | 10.2             |
| exp prop continuous   | unequal, low           | 13.2       | 12.5            | 11.9             |
| exp prop discrete     | unequal, low           | 13.2       | 12.7            | 12.3             |
| logn continuous       | equal                  | 29.3       | 28.2            | 27.2             |
| logn discrete         | equal                  | 35.5       | 34.7            | 31.7             |
| logn continuous       | unequal, high          | 22.4       | 21.8            | 19.1             |
| logn discrete         | unequal, high          | 26.6       | 25.8            | 23.1             |
| logn continuous       | unequal, low           | 29.1       | 28.4            | 26.2             |
| logn discrete         | unequal, low           | 33.1       | 32.5            | 31.7             |
| pwExp continuous      | equal                  | 13.6       | 13.1            | 11.3             |
| pwExp discrete        | equal                  | 14.1       | 13.8            | 12.5             |
| pwExp continuous      | unequal, high          | 12.8       | 12.2            | 11.4             |
| pwExp discrete        | unequal, high          | 13.8       | 12.9            | 10.5             |
| pwExp continuous      | unequal, low           | 12.8       | 12.4            | 10.7             |
| pwExp discrete        | unequal, low           | 14.3       | 13.5            | 13.1             |
| Weib late continuous  | equal                  | 30.0       | 29.6            | 27.5             |
| Weib late discrete    | equal                  | 32.6       | 32.0            | 30.3             |
| Weib late continuous  | unequal, high          | 22.1       | 21.9            | 19.0             |
| Weib late discrete    | unequal, high          | 24.0       | 23.3            | 21.4             |
| Weib late continuous  | unequal, low           | 29.2       | 28.7            | 27.0             |
| Weib late discrete    | unequal, low           | 32.7       | 31.7            | 29.8             |
| Weib prop continuous  | equal                  | 28.4       | 27.6            | 25.1             |
| Weib prop discrete    | equal                  | 30.6       | 29.7            | 28.2             |
| Weib prop continuous  | unequal, high          | 21.6       | 21.1            | 19.6             |
| Weib prop discrete    | unequal, high          | 23.7       | 23.1            | 20.7             |
| Weib prop continuous  | unequal, low           | 28.0       | 27.3            | 25.9             |
| Weib prop discrete    | unequal, low           | 31.7       | 30.9            | 28.9             |
| Weib scale continuous | equal                  | 23.9       | 23.1            | 21.7             |
| Weib scale discrete   | equal                  | 26.5       | 25.5            | 23.2             |
| Weib scale continuous | unequal, high          | 19.2       | 18.2            | 15.8             |
| Weib scale discrete   | unequal, high          | 20.5       | 19.8            | 17.5             |
| Weib scale continuous | unequal, low           | 24.3       | 24.0            | 21.3             |
| Weib scale discrete   | unequal, low           | 26.2       | 24.9            | 25.1             |
| Weib shape continuous | equal                  | 19.0       | 18.2            | 17.0             |
| Weib shape discrete   | equal                  | 20.7       | 19.0            | 18.8             |
| Weib shape continuous | unequal, high          | 16.3       | 16.0            | 13.9             |
| Weib shape discrete   | unequal, high          | 17.8       | 17.4            | 15.4             |
| Weib shape continuous | unequal, low           | 18.1       | 17.3            | 17.0             |
| Weib shape discrete   | unequal, low           | 21.0       | 19.5            | 19.3             |

Table S22: Rejection rates in percent for the 2-by-2 design with  $\delta = 1.5$  and unbalanced large sample sizes.

| Distribution          | Censoring distribution | asymptotic | asymptotic_bonf | permutation_bonf |
|-----------------------|------------------------|------------|-----------------|------------------|
| exp early continuous  | equal                  | 93.4       | 92.3            | 91.6             |
| exp early discrete    | equal                  | 96.8       | 96.1            | 95.4             |
| exp early continuous  | unequal, high          | 85.2       | 83.4            | 83.7             |
| exp early discrete    | unequal, high          | 87.7       | 86.2            | 85.1             |
| exp early continuous  | unequal, low           | 93.3       | 91.9            | 91.5             |
| exp early discrete    | unequal, low           | 97.0       | 96.0            | 95.5             |
| exp late continuous   | equal                  | 97.3       | 96.9            | 96.9             |
| exp late discrete     | equal                  | 98.8       | 98.2            | 98.4             |
| exp late continuous   | unequal, high          | 89.6       | 88.3            | 88.2             |
| exp late discrete     | unequal, high          | 93.5       | 91.6            | 90.8             |
| exp late continuous   | unequal, low           | 97.9       | 97.4            | 96.9             |
| exp late discrete     | unequal, low           | 99.1       | 98.6            | 98.5             |
| exp prop continuous   | equal                  | 94.8       | 94.0            | 94.3             |
| exp prop discrete     | equal                  | 98.0       | 97.0            | 96.4             |
| exp prop continuous   | unequal, high          | 85.8       | 83.9            | 83.3             |
| exp prop discrete     | unequal, high          | 89.9       | 88.1            | 86.8             |
| exp prop continuous   | unequal, low           | 95.5       | 94.0            | 93.4             |
| exp prop discrete     | unequal, low           | 98.0       | 97.4            | 96.4             |
| logn continuous       | equal                  | 100.0      | 100.0           | 100.0            |
| logn discrete         | equal                  | 100.0      | 100.0           | 100.0            |
| logn continuous       | unequal, high          | 99.8       | 99.8            | 99.8             |
| logn discrete         | unequal, high          | 99.9       | 99.9            | 99.9             |
| logn continuous       | unequal, low           | 100.0      | 100.0           | 100.0            |
| logn discrete         | unequal, low           | 100.0      | 100.0           | 100.0            |
| pwExp continuous      | equal                  | 92.6       | 90.6            | 91.1             |
| pwExp discrete        | equal                  | 95.6       | 94.5            | 95.2             |
| pwExp continuous      | unequal, high          | 85.0       | 83.0            | 83.4             |
| pwExp discrete        | unequal, high          | 87.6       | 85.7            | 84.9             |
| pwExp continuous      | unequal, low           | 92.7       | 90.4            | 90.7             |
| pwExp discrete        | unequal, low           | 95.9       | 95.1            | 95.0             |
| Weib late continuous  | equal                  | 100.0      | 100.0           | 100.0            |
| Weib late discrete    | equal                  | 99.8       | 99.6            | 99.7             |
| Weib late continuous  | unequal, high          | 100.0      | 100.0           | 99.9             |
| Weib late discrete    | unequal, high          | 99.2       | 99.1            | 99.0             |
| Weib late continuous  | unequal, low           | 100.0      | 100.0           | 100.0            |
| Weib late discrete    | unequal, low           | 99.9       | 99.9            | 99.9             |
| Weib prop continuous  | equal                  | 100.0      | 100.0           | 100.0            |
| Weib prop discrete    | equal                  | 100.0      | 100.0           | 100.0            |
| Weib prop continuous  | unequal, high          | 99.8       | 99.8            | 99.8             |
| Weib prop discrete    | unequal, high          | 100.0      | 100.0           | 99.9             |
| Weib prop continuous  | unequal, low           | 100.0      | 100.0           | 100.0            |
| Weib prop discrete    | unequal, low           | 100.0      | 100.0           | 100.0            |
| Weib scale continuous | equal                  | 100.0      | 100.0           | 100.0            |
| Weib scale discrete   | equal                  | 100.0      | 100.0           | 100.0            |
| Weib scale continuous | unequal, high          | 99.2       | 98.6            | 98.2             |
| Weib scale discrete   | unequal, high          | 99.9       | 99.8            | 99.4             |
| Weib scale continuous | unequal, low           | 100.0      | 100.0           | 100.0            |
| Weib scale discrete   | unequal, low           | 100.0      | 100.0           | 100.0            |
| Weib shape continuous | equal                  | 99.3       | 98.9            | 98.6             |
| Weib shape discrete   | equal                  | 99.6       | 99.5            | 99.6             |
| Weib shape continuous | unequal, high          | 97.2       | 96.2            | 95.3             |
| Weib shape discrete   | unequal, high          | 98.0       | 97.4            | 97.6             |
| Weib shape continuous | unequal, low           | 99.1       | 98.8            | 98.3             |
| Weib shape discrete   | unequal, low           | 99.8       | 99.6            | 99.6             |

Table S23: Rejection rates in percent for the 2-by-2 design with  $\delta = 1.5$  and unbalanced medium sample sizes.

| Distribution          | Censoring distribution | asymptotic | asymptotic_bonf | permutation_bonf |
|-----------------------|------------------------|------------|-----------------|------------------|
| exp early continuous  | equal                  | 22.1       | 19.6            | 16.2             |
| exp early discrete    | equal                  | 24.7       | 22.3            | 19.3             |
| exp early continuous  | unequal, high          | 20.3       | 18.3            | 14.8             |
| exp early discrete    | unequal, high          | 20.9       | 19.4            | 15.0             |
| exp early continuous  | unequal, low           | 20.9       | 19.1            | 15.6             |
| exp early discrete    | unequal, low           | 24.0       | 21.4            | 18.4             |
| exp late continuous   | equal                  | 26.7       | 23.5            | 19.5             |
| exp late discrete     | equal                  | 27.6       | 25.4            | 22.1             |
| exp late continuous   | unequal, high          | 21.2       | 19.6            | 15.5             |
| exp late discrete     | unequal, high          | 22.3       | 20.0            | 16.8             |
| exp late continuous   | unequal, low           | 24.5       | 22.2            | 18.9             |
| exp late discrete     | unequal, low           | 27.6       | 25.5            | 21.0             |
| exp prop continuous   | equal                  | 22.9       | 20.6            | 17.8             |
| exp prop discrete     | equal                  | 25.3       | 23.2            | 20.9             |
| exp prop continuous   | unequal, high          | 19.2       | 17.5            | 14.0             |
| exp prop discrete     | unequal, high          | 21.3       | 19.7            | 15.5             |
| exp prop continuous   | unequal, low           | 23.6       | 21.2            | 17.8             |
| exp prop discrete     | unequal, low           | 26.5       | 23.9            | 21.2             |
| logn continuous       | equal                  | 50.4       | 47.3            | 40.8             |
| logn discrete         | equal                  | 58.6       | 54.3            | 48.0             |
| logn continuous       | unequal, high          | 36.1       | 33.5            | 25.3             |
| logn discrete         | unequal, high          | 40.3       | 36.1            | 26.5             |
| logn continuous       | unequal, low           | 53.9       | 50.4            | 43.0             |
| logn discrete         | unequal, low           | 61.7       | 58.1            | 49.2             |
| pwExp continuous      | equal                  | 21.3       | 17.9            | 16.8             |
| pwExp discrete        | equal                  | 24.3       | 21.0            | 19.0             |
| pwExp continuous      | unequal, high          | 18.9       | 17.0            | 14.3             |
| pwExp discrete        | unequal, high          | 20.1       | 18.5            | 15.0             |
| pwExp continuous      | unequal, low           | 21.0       | 18.6            | 14.9             |
| pwExp discrete        | unequal, low           | 23.5       | 21.2            | 17.8             |
| Weib late continuous  | equal                  | 56.0       | 52.0            | 45.0             |
| Weib late discrete    | equal                  | 62.9       | 59.6            | 51.4             |
| Weib late continuous  | unequal, high          | 38.6       | 35.2            | 26.4             |
| Weib late discrete    | unequal, high          | 45.3       | 40.8            | 29.4             |
| Weib late continuous  | unequal, low           | 60.8       | 56.3            | 48.7             |
| Weib late discrete    | unequal, low           | 69.3       | 65.1            | 55.2             |
| Weib prop continuous  | equal                  | 50.9       | 47.1            | 39.6             |
| Weib prop discrete    | equal                  | 57.6       | 52.8            | 44.6             |
| Weib prop continuous  | unequal, high          | 35.4       | 32.5            | 24.6             |
| Weib prop discrete    | unequal, high          | 41.4       | 38.7            | 26.9             |
| Weib prop continuous  | unequal, low           | 54.3       | 51.0            | 43.4             |
| Weib prop discrete    | unequal, low           | 62.7       | 58.8            | 49.7             |
| Weib scale continuous | equal                  | 39.4       | 35.0            | 28.9             |
| Weib scale discrete   | equal                  | 43.4       | 40.4            | 33.5             |
| Weib scale continuous | unequal, high          | 28.7       | 26.1            | 18.9             |
| Weib scale discrete   | unequal, high          | 32.2       | 29.1            | 19.3             |
| Weib scale continuous | unequal, low           | 40.2       | 36.7            | 30.7             |
| Weib scale discrete   | unequal, low           | 46.5       | 42.8            | 34.3             |
| Weib shape continuous | equal                  | 25.6       | 20.9            | 16.8             |
| Weib shape discrete   | equal                  | 31.4       | 26.8            | 21.9             |
| Weib shape continuous | unequal, high          | 22.5       | 20.1            | 14.9             |
| Weib shape discrete   | unequal, high          | 24.7       | 22.3            | 15.2             |
| Weib shape continuous | unequal, low           | 26.1       | 21.0            | 16.2             |
| Weib shape discrete   | unequal, low           | 33.3       | 28.9            | 20.9             |

Table S24: Rejection rates in percent for the 2-by-2 design with  $\delta = 1.5$  and unbalanced small sample sizes.

| Distribution          | Censoring distribution | asymptotic | asymptotic_bonf | permutation_bonf |
|-----------------------|------------------------|------------|-----------------|------------------|
| exp early continuous  | equal                  | 9.1        | 8.2             | 3.5              |
| exp early discrete    | equal                  | 8.9        | 8.2             | 3.7              |
| exp early continuous  | unequal, high          | 10.4       | 9.7             | 2.3              |
| exp early discrete    | unequal, high          | 10.7       | 9.8             | 2.7              |
| exp early continuous  | unequal, low           | 9.1        | 8.0             | 3.4              |
| exp early discrete    | unequal, low           | 8.6        | 7.9             | 3.0              |
| exp late continuous   | equal                  | 9.4        | 8.5             | 3.5              |
| exp late discrete     | equal                  | 10.6       | 9.4             | 4.1              |
| exp late continuous   | unequal, high          | 10.6       | 9.6             | 2.2              |
| exp late discrete     | unequal, high          | 11.3       | 10.4            | 2.4              |
| exp late continuous   | unequal, low           | 8.9        | 7.3             | 3.1              |
| exp late discrete     | unequal, low           | 9.6        | 8.1             | 2.8              |
| exp prop continuous   | equal                  | 10.4       | 9.6             | 3.9              |
| exp prop discrete     | equal                  | 10.8       | 9.9             | 4.8              |
| exp prop continuous   | unequal, high          | 10.7       | 9.9             | 3.0              |
| exp prop discrete     | unequal, high          | 9.9        | 9.1             | 3.6              |
| exp prop continuous   | unequal, low           | 9.9        | 9.2             | 4.0              |
| exp prop discrete     | unequal, low           | 10.7       | 9.8             | 3.7              |
| logn continuous       | equal                  | 12.0       | 11.4            | 3.4              |
| logn discrete         | equal                  | 13.1       | 11.6            | 4.2              |
| logn continuous       | unequal, high          | 13.1       | 12.0            | 4.5              |
| logn discrete         | unequal, high          | 15.0       | 13.7            | 4.7              |
| logn continuous       | unequal, low           | 11.7       | 10.4            | 3.2              |
| logn discrete         | unequal, low           | 12.8       | 11.7            | 3.2              |
| pwExp continuous      | equal                  | 8.6        | 8.0             | 3.3              |
| pwExp discrete        | equal                  | 9.5        | 8.2             | 3.5              |
| pwExp continuous      | unequal, high          | 9.4        | 8.8             | 2.1              |
| pwExp discrete        | unequal, high          | 10.2       | 9.3             | 2.6              |
| pwExp continuous      | unequal, low           | 8.9        | 7.2             | 2.9              |
| pwExp discrete        | unequal, low           | 8.7        | 7.6             | 2.9              |
| Weib late continuous  | equal                  | 13.1       | 11.5            | 3.9              |
| Weib late discrete    | equal                  | 14.3       | 12.4            | 4.5              |
| Weib late continuous  | unequal, high          | 14.6       | 13.1            | 3.8              |
| Weib late discrete    | unequal, high          | 15.6       | 14.1            | 4.1              |
| Weib late continuous  | unequal, low           | 14.0       | 12.9            | 3.8              |
| Weib late discrete    | unequal, low           | 16.1       | 13.9            | 4.4              |
| Weib prop continuous  | equal                  | 12.1       | 10.8            | 3.5              |
| Weib prop discrete    | equal                  | 13.4       | 11.9            | 3.8              |
| Weib prop continuous  | unequal, high          | 13.7       | 12.4            | 3.5              |
| Weib prop discrete    | unequal, high          | 13.9       | 12.3            | 4.0              |
| Weib prop continuous  | unequal, low           | 12.7       | 10.8            | 3.6              |
| Weib prop discrete    | unequal, low           | 13.3       | 12.0            | 3.8              |
| Weib scale continuous | equal                  | 11.4       | 10.2            | 3.6              |
| Weib scale discrete   | equal                  | 11.3       | 10.2            | 3.9              |
| Weib scale continuous | unequal, high          | 13.2       | 12.1            | 3.9              |
| Weib scale discrete   | unequal, high          | 13.5       | 11.4            | 3.6              |
| Weib scale continuous | unequal, low           | 9.8        | 8.4             | 3.3              |
| Weib scale discrete   | unequal, low           | 10.0       | 8.5             | 3.2              |
| Weib shape continuous | equal                  | 15.0       | 13.2            | 6.6              |
| Weib shape discrete   | equal                  | 14.8       | 13.3            | 5.7              |
| Weib shape continuous | unequal, high          | 12.9       | 11.3            | 3.6              |
| Weib shape discrete   | unequal, high          | 13.7       | 12.1            | 3.6              |
| Weib shape continuous | unequal, low           | 12.9       | 12.1            | 5.6              |
| Weib shape discrete   | unequal, low           | 12.8       | 12.0            | 5.0              |

Table S25: Rejection rates in percent for the Dunnett-type contrast matrix with  $\delta = 1.5$  and balanced large sample sizes.

| Distribution          | Censoring distribution | asymptotic | asymptotic_bonf | permutation_bonf |
|-----------------------|------------------------|------------|-----------------|------------------|
| exp early continuous  | equal                  | 100.0      | 100.0           | 100.0            |
| exp early discrete    | equal                  | 100.0      | 100.0           | 100.0            |
| exp early continuous  | unequal, high          | 99.9       | 99.9            | 99.9             |
| exp early discrete    | unequal, high          | 100.0      | 100.0           | 100.0            |
| exp early continuous  | unequal, low           | 100.0      | 100.0           | 100.0            |
| exp early discrete    | unequal, low           | 100.0      | 100.0           | 100.0            |
| exp late continuous   | equal                  | 100.0      | 100.0           | 100.0            |
| exp late discrete     | equal                  | 100.0      | 100.0           | 100.0            |
| exp late continuous   | unequal, high          | 100.0      | 100.0           | 100.0            |
| exp late discrete     | unequal, high          | 99.9       | 99.9            | 99.9             |
| exp late continuous   | unequal, low           | 100.0      | 100.0           | 100.0            |
| exp late discrete     | unequal, low           | 100.0      | 100.0           | 100.0            |
| exp prop continuous   | equal                  | 100.0      | 100.0           | 100.0            |
| exp prop discrete     | equal                  | 100.0      | 100.0           | 100.0            |
| exp prop continuous   | unequal, high          | 100.0      | 100.0           | 100.0            |
| exp prop discrete     | unequal, high          | 100.0      | 100.0           | 100.0            |
| exp prop continuous   | unequal, low           | 100.0      | 100.0           | 100.0            |
| exp prop discrete     | unequal, low           | 100.0      | 100.0           | 100.0            |
| logn continuous       | equal                  | 100.0      | 100.0           | 100.0            |
| logn discrete         | equal                  | 100.0      | 100.0           | 100.0            |
| logn continuous       | unequal, high          | 100.0      | 100.0           | 100.0            |
| logn discrete         | unequal, high          | 100.0      | 100.0           | 100.0            |
| logn continuous       | unequal, low           | 100.0      | 100.0           | 100.0            |
| logn discrete         | unequal, low           | 100.0      | 100.0           | 100.0            |
| pwExp continuous      | equal                  | 100.0      | 100.0           | 100.0            |
| pwExp discrete        | equal                  | 100.0      | 100.0           | 100.0            |
| pwExp continuous      | unequal, high          | 100.0      | 100.0           | 100.0            |
| pwExp discrete        | unequal, high          | 100.0      | 100.0           | 100.0            |
| pwExp continuous      | unequal, low           | 100.0      | 100.0           | 100.0            |
| pwExp discrete        | unequal, low           | 100.0      | 100.0           | 100.0            |
| Weib late continuous  | equal                  | 100.0      | 100.0           | 100.0            |
| Weib late discrete    | equal                  | 100.0      | 100.0           | 100.0            |
| Weib late continuous  | unequal, high          | 100.0      | 100.0           | 100.0            |
| Weib late discrete    | unequal, high          | 100.0      | 100.0           | 100.0            |
| Weib late continuous  | unequal, low           | 100.0      | 100.0           | 100.0            |
| Weib late discrete    | unequal, low           | 100.0      | 100.0           | 100.0            |
| Weib prop continuous  | equal                  | 100.0      | 100.0           | 100.0            |
| Weib prop discrete    | equal                  | 100.0      | 100.0           | 100.0            |
| Weib prop continuous  | unequal, high          | 100.0      | 100.0           | 100.0            |
| Weib prop discrete    | unequal, high          | 100.0      | 100.0           | 100.0            |
| Weib prop continuous  | unequal, low           | 100.0      | 100.0           | 100.0            |
| Weib prop discrete    | unequal, low           | 100.0      | 100.0           | 100.0            |
| Weib scale continuous | equal                  | 100.0      | 100.0           | 100.0            |
| Weib scale discrete   | equal                  | 100.0      | 100.0           | 100.0            |
| Weib scale continuous | unequal, high          | 100.0      | 100.0           | 100.0            |
| Weib scale discrete   | unequal, high          | 100.0      | 100.0           | 100.0            |
| Weib scale continuous | unequal, low           | 100.0      | 100.0           | 100.0            |
| Weib scale discrete   | unequal, low           | 100.0      | 100.0           | 100.0            |
| Weib shape continuous | equal                  | 100.0      | 100.0           | 100.0            |
| Weib shape discrete   | equal                  | 100.0      | 100.0           | 100.0            |
| Weib shape continuous | unequal, high          | 100.0      | 100.0           | 100.0            |
| Weib shape discrete   | unequal, high          | 100.0      | 100.0           | 100.0            |
| Weib shape continuous | unequal, low           | 100.0      | 100.0           | 100.0            |
| Weib shape discrete   | unequal, low           | 100.0      | 100.0           | 100.0            |



Table S26: Rejection rates in percent for the Dunnett-type contrast matrix with  $\delta = 1.5$  and balanced medium sample sizes.

| Distribution          | Censoring distribution | asymptotic | asymptotic_bonf | permutation_bonf |
|-----------------------|------------------------|------------|-----------------|------------------|
| exp early continuous  | equal                  | 46.5       | 43.8            | 42.7             |
| exp early discrete    | equal                  | 53.9       | 50.7            | 50.7             |
| exp early continuous  | unequal, high          | 37.0       | 34.2            | 33.2             |
| exp early discrete    | unequal, high          | 39.3       | 37.5            | 37.0             |
| exp early continuous  | unequal, low           | 45.7       | 42.2            | 42.9             |
| exp early discrete    | unequal, low           | 52.9       | 49.7            | 50.1             |
| exp late continuous   | equal                  | 50.7       | 46.7            | 47.4             |
| exp late discrete     | equal                  | 58.9       | 55.6            | 55.7             |
| exp late continuous   | unequal, high          | 38.3       | 36.5            | 35.4             |
| exp late discrete     | unequal, high          | 42.3       | 39.4            | 39.2             |
| exp late continuous   | unequal, low           | 50.4       | 47.2            | 47.4             |
| exp late discrete     | unequal, low           | 57.6       | 54.8            | 55.2             |
| exp prop continuous   | equal                  | 49.8       | 47.4            | 45.9             |
| exp prop discrete     | equal                  | 55.6       | 52.3            | 50.9             |
| exp prop continuous   | unequal, high          | 40.7       | 37.6            | 37.3             |
| exp prop discrete     | unequal, high          | 43.2       | 40.8            | 40.6             |
| exp prop continuous   | unequal, low           | 47.4       | 44.7            | 45.4             |
| exp prop discrete     | unequal, low           | 53.1       | 50.8            | 49.6             |
| logn continuous       | equal                  | 93.9       | 93.1            | 93.2             |
| logn discrete         | equal                  | 96.8       | 96.3            | 96.3             |
| logn continuous       | unequal, high          | 74.7       | 72.6            | 71.5             |
| logn discrete         | unequal, high          | 82.8       | 81.7            | 80.3             |
| logn continuous       | unequal, low           | 94.8       | 93.5            | 93.3             |
| logn discrete         | unequal, low           | 96.9       | 96.3            | 96.4             |
| pwExp continuous      | equal                  | 45.5       | 43.4            | 42.9             |
| pwExp discrete        | equal                  | 52.4       | 49.8            | 48.2             |
| pwExp continuous      | unequal, high          | 36.2       | 34.5            | 33.0             |
| pwExp discrete        | unequal, high          | 40.5       | 38.4            | 38.5             |
| pwExp continuous      | unequal, low           | 46.5       | 43.8            | 43.9             |
| pwExp discrete        | unequal, low           | 52.7       | 49.9            | 49.5             |
| Weib late continuous  | equal                  | 95.2       | 94.2            | 93.4             |
| Weib late discrete    | equal                  | 96.6       | 95.7            | 95.6             |
| Weib late continuous  | unequal, high          | 78.8       | 77.8            | 76.0             |
| Weib late discrete    | unequal, high          | 82.6       | 81.0            | 79.2             |
| Weib late continuous  | unequal, low           | 96.9       | 95.6            | 95.2             |
| Weib late discrete    | unequal, low           | 97.8       | 97.7            | 97.2             |
| Weib prop continuous  | equal                  | 92.7       | 92.1            | 91.5             |
| Weib prop discrete    | equal                  | 97.0       | 96.6            | 96.7             |
| Weib prop continuous  | unequal, high          | 76.2       | 74.8            | 73.1             |
| Weib prop discrete    | unequal, high          | 84.8       | 83.2            | 82.3             |
| Weib prop continuous  | unequal, low           | 95.2       | 94.2            | 93.6             |
| Weib prop discrete    | unequal, low           | 98.0       | 97.4            | 96.7             |
| Weib scale continuous | equal                  | 86.0       | 84.5            | 84.2             |
| Weib scale discrete   | equal                  | 92.2       | 91.4            | 91.4             |
| Weib scale continuous | unequal, high          | 69.2       | 67.2            | 66.2             |
| Weib scale discrete   | unequal, high          | 78.7       | 77.1            | 75.7             |
| Weib scale continuous | unequal, low           | 89.0       | 87.2            | 85.9             |
| Weib scale discrete   | unequal, low           | 93.7       | 92.8            | 91.6             |
| Weib shape continuous | equal                  | 72.0       | 69.9            | 68.2             |
| Weib shape discrete   | equal                  | 81.8       | 80.4            | 79.6             |
| Weib shape continuous | unequal, high          | 60.8       | 58.6            | 56.4             |
| Weib shape discrete   | unequal, high          | 67.2       | 66.3            | 64.9             |
| Weib shape continuous | unequal, low           | 71.5       | 69.7            | 69.8             |
| Weib shape discrete   | unequal, low           | 83.0       | 81.1            | 80.8             |

Table S27: Rejection rates in percent for the Dunnett-type contrast matrix with  $\delta = 1.5$  and balanced small sample sizes.

| Distribution          | Censoring distribution | asymptotic | asymptotic_bonf | permutation_bonf |
|-----------------------|------------------------|------------|-----------------|------------------|
| exp early continuous  | equal                  | 11.6       | 10.1            | 8.0              |
| exp early discrete    | equal                  | 10.1       | 9.5             | 8.7              |
| exp early continuous  | unequal, high          | 11.7       | 10.6            | 8.7              |
| exp early discrete    | unequal, high          | 9.7        | 8.6             | 7.3              |
| exp early continuous  | unequal, low           | 11.5       | 10.2            | 9.0              |
| exp early discrete    | unequal, low           | 10.4       | 9.2             | 7.9              |
| exp late continuous   | equal                  | 12.2       | 10.5            | 8.3              |
| exp late discrete     | equal                  | 12.0       | 10.5            | 9.5              |
| exp late continuous   | unequal, high          | 12.6       | 11.3            | 8.8              |
| exp late discrete     | unequal, high          | 12.3       | 10.9            | 8.8              |
| exp late continuous   | unequal, low           | 12.0       | 10.7            | 9.5              |
| exp late discrete     | unequal, low           | 13.2       | 11.6            | 10.4             |
| exp prop continuous   | equal                  | 10.0       | 9.7             | 7.3              |
| exp prop discrete     | equal                  | 12.0       | 11.2            | 10.0             |
| exp prop continuous   | unequal, high          | 11.1       | 10.6            | 8.1              |
| exp prop discrete     | unequal, high          | 10.5       | 9.4             | 7.8              |
| exp prop continuous   | unequal, low           | 10.4       | 9.2             | 7.9              |
| exp prop discrete     | unequal, low           | 11.5       | 10.8            | 8.9              |
| logn continuous       | equal                  | 24.1       | 22.2            | 20.1             |
| logn discrete         | equal                  | 27.4       | 25.8            | 23.3             |
| logn continuous       | unequal, high          | 19.2       | 18.0            | 16.0             |
| logn discrete         | unequal, high          | 20.9       | 19.9            | 17.5             |
| logn continuous       | unequal, low           | 25.4       | 23.7            | 20.9             |
| logn discrete         | unequal, low           | 28.8       | 26.8            | 25.7             |
| pwExp continuous      | equal                  | 10.9       | 9.5             | 7.3              |
| pwExp discrete        | equal                  | 10.9       | 9.7             | 7.6              |
| pwExp continuous      | unequal, high          | 11.3       | 10.4            | 7.5              |
| pwExp discrete        | unequal, high          | 12.4       | 11.3            | 9.1              |
| pwExp continuous      | unequal, low           | 10.5       | 8.9             | 8.1              |
| pwExp discrete        | unequal, low           | 11.4       | 10.1            | 8.8              |
| Weib late continuous  | equal                  | 23.4       | 21.9            | 19.9             |
| Weib late discrete    | equal                  | 27.1       | 24.9            | 22.1             |
| Weib late continuous  | unequal, high          | 18.4       | 17.5            | 13.3             |
| Weib late discrete    | unequal, high          | 21.3       | 20.2            | 16.1             |
| Weib late continuous  | unequal, low           | 27.5       | 26.3            | 22.6             |
| Weib late discrete    | unequal, low           | 30.6       | 29.1            | 25.9             |
| Weib prop continuous  | equal                  | 21.8       | 20.7            | 18.4             |
| Weib prop discrete    | equal                  | 24.4       | 23.1            | 20.0             |
| Weib prop continuous  | unequal, high          | 17.8       | 16.7            | 12.8             |
| Weib prop discrete    | unequal, high          | 20.0       | 19.0            | 14.5             |
| Weib prop continuous  | unequal, low           | 25.6       | 23.5            | 21.7             |
| Weib prop discrete    | unequal, low           | 29.3       | 26.9            | 24.6             |
| Weib scale continuous | equal                  | 16.8       | 15.6            | 14.1             |
| Weib scale discrete   | equal                  | 17.5       | 15.9            | 15.3             |
| Weib scale continuous | unequal, high          | 13.3       | 12.6            | 10.7             |
| Weib scale discrete   | unequal, high          | 14.6       | 13.5            | 11.3             |
| Weib scale continuous | unequal, low           | 18.3       | 16.7            | 15.8             |
| Weib scale discrete   | unequal, low           | 20.4       | 18.7            | 17.2             |
| Weib shape continuous | equal                  | 12.2       | 11.2            | 10.9             |
| Weib shape discrete   | equal                  | 13.5       | 12.3            | 11.6             |
| Weib shape continuous | unequal, high          | 10.8       | 10.1            | 8.7              |
| Weib shape discrete   | unequal, high          | 11.6       | 10.7            | 9.7              |
| Weib shape continuous | unequal, low           | 12.1       | 11.2            | 11.7             |
| Weib shape discrete   | unequal, low           | 13.2       | 12.7            | 13.1             |

Table S28: Rejection rates in percent for the Dunnett-type contrast matrix with  $\delta = 1.5$  and unbalanced large sample sizes.

| Distribution          | Censoring distribution | asymptotic | asymptotic_bonf | permutation_bonf |
|-----------------------|------------------------|------------|-----------------|------------------|
| exp early continuous  | equal                  | 89.8       | 89.1            | 85.7             |
| exp early discrete    | equal                  | 94.7       | 93.8            | 92.2             |
| exp early continuous  | unequal, high          | 83.5       | 82.2            | 78.1             |
| exp early discrete    | unequal, high          | 86.9       | 86.0            | 83.3             |
| exp early continuous  | unequal, low           | 90.1       | 88.8            | 88.0             |
| exp early discrete    | unequal, low           | 94.7       | 93.8            | 92.4             |
| exp late continuous   | equal                  | 97.1       | 96.9            | 94.9             |
| exp late discrete     | equal                  | 98.6       | 98.5            | 97.1             |
| exp late continuous   | unequal, high          | 89.2       | 88.1            | 84.5             |
| exp late discrete     | unequal, high          | 92.6       | 91.9            | 88.5             |
| exp late continuous   | unequal, low           | 97.7       | 97.5            | 96.0             |
| exp late discrete     | unequal, low           | 99.3       | 99.2            | 98.8             |
| exp prop continuous   | equal                  | 94.7       | 94.3            | 92.3             |
| exp prop discrete     | equal                  | 98.0       | 97.7            | 96.3             |
| exp prop continuous   | unequal, high          | 84.3       | 82.9            | 80.2             |
| exp prop discrete     | unequal, high          | 89.4       | 88.6            | 83.8             |
| exp prop continuous   | unequal, low           | 94.6       | 94.1            | 92.8             |
| exp prop discrete     | unequal, low           | 97.9       | 97.8            | 96.2             |
| logn continuous       | equal                  | 100.0      | 100.0           | 100.0            |
| logn discrete         | equal                  | 100.0      | 100.0           | 100.0            |
| logn continuous       | unequal, high          | 99.8       | 99.8            | 99.7             |
| logn discrete         | unequal, high          | 99.9       | 99.9            | 99.6             |
| logn continuous       | unequal, low           | 100.0      | 100.0           | 100.0            |
| logn discrete         | unequal, low           | 100.0      | 100.0           | 100.0            |
| pwExp continuous      | equal                  | 88.8       | 88.1            | 85.3             |
| pwExp discrete        | equal                  | 93.5       | 92.9            | 91.3             |
| pwExp continuous      | unequal, high          | 81.5       | 80.8            | 78.0             |
| pwExp discrete        | unequal, high          | 85.5       | 84.4            | 82.3             |
| pwExp continuous      | unequal, low           | 88.4       | 87.4            | 85.0             |
| pwExp discrete        | unequal, low           | 94.5       | 94.4            | 92.2             |
| Weib late continuous  | equal                  | 100.0      | 100.0           | 100.0            |
| Weib late discrete    | equal                  | 99.7       | 99.7            | 99.5             |
| Weib late continuous  | unequal, high          | 100.0      | 100.0           | 99.9             |
| Weib late discrete    | unequal, high          | 98.8       | 98.8            | 98.7             |
| Weib late continuous  | unequal, low           | 100.0      | 100.0           | 100.0            |
| Weib late discrete    | unequal, low           | 99.9       | 99.9            | 99.9             |
| Weib prop continuous  | equal                  | 100.0      | 100.0           | 100.0            |
| Weib prop discrete    | equal                  | 100.0      | 100.0           | 100.0            |
| Weib prop continuous  | unequal, high          | 100.0      | 100.0           | 99.5             |
| Weib prop discrete    | unequal, high          | 100.0      | 100.0           | 99.8             |
| Weib prop continuous  | unequal, low           | 100.0      | 100.0           | 100.0            |
| Weib prop discrete    | unequal, low           | 100.0      | 100.0           | 100.0            |
| Weib scale continuous | equal                  | 99.9       | 99.9            | 99.7             |
| Weib scale discrete   | equal                  | 100.0      | 100.0           | 100.0            |
| Weib scale continuous | unequal, high          | 98.5       | 98.2            | 97.2             |
| Weib scale discrete   | unequal, high          | 99.7       | 99.7            | 98.8             |
| Weib scale continuous | unequal, low           | 100.0      | 100.0           | 99.8             |
| Weib scale discrete   | unequal, low           | 100.0      | 100.0           | 100.0            |
| Weib shape continuous | equal                  | 97.2       | 96.9            | 95.3             |
| Weib shape discrete   | equal                  | 99.2       | 99.1            | 98.3             |
| Weib shape continuous | unequal, high          | 94.1       | 93.8            | 90.6             |
| Weib shape discrete   | unequal, high          | 97.1       | 96.9            | 94.0             |
| Weib shape continuous | unequal, low           | 96.9       | 96.6            | 95.5             |
| Weib shape discrete   | unequal, low           | 98.9       | 98.9            | 98.1             |

Table S29: Rejection rates in percent for the Dunnett-type contrast matrix with  $\delta = 1.5$  and unbalanced medium sample sizes.

| Distribution          | Censoring distribution | asymptotic | asymptotic_bonf | permutation_bonf |
|-----------------------|------------------------|------------|-----------------|------------------|
| exp early continuous  | equal                  | 14.1       | 13.8            | 8.5              |
| exp early discrete    | equal                  | 16.0       | 15.0            | 9.9              |
| exp early continuous  | unequal, high          | 12.9       | 12.2            | 7.1              |
| exp early discrete    | unequal, high          | 13.5       | 12.9            | 6.5              |
| exp early continuous  | unequal, low           | 14.5       | 13.5            | 9.5              |
| exp early discrete    | unequal, low           | 17.2       | 15.9            | 10.3             |
| exp late continuous   | equal                  | 17.3       | 16.4            | 11.0             |
| exp late discrete     | equal                  | 19.1       | 17.8            | 12.3             |
| exp late continuous   | unequal, high          | 13.5       | 12.9            | 7.2              |
| exp late discrete     | unequal, high          | 14.3       | 13.4            | 7.9              |
| exp late continuous   | unequal, low           | 16.8       | 15.9            | 10.9             |
| exp late discrete     | unequal, low           | 19.6       | 18.2            | 11.7             |
| exp prop continuous   | equal                  | 15.2       | 14.2            | 9.9              |
| exp prop discrete     | equal                  | 17.0       | 16.2            | 9.6              |
| exp prop continuous   | unequal, high          | 12.5       | 11.9            | 7.7              |
| exp prop discrete     | unequal, high          | 15.2       | 14.3            | 8.6              |
| exp prop continuous   | unequal, low           | 14.7       | 13.8            | 10.1             |
| exp prop discrete     | unequal, low           | 17.9       | 16.4            | 10.4             |
| logn continuous       | equal                  | 36.7       | 35.6            | 18.5             |
| logn discrete         | equal                  | 40.4       | 39.4            | 19.0             |
| logn continuous       | unequal, high          | 23.9       | 23.1            | 8.0              |
| logn discrete         | unequal, high          | 26.1       | 25.5            | 7.6              |
| logn continuous       | unequal, low           | 40.6       | 39.5            | 18.1             |
| logn discrete         | unequal, low           | 45.8       | 45.2            | 20.6             |
| pwExp continuous      | equal                  | 13.1       | 12.8            | 8.9              |
| pwExp discrete        | equal                  | 15.4       | 14.6            | 10.2             |
| pwExp continuous      | unequal, high          | 12.3       | 11.4            | 6.6              |
| pwExp discrete        | unequal, high          | 12.8       | 12.0            | 7.5              |
| pwExp continuous      | unequal, low           | 14.1       | 13.0            | 8.9              |
| pwExp discrete        | unequal, low           | 15.6       | 14.7            | 9.4              |
| Weib late continuous  | equal                  | 41.8       | 40.2            | 22.0             |
| Weib late discrete    | equal                  | 48.9       | 46.9            | 26.1             |
| Weib late continuous  | unequal, high          | 28.5       | 26.7            | 10.8             |
| Weib late discrete    | unequal, high          | 31.7       | 30.3            | 10.5             |
| Weib late continuous  | unequal, low           | 47.4       | 45.8            | 24.6             |
| Weib late discrete    | unequal, low           | 55.5       | 54.2            | 27.2             |
| Weib prop continuous  | equal                  | 36.9       | 35.7            | 18.9             |
| Weib prop discrete    | equal                  | 42.0       | 41.1            | 19.6             |
| Weib prop continuous  | unequal, high          | 25.7       | 25.0            | 10.4             |
| Weib prop discrete    | unequal, high          | 29.9       | 28.4            | 9.8              |
| Weib prop continuous  | unequal, low           | 41.8       | 40.5            | 19.5             |
| Weib prop discrete    | unequal, low           | 48.7       | 47.6            | 21.6             |
| Weib scale continuous | equal                  | 25.3       | 24.2            | 12.4             |
| Weib scale discrete   | equal                  | 28.6       | 27.7            | 12.8             |
| Weib scale continuous | unequal, high          | 20.0       | 19.2            | 8.0              |
| Weib scale discrete   | unequal, high          | 21.6       | 20.8            | 7.0              |
| Weib scale continuous | unequal, low           | 25.6       | 24.8            | 11.1             |
| Weib scale discrete   | unequal, low           | 30.1       | 29.2            | 12.3             |
| Weib shape continuous | equal                  | 14.6       | 13.9            | 7.3              |
| Weib shape discrete   | equal                  | 17.7       | 16.8            | 7.2              |
| Weib shape continuous | unequal, high          | 15.9       | 15.0            | 6.9              |
| Weib shape discrete   | unequal, high          | 17.2       | 17.0            | 6.6              |
| Weib shape continuous | unequal, low           | 14.2       | 13.8            | 7.0              |
| Weib shape discrete   | unequal, low           | 17.8       | 17.2            | 7.5              |

Table S30: Rejection rates in percent for the Dunnett-type contrast matrix with  $\delta = 1.5$  and unbalanced small sample sizes.

| Distribution          | Censoring distribution | asymptotic | asymptotic_bonf | permutation_bonf |
|-----------------------|------------------------|------------|-----------------|------------------|
| exp early continuous  | equal                  | 11.8       | 11.4            | 4.2              |
| exp early discrete    | equal                  | 11.3       | 10.8            | 3.1              |
| exp early continuous  | unequal, high          | 13.2       | 12.8            | 3.6              |
| exp early discrete    | unequal, high          | 16.0       | 15.6            | 4.0              |
| exp early continuous  | unequal, low           | 12.0       | 11.7            | 3.8              |
| exp early discrete    | unequal, low           | 12.3       | 11.6            | 3.0              |
| exp late continuous   | equal                  | 11.9       | 10.9            | 3.8              |
| exp late discrete     | equal                  | 11.7       | 11.1            | 3.1              |
| exp late continuous   | unequal, high          | 12.9       | 12.5            | 3.5              |
| exp late discrete     | unequal, high          | 15.3       | 14.6            | 4.0              |
| exp late continuous   | unequal, low           | 11.8       | 11.3            | 3.9              |
| exp late discrete     | unequal, low           | 12.2       | 11.3            | 3.1              |
| exp prop continuous   | equal                  | 12.2       | 11.7            | 5.1              |
| exp prop discrete     | equal                  | 12.7       | 12.4            | 4.9              |
| exp prop continuous   | unequal, high          | 15.7       | 15.2            | 5.0              |
| exp prop discrete     | unequal, high          | 16.3       | 15.8            | 5.0              |
| exp prop continuous   | unequal, low           | 11.8       | 11.0            | 4.5              |
| exp prop discrete     | unequal, low           | 12.3       | 11.8            | 4.1              |
| logn continuous       | equal                  | 17.2       | 16.9            | 5.0              |
| logn discrete         | equal                  | 17.8       | 17.3            | 4.6              |
| logn continuous       | unequal, high          | 29.0       | 28.7            | 5.8              |
| logn discrete         | unequal, high          | 31.1       | 30.6            | 5.5              |
| logn continuous       | unequal, low           | 16.2       | 15.8            | 3.8              |
| logn discrete         | unequal, low           | 16.4       | 16.2            | 4.0              |
| pwExp continuous      | equal                  | 11.0       | 10.2            | 3.9              |
| pwExp discrete        | equal                  | 10.9       | 10.5            | 3.7              |
| pwExp continuous      | unequal, high          | 12.9       | 12.4            | 3.6              |
| pwExp discrete        | unequal, high          | 14.9       | 14.4            | 4.0              |
| pwExp continuous      | unequal, low           | 11.1       | 10.7            | 3.7              |
| pwExp discrete        | unequal, low           | 11.3       | 10.7            | 3.7              |
| Weib late continuous  | equal                  | 13.5       | 13.1            | 4.1              |
| Weib late discrete    | equal                  | 15.5       | 15.0            | 3.6              |
| Weib late continuous  | unequal, high          | 21.5       | 20.8            | 4.5              |
| Weib late discrete    | unequal, high          | 25.8       | 25.1            | 4.6              |
| Weib late continuous  | unequal, low           | 14.3       | 13.9            | 3.7              |
| Weib late discrete    | unequal, low           | 16.1       | 16.0            | 4.1              |
| Weib prop continuous  | equal                  | 14.0       | 13.6            | 4.1              |
| Weib prop discrete    | equal                  | 15.7       | 15.3            | 4.6              |
| Weib prop continuous  | unequal, high          | 22.6       | 21.8            | 4.8              |
| Weib prop discrete    | unequal, high          | 27.4       | 26.8            | 5.1              |
| Weib prop continuous  | unequal, low           | 13.7       | 13.3            | 3.5              |
| Weib prop discrete    | unequal, low           | 15.6       | 15.3            | 3.1              |
| Weib scale continuous | equal                  | 15.9       | 15.6            | 4.7              |
| Weib scale discrete   | equal                  | 18.3       | 18.2            | 5.0              |
| Weib scale continuous | unequal, high          | 26.9       | 26.6            | 4.4              |
| Weib scale discrete   | unequal, high          | 30.7       | 30.2            | 4.8              |
| Weib scale continuous | unequal, low           | 15.9       | 15.6            | 3.7              |
| Weib scale discrete   | unequal, low           | 17.1       | 16.8            | 3.3              |
| Weib shape continuous | equal                  | 23.1       | 22.8            | 6.8              |
| Weib shape discrete   | equal                  | 24.0       | 23.9            | 6.2              |
| Weib shape continuous | unequal, high          | 29.7       | 29.5            | 4.8              |
| Weib shape discrete   | unequal, high          | 34.5       | 34.3            | 6.0              |
| Weib shape continuous | unequal, low           | 24.1       | 23.9            | 5.7              |
| Weib shape discrete   | unequal, low           | 24.7       | 24.6            | 5.4              |

Table S31: Rejection rates in percent for the Tukey-type contrast matrix with  $\delta = 1.5$  and balanced large sample sizes.

| Distribution          | Censoring distribution | asymptotic | asymptotic_bonf | permutation_bonf |
|-----------------------|------------------------|------------|-----------------|------------------|
| exp early continuous  | equal                  | 100.0      | 100.0           | 100.0            |
| exp early discrete    | equal                  | 100.0      | 100.0           | 100.0            |
| exp early continuous  | unequal, high          | 100.0      | 100.0           | 100.0            |
| exp early discrete    | unequal, high          | 100.0      | 100.0           | 100.0            |
| exp early continuous  | unequal, low           | 100.0      | 100.0           | 100.0            |
| exp early discrete    | unequal, low           | 100.0      | 100.0           | 100.0            |
| exp late continuous   | equal                  | 100.0      | 100.0           | 100.0            |
| exp late discrete     | equal                  | 100.0      | 100.0           | 100.0            |
| exp late continuous   | unequal, high          | 100.0      | 100.0           | 100.0            |
| exp late discrete     | unequal, high          | 99.9       | 99.9            | 99.9             |
| exp late continuous   | unequal, low           | 100.0      | 100.0           | 100.0            |
| exp late discrete     | unequal, low           | 100.0      | 100.0           | 100.0            |
| exp prop continuous   | equal                  | 100.0      | 100.0           | 100.0            |
| exp prop discrete     | equal                  | 100.0      | 100.0           | 100.0            |
| exp prop continuous   | unequal, high          | 100.0      | 100.0           | 100.0            |
| exp prop discrete     | unequal, high          | 100.0      | 100.0           | 100.0            |
| exp prop continuous   | unequal, low           | 100.0      | 100.0           | 100.0            |
| exp prop discrete     | unequal, low           | 100.0      | 100.0           | 100.0            |
| logn continuous       | equal                  | 100.0      | 100.0           | 100.0            |
| logn discrete         | equal                  | 100.0      | 100.0           | 100.0            |
| logn continuous       | unequal, high          | 100.0      | 100.0           | 100.0            |
| logn discrete         | unequal, high          | 100.0      | 100.0           | 100.0            |
| logn continuous       | unequal, low           | 100.0      | 100.0           | 100.0            |
| logn discrete         | unequal, low           | 100.0      | 100.0           | 100.0            |
| pwExp continuous      | equal                  | 100.0      | 100.0           | 100.0            |
| pwExp discrete        | equal                  | 100.0      | 100.0           | 100.0            |
| pwExp continuous      | unequal, high          | 100.0      | 100.0           | 100.0            |
| pwExp discrete        | unequal, high          | 100.0      | 100.0           | 100.0            |
| pwExp continuous      | unequal, low           | 100.0      | 100.0           | 100.0            |
| pwExp discrete        | unequal, low           | 100.0      | 100.0           | 100.0            |
| Weib late continuous  | equal                  | 100.0      | 100.0           | 100.0            |
| Weib late discrete    | equal                  | 100.0      | 100.0           | 100.0            |
| Weib late continuous  | unequal, high          | 100.0      | 100.0           | 100.0            |
| Weib late discrete    | unequal, high          | 100.0      | 100.0           | 100.0            |
| Weib late continuous  | unequal, low           | 100.0      | 100.0           | 100.0            |
| Weib late discrete    | unequal, low           | 100.0      | 100.0           | 100.0            |
| Weib prop continuous  | equal                  | 100.0      | 100.0           | 100.0            |
| Weib prop discrete    | equal                  | 100.0      | 100.0           | 100.0            |
| Weib prop continuous  | unequal, high          | 100.0      | 100.0           | 100.0            |
| Weib prop discrete    | unequal, high          | 100.0      | 100.0           | 100.0            |
| Weib prop continuous  | unequal, low           | 100.0      | 100.0           | 100.0            |
| Weib prop discrete    | unequal, low           | 100.0      | 100.0           | 100.0            |
| Weib scale continuous | equal                  | 100.0      | 100.0           | 100.0            |
| Weib scale discrete   | equal                  | 100.0      | 100.0           | 100.0            |
| Weib scale continuous | unequal, high          | 100.0      | 100.0           | 100.0            |
| Weib scale discrete   | unequal, high          | 100.0      | 100.0           | 100.0            |
| Weib scale continuous | unequal, low           | 100.0      | 100.0           | 100.0            |
| Weib scale discrete   | unequal, low           | 100.0      | 100.0           | 100.0            |
| Weib shape continuous | equal                  | 100.0      | 100.0           | 100.0            |
| Weib shape discrete   | equal                  | 100.0      | 100.0           | 100.0            |
| Weib shape continuous | unequal, high          | 100.0      | 100.0           | 100.0            |
| Weib shape discrete   | unequal, high          | 100.0      | 100.0           | 100.0            |
| Weib shape continuous | unequal, low           | 100.0      | 100.0           | 100.0            |
| Weib shape discrete   | unequal, low           | 100.0      | 100.0           | 100.0            |

Table S32: Rejection rates in percent for the Tukey-type contrast matrix with  $\delta = 1.5$  and balanced medium sample sizes.

| Distribution          | Censoring distribution | asymptotic | asymptotic_bonf | permutation_bonf |
|-----------------------|------------------------|------------|-----------------|------------------|
| exp early continuous  | equal                  | 65.9       | 61.6            | 60.0             |
| exp early discrete    | equal                  | 74.4       | 70.4            | 67.7             |
| exp early continuous  | unequal, high          | 54.1       | 50.2            | 49.3             |
| exp early discrete    | unequal, high          | 59.9       | 55.5            | 53.8             |
| exp early continuous  | unequal, low           | 66.6       | 63.1            | 60.4             |
| exp early discrete    | unequal, low           | 74.0       | 69.9            | 67.0             |
| exp late continuous   | equal                  | 72.1       | 67.9            | 66.4             |
| exp late discrete     | equal                  | 79.5       | 75.9            | 74.9             |
| exp late continuous   | unequal, high          | 59.0       | 54.5            | 52.8             |
| exp late discrete     | unequal, high          | 63.6       | 58.9            | 57.9             |
| exp late continuous   | unequal, low           | 73.4       | 70.1            | 67.0             |
| exp late discrete     | unequal, low           | 79.6       | 76.0            | 73.8             |
| exp prop continuous   | equal                  | 66.1       | 62.0            | 61.2             |
| exp prop discrete     | equal                  | 74.4       | 71.0            | 68.7             |
| exp prop continuous   | unequal, high          | 56.0       | 51.7            | 51.1             |
| exp prop discrete     | unequal, high          | 61.7       | 57.3            | 54.5             |
| exp prop continuous   | unequal, low           | 66.5       | 63.0            | 60.0             |
| exp prop discrete     | unequal, low           | 73.9       | 70.0            | 67.0             |
| logn continuous       | equal                  | 99.3       | 99.2            | 98.8             |
| logn discrete         | equal                  | 99.8       | 99.6            | 99.5             |
| logn continuous       | unequal, high          | 89.8       | 87.8            | 85.6             |
| logn discrete         | unequal, high          | 94.4       | 92.9            | 92.2             |
| logn continuous       | unequal, low           | 99.4       | 99.2            | 98.9             |
| logn discrete         | unequal, low           | 99.9       | 99.8            | 99.7             |
| pwExp continuous      | equal                  | 63.8       | 59.1            | 59.3             |
| pwExp discrete        | equal                  | 70.1       | 66.5            | 66.0             |
| pwExp continuous      | unequal, high          | 51.8       | 48.9            | 48.4             |
| pwExp discrete        | unequal, high          | 59.0       | 55.2            | 52.4             |
| pwExp continuous      | unequal, low           | 63.4       | 59.2            | 57.2             |
| pwExp discrete        | unequal, low           | 69.9       | 66.5            | 64.7             |
| Weib late continuous  | equal                  | 99.5       | 99.3            | 99.2             |
| Weib late discrete    | equal                  | 99.3       | 98.9            | 98.6             |
| Weib late continuous  | unequal, high          | 93.6       | 92.2            | 90.4             |
| Weib late discrete    | unequal, high          | 95.8       | 94.4            | 92.7             |
| Weib late continuous  | unequal, low           | 99.6       | 99.5            | 99.4             |
| Weib late discrete    | unequal, low           | 99.3       | 99.3            | 99.0             |
| Weib prop continuous  | equal                  | 99.1       | 98.7            | 98.5             |
| Weib prop discrete    | equal                  | 99.9       | 99.8            | 99.7             |
| Weib prop continuous  | unequal, high          | 92.8       | 90.8            | 88.6             |
| Weib prop discrete    | unequal, high          | 95.8       | 94.9            | 93.9             |
| Weib prop continuous  | unequal, low           | 99.5       | 99.0            | 99.0             |
| Weib prop discrete    | unequal, low           | 100.0      | 99.9            | 99.8             |
| Weib scale continuous | equal                  | 95.1       | 94.2            | 93.6             |
| Weib scale discrete   | equal                  | 97.8       | 97.2            | 96.5             |
| Weib scale continuous | unequal, high          | 84.5       | 81.6            | 80.8             |
| Weib scale discrete   | unequal, high          | 91.2       | 88.7            | 87.2             |
| Weib scale continuous | unequal, low           | 95.7       | 95.1            | 94.2             |
| Weib scale discrete   | unequal, low           | 98.7       | 98.4            | 98.1             |
| Weib shape continuous | equal                  | 84.5       | 81.0            | 80.2             |
| Weib shape discrete   | equal                  | 91.5       | 89.4            | 88.0             |
| Weib shape continuous | unequal, high          | 75.0       | 72.2            | 71.2             |
| Weib shape discrete   | unequal, high          | 81.7       | 79.8            | 77.6             |
| Weib shape continuous | unequal, low           | 83.4       | 81.3            | 80.4             |
| Weib shape discrete   | unequal, low           | 91.4       | 88.6            | 88.8             |

Table S33: Rejection rates in percent for the Tukey-type contrast matrix with  $\delta = 1.5$  and balanced small sample sizes.

| Distribution          | Censoring distribution | asymptotic | asymptotic_bonf | permutation_bonf |
|-----------------------|------------------------|------------|-----------------|------------------|
| exp early continuous  | equal                  | 14.9       | 12.5            | 9.9              |
| exp early discrete    | equal                  | 14.3       | 12.4            | 10.3             |
| exp early continuous  | unequal, high          | 16.4       | 13.5            | 11.4             |
| exp early discrete    | unequal, high          | 13.5       | 11.8            | 9.8              |
| exp early continuous  | unequal, low           | 16.3       | 14.5            | 10.3             |
| exp early discrete    | unequal, low           | 14.8       | 12.2            | 10.9             |
| exp late continuous   | equal                  | 17.4       | 15.7            | 12.7             |
| exp late discrete     | equal                  | 18.0       | 15.9            | 14.5             |
| exp late continuous   | unequal, high          | 17.8       | 15.3            | 10.6             |
| exp late discrete     | unequal, high          | 17.7       | 15.4            | 10.9             |
| exp late continuous   | unequal, low           | 18.1       | 16.7            | 12.9             |
| exp late discrete     | unequal, low           | 20.0       | 18.2            | 14.0             |
| exp prop continuous   | equal                  | 14.2       | 12.5            | 10.9             |
| exp prop discrete     | equal                  | 15.7       | 14.1            | 12.1             |
| exp prop continuous   | unequal, high          | 14.0       | 12.5            | 10.6             |
| exp prop discrete     | unequal, high          | 15.6       | 13.4            | 10.0             |
| exp prop continuous   | unequal, low           | 14.6       | 12.7            | 10.0             |
| exp prop discrete     | unequal, low           | 16.9       | 14.9            | 12.3             |
| logn continuous       | equal                  | 32.8       | 29.5            | 26.8             |
| logn discrete         | equal                  | 38.7       | 34.6            | 31.6             |
| logn continuous       | unequal, high          | 27.0       | 24.0            | 19.5             |
| logn discrete         | unequal, high          | 30.2       | 27.2            | 22.2             |
| logn continuous       | unequal, low           | 36.2       | 32.6            | 28.1             |
| logn discrete         | unequal, low           | 43.1       | 38.7            | 34.9             |
| pwExp continuous      | equal                  | 13.5       | 11.4            | 9.7              |
| pwExp discrete        | equal                  | 14.9       | 12.5            | 10.4             |
| pwExp continuous      | unequal, high          | 15.1       | 13.0            | 9.4              |
| pwExp discrete        | unequal, high          | 16.6       | 14.0            | 11.3             |
| pwExp continuous      | unequal, low           | 14.6       | 13.3            | 9.9              |
| pwExp discrete        | unequal, low           | 16.9       | 14.3            | 11.0             |
| Weib late continuous  | equal                  | 34.9       | 31.9            | 26.9             |
| Weib late discrete    | equal                  | 40.0       | 36.1            | 30.7             |
| Weib late continuous  | unequal, high          | 29.0       | 25.6            | 19.4             |
| Weib late discrete    | unequal, high          | 30.7       | 28.1            | 22.1             |
| Weib late continuous  | unequal, low           | 40.4       | 37.0            | 30.4             |
| Weib late discrete    | unequal, low           | 46.3       | 42.9            | 37.5             |
| Weib prop continuous  | equal                  | 30.9       | 28.7            | 25.0             |
| Weib prop discrete    | equal                  | 36.4       | 32.0            | 29.6             |
| Weib prop continuous  | unequal, high          | 26.8       | 23.7            | 17.9             |
| Weib prop discrete    | unequal, high          | 27.8       | 25.5            | 19.9             |
| Weib prop continuous  | unequal, low           | 36.6       | 32.4            | 27.9             |
| Weib prop discrete    | unequal, low           | 42.6       | 39.1            | 33.6             |
| Weib scale continuous | equal                  | 22.2       | 18.9            | 16.9             |
| Weib scale discrete   | equal                  | 25.3       | 22.0            | 19.0             |
| Weib scale continuous | unequal, high          | 20.2       | 16.9            | 14.1             |
| Weib scale discrete   | unequal, high          | 20.8       | 17.8            | 14.8             |
| Weib scale continuous | unequal, low           | 23.6       | 21.0            | 18.1             |
| Weib scale discrete   | unequal, low           | 29.0       | 25.6            | 22.2             |
| Weib shape continuous | equal                  | 13.4       | 11.2            | 11.6             |
| Weib shape discrete   | equal                  | 15.1       | 13.0            | 12.2             |
| Weib shape continuous | unequal, high          | 14.9       | 12.8            | 10.9             |
| Weib shape discrete   | unequal, high          | 16.0       | 13.8            | 12.3             |
| Weib shape continuous | unequal, low           | 15.4       | 13.2            | 12.4             |
| Weib shape discrete   | unequal, low           | 18.0       | 15.6            | 14.2             |



Table S34: Rejection rates in percent for the Tukey-type contrast matrix with  $\delta = 1.5$  and unbalanced large sample sizes.

| Distribution          | Censoring distribution | asymptotic | asymptotic_bonf | permutation_bonf |
|-----------------------|------------------------|------------|-----------------|------------------|
| exp early continuous  | equal                  | 92.2       | 89.3            | 85.1             |
| exp early discrete    | equal                  | 95.6       | 93.7            | 91.7             |
| exp early continuous  | unequal, high          | 85.1       | 80.7            | 76.9             |
| exp early discrete    | unequal, high          | 88.3       | 85.5            | 81.1             |
| exp early continuous  | unequal, low           | 91.7       | 89.5            | 86.6             |
| exp early discrete    | unequal, low           | 96.1       | 93.7            | 92.5             |
| exp late continuous   | equal                  | 98.4       | 95.9            | 94.3             |
| exp late discrete     | equal                  | 99.0       | 98.2            | 97.2             |
| exp late continuous   | unequal, high          | 91.7       | 87.5            | 83.9             |
| exp late discrete     | unequal, high          | 95.0       | 92.1            | 88.3             |
| exp late continuous   | unequal, low           | 98.3       | 96.9            | 96.4             |
| exp late discrete     | unequal, low           | 99.6       | 99.0            | 98.3             |
| exp prop continuous   | equal                  | 95.9       | 93.1            | 91.7             |
| exp prop discrete     | equal                  | 98.3       | 96.9            | 95.0             |
| exp prop continuous   | unequal, high          | 88.6       | 84.6            | 80.3             |
| exp prop discrete     | unequal, high          | 91.3       | 88.0            | 84.9             |
| exp prop continuous   | unequal, low           | 96.2       | 93.5            | 92.7             |
| exp prop discrete     | unequal, low           | 98.9       | 97.6            | 96.8             |
| logn continuous       | equal                  | 100.0      | 100.0           | 100.0            |
| logn discrete         | equal                  | 100.0      | 100.0           | 100.0            |
| logn continuous       | unequal, high          | 99.9       | 99.8            | 99.2             |
| logn discrete         | unequal, high          | 99.9       | 99.9            | 99.8             |
| logn continuous       | unequal, low           | 100.0      | 100.0           | 100.0            |
| logn discrete         | unequal, low           | 100.0      | 100.0           | 100.0            |
| pwExp continuous      | equal                  | 90.4       | 87.2            | 85.8             |
| pwExp discrete        | equal                  | 95.5       | 92.9            | 91.2             |
| pwExp continuous      | unequal, high          | 84.6       | 81.5            | 77.6             |
| pwExp discrete        | unequal, high          | 88.8       | 84.6            | 81.7             |
| pwExp continuous      | unequal, low           | 91.0       | 87.5            | 86.3             |
| pwExp discrete        | unequal, low           | 95.3       | 93.7            | 91.6             |
| Weib late continuous  | equal                  | 100.0      | 100.0           | 100.0            |
| Weib late discrete    | equal                  | 99.7       | 99.7            | 99.6             |
| Weib late continuous  | unequal, high          | 100.0      | 100.0           | 100.0            |
| Weib late discrete    | unequal, high          | 99.1       | 98.7            | 98.5             |
| Weib late continuous  | unequal, low           | 100.0      | 100.0           | 100.0            |
| Weib late discrete    | unequal, low           | 99.9       | 99.9            | 99.9             |
| Weib prop continuous  | equal                  | 100.0      | 100.0           | 100.0            |
| Weib prop discrete    | equal                  | 100.0      | 100.0           | 100.0            |
| Weib prop continuous  | unequal, high          | 99.9       | 99.9            | 99.9             |
| Weib prop discrete    | unequal, high          | 100.0      | 100.0           | 99.8             |
| Weib prop continuous  | unequal, low           | 100.0      | 100.0           | 100.0            |
| Weib prop discrete    | unequal, low           | 100.0      | 100.0           | 100.0            |
| Weib scale continuous | equal                  | 100.0      | 100.0           | 99.9             |
| Weib scale discrete   | equal                  | 100.0      | 100.0           | 99.9             |
| Weib scale continuous | unequal, high          | 99.0       | 98.6            | 97.0             |
| Weib scale discrete   | unequal, high          | 99.7       | 99.3            | 98.5             |
| Weib scale continuous | unequal, low           | 100.0      | 99.9            | 99.8             |
| Weib scale discrete   | unequal, low           | 100.0      | 100.0           | 100.0            |
| Weib shape continuous | equal                  | 97.7       | 96.5            | 95.0             |
| Weib shape discrete   | equal                  | 99.4       | 99.0            | 98.3             |
| Weib shape continuous | unequal, high          | 95.9       | 94.3            | 89.3             |
| Weib shape discrete   | unequal, high          | 97.6       | 96.6            | 93.1             |
| Weib shape continuous | unequal, low           | 97.9       | 97.2            | 95.1             |
| Weib shape discrete   | unequal, low           | 99.3       | 99.0            | 98.1             |

Table S35: Rejection rates in percent for the Tukey-type contrast matrix with  $\delta = 1.5$  and unbalanced medium sample sizes.

| Distribution          | Censoring distribution | asymptotic | asymptotic_bonf | permutation_bonf |
|-----------------------|------------------------|------------|-----------------|------------------|
| exp early continuous  | equal                  | 16.1       | 12.9            | 9.2              |
| exp early discrete    | equal                  | 19.3       | 15.6            | 10.7             |
| exp early continuous  | unequal, high          | 13.8       | 11.4            | 6.7              |
| exp early discrete    | unequal, high          | 15.1       | 12.4            | 6.6              |
| exp early continuous  | unequal, low           | 15.7       | 12.9            | 8.9              |
| exp early discrete    | unequal, low           | 19.1       | 15.4            | 11.5             |
| exp late continuous   | equal                  | 19.4       | 15.3            | 11.0             |
| exp late discrete     | equal                  | 21.6       | 18.1            | 11.8             |
| exp late continuous   | unequal, high          | 16.0       | 12.3            | 7.3              |
| exp late discrete     | unequal, high          | 16.8       | 13.8            | 7.5              |
| exp late continuous   | unequal, low           | 18.5       | 15.8            | 10.1             |
| exp late discrete     | unequal, low           | 22.5       | 17.8            | 12.8             |
| exp prop continuous   | equal                  | 15.8       | 12.8            | 8.9              |
| exp prop discrete     | equal                  | 18.6       | 15.6            | 10.1             |
| exp prop continuous   | unequal, high          | 15.0       | 12.7            | 8.0              |
| exp prop discrete     | unequal, high          | 16.3       | 14.2            | 8.6              |
| exp prop continuous   | unequal, low           | 16.8       | 13.2            | 9.5              |
| exp prop discrete     | unequal, low           | 19.7       | 16.5            | 9.6              |
| logn continuous       | equal                  | 42.0       | 36.2            | 19.7             |
| logn discrete         | equal                  | 46.3       | 39.8            | 23.1             |
| logn continuous       | unequal, high          | 28.3       | 24.0            | 8.5              |
| logn discrete         | unequal, high          | 30.4       | 27.3            | 9.7              |
| logn continuous       | unequal, low           | 45.5       | 40.7            | 20.6             |
| logn discrete         | unequal, low           | 52.2       | 46.9            | 24.5             |
| pwExp continuous      | equal                  | 15.3       | 11.9            | 8.3              |
| pwExp discrete        | equal                  | 17.9       | 14.4            | 9.7              |
| pwExp continuous      | unequal, high          | 13.6       | 11.9            | 6.2              |
| pwExp discrete        | unequal, high          | 14.7       | 12.0            | 6.4              |
| pwExp continuous      | unequal, low           | 14.5       | 12.0            | 8.7              |
| pwExp discrete        | unequal, low           | 17.3       | 13.7            | 9.3              |
| Weib late continuous  | equal                  | 48.5       | 40.7            | 23.9             |
| Weib late discrete    | equal                  | 54.5       | 48.0            | 27.5             |
| Weib late continuous  | unequal, high          | 31.1       | 26.5            | 11.2             |
| Weib late discrete    | unequal, high          | 36.3       | 31.2            | 11.7             |
| Weib late continuous  | unequal, low           | 54.5       | 49.3            | 25.0             |
| Weib late discrete    | unequal, low           | 61.4       | 55.9            | 30.7             |
| Weib prop continuous  | equal                  | 42.3       | 36.1            | 20.2             |
| Weib prop discrete    | equal                  | 47.1       | 39.8            | 21.4             |
| Weib prop continuous  | unequal, high          | 29.3       | 24.6            | 10.9             |
| Weib prop discrete    | unequal, high          | 33.0       | 27.4            | 10.4             |
| Weib prop continuous  | unequal, low           | 47.0       | 40.4            | 20.2             |
| Weib prop discrete    | unequal, low           | 55.0       | 48.4            | 24.6             |
| Weib scale continuous | equal                  | 27.9       | 23.4            | 12.4             |
| Weib scale discrete   | equal                  | 31.6       | 27.0            | 14.4             |
| Weib scale continuous | unequal, high          | 21.7       | 17.7            | 7.9              |
| Weib scale discrete   | unequal, high          | 23.7       | 19.4            | 8.1              |
| Weib scale continuous | unequal, low           | 27.0       | 21.6            | 11.7             |
| Weib scale discrete   | unequal, low           | 34.7       | 27.7            | 12.1             |
| Weib shape continuous | equal                  | 16.1       | 12.9            | 6.9              |
| Weib shape discrete   | equal                  | 19.2       | 15.8            | 8.3              |
| Weib shape continuous | unequal, high          | 16.6       | 13.3            | 7.0              |
| Weib shape discrete   | unequal, high          | 17.4       | 14.9            | 6.0              |
| Weib shape continuous | unequal, low           | 16.5       | 12.4            | 6.4              |
| Weib shape discrete   | unequal, low           | 19.3       | 15.6            | 7.6              |

Table S36: Rejection rates in percent for the Tukey-type contrast matrix with  $\delta = 1.5$  and unbalanced small sample sizes.

| Distribution          | Censoring distribution | asymptotic | asymptotic_bonf | permutation_bonf |
|-----------------------|------------------------|------------|-----------------|------------------|
| exp early continuous  | equal                  | 11.5       | 10.1            | 3.4              |
| exp early discrete    | equal                  | 11.0       | 9.6             | 3.2              |
| exp early continuous  | unequal, high          | 13.2       | 11.8            | 3.6              |
| exp early discrete    | unequal, high          | 15.7       | 14.5            | 3.9              |
| exp early continuous  | unequal, low           | 11.1       | 10.0            | 2.2              |
| exp early discrete    | unequal, low           | 11.3       | 10.3            | 2.8              |
| exp late continuous   | equal                  | 11.9       | 9.4             | 2.5              |
| exp late discrete     | equal                  | 11.8       | 10.4            | 2.6              |
| exp late continuous   | unequal, high          | 13.0       | 11.9            | 3.3              |
| exp late discrete     | unequal, high          | 14.7       | 13.4            | 3.4              |
| exp late continuous   | unequal, low           | 11.1       | 9.6             | 2.0              |
| exp late discrete     | unequal, low           | 12.1       | 10.3            | 2.2              |
| exp prop continuous   | equal                  | 12.4       | 11.1            | 3.4              |
| exp prop discrete     | equal                  | 13.3       | 11.0            | 3.8              |
| exp prop continuous   | unequal, high          | 15.4       | 13.6            | 4.3              |
| exp prop discrete     | unequal, high          | 16.1       | 14.7            | 3.6              |
| exp prop continuous   | unequal, low           | 11.4       | 9.6             | 3.5              |
| exp prop discrete     | unequal, low           | 12.1       | 10.1            | 2.9              |
| logn continuous       | equal                  | 16.3       | 14.8            | 3.9              |
| logn discrete         | equal                  | 18.1       | 16.4            | 3.6              |
| logn continuous       | unequal, high          | 28.5       | 26.6            | 4.7              |
| logn discrete         | unequal, high          | 30.5       | 27.7            | 5.0              |
| logn continuous       | unequal, low           | 15.1       | 13.0            | 3.3              |
| logn discrete         | unequal, low           | 15.8       | 13.5            | 2.9              |
| pwExp continuous      | equal                  | 11.7       | 9.6             | 2.9              |
| pwExp discrete        | equal                  | 11.2       | 9.7             | 2.6              |
| pwExp continuous      | unequal, high          | 13.4       | 12.0            | 3.1              |
| pwExp discrete        | unequal, high          | 14.5       | 13.4            | 3.5              |
| pwExp continuous      | unequal, low           | 10.6       | 9.3             | 2.0              |
| pwExp discrete        | unequal, low           | 11.3       | 9.9             | 2.5              |
| Weib late continuous  | equal                  | 14.2       | 12.9            | 3.5              |
| Weib late discrete    | equal                  | 16.6       | 14.4            | 3.3              |
| Weib late continuous  | unequal, high          | 20.2       | 18.2            | 4.8              |
| Weib late discrete    | unequal, high          | 24.9       | 22.3            | 4.4              |
| Weib late continuous  | unequal, low           | 14.5       | 12.7            | 2.5              |
| Weib late discrete    | unequal, low           | 16.2       | 14.1            | 3.3              |
| Weib prop continuous  | equal                  | 14.5       | 13.3            | 3.5              |
| Weib prop discrete    | equal                  | 17.0       | 15.0            | 3.4              |
| Weib prop continuous  | unequal, high          | 21.3       | 18.5            | 4.4              |
| Weib prop discrete    | unequal, high          | 25.7       | 22.8            | 4.1              |
| Weib prop continuous  | unequal, low           | 14.2       | 12.6            | 2.4              |
| Weib prop discrete    | unequal, low           | 15.6       | 13.8            | 3.2              |
| Weib scale continuous | equal                  | 15.9       | 15.3            | 3.5              |
| Weib scale discrete   | equal                  | 18.6       | 17.3            | 3.8              |
| Weib scale continuous | unequal, high          | 26.4       | 24.4            | 4.4              |
| Weib scale discrete   | unequal, high          | 29.3       | 27.1            | 4.1              |
| Weib scale continuous | unequal, low           | 15.6       | 13.8            | 2.8              |
| Weib scale discrete   | unequal, low           | 17.3       | 15.3            | 3.4              |
| Weib shape continuous | equal                  | 23.2       | 22.2            | 6.6              |
| Weib shape discrete   | equal                  | 24.3       | 22.9            | 5.6              |
| Weib shape continuous | unequal, high          | 28.8       | 26.7            | 4.6              |
| Weib shape discrete   | unequal, high          | 33.5       | 31.3            | 4.7              |
| Weib shape continuous | unequal, low           | 23.6       | 22.1            | 5.3              |
| Weib shape discrete   | unequal, low           | 24.5       | 22.8            | 5.5              |

Table S37: Rejection rates in percent for the 2-by-2 design with  $\delta = 1.5$  and balanced large sample sizes under equal censoring.

| Distribution          | Method           | $\mathcal{H}_{0,4}$ | $\mathcal{H}_{0,5}$ | $\mathcal{H}_{0,6}$ | $\mathcal{H}_{0,1}$ | $\mathcal{H}_{0,2}$ | $\mathcal{H}_{0,3}$ | $\mathcal{H}_{0,7}$ | $\mathcal{H}_{0,8}$ | $\mathcal{H}_{0,9}$ |
|-----------------------|------------------|---------------------|---------------------|---------------------|---------------------|---------------------|---------------------|---------------------|---------------------|---------------------|
| exp early continuous  | asymptotic       | 50.5                | 32.8                | 69.2                | 49.6                | 33.6                | 72.1                | 49.1                | 32.4                | 69.5                |
|                       | asymptotic_bonf  | 49.9                | 32.0                | 68.6                | 48.9                | 33.0                | 71.4                | 48.3                | 31.8                | 69.2                |
|                       | permutation_bonf | 50.0                | 31.9                | 68.7                | 48.0                | 32.3                | 70.2                | 48.5                | 31.9                | 69.6                |
| exp early discrete    | asymptotic       | 59.1                | 37.9                | 74.8                | 56.4                | 38.0                | 77.0                | 55.4                | 37.8                | 77.4                |
|                       | asymptotic_bonf  | 58.0                | 37.7                | 74.1                | 55.8                | 37.3                | 76.7                | 55.1                | 37.0                | 77.1                |
|                       | permutation_bonf | 58.3                | 37.0                | 73.9                | 55.2                | 37.0                | 76.0                | 54.7                | 37.7                | 76.1                |
| exp late continuous   | asymptotic       | 52.8                | 34.9                | 72.2                | 52.5                | 34.6                | 73.9                | 50.9                | 33.5                | 74.0                |
|                       | asymptotic_bonf  | 52.3                | 33.9                | 71.9                | 51.4                | 33.4                | 73.5                | 49.7                | 32.7                | 72.8                |
|                       | permutation_bonf | 52.3                | 33.0                | 70.9                | 50.8                | 33.1                | 72.7                | 49.7                | 32.7                | 72.6                |
| exp late discrete     | asymptotic       | 61.5                | 41.2                | 78.7                | 59.6                | 40.5                | 79.8                | 59.0                | 39.7                | 79.7                |
|                       | asymptotic_bonf  | 60.6                | 40.4                | 78.2                | 59.1                | 39.7                | 79.4                | 58.3                | 39.3                | 79.0                |
|                       | permutation_bonf | 60.3                | 39.7                | 77.7                | 57.8                | 38.2                | 79.1                | 57.0                | 38.4                | 78.1                |
| exp prop continuous   | asymptotic       | 51.1                | 35.6                | 70.1                | 51.3                | 34.6                | 71.0                | 51.1                | 36.1                | 73.0                |
|                       | asymptotic_bonf  | 50.0                | 35.2                | 69.5                | 50.4                | 33.7                | 70.5                | 50.1                | 35.2                | 72.3                |
|                       | permutation_bonf | 51.2                | 34.5                | 69.3                | 50.1                | 34.7                | 69.6                | 49.8                | 34.7                | 72.1                |
| exp prop discrete     | asymptotic       | 57.8                | 41.2                | 77.2                | 57.2                | 39.4                | 77.9                | 58.2                | 40.7                | 78.7                |
|                       | asymptotic_bonf  | 57.2                | 40.4                | 76.7                | 56.4                | 38.7                | 77.2                | 57.2                | 40.4                | 78.3                |
|                       | permutation_bonf | 56.7                | 40.1                | 76.3                | 57.5                | 38.1                | 76.7                | 58.0                | 39.3                | 77.6                |
| logn continuous       | asymptotic       | 95.6                | 83.0                | 99.3                | 95.3                | 84.0                | 99.3                | 95.7                | 84.2                | 99.0                |
|                       | asymptotic_bonf  | 95.4                | 82.9                | 99.2                | 95.2                | 83.7                | 99.3                | 95.6                | 83.7                | 99.0                |
|                       | permutation_bonf | 95.1                | 82.4                | 99.4                | 95.2                | 83.5                | 99.6                | 95.4                | 83.1                | 99.0                |
| logn discrete         | asymptotic       | 97.4                | 89.1                | 99.8                | 98.1                | 90.2                | 99.8                | 97.3                | 90.1                | 99.9                |
|                       | asymptotic_bonf  | 97.4                | 89.1                | 99.8                | 98.0                | 89.8                | 99.8                | 97.3                | 89.8                | 99.8                |
|                       | permutation_bonf | 97.7                | 88.8                | 99.7                | 97.8                | 90.3                | 99.8                | 97.1                | 89.7                | 99.7                |
| pwExp continuous      | asymptotic       | 51.2                | 33.2                | 69.4                | 49.4                | 32.4                | 71.3                | 48.4                | 31.8                | 70.5                |
|                       | asymptotic_bonf  | 50.2                | 32.6                | 68.6                | 49.1                | 32.1                | 70.9                | 48.0                | 31.2                | 70.2                |
|                       | permutation_bonf | 48.7                | 32.3                | 68.7                | 47.2                | 32.3                | 70.3                | 48.4                | 31.2                | 68.7                |
| pwExp discrete        | asymptotic       | 57.8                | 39.4                | 76.6                | 57.6                | 38.4                | 77.5                | 54.6                | 37.9                | 76.0                |
|                       | asymptotic_bonf  | 57.1                | 39.0                | 76.2                | 57.0                | 37.7                | 77.1                | 53.9                | 37.5                | 75.7                |
|                       | permutation_bonf | 56.7                | 38.2                | 75.6                | 56.1                | 38.1                | 75.7                | 54.1                | 38.0                | 76.0                |
| Weib late continuous  | asymptotic       | 95.4                | 80.7                | 99.3                | 95.0                | 81.4                | 99.4                | 94.4                | 83.5                | 99.0                |
|                       | asymptotic_bonf  | 95.1                | 80.0                | 99.3                | 94.8                | 81.4                | 99.4                | 94.0                | 82.7                | 99.0                |
|                       | permutation_bonf | 95.0                | 80.2                | 99.2                | 94.7                | 80.2                | 99.1                | 93.8                | 82.5                | 98.9                |
| Weib late discrete    | asymptotic       | 97.6                | 88.1                | 99.7                | 97.9                | 89.7                | 100.0               | 98.0                | 88.9                | 99.6                |
|                       | asymptotic_bonf  | 97.5                | 87.8                | 99.7                | 97.9                | 89.4                | 100.0               | 98.0                | 88.6                | 99.6                |
|                       | permutation_bonf | 97.4                | 87.6                | 99.9                | 97.7                | 88.7                | 100.0               | 97.7                | 88.2                | 99.6                |
| Weib prop continuous  | asymptotic       | 94.3                | 80.1                | 99.1                | 94.8                | 80.2                | 99.0                | 93.9                | 82.2                | 99.0                |
|                       | asymptotic_bonf  | 94.3                | 79.6                | 99.0                | 94.8                | 79.8                | 99.0                | 93.7                | 81.9                | 99.0                |
|                       | permutation_bonf | 93.8                | 79.5                | 98.8                | 94.5                | 79.7                | 99.0                | 93.2                | 82.0                | 99.0                |
| Weib prop discrete    | asymptotic       | 97.1                | 86.8                | 99.8                | 97.7                | 88.4                | 99.9                | 97.3                | 87.7                | 99.6                |
|                       | asymptotic_bonf  | 97.0                | 86.7                | 99.8                | 97.7                | 88.2                | 99.8                | 97.2                | 87.5                | 99.6                |
|                       | permutation_bonf | 97.0                | 86.3                | 99.9                | 97.4                | 87.8                | 99.9                | 97.1                | 86.9                | 99.6                |
| Weib scale continuous | asymptotic       | 92.3                | 76.6                | 98.2                | 92.5                | 76.7                | 98.1                | 91.3                | 78.2                | 98.4                |
|                       | asymptotic_bonf  | 92.3                | 76.4                | 98.1                | 92.3                | 76.6                | 98.0                | 91.0                | 77.9                | 98.4                |
|                       | permutation_bonf | 91.8                | 75.6                | 97.9                | 92.0                | 76.4                | 98.1                | 90.8                | 77.8                | 98.6                |
| Weib scale discrete   | asymptotic       | 95.9                | 84.6                | 99.4                | 96.9                | 85.6                | 99.5                | 95.9                | 85.1                | 99.1                |
|                       | asymptotic_bonf  | 95.8                | 84.3                | 99.3                | 96.8                | 85.4                | 99.5                | 95.8                | 84.9                | 99.1                |
|                       | permutation_bonf | 95.6                | 83.9                | 99.3                | 96.3                | 85.9                | 99.5                | 94.8                | 84.3                | 99.3                |
| Weib shape continuous | asymptotic       | 87.9                | 70.7                | 96.1                | 88.3                | 71.4                | 95.9                | 87.4                | 73.7                | 96.4                |
|                       | asymptotic_bonf  | 87.3                | 70.4                | 95.9                | 87.9                | 71.0                | 95.7                | 87.2                | 73.0                | 96.4                |
|                       | permutation_bonf | 87.5                | 69.5                | 96.1                | 88.0                | 71.0                | 96.0                | 87.3                | 73.2                | 96.4                |
| Weib shape discrete   | asymptotic       | 94.1                | 79.9                | 98.6                | 94.1                | 80.4                | 98.7                | 93.6                | 81.1                | 98.3                |
|                       | asymptotic_bonf  | 93.9                | 79.5                | 98.5                | 93.9                | 80.0                | 98.7                | 93.6                | 80.8                | 98.3                |
|                       | permutation_bonf | 93.4                | 79.2                | 98.3                | 94.1                | 80.3                | 98.8                | 93.7                | 79.7                | 97.9                |

Table S38: Rejection rates in percent for the 2-by-2 design with  $\delta = 1.5$  and balanced medium sample sizes under equal censoring.

| Distribution          | Method           | $\mathcal{H}_{0,4}$ | $\mathcal{H}_{0,5}$ | $\mathcal{H}_{0,6}$ | $\mathcal{H}_{0,1}$ | $\mathcal{H}_{0,2}$ | $\mathcal{H}_{0,3}$ | $\mathcal{H}_{0,7}$ | $\mathcal{H}_{0,8}$ | $\mathcal{H}_{0,9}$ |
|-----------------------|------------------|---------------------|---------------------|---------------------|---------------------|---------------------|---------------------|---------------------|---------------------|---------------------|
| exp early continuous  | asymptotic       | 7.4                 | 5.7                 | 9.4                 | 7.2                 | 3.3                 | 10.4                | 6.1                 | 3.0                 | 11.0                |
|                       | asymptotic_bonf  | 7.2                 | 5.6                 | 9.2                 | 7.0                 | 3.3                 | 9.8                 | 6.0                 | 3.0                 | 10.8                |
|                       | permutation_bonf | 7.1                 | 5.3                 | 9.2                 | 6.8                 | 3.3                 | 9.3                 | 5.9                 | 3.0                 | 10.1                |
| exp early discrete    | asymptotic       | 8.2                 | 6.3                 | 12.0                | 8.2                 | 3.9                 | 12.1                | 7.4                 | 3.4                 | 12.6                |
|                       | asymptotic_bonf  | 8.0                 | 6.0                 | 11.2                | 8.1                 | 3.9                 | 11.6                | 7.3                 | 3.3                 | 12.4                |
|                       | permutation_bonf | 8.5                 | 5.6                 | 11.8                | 8.1                 | 4.4                 | 12.0                | 7.1                 | 3.0                 | 12.8                |
| exp late continuous   | asymptotic       | 6.8                 | 6.2                 | 9.5                 | 7.0                 | 3.4                 | 10.8                | 6.5                 | 3.2                 | 11.7                |
|                       | asymptotic_bonf  | 6.7                 | 5.6                 | 9.1                 | 6.6                 | 3.2                 | 10.4                | 6.3                 | 3.2                 | 11.4                |
|                       | permutation_bonf | 6.9                 | 6.0                 | 10.0                | 6.8                 | 3.5                 | 10.2                | 6.2                 | 3.3                 | 10.4                |
| exp late discrete     | asymptotic       | 7.7                 | 6.6                 | 11.9                | 8.2                 | 4.6                 | 13.0                | 8.3                 | 3.5                 | 13.1                |
|                       | asymptotic_bonf  | 7.4                 | 6.3                 | 11.0                | 7.9                 | 4.1                 | 12.5                | 7.8                 | 3.5                 | 12.7                |
|                       | permutation_bonf | 7.9                 | 6.0                 | 11.7                | 8.3                 | 4.5                 | 12.3                | 7.8                 | 3.3                 | 13.2                |
| exp prop continuous   | asymptotic       | 7.4                 | 5.1                 | 9.4                 | 6.4                 | 4.7                 | 8.9                 | 7.0                 | 4.9                 | 9.1                 |
|                       | asymptotic_bonf  | 7.4                 | 4.9                 | 9.1                 | 6.3                 | 4.5                 | 8.8                 | 6.4                 | 4.7                 | 9.1                 |
|                       | permutation_bonf | 6.8                 | 4.6                 | 9.0                 | 6.8                 | 4.4                 | 8.7                 | 6.9                 | 4.8                 | 9.0                 |
| exp prop discrete     | asymptotic       | 8.3                 | 5.6                 | 10.9                | 7.1                 | 5.3                 | 10.2                | 7.9                 | 5.4                 | 11.5                |
|                       | asymptotic_bonf  | 8.3                 | 5.3                 | 10.9                | 7.0                 | 5.3                 | 10.0                | 7.4                 | 5.2                 | 10.7                |
|                       | permutation_bonf | 8.3                 | 5.4                 | 11.0                | 6.8                 | 5.2                 | 10.0                | 7.8                 | 5.5                 | 10.5                |
| logn continuous       | asymptotic       | 19.9                | 13.2                | 33.1                | 22.0                | 14.2                | 33.4                | 23.1                | 13.5                | 33.3                |
|                       | asymptotic_bonf  | 19.2                | 12.7                | 32.6                | 21.6                | 13.9                | 32.8                | 22.6                | 13.2                | 32.6                |
|                       | permutation_bonf | 18.5                | 12.9                | 32.1                | 23.1                | 14.2                | 33.1                | 21.9                | 12.9                | 31.7                |
| logn discrete         | asymptotic       | 25.4                | 16.4                | 41.3                | 26.4                | 17.7                | 40.5                | 26.7                | 17.3                | 39.3                |
|                       | asymptotic_bonf  | 24.7                | 16.2                | 40.4                | 26.2                | 17.2                | 39.6                | 26.0                | 16.9                | 39.2                |
|                       | permutation_bonf | 24.4                | 15.5                | 39.4                | 25.3                | 17.4                | 39.4                | 27.3                | 16.6                | 38.7                |
| pwExp continuous      | asymptotic       | 7.2                 | 5.3                 | 9.4                 | 6.7                 | 3.9                 | 9.4                 | 5.6                 | 2.7                 | 9.9                 |
|                       | asymptotic_bonf  | 6.9                 | 5.3                 | 9.0                 | 6.6                 | 3.6                 | 9.1                 | 5.4                 | 2.6                 | 9.6                 |
|                       | permutation_bonf | 7.0                 | 5.1                 | 8.6                 | 5.6                 | 3.7                 | 8.8                 | 5.9                 | 2.4                 | 9.1                 |
| pwExp discrete        | asymptotic       | 8.7                 | 6.2                 | 11.7                | 7.2                 | 4.5                 | 11.5                | 7.4                 | 3.4                 | 12.1                |
|                       | asymptotic_bonf  | 8.7                 | 5.8                 | 11.3                | 7.1                 | 4.4                 | 11.0                | 7.2                 | 3.0                 | 11.8                |
|                       | permutation_bonf | 7.9                 | 6.0                 | 11.0                | 6.8                 | 4.6                 | 11.1                | 7.0                 | 3.4                 | 12.0                |
| Weib late continuous  | asymptotic       | 19.3                | 12.9                | 35.3                | 20.7                | 13.6                | 31.3                | 22.0                | 11.8                | 34.1                |
|                       | asymptotic_bonf  | 18.8                | 12.6                | 34.8                | 20.3                | 13.3                | 31.0                | 21.7                | 11.3                | 33.4                |
|                       | permutation_bonf | 18.2                | 12.4                | 34.6                | 21.0                | 13.7                | 30.9                | 21.8                | 12.0                | 34.1                |
| Weib late discrete    | asymptotic       | 23.1                | 15.3                | 40.0                | 25.3                | 16.4                | 36.8                | 27.4                | 14.3                | 38.7                |
|                       | asymptotic_bonf  | 23.0                | 14.9                | 39.6                | 24.4                | 16.2                | 36.1                | 26.4                | 14.0                | 38.4                |
|                       | permutation_bonf | 22.3                | 14.7                | 39.2                | 24.9                | 15.2                | 35.6                | 25.9                | 14.3                | 38.3                |
| Weib prop continuous  | asymptotic       | 19.0                | 12.5                | 33.9                | 19.7                | 13.1                | 29.9                | 21.9                | 11.7                | 33.2                |
|                       | asymptotic_bonf  | 18.5                | 12.1                | 33.8                | 19.4                | 12.9                | 29.5                | 21.5                | 11.1                | 32.8                |
|                       | permutation_bonf | 18.1                | 12.4                | 33.5                | 20.4                | 13.0                | 29.9                | 20.8                | 11.6                | 33.6                |
| Weib prop discrete    | asymptotic       | 22.9                | 16.0                | 40.9                | 25.7                | 15.2                | 36.9                | 26.5                | 14.9                | 39.0                |
|                       | asymptotic_bonf  | 22.7                | 15.7                | 40.3                | 25.1                | 14.9                | 36.4                | 25.9                | 14.5                | 38.1                |
|                       | permutation_bonf | 21.4                | 15.5                | 40.9                | 25.3                | 15.8                | 36.3                | 26.1                | 14.4                | 38.0                |
| Weib scale continuous | asymptotic       | 16.6                | 11.2                | 30.3                | 18.3                | 11.3                | 26.3                | 18.5                | 10.5                | 28.8                |
|                       | asymptotic_bonf  | 16.6                | 10.7                | 29.6                | 17.4                | 11.0                | 25.9                | 18.0                | 10.2                | 28.5                |
|                       | permutation_bonf | 16.4                | 11.7                | 30.1                | 17.5                | 11.6                | 26.3                | 18.2                | 10.7                | 28.2                |
| Weib scale discrete   | asymptotic       | 20.0                | 14.2                | 37.0                | 22.8                | 14.1                | 31.5                | 23.3                | 13.8                | 34.3                |
|                       | asymptotic_bonf  | 19.6                | 14.1                | 35.8                | 22.6                | 13.9                | 31.1                | 22.6                | 13.4                | 33.7                |
|                       | permutation_bonf | 19.4                | 14.5                | 37.0                | 22.8                | 13.6                | 31.2                | 22.8                | 13.2                | 32.7                |
| Weib shape continuous | asymptotic       | 13.5                | 9.4                 | 24.9                | 15.3                | 9.4                 | 21.8                | 15.9                | 8.3                 | 24.2                |
|                       | asymptotic_bonf  | 13.0                | 8.8                 | 24.3                | 14.7                | 9.3                 | 21.1                | 15.5                | 8.1                 | 23.6                |
|                       | permutation_bonf | 13.6                | 9.9                 | 24.7                | 14.4                | 9.3                 | 20.9                | 15.0                | 8.7                 | 24.1                |
| Weib shape discrete   | asymptotic       | 16.8                | 12.3                | 31.9                | 18.5                | 10.9                | 27.2                | 20.1                | 11.1                | 29.5                |
|                       | asymptotic_bonf  | 16.5                | 11.9                | 31.2                | 18.1                | 10.5                | 26.3                | 19.6                | 10.7                | 28.8                |
|                       | permutation_bonf | 16.2                | 11.9                | 31.7                | 18.2                | 11.2                | 26.3                | 18.9                | 11.3                | 28.5                |

Table S39: Rejection rates in percent for the 2-by-2 design with  $\delta = 1.5$  and balanced small sample sizes under equal censoring.

| Distribution          | Method           | $\mathcal{H}_{0,4}$ | $\mathcal{H}_{0,5}$ | $\mathcal{H}_{0,6}$ | $\mathcal{H}_{0,1}$ | $\mathcal{H}_{0,2}$ | $\mathcal{H}_{0,3}$ | $\mathcal{H}_{0,7}$ | $\mathcal{H}_{0,8}$ | $\mathcal{H}_{0,9}$ |
|-----------------------|------------------|---------------------|---------------------|---------------------|---------------------|---------------------|---------------------|---------------------|---------------------|---------------------|
| exp early continuous  | asymptotic       | 2.1                 | 1.3                 | 1.7                 | 2.0                 | 0.8                 | 1.7                 | 1.3                 | 1.6                 | 1.2                 |
|                       | asymptotic_bonf  | 2.0                 | 1.3                 | 1.4                 | 1.9                 | 0.8                 | 1.7                 | 1.2                 | 1.4                 | 1.1                 |
|                       | permutation_bonf | 1.7                 | 1.2                 | 1.5                 | 1.7                 | 0.8                 | 1.5                 | 1.4                 | 1.7                 | 0.9                 |
| exp early discrete    | asymptotic       | 2.0                 | 1.4                 | 1.2                 | 1.0                 | 1.6                 | 1.5                 | 2.0                 | 0.8                 | 1.7                 |
|                       | asymptotic_bonf  | 1.9                 | 1.4                 | 1.2                 | 1.0                 | 1.6                 | 1.5                 | 1.9                 | 0.8                 | 1.7                 |
|                       | permutation_bonf | 1.6                 | 1.5                 | 1.5                 | 0.8                 | 1.0                 | 1.2                 | 1.7                 | 0.5                 | 1.5                 |
| exp late continuous   | asymptotic       | 2.2                 | 1.2                 | 1.6                 | 2.2                 | 1.0                 | 1.8                 | 2.1                 | 1.3                 | 1.4                 |
|                       | asymptotic_bonf  | 1.9                 | 1.2                 | 1.4                 | 2.1                 | 0.9                 | 1.8                 | 2.0                 | 1.2                 | 1.3                 |
|                       | permutation_bonf | 1.5                 | 1.2                 | 1.6                 | 2.0                 | 1.1                 | 1.6                 | 1.5                 | 1.5                 | 1.1                 |
| exp late discrete     | asymptotic       | 2.2                 | 1.2                 | 1.4                 | 2.2                 | 1.0                 | 2.3                 | 2.1                 | 1.6                 | 1.3                 |
|                       | asymptotic_bonf  | 2.0                 | 1.2                 | 1.4                 | 2.0                 | 1.0                 | 2.2                 | 2.0                 | 1.5                 | 1.3                 |
|                       | permutation_bonf | 1.9                 | 1.0                 | 1.7                 | 1.9                 | 1.1                 | 2.1                 | 2.3                 | 1.6                 | 1.4                 |
| exp prop continuous   | asymptotic       | 1.2                 | 1.3                 | 1.9                 | 1.8                 | 1.4                 | 2.1                 | 0.8                 | 1.0                 | 2.0                 |
|                       | asymptotic_bonf  | 1.2                 | 1.3                 | 1.8                 | 1.8                 | 1.4                 | 2.0                 | 0.8                 | 0.9                 | 1.8                 |
|                       | permutation_bonf | 0.9                 | 0.8                 | 2.0                 | 1.3                 | 1.3                 | 1.9                 | 0.7                 | 0.9                 | 1.5                 |
| exp prop discrete     | asymptotic       | 2.0                 | 0.9                 | 2.1                 | 1.0                 | 0.8                 | 2.5                 | 1.3                 | 1.2                 | 2.5                 |
|                       | asymptotic_bonf  | 2.0                 | 0.9                 | 2.0                 | 1.0                 | 0.8                 | 2.5                 | 1.1                 | 1.1                 | 2.5                 |
|                       | permutation_bonf | 2.0                 | 1.0                 | 1.8                 | 0.9                 | 0.8                 | 1.9                 | 1.2                 | 1.0                 | 2.2                 |
| logn continuous       | asymptotic       | 4.1                 | 1.9                 | 3.9                 | 4.0                 | 3.4                 | 7.0                 | 3.0                 | 1.4                 | 3.8                 |
|                       | asymptotic_bonf  | 3.7                 | 1.7                 | 3.9                 | 3.8                 | 3.4                 | 6.8                 | 2.9                 | 1.4                 | 3.7                 |
|                       | permutation_bonf | 4.0                 | 1.7                 | 4.1                 | 3.5                 | 3.3                 | 6.1                 | 2.7                 | 1.5                 | 3.8                 |
| logn discrete         | asymptotic       | 4.2                 | 2.2                 | 5.3                 | 4.5                 | 4.0                 | 7.6                 | 4.0                 | 2.0                 | 6.0                 |
|                       | asymptotic_bonf  | 4.1                 | 2.2                 | 5.1                 | 4.5                 | 3.7                 | 7.5                 | 4.0                 | 1.8                 | 5.8                 |
|                       | permutation_bonf | 3.8                 | 2.1                 | 4.7                 | 4.1                 | 3.7                 | 7.3                 | 3.3                 | 1.6                 | 4.7                 |
| pwExp continuous      | asymptotic       | 1.9                 | 1.1                 | 1.6                 | 2.1                 | 0.9                 | 1.9                 | 1.9                 | 1.5                 | 1.4                 |
|                       | asymptotic_bonf  | 1.8                 | 1.0                 | 1.5                 | 2.1                 | 0.8                 | 1.7                 | 1.9                 | 1.5                 | 1.4                 |
|                       | permutation_bonf | 1.6                 | 1.1                 | 1.3                 | 1.9                 | 0.7                 | 1.6                 | 1.2                 | 1.4                 | 1.0                 |
| pwExp discrete        | asymptotic       | 2.2                 | 1.0                 | 1.6                 | 2.4                 | 0.9                 | 1.9                 | 1.9                 | 1.5                 | 1.6                 |
|                       | asymptotic_bonf  | 2.2                 | 1.0                 | 1.6                 | 2.3                 | 0.9                 | 1.9                 | 1.9                 | 1.4                 | 1.5                 |
|                       | permutation_bonf | 1.7                 | 1.1                 | 1.5                 | 1.9                 | 0.7                 | 1.8                 | 1.6                 | 1.5                 | 1.4                 |
| Weib late continuous  | asymptotic       | 4.1                 | 2.4                 | 4.8                 | 3.0                 | 3.2                 | 5.0                 | 4.2                 | 2.8                 | 4.8                 |
|                       | asymptotic_bonf  | 4.0                 | 2.4                 | 4.6                 | 3.0                 | 3.1                 | 5.0                 | 4.1                 | 2.6                 | 4.7                 |
|                       | permutation_bonf | 3.6                 | 2.0                 | 4.1                 | 2.7                 | 2.7                 | 4.8                 | 3.7                 | 2.7                 | 4.4                 |
| Weib late discrete    | asymptotic       | 4.9                 | 3.0                 | 5.9                 | 3.7                 | 3.4                 | 5.2                 | 3.9                 | 2.5                 | 5.8                 |
|                       | asymptotic_bonf  | 4.8                 | 2.9                 | 5.8                 | 3.5                 | 3.4                 | 4.9                 | 3.8                 | 2.5                 | 5.7                 |
|                       | permutation_bonf | 4.0                 | 2.4                 | 5.6                 | 3.1                 | 3.3                 | 4.6                 | 3.2                 | 2.5                 | 5.6                 |
| Weib prop continuous  | asymptotic       | 4.0                 | 2.0                 | 4.6                 | 2.9                 | 3.1                 | 4.3                 | 3.7                 | 2.7                 | 5.1                 |
|                       | asymptotic_bonf  | 3.9                 | 2.0                 | 4.3                 | 2.8                 | 3.1                 | 4.1                 | 3.5                 | 2.5                 | 5.0                 |
|                       | permutation_bonf | 3.3                 | 1.6                 | 4.0                 | 2.4                 | 2.6                 | 4.1                 | 3.5                 | 2.6                 | 4.0                 |
| Weib prop discrete    | asymptotic       | 4.5                 | 2.7                 | 5.4                 | 3.4                 | 3.3                 | 4.6                 | 3.5                 | 2.4                 | 5.7                 |
|                       | asymptotic_bonf  | 4.5                 | 2.3                 | 5.2                 | 3.3                 | 3.3                 | 4.5                 | 3.4                 | 2.4                 | 5.5                 |
|                       | permutation_bonf | 3.9                 | 2.3                 | 4.7                 | 3.3                 | 2.8                 | 4.2                 | 3.6                 | 2.6                 | 4.6                 |
| Weib scale continuous | asymptotic       | 2.9                 | 2.0                 | 4.4                 | 2.7                 | 2.4                 | 3.5                 | 2.8                 | 1.9                 | 4.3                 |
|                       | asymptotic_bonf  | 2.6                 | 1.8                 | 4.1                 | 2.5                 | 2.4                 | 3.3                 | 2.8                 | 1.8                 | 4.3                 |
|                       | permutation_bonf | 2.5                 | 1.8                 | 4.4                 | 1.8                 | 2.2                 | 3.6                 | 2.6                 | 2.3                 | 3.3                 |
| Weib scale discrete   | asymptotic       | 2.9                 | 1.9                 | 4.6                 | 2.8                 | 3.2                 | 3.8                 | 2.9                 | 2.7                 | 5.4                 |
|                       | asymptotic_bonf  | 2.9                 | 1.8                 | 4.4                 | 2.7                 | 3.0                 | 3.6                 | 2.7                 | 2.5                 | 5.1                 |
|                       | permutation_bonf | 2.5                 | 1.7                 | 4.1                 | 2.5                 | 2.9                 | 3.4                 | 2.4                 | 2.3                 | 4.4                 |
| Weib shape continuous | asymptotic       | 1.9                 | 1.8                 | 2.8                 | 1.3                 | 2.3                 | 3.1                 | 1.9                 | 1.7                 | 4.1                 |
|                       | asymptotic_bonf  | 1.8                 | 1.6                 | 2.8                 | 1.2                 | 2.2                 | 2.9                 | 1.8                 | 1.7                 | 3.6                 |
|                       | permutation_bonf | 1.6                 | 1.5                 | 3.0                 | 1.4                 | 1.9                 | 2.5                 | 1.9                 | 1.7                 | 3.1                 |
| Weib shape discrete   | asymptotic       | 2.5                 | 1.6                 | 3.6                 | 1.8                 | 2.4                 | 2.9                 | 2.0                 | 1.9                 | 4.1                 |
|                       | asymptotic_bonf  | 2.1                 | 1.3                 | 3.4                 | 1.5                 | 2.3                 | 2.7                 | 1.9                 | 1.8                 | 3.8                 |
|                       | permutation_bonf | 2.2                 | 1.6                 | 3.6                 | 1.3                 | 2.1                 | 2.0                 | 2.2                 | 2.0                 | 3.6                 |

Table S40: Rejection rates in percent for the 2-by-2 design with  $\delta = 1.5$  and unbalanced large sample sizes under equal censoring.

| Distribution          | Method           | $\mathcal{H}_{0,4}$ | $\mathcal{H}_{0,5}$ | $\mathcal{H}_{0,6}$ | $\mathcal{H}_{0,1}$ | $\mathcal{H}_{0,2}$ | $\mathcal{H}_{0,3}$ | $\mathcal{H}_{0,7}$ | $\mathcal{H}_{0,8}$ | $\mathcal{H}_{0,9}$ |
|-----------------------|------------------|---------------------|---------------------|---------------------|---------------------|---------------------|---------------------|---------------------|---------------------|---------------------|
| exp early continuous  | asymptotic       | 25.0                | 13.5                | 39.6                | 25.4                | 13.2                | 38.0                | 24.2                | 13.6                | 37.5                |
|                       | asymptotic.bonf  | 23.2                | 12.2                | 37.6                | 23.8                | 12.2                | 36.2                | 22.4                | 12.3                | 35.9                |
|                       | permutation.bonf | 23.1                | 12.1                | 36.7                | 22.7                | 11.8                | 35.4                | 21.8                | 12.1                | 35.1                |
| exp early discrete    | asymptotic       | 28.8                | 15.4                | 45.8                | 28.9                | 15.7                | 45.3                | 28.6                | 16.5                | 43.1                |
|                       | asymptotic.bonf  | 26.8                | 14.4                | 43.7                | 26.9                | 14.8                | 42.6                | 27.3                | 14.9                | 41.3                |
|                       | permutation.bonf | 26.8                | 14.0                | 42.2                | 25.9                | 14.6                | 42.1                | 26.5                | 15.0                | 40.6                |
| exp late continuous   | asymptotic       | 27.0                | 14.4                | 45.2                | 26.3                | 15.2                | 43.3                | 26.4                | 15.3                | 42.7                |
|                       | asymptotic.bonf  | 25.3                | 13.2                | 43.6                | 24.7                | 13.7                | 40.9                | 25.1                | 13.5                | 40.7                |
|                       | permutation.bonf | 24.9                | 13.1                | 42.8                | 25.0                | 13.1                | 40.4                | 24.2                | 14.3                | 40.5                |
| exp late discrete     | asymptotic       | 31.3                | 18.1                | 52.7                | 30.2                | 17.3                | 51.0                | 31.2                | 18.1                | 47.4                |
|                       | asymptotic.bonf  | 29.4                | 16.8                | 49.4                | 29.2                | 15.6                | 49.0                | 29.6                | 16.9                | 46.1                |
|                       | permutation.bonf | 28.4                | 15.7                | 49.1                | 29.2                | 15.3                | 47.3                | 29.2                | 16.5                | 45.7                |
| exp prop continuous   | asymptotic       | 28.5                | 17.0                | 38.1                | 26.0                | 16.0                | 40.4                | 26.2                | 15.4                | 36.2                |
|                       | asymptotic.bonf  | 26.6                | 16.2                | 36.2                | 24.3                | 15.2                | 38.0                | 24.2                | 14.2                | 34.8                |
|                       | permutation.bonf | 27.4                | 14.9                | 35.1                | 24.3                | 13.0                | 38.0                | 24.3                | 14.1                | 34.8                |
| exp prop discrete     | asymptotic       | 32.3                | 20.3                | 44.6                | 28.8                | 18.6                | 45.8                | 31.1                | 17.8                | 43.6                |
|                       | asymptotic.bonf  | 30.9                | 18.8                | 42.0                | 27.2                | 17.6                | 44.6                | 29.0                | 16.5                | 41.5                |
|                       | permutation.bonf | 30.6                | 18.0                | 40.2                | 27.6                | 16.3                | 43.0                | 28.2                | 16.4                | 41.1                |
| logn continuous       | asymptotic       | 69.1                | 48.7                | 84.3                | 69.4                | 52.8                | 84.3                | 68.9                | 49.1                | 82.9                |
|                       | asymptotic.bonf  | 67.1                | 46.0                | 82.6                | 67.2                | 49.7                | 83.0                | 66.7                | 46.5                | 81.8                |
|                       | permutation.bonf | 66.5                | 45.4                | 81.8                | 65.6                | 49.2                | 82.2                | 66.5                | 45.1                | 81.2                |
| logn discrete         | asymptotic       | 77.3                | 58.0                | 89.8                | 76.8                | 58.8                | 88.9                | 76.5                | 57.9                | 88.9                |
|                       | asymptotic.bonf  | 75.8                | 55.1                | 88.0                | 75.4                | 57.0                | 87.6                | 75.0                | 54.5                | 88.1                |
|                       | permutation.bonf | 74.9                | 53.9                | 87.2                | 74.3                | 55.8                | 87.3                | 74.3                | 53.9                | 87.9                |
| pwExp continuous      | asymptotic       | 23.9                | 13.3                | 39.6                | 22.9                | 12.8                | 38.9                | 22.9                | 13.1                | 37.7                |
|                       | asymptotic.bonf  | 22.6                | 11.9                | 36.8                | 21.6                | 11.7                | 35.8                | 21.4                | 12.4                | 35.1                |
|                       | permutation.bonf | 22.1                | 11.5                | 37.2                | 20.9                | 11.2                | 35.1                | 22.0                | 12.0                | 34.6                |
| pwExp discrete        | asymptotic       | 26.9                | 16.1                | 46.1                | 26.6                | 14.9                | 44.8                | 26.4                | 16.0                | 43.0                |
|                       | asymptotic.bonf  | 25.8                | 14.5                | 44.3                | 24.6                | 13.8                | 43.0                | 25.3                | 14.9                | 41.3                |
|                       | permutation.bonf | 26.8                | 14.5                | 44.9                | 24.5                | 13.7                | 42.2                | 25.4                | 14.6                | 40.2                |
| Weib late continuous  | asymptotic       | 70.4                | 46.9                | 86.6                | 70.9                | 45.8                | 88.4                | 70.5                | 48.8                | 87.1                |
|                       | asymptotic.bonf  | 68.2                | 44.7                | 85.6                | 69.2                | 43.9                | 87.5                | 68.5                | 46.8                | 85.6                |
|                       | permutation.bonf | 66.7                | 44.5                | 85.7                | 68.4                | 42.6                | 86.7                | 68.1                | 45.7                | 85.5                |
| Weib late discrete    | asymptotic       | 76.1                | 54.5                | 90.5                | 74.1                | 54.8                | 92.2                | 76.4                | 54.1                | 90.2                |
|                       | asymptotic.bonf  | 75.0                | 51.8                | 89.0                | 72.7                | 51.8                | 90.8                | 73.9                | 52.8                | 89.6                |
|                       | permutation.bonf | 74.1                | 50.9                | 88.5                | 72.3                | 50.4                | 90.2                | 73.3                | 50.7                | 89.4                |
| Weib prop continuous  | asymptotic       | 67.5                | 45.8                | 84.3                | 67.8                | 44.7                | 86.1                | 67.7                | 47.0                | 84.3                |
|                       | asymptotic.bonf  | 65.7                | 43.0                | 83.3                | 66.1                | 42.5                | 84.7                | 65.3                | 44.4                | 82.8                |
|                       | permutation.bonf | 63.6                | 42.3                | 82.8                | 65.4                | 41.1                | 84.9                | 66.0                | 43.9                | 83.2                |
| Weib prop discrete    | asymptotic       | 76.9                | 54.1                | 90.4                | 75.7                | 54.1                | 91.6                | 77.2                | 53.9                | 90.3                |
|                       | asymptotic.bonf  | 74.7                | 51.8                | 89.4                | 73.1                | 51.9                | 91.2                | 76.0                | 51.7                | 89.6                |
|                       | permutation.bonf | 74.2                | 50.6                | 88.8                | 72.6                | 50.1                | 90.2                | 75.3                | 51.1                | 89.6                |
| Weib scale continuous | asymptotic       | 58.5                | 38.3                | 76.6                | 58.9                | 39.5                | 77.4                | 59.0                | 39.0                | 76.2                |
|                       | asymptotic.bonf  | 57.0                | 36.4                | 74.8                | 56.9                | 37.5                | 75.6                | 56.6                | 36.4                | 74.3                |
|                       | permutation.bonf | 54.3                | 34.8                | 73.6                | 55.8                | 35.0                | 74.3                | 55.0                | 36.2                | 73.1                |
| Weib scale discrete   | asymptotic       | 66.4                | 46.2                | 84.2                | 67.3                | 46.4                | 85.3                | 67.7                | 46.9                | 83.8                |
|                       | asymptotic.bonf  | 64.4                | 44.8                | 82.5                | 64.6                | 44.2                | 84.2                | 65.4                | 43.3                | 82.8                |
|                       | permutation.bonf | 63.7                | 43.5                | 81.3                | 64.4                | 43.2                | 82.5                | 64.2                | 42.3                | 82.6                |
| Weib shape continuous | asymptotic       | 45.5                | 29.0                | 63.0                | 49.0                | 30.5                | 64.9                | 45.7                | 29.8                | 65.1                |
|                       | asymptotic.bonf  | 41.7                | 25.5                | 59.8                | 46.0                | 27.8                | 62.0                | 42.2                | 27.0                | 61.0                |
|                       | permutation.bonf | 41.5                | 24.9                | 58.9                | 44.5                | 25.7                | 61.2                | 42.3                | 26.9                | 60.3                |
| Weib shape discrete   | asymptotic       | 55.5                | 35.9                | 75.0                | 56.7                | 37.4                | 75.5                | 56.0                | 36.7                | 74.9                |
|                       | asymptotic.bonf  | 52.6                | 33.9                | 71.5                | 53.3                | 34.6                | 73.0                | 51.8                | 34.5                | 72.2                |
|                       | permutation.bonf | 51.8                | 32.5                | 70.6                | 53.4                | 33.4                | 71.8                | 51.8                | 33.5                | 71.9                |

Table S41: Rejection rates in percent for the 2-by-2 design with  $\delta = 1.5$  and unbalanced medium sample sizes under equal censoring.

| Distribution          | Method           | $\mathcal{H}_{0,4}$ | $\mathcal{H}_{0,5}$ | $\mathcal{H}_{0,6}$ | $\mathcal{H}_{0,1}$ | $\mathcal{H}_{0,2}$ | $\mathcal{H}_{0,3}$ | $\mathcal{H}_{0,7}$ | $\mathcal{H}_{0,8}$ | $\mathcal{H}_{0,9}$ |
|-----------------------|------------------|---------------------|---------------------|---------------------|---------------------|---------------------|---------------------|---------------------|---------------------|---------------------|
| exp early continuous  | asymptotic       | 3.0                 | 1.9                 | 4.5                 | 3.3                 | 1.5                 | 4.0                 | 3.3                 | 1.9                 | 4.2                 |
|                       | asymptotic_bonf  | 2.4                 | 1.5                 | 4.1                 | 2.8                 | 1.3                 | 3.6                 | 2.8                 | 1.8                 | 3.7                 |
|                       | permutation_bonf | 1.6                 | 1.6                 | 3.1                 | 2.4                 | 0.9                 | 3.2                 | 2.4                 | 1.3                 | 3.3                 |
| exp early discrete    | asymptotic       | 3.3                 | 2.0                 | 5.0                 | 3.6                 | 1.7                 | 4.2                 | 3.6                 | 2.3                 | 5.4                 |
|                       | asymptotic_bonf  | 2.9                 | 1.8                 | 4.5                 | 3.5                 | 1.4                 | 4.1                 | 2.9                 | 1.9                 | 5.0                 |
|                       | permutation_bonf | 1.8                 | 1.7                 | 4.1                 | 2.8                 | 0.9                 | 3.2                 | 2.7                 | 1.8                 | 4.3                 |
| exp late continuous   | asymptotic       | 2.8                 | 2.1                 | 4.7                 | 4.1                 | 2.3                 | 4.6                 | 4.1                 | 2.1                 | 5.3                 |
|                       | asymptotic_bonf  | 2.2                 | 2.0                 | 4.3                 | 3.8                 | 1.6                 | 4.1                 | 3.8                 | 1.9                 | 4.3                 |
|                       | permutation_bonf | 2.3                 | 1.9                 | 3.7                 | 3.3                 | 1.1                 | 3.4                 | 2.8                 | 1.4                 | 3.5                 |
| exp late discrete     | asymptotic       | 2.9                 | 2.2                 | 5.2                 | 4.5                 | 2.1                 | 5.2                 | 4.1                 | 2.2                 | 5.9                 |
|                       | asymptotic_bonf  | 2.4                 | 2.0                 | 4.8                 | 4.3                 | 1.9                 | 4.4                 | 3.9                 | 2.0                 | 5.2                 |
|                       | permutation_bonf | 2.2                 | 2.1                 | 4.0                 | 3.1                 | 1.3                 | 3.8                 | 3.4                 | 1.8                 | 4.8                 |
| exp prop continuous   | asymptotic       | 3.4                 | 2.5                 | 4.2                 | 2.3                 | 1.9                 | 4.6                 | 3.2                 | 2.1                 | 4.8                 |
|                       | asymptotic_bonf  | 3.0                 | 2.2                 | 3.7                 | 1.9                 | 1.7                 | 4.3                 | 3.0                 | 1.8                 | 4.3                 |
|                       | permutation_bonf | 2.5                 | 1.7                 | 2.9                 | 1.9                 | 1.2                 | 3.7                 | 2.2                 | 1.8                 | 4.4                 |
| exp prop discrete     | asymptotic       | 3.4                 | 3.0                 | 4.6                 | 2.8                 | 2.4                 | 5.3                 | 3.3                 | 1.8                 | 5.4                 |
|                       | asymptotic_bonf  | 2.8                 | 2.9                 | 4.4                 | 2.4                 | 2.1                 | 4.7                 | 3.1                 | 1.7                 | 4.7                 |
|                       | permutation_bonf | 2.8                 | 2.1                 | 3.6                 | 2.0                 | 1.3                 | 3.8                 | 2.8                 | 1.7                 | 4.9                 |
| logn continuous       | asymptotic       | 8.3                 | 5.6                 | 12.6                | 6.8                 | 4.4                 | 12.7                | 6.6                 | 6.0                 | 13.6                |
|                       | asymptotic_bonf  | 7.3                 | 5.1                 | 11.5                | 5.7                 | 3.7                 | 12.2                | 5.9                 | 5.4                 | 12.5                |
|                       | permutation_bonf | 6.0                 | 3.5                 | 9.6                 | 5.2                 | 2.4                 | 9.8                 | 5.0                 | 3.9                 | 11.8                |
| logn discrete         | asymptotic       | 10.3                | 6.3                 | 16.4                | 8.0                 | 5.1                 | 14.7                | 8.5                 | 6.7                 | 16.3                |
|                       | asymptotic_bonf  | 9.1                 | 5.3                 | 14.5                | 7.4                 | 4.4                 | 13.9                | 7.9                 | 6.1                 | 14.6                |
|                       | permutation_bonf | 7.1                 | 4.2                 | 11.4                | 6.4                 | 2.6                 | 12.0                | 6.3                 | 5.2                 | 14.1                |
| pwExp continuous      | asymptotic       | 1.9                 | 2.2                 | 4.0                 | 2.9                 | 1.8                 | 3.9                 | 3.1                 | 1.7                 | 4.5                 |
|                       | asymptotic_bonf  | 1.6                 | 1.7                 | 3.5                 | 2.2                 | 1.2                 | 3.3                 | 2.6                 | 1.6                 | 4.2                 |
|                       | permutation_bonf | 1.5                 | 1.8                 | 3.5                 | 2.2                 | 1.4                 | 2.8                 | 2.4                 | 1.1                 | 3.8                 |
| pwExp discrete        | asymptotic       | 2.1                 | 2.3                 | 4.9                 | 3.4                 | 2.0                 | 4.5                 | 3.3                 | 1.8                 | 5.7                 |
|                       | asymptotic_bonf  | 1.7                 | 2.2                 | 4.3                 | 2.8                 | 1.6                 | 3.9                 | 2.8                 | 1.6                 | 4.7                 |
|                       | permutation_bonf | 1.4                 | 1.8                 | 3.7                 | 2.4                 | 1.7                 | 3.3                 | 2.7                 | 1.3                 | 4.6                 |
| Weib late continuous  | asymptotic       | 8.8                 | 4.7                 | 14.0                | 7.2                 | 5.1                 | 14.4                | 9.9                 | 4.7                 | 14.7                |
|                       | asymptotic_bonf  | 7.8                 | 4.1                 | 12.4                | 6.3                 | 4.4                 | 13.2                | 8.8                 | 3.8                 | 13.7                |
|                       | permutation_bonf | 6.6                 | 2.9                 | 10.4                | 5.1                 | 2.6                 | 11.0                | 6.7                 | 3.2                 | 13.0                |
| Weib late discrete    | asymptotic       | 9.5                 | 6.4                 | 16.2                | 9.6                 | 6.3                 | 16.8                | 12.7                | 5.5                 | 17.6                |
|                       | asymptotic_bonf  | 8.1                 | 5.6                 | 14.9                | 8.3                 | 6.0                 | 15.3                | 11.6                | 5.4                 | 15.3                |
|                       | permutation_bonf | 6.8                 | 3.6                 | 13.0                | 6.3                 | 3.4                 | 12.5                | 9.7                 | 4.5                 | 13.7                |
| Weib prop continuous  | asymptotic       | 7.6                 | 4.3                 | 12.4                | 6.3                 | 4.8                 | 12.8                | 8.7                 | 4.3                 | 13.9                |
|                       | asymptotic_bonf  | 7.0                 | 3.7                 | 11.4                | 5.7                 | 4.2                 | 11.6                | 7.7                 | 3.6                 | 12.6                |
|                       | permutation_bonf | 6.2                 | 2.5                 | 9.7                 | 4.5                 | 1.8                 | 9.5                 | 6.3                 | 2.9                 | 11.8                |
| Weib prop discrete    | asymptotic       | 9.1                 | 5.8                 | 14.5                | 8.6                 | 5.7                 | 15.6                | 10.4                | 5.0                 | 15.5                |
|                       | asymptotic_bonf  | 7.9                 | 4.7                 | 13.8                | 7.9                 | 5.0                 | 13.7                | 8.8                 | 4.6                 | 14.4                |
|                       | permutation_bonf | 6.4                 | 2.9                 | 11.4                | 5.6                 | 3.3                 | 11.6                | 7.6                 | 3.5                 | 12.7                |
| Weib scale continuous | asymptotic       | 6.1                 | 3.1                 | 8.9                 | 5.7                 | 3.6                 | 9.9                 | 6.4                 | 3.1                 | 10.3                |
|                       | asymptotic_bonf  | 5.7                 | 2.4                 | 7.5                 | 4.6                 | 2.9                 | 8.4                 | 5.7                 | 2.6                 | 8.8                 |
|                       | permutation_bonf | 4.5                 | 1.8                 | 6.2                 | 3.1                 | 1.3                 | 6.9                 | 5.3                 | 2.1                 | 7.7                 |
| Weib scale discrete   | asymptotic       | 7.2                 | 3.2                 | 11.0                | 6.7                 | 3.9                 | 11.8                | 7.8                 | 3.7                 | 11.6                |
|                       | asymptotic_bonf  | 6.3                 | 3.0                 | 9.9                 | 5.7                 | 3.5                 | 10.5                | 6.9                 | 3.4                 | 10.3                |
|                       | permutation_bonf | 5.3                 | 1.8                 | 7.6                 | 4.1                 | 1.9                 | 8.5                 | 6.2                 | 2.6                 | 8.7                 |
| Weib shape continuous | asymptotic       | 4.0                 | 1.8                 | 5.9                 | 3.5                 | 2.3                 | 6.0                 | 4.5                 | 2.5                 | 5.7                 |
|                       | asymptotic_bonf  | 2.8                 | 1.2                 | 5.2                 | 2.7                 | 1.7                 | 4.8                 | 3.3                 | 1.9                 | 4.6                 |
|                       | permutation_bonf | 2.0                 | 0.9                 | 4.3                 | 1.5                 | 1.2                 | 4.0                 | 2.8                 | 1.3                 | 3.9                 |
| Weib shape discrete   | asymptotic       | 4.9                 | 1.8                 | 7.6                 | 5.6                 | 2.5                 | 7.1                 | 5.7                 | 3.0                 | 8.1                 |
|                       | asymptotic_bonf  | 4.1                 | 1.3                 | 6.3                 | 4.0                 | 2.1                 | 6.0                 | 4.4                 | 2.6                 | 7.0                 |
|                       | permutation_bonf | 2.7                 | 0.7                 | 5.0                 | 2.3                 | 1.3                 | 4.9                 | 4.4                 | 2.0                 | 6.2                 |



Table S42: Rejection rates in percent for the 2-by-2 design with  $\delta = 1.5$  and unbalanced small sample sizes under equal censoring.

| Distribution          | Method           | $\mathcal{H}_{0,4}$ | $\mathcal{H}_{0,5}$ | $\mathcal{H}_{0,6}$ | $\mathcal{H}_{0,1}$ | $\mathcal{H}_{0,2}$ | $\mathcal{H}_{0,3}$ | $\mathcal{H}_{0,7}$ | $\mathcal{H}_{0,8}$ | $\mathcal{H}_{0,9}$ |
|-----------------------|------------------|---------------------|---------------------|---------------------|---------------------|---------------------|---------------------|---------------------|---------------------|---------------------|
| exp early continuous  | asymptotic       | 1.3                 | 1.4                 | 1.9                 | 1.2                 | 1.2                 | 1.0                 | 0.6                 | 1.0                 | 2.2                 |
|                       | asymptotic_bonf  | 1.2                 | 1.3                 | 1.4                 | 1.0                 | 1.2                 | 0.9                 | 0.5                 | 1.0                 | 1.9                 |
|                       | permutation_bonf | 0.3                 | 0.5                 | 0.5                 | 0.1                 | 0.4                 | 0.4                 | 0.3                 | 0.4                 | 1.2                 |
| exp early discrete    | asymptotic       | 1.4                 | 1.1                 | 1.6                 | 1.4                 | 1.2                 | 1.0                 | 0.8                 | 1.3                 | 2.0                 |
|                       | asymptotic_bonf  | 1.2                 | 1.1                 | 1.5                 | 1.2                 | 1.1                 | 1.0                 | 0.7                 | 0.9                 | 2.0                 |
|                       | permutation_bonf | 0.2                 | 0.3                 | 0.6                 | 0.2                 | 0.4                 | 0.5                 | 0.3                 | 0.6                 | 1.0                 |
| exp late continuous   | asymptotic       | 1.6                 | 0.9                 | 1.5                 | 1.2                 | 1.0                 | 1.3                 | 0.7                 | 1.0                 | 2.4                 |
|                       | asymptotic_bonf  | 1.4                 | 0.9                 | 1.4                 | 0.8                 | 0.8                 | 1.2                 | 0.5                 | 1.0                 | 2.3                 |
|                       | permutation_bonf | 0.2                 | 0.3                 | 0.3                 | 0.4                 | 0.3                 | 0.4                 | 0.2                 | 0.4                 | 1.3                 |
| exp late discrete     | asymptotic       | 1.9                 | 1.0                 | 1.7                 | 0.9                 | 1.2                 | 1.7                 | 0.9                 | 1.1                 | 2.6                 |
|                       | asymptotic_bonf  | 1.5                 | 0.9                 | 1.2                 | 0.9                 | 1.0                 | 1.7                 | 0.6                 | 1.0                 | 2.4                 |
|                       | permutation_bonf | 0.2                 | 0.0                 | 0.8                 | 0.4                 | 0.2                 | 0.6                 | 0.1                 | 0.5                 | 1.7                 |
| exp prop continuous   | asymptotic       | 1.4                 | 1.6                 | 2.2                 | 1.1                 | 1.1                 | 2.0                 | 1.2                 | 0.8                 | 1.8                 |
|                       | asymptotic_bonf  | 1.4                 | 1.3                 | 2.0                 | 1.1                 | 1.1                 | 1.9                 | 1.2                 | 0.8                 | 1.4                 |
|                       | permutation_bonf | 0.8                 | 0.4                 | 0.5                 | 0.4                 | 0.0                 | 0.9                 | 0.6                 | 0.3                 | 0.7                 |
| exp prop discrete     | asymptotic       | 1.4                 | 1.4                 | 2.1                 | 1.1                 | 1.0                 | 2.5                 | 1.1                 | 1.0                 | 1.8                 |
|                       | asymptotic_bonf  | 1.3                 | 1.4                 | 2.0                 | 0.9                 | 0.9                 | 2.3                 | 1.0                 | 0.7                 | 1.8                 |
|                       | permutation_bonf | 0.4                 | 0.6                 | 1.1                 | 0.5                 | 0.1                 | 1.0                 | 0.5                 | 0.6                 | 0.7                 |
| logn continuous       | asymptotic       | 1.5                 | 1.0                 | 2.7                 | 1.9                 | 1.9                 | 2.0                 | 1.9                 | 1.4                 | 2.6                 |
|                       | asymptotic_bonf  | 1.3                 | 0.7                 | 2.6                 | 1.8                 | 1.6                 | 2.0                 | 1.9                 | 0.9                 | 2.4                 |
|                       | permutation_bonf | 0.3                 | 0.3                 | 1.0                 | 0.2                 | 0.3                 | 0.6                 | 0.7                 | 0.2                 | 0.8                 |
| logn discrete         | asymptotic       | 2.1                 | 1.4                 | 2.8                 | 2.2                 | 1.6                 | 2.3                 | 1.9                 | 1.3                 | 2.8                 |
|                       | asymptotic_bonf  | 1.9                 | 1.1                 | 2.6                 | 2.0                 | 1.2                 | 1.9                 | 1.7                 | 0.9                 | 2.5                 |
|                       | permutation_bonf | 0.4                 | 0.2                 | 1.2                 | 0.3                 | 0.3                 | 0.6                 | 0.8                 | 0.2                 | 1.1                 |
| pwExp continuous      | asymptotic       | 0.8                 | 1.4                 | 1.6                 | 0.5                 | 1.1                 | 1.4                 | 0.6                 | 1.0                 | 1.9                 |
|                       | asymptotic_bonf  | 0.7                 | 1.3                 | 1.4                 | 0.5                 | 0.9                 | 1.4                 | 0.6                 | 1.0                 | 1.8                 |
|                       | permutation_bonf | 0.2                 | 0.3                 | 0.5                 | 0.1                 | 0.3                 | 0.6                 | 0.1                 | 0.5                 | 1.0                 |
| pwExp discrete        | asymptotic       | 1.2                 | 1.4                 | 1.8                 | 0.7                 | 0.9                 | 1.7                 | 0.6                 | 1.2                 | 2.2                 |
|                       | asymptotic_bonf  | 0.8                 | 1.3                 | 1.5                 | 0.5                 | 0.8                 | 1.7                 | 0.6                 | 1.0                 | 1.8                 |
|                       | permutation_bonf | 0.2                 | 0.5                 | 0.6                 | 0.2                 | 0.2                 | 0.5                 | 0.2                 | 0.5                 | 1.1                 |
| Weib late continuous  | asymptotic       | 1.9                 | 1.4                 | 3.4                 | 1.9                 | 1.6                 | 2.3                 | 1.7                 | 1.2                 | 2.3                 |
|                       | asymptotic_bonf  | 1.7                 | 1.3                 | 2.9                 | 1.6                 | 1.4                 | 1.9                 | 1.3                 | 1.1                 | 2.2                 |
|                       | permutation_bonf | 0.4                 | 0.4                 | 0.7                 | 0.1                 | 0.1                 | 0.7                 | 0.6                 | 0.5                 | 1.1                 |
| Weib late discrete    | asymptotic       | 2.3                 | 1.5                 | 3.2                 | 2.0                 | 1.6                 | 2.5                 | 1.7                 | 1.3                 | 3.0                 |
|                       | asymptotic_bonf  | 1.9                 | 1.5                 | 2.8                 | 1.7                 | 1.1                 | 2.2                 | 1.6                 | 1.2                 | 2.7                 |
|                       | permutation_bonf | 0.8                 | 0.6                 | 0.9                 | 0.4                 | 0.2                 | 0.4                 | 0.7                 | 0.5                 | 0.9                 |
| Weib prop continuous  | asymptotic       | 1.8                 | 1.5                 | 2.8                 | 1.4                 | 1.7                 | 2.2                 | 1.3                 | 1.5                 | 1.9                 |
|                       | asymptotic_bonf  | 1.6                 | 1.4                 | 2.3                 | 1.1                 | 1.6                 | 1.9                 | 1.2                 | 1.1                 | 1.8                 |
|                       | permutation_bonf | 0.3                 | 0.4                 | 0.9                 | 0.2                 | 0.1                 | 0.7                 | 0.5                 | 0.3                 | 0.9                 |
| Weib prop discrete    | asymptotic       | 2.0                 | 1.4                 | 2.8                 | 1.8                 | 1.7                 | 2.8                 | 1.3                 | 1.2                 | 2.2                 |
|                       | asymptotic_bonf  | 1.6                 | 1.4                 | 2.5                 | 1.5                 | 1.4                 | 2.5                 | 1.0                 | 0.9                 | 1.9                 |
|                       | permutation_bonf | 0.4                 | 0.5                 | 1.2                 | 0.3                 | 0.1                 | 0.5                 | 0.3                 | 0.3                 | 1.0                 |
| Weib scale continuous | asymptotic       | 1.6                 | 1.3                 | 2.6                 | 1.5                 | 1.8                 | 2.0                 | 1.1                 | 1.3                 | 1.8                 |
|                       | asymptotic_bonf  | 1.5                 | 1.3                 | 2.1                 | 1.4                 | 1.6                 | 1.8                 | 1.1                 | 0.8                 | 1.7                 |
|                       | permutation_bonf | 0.3                 | 0.3                 | 0.8                 | 0.2                 | 0.3                 | 0.8                 | 0.4                 | 0.1                 | 0.7                 |
| Weib scale discrete   | asymptotic       | 1.5                 | 1.5                 | 2.3                 | 1.4                 | 2.4                 | 2.3                 | 0.8                 | 0.9                 | 2.0                 |
|                       | asymptotic_bonf  | 1.2                 | 1.4                 | 2.0                 | 1.3                 | 2.1                 | 2.2                 | 0.8                 | 0.7                 | 1.8                 |
|                       | permutation_bonf | 0.5                 | 0.6                 | 0.8                 | 0.4                 | 0.3                 | 0.4                 | 0.7                 | 0.1                 | 0.7                 |
| Weib shape continuous | asymptotic       | 2.6                 | 1.6                 | 2.4                 | 2.0                 | 3.4                 | 1.7                 | 2.2                 | 2.4                 | 1.7                 |
|                       | asymptotic_bonf  | 2.2                 | 1.4                 | 2.1                 | 1.9                 | 3.0                 | 1.6                 | 1.8                 | 1.8                 | 1.5                 |
|                       | permutation_bonf | 0.9                 | 0.5                 | 1.0                 | 0.4                 | 0.8                 | 0.9                 | 1.1                 | 0.5                 | 0.9                 |
| Weib shape discrete   | asymptotic       | 2.4                 | 1.7                 | 2.5                 | 1.8                 | 3.1                 | 2.6                 | 2.2                 | 1.7                 | 1.8                 |
|                       | asymptotic_bonf  | 2.1                 | 1.6                 | 2.3                 | 1.6                 | 2.5                 | 2.0                 | 2.0                 | 1.4                 | 1.7                 |
|                       | permutation_bonf | 0.7                 | 0.7                 | 0.9                 | 0.3                 | 0.5                 | 0.5                 | 1.1                 | 0.5                 | 0.8                 |

Table S43: Rejection rates in percent for the 2-by-2 design with  $\delta = 1.5$  and balanced large sample sizes under unequal, high censoring.

| Distribution          | Method           | $\mathcal{H}_{0,4}$ | $\mathcal{H}_{0,5}$ | $\mathcal{H}_{0,6}$ | $\mathcal{H}_{0,1}$ | $\mathcal{H}_{0,2}$ | $\mathcal{H}_{0,3}$ | $\mathcal{H}_{0,7}$ | $\mathcal{H}_{0,8}$ | $\mathcal{H}_{0,9}$ |
|-----------------------|------------------|---------------------|---------------------|---------------------|---------------------|---------------------|---------------------|---------------------|---------------------|---------------------|
| exp early continuous  | asymptotic       | 38.0                | 25.0                | 55.3                | 35.6                | 24.5                | 55.1                | 38.9                | 22.5                | 55.6                |
|                       | asymptotic_bonf  | 37.4                | 24.5                | 54.8                | 35.0                | 24.0                | 54.5                | 38.3                | 22.3                | 55.2                |
|                       | permutation_bonf | 38.1                | 23.3                | 53.7                | 35.7                | 23.9                | 54.5                | 37.2                | 22.8                | 54.2                |
| exp early discrete    | asymptotic       | 41.8                | 27.3                | 60.0                | 39.5                | 27.6                | 60.1                | 41.6                | 26.1                | 61.0                |
|                       | asymptotic_bonf  | 41.7                | 26.9                | 59.5                | 38.9                | 27.0                | 59.6                | 41.4                | 25.2                | 60.7                |
|                       | permutation_bonf | 42.3                | 26.5                | 59.2                | 37.2                | 27.3                | 60.0                | 39.6                | 25.4                | 59.4                |
| exp late continuous   | asymptotic       | 38.6                | 24.5                | 56.8                | 36.9                | 24.1                | 55.6                | 39.4                | 24.5                | 57.3                |
|                       | asymptotic_bonf  | 37.9                | 24.0                | 55.9                | 36.5                | 23.3                | 55.0                | 38.8                | 23.8                | 56.8                |
|                       | permutation_bonf | 37.7                | 24.5                | 55.1                | 36.2                | 24.5                | 54.2                | 38.9                | 24.2                | 55.9                |
| exp late discrete     | asymptotic       | 43.7                | 28.3                | 61.6                | 40.8                | 27.6                | 61.4                | 42.7                | 26.1                | 62.1                |
|                       | asymptotic_bonf  | 43.2                | 27.5                | 61.1                | 40.1                | 27.2                | 60.4                | 41.7                | 25.5                | 61.2                |
|                       | permutation_bonf | 43.1                | 26.6                | 59.8                | 39.4                | 26.9                | 60.9                | 41.1                | 26.2                | 60.8                |
| exp prop continuous   | asymptotic       | 39.2                | 25.7                | 54.0                | 38.9                | 23.2                | 55.4                | 38.2                | 25.3                | 54.5                |
|                       | asymptotic_bonf  | 38.6                | 25.2                | 53.6                | 38.2                | 22.7                | 54.3                | 37.5                | 24.9                | 53.7                |
|                       | permutation_bonf | 38.8                | 24.9                | 54.2                | 37.7                | 23.3                | 53.7                | 36.3                | 24.2                | 53.5                |
| exp prop discrete     | asymptotic       | 42.5                | 27.2                | 58.8                | 41.7                | 25.9                | 59.0                | 42.1                | 27.9                | 58.0                |
|                       | asymptotic_bonf  | 42.2                | 26.5                | 57.7                | 41.3                | 25.5                | 58.1                | 41.3                | 27.3                | 57.7                |
|                       | permutation_bonf | 42.1                | 27.4                | 59.0                | 41.2                | 25.4                | 58.1                | 41.1                | 27.4                | 58.4                |
| logn continuous       | asymptotic       | 79.1                | 58.9                | 90.4                | 80.5                | 60.4                | 92.0                | 80.1                | 59.4                | 91.9                |
|                       | asymptotic_bonf  | 78.9                | 58.3                | 90.4                | 79.9                | 60.1                | 91.7                | 79.8                | 58.9                | 91.7                |
|                       | permutation_bonf | 78.3                | 58.4                | 90.9                | 78.7                | 59.6                | 90.8                | 79.2                | 59.2                | 91.6                |
| logn discrete         | asymptotic       | 86.8                | 67.4                | 95.6                | 87.4                | 71.7                | 96.5                | 85.8                | 69.6                | 95.6                |
|                       | asymptotic_bonf  | 86.4                | 67.1                | 95.5                | 86.7                | 71.3                | 96.3                | 85.5                | 69.5                | 95.5                |
|                       | permutation_bonf | 86.7                | 67.4                | 95.4                | 86.6                | 70.0                | 95.7                | 85.8                | 69.1                | 94.9                |
| pwExp continuous      | asymptotic       | 36.8                | 24.1                | 54.6                | 35.0                | 23.8                | 55.4                | 37.3                | 23.1                | 55.9                |
|                       | asymptotic_bonf  | 36.2                | 23.7                | 54.3                | 34.2                | 23.3                | 54.7                | 36.5                | 22.4                | 55.2                |
|                       | permutation_bonf | 35.9                | 24.1                | 53.2                | 35.1                | 22.8                | 54.4                | 36.6                | 23.0                | 54.5                |
| pwExp discrete        | asymptotic       | 41.4                | 25.8                | 58.2                | 38.7                | 25.9                | 59.2                | 40.0                | 26.4                | 59.8                |
|                       | asymptotic_bonf  | 40.6                | 25.2                | 57.5                | 38.1                | 25.5                | 58.8                | 39.6                | 26.1                | 59.1                |
|                       | permutation_bonf | 40.7                | 25.8                | 58.3                | 38.5                | 26.0                | 59.2                | 39.1                | 25.7                | 58.6                |
| Weib late continuous  | asymptotic       | 78.5                | 60.1                | 93.5                | 78.6                | 59.4                | 91.1                | 78.3                | 60.4                | 91.8                |
|                       | asymptotic_bonf  | 77.6                | 59.3                | 93.3                | 78.1                | 58.8                | 90.9                | 77.7                | 59.8                | 91.6                |
|                       | permutation_bonf | 76.4                | 59.3                | 92.7                | 78.6                | 59.3                | 90.9                | 77.9                | 59.3                | 90.8                |
| Weib late discrete    | asymptotic       | 84.6                | 67.8                | 96.4                | 85.0                | 67.5                | 95.8                | 85.2                | 70.9                | 95.9                |
|                       | asymptotic_bonf  | 84.1                | 67.2                | 96.4                | 84.8                | 67.1                | 95.7                | 84.8                | 70.4                | 95.8                |
|                       | permutation_bonf | 83.0                | 66.7                | 96.2                | 85.5                | 67.2                | 95.1                | 84.3                | 69.9                | 95.5                |
| Weib prop continuous  | asymptotic       | 76.8                | 59.3                | 92.4                | 77.2                | 58.7                | 90.6                | 77.9                | 59.5                | 91.5                |
|                       | asymptotic_bonf  | 76.4                | 58.7                | 92.2                | 77.0                | 57.7                | 90.3                | 77.6                | 58.5                | 91.2                |
|                       | permutation_bonf | 76.5                | 58.7                | 92.0                | 77.6                | 58.1                | 90.7                | 77.6                | 58.5                | 91.2                |
| Weib prop discrete    | asymptotic       | 84.0                | 66.8                | 96.0                | 84.5                | 67.0                | 95.6                | 84.4                | 69.2                | 95.2                |
|                       | asymptotic_bonf  | 83.8                | 66.5                | 95.9                | 84.5                | 66.7                | 95.5                | 84.0                | 68.8                | 95.2                |
|                       | permutation_bonf | 83.3                | 66.0                | 95.9                | 85.3                | 66.5                | 94.8                | 84.0                | 68.7                | 94.8                |
| Weib scale continuous | asymptotic       | 74.1                | 56.7                | 90.6                | 75.2                | 56.2                | 89.4                | 73.8                | 56.9                | 88.9                |
|                       | asymptotic_bonf  | 73.2                | 56.0                | 90.4                | 75.0                | 55.4                | 89.1                | 73.2                | 56.4                | 88.6                |
|                       | permutation_bonf | 72.3                | 55.7                | 89.8                | 74.1                | 54.7                | 88.5                | 73.1                | 56.6                | 89.0                |
| Weib scale discrete   | asymptotic       | 81.2                | 64.8                | 95.0                | 82.6                | 64.2                | 93.6                | 82.6                | 66.4                | 93.6                |
|                       | asymptotic_bonf  | 80.8                | 64.3                | 94.7                | 82.3                | 63.7                | 93.3                | 82.2                | 65.8                | 93.5                |
|                       | permutation_bonf | 80.6                | 63.8                | 94.0                | 81.7                | 63.9                | 92.9                | 81.9                | 66.8                | 93.4                |
| Weib shape continuous | asymptotic       | 70.9                | 53.9                | 88.3                | 71.6                | 52.8                | 87.0                | 72.3                | 53.2                | 86.9                |
|                       | asymptotic_bonf  | 70.4                | 53.3                | 87.8                | 71.0                | 52.3                | 86.8                | 71.8                | 52.7                | 86.9                |
|                       | permutation_bonf | 70.4                | 53.2                | 88.3                | 71.6                | 52.4                | 86.2                | 71.4                | 53.2                | 86.4                |
| Weib shape discrete   | asymptotic       | 78.9                | 63.0                | 92.0                | 79.3                | 62.1                | 92.2                | 80.4                | 62.7                | 91.8                |
|                       | asymptotic_bonf  | 78.5                | 62.5                | 91.9                | 78.9                | 61.9                | 92.0                | 80.0                | 62.2                | 91.5                |
|                       | permutation_bonf | 77.9                | 61.7                | 92.0                | 80.3                | 61.1                | 92.3                | 79.8                | 62.7                | 91.5                |

Table S44: Rejection rates in percent for the 2-by-2 design with  $\delta = 1.5$  and balanced medium sample sizes under unequal, high censoring.

| Distribution          | Method           | $\mathcal{H}_{0,4}$ | $\mathcal{H}_{0,5}$ | $\mathcal{H}_{0,6}$ | $\mathcal{H}_{0,1}$ | $\mathcal{H}_{0,2}$ | $\mathcal{H}_{0,3}$ | $\mathcal{H}_{0,7}$ | $\mathcal{H}_{0,8}$ | $\mathcal{H}_{0,9}$ |
|-----------------------|------------------|---------------------|---------------------|---------------------|---------------------|---------------------|---------------------|---------------------|---------------------|---------------------|
| exp early continuous  | asymptotic       | 4.7                 | 3.9                 | 6.9                 | 5.2                 | 2.9                 | 8.4                 | 5.6                 | 2.5                 | 7.0                 |
|                       | asymptotic_bonf  | 4.5                 | 3.6                 | 6.6                 | 5.0                 | 2.8                 | 8.1                 | 5.3                 | 2.4                 | 6.9                 |
|                       | permutation_bonf | 4.9                 | 3.8                 | 7.3                 | 4.6                 | 2.8                 | 8.3                 | 5.4                 | 2.6                 | 6.4                 |
| exp early discrete    | asymptotic       | 6.7                 | 3.9                 | 7.7                 | 5.4                 | 3.3                 | 8.8                 | 5.8                 | 2.7                 | 8.0                 |
|                       | asymptotic_bonf  | 6.3                 | 3.8                 | 7.7                 | 5.3                 | 3.2                 | 8.5                 | 5.6                 | 2.5                 | 7.7                 |
|                       | permutation_bonf | 5.8                 | 4.1                 | 7.7                 | 5.4                 | 4.2                 | 8.7                 | 5.6                 | 2.2                 | 7.3                 |
| exp late continuous   | asymptotic       | 5.1                 | 3.7                 | 7.2                 | 4.7                 | 3.4                 | 8.7                 | 5.4                 | 3.0                 | 7.2                 |
|                       | asymptotic_bonf  | 4.7                 | 3.6                 | 7.0                 | 4.5                 | 3.1                 | 8.5                 | 5.3                 | 3.0                 | 6.6                 |
|                       | permutation_bonf | 5.0                 | 3.8                 | 7.6                 | 4.4                 | 2.9                 | 8.6                 | 5.0                 | 2.8                 | 6.0                 |
| exp late discrete     | asymptotic       | 6.4                 | 4.3                 | 7.8                 | 5.7                 | 3.7                 | 8.9                 | 6.3                 | 2.6                 | 8.4                 |
|                       | asymptotic_bonf  | 6.1                 | 3.8                 | 7.6                 | 5.4                 | 3.6                 | 8.8                 | 5.9                 | 2.5                 | 8.0                 |
|                       | permutation_bonf | 5.9                 | 3.8                 | 7.9                 | 5.2                 | 3.6                 | 8.3                 | 5.9                 | 2.4                 | 7.1                 |
| exp prop continuous   | asymptotic       | 6.0                 | 4.7                 | 7.4                 | 4.9                 | 3.4                 | 6.2                 | 4.8                 | 4.0                 | 7.2                 |
|                       | asymptotic_bonf  | 5.9                 | 4.4                 | 7.1                 | 4.7                 | 3.2                 | 6.2                 | 4.5                 | 3.9                 | 6.8                 |
|                       | permutation_bonf | 5.2                 | 4.1                 | 6.8                 | 5.3                 | 3.1                 | 6.2                 | 4.7                 | 3.7                 | 7.1                 |
| exp prop discrete     | asymptotic       | 5.9                 | 5.3                 | 8.4                 | 5.0                 | 4.2                 | 7.3                 | 5.3                 | 4.1                 | 7.7                 |
|                       | asymptotic_bonf  | 5.7                 | 5.1                 | 8.1                 | 4.8                 | 4.0                 | 7.0                 | 5.0                 | 4.0                 | 7.7                 |
|                       | permutation_bonf | 6.2                 | 5.4                 | 8.2                 | 5.7                 | 4.4                 | 6.5                 | 4.8                 | 3.9                 | 8.4                 |
| logn continuous       | asymptotic       | 12.0                | 7.8                 | 20.3                | 12.6                | 7.4                 | 18.5                | 14.0                | 8.0                 | 19.2                |
|                       | asymptotic_bonf  | 11.2                | 7.5                 | 19.8                | 12.5                | 7.3                 | 17.8                | 13.7                | 7.5                 | 18.6                |
|                       | permutation_bonf | 11.2                | 7.5                 | 18.9                | 12.3                | 7.0                 | 17.6                | 12.6                | 8.1                 | 17.7                |
| logn discrete         | asymptotic       | 13.2                | 9.7                 | 23.5                | 14.3                | 8.9                 | 22.8                | 15.9                | 10.0                | 23.3                |
|                       | asymptotic_bonf  | 12.9                | 9.7                 | 22.8                | 14.0                | 8.8                 | 21.7                | 15.4                | 9.4                 | 22.7                |
|                       | permutation_bonf | 12.7                | 9.8                 | 22.8                | 15.0                | 8.6                 | 22.4                | 15.9                | 9.9                 | 22.4                |
| pwExp continuous      | asymptotic       | 4.4                 | 3.8                 | 7.1                 | 4.5                 | 3.5                 | 7.8                 | 5.5                 | 2.7                 | 6.8                 |
|                       | asymptotic_bonf  | 4.4                 | 3.7                 | 6.7                 | 4.1                 | 3.4                 | 7.3                 | 5.4                 | 2.6                 | 6.8                 |
|                       | permutation_bonf | 4.6                 | 4.3                 | 6.8                 | 3.8                 | 3.3                 | 7.1                 | 5.6                 | 2.5                 | 6.9                 |
| pwExp discrete        | asymptotic       | 5.8                 | 3.8                 | 8.2                 | 4.8                 | 3.9                 | 8.7                 | 6.3                 | 2.3                 | 8.0                 |
|                       | asymptotic_bonf  | 5.7                 | 3.8                 | 8.1                 | 4.8                 | 3.8                 | 8.5                 | 5.9                 | 2.2                 | 8.0                 |
|                       | permutation_bonf | 5.6                 | 3.9                 | 7.6                 | 4.8                 | 3.4                 | 8.0                 | 5.6                 | 2.3                 | 7.8                 |
| Weib late continuous  | asymptotic       | 11.2                | 7.5                 | 20.7                | 12.1                | 8.6                 | 19.4                | 12.1                | 7.8                 | 19.7                |
|                       | asymptotic_bonf  | 10.9                | 7.4                 | 20.4                | 11.7                | 8.5                 | 18.8                | 12.0                | 7.7                 | 19.0                |
|                       | permutation_bonf | 10.8                | 6.8                 | 20.0                | 11.7                | 8.4                 | 18.0                | 11.5                | 7.6                 | 18.5                |
| Weib late discrete    | asymptotic       | 13.2                | 8.5                 | 24.3                | 14.6                | 8.9                 | 23.2                | 13.7                | 8.9                 | 22.3                |
|                       | asymptotic_bonf  | 13.0                | 7.8                 | 23.6                | 14.2                | 8.8                 | 22.7                | 13.4                | 8.5                 | 21.9                |
|                       | permutation_bonf | 12.8                | 8.4                 | 22.4                | 13.8                | 8.8                 | 22.1                | 13.3                | 9.1                 | 22.7                |
| Weib prop continuous  | asymptotic       | 11.1                | 6.7                 | 20.1                | 11.6                | 8.5                 | 18.9                | 12.2                | 7.8                 | 19.1                |
|                       | asymptotic_bonf  | 10.6                | 6.6                 | 19.8                | 10.9                | 8.5                 | 18.4                | 11.7                | 7.8                 | 18.8                |
|                       | permutation_bonf | 10.4                | 6.9                 | 19.0                | 11.3                | 7.9                 | 18.0                | 10.8                | 7.9                 | 18.0                |
| Weib prop discrete    | asymptotic       | 13.5                | 8.0                 | 24.2                | 15.4                | 9.0                 | 23.8                | 13.7                | 9.6                 | 22.9                |
|                       | asymptotic_bonf  | 13.1                | 7.6                 | 23.5                | 14.8                | 8.4                 | 23.0                | 13.4                | 9.3                 | 22.4                |
|                       | permutation_bonf | 12.4                | 7.8                 | 23.4                | 14.7                | 9.0                 | 22.0                | 12.6                | 8.9                 | 22.9                |
| Weib scale continuous | asymptotic       | 9.9                 | 6.8                 | 17.9                | 11.4                | 7.1                 | 16.1                | 10.5                | 6.7                 | 17.8                |
|                       | asymptotic_bonf  | 9.8                 | 6.5                 | 17.6                | 11.1                | 6.8                 | 15.8                | 10.0                | 6.5                 | 17.2                |
|                       | permutation_bonf | 9.7                 | 6.4                 | 16.8                | 11.0                | 7.1                 | 15.9                | 10.2                | 6.7                 | 16.5                |
| Weib scale discrete   | asymptotic       | 12.6                | 7.5                 | 22.0                | 13.0                | 8.1                 | 21.7                | 12.7                | 8.0                 | 20.7                |
|                       | asymptotic_bonf  | 12.4                | 7.2                 | 21.9                | 12.7                | 8.0                 | 21.1                | 12.2                | 8.0                 | 20.4                |
|                       | permutation_bonf | 12.1                | 7.4                 | 21.4                | 12.7                | 8.5                 | 20.1                | 12.3                | 8.8                 | 19.3                |
| Weib shape continuous | asymptotic       | 9.7                 | 6.0                 | 16.6                | 9.0                 | 6.9                 | 14.7                | 9.9                 | 6.0                 | 17.0                |
|                       | asymptotic_bonf  | 9.3                 | 5.7                 | 16.2                | 8.7                 | 6.6                 | 14.5                | 9.8                 | 5.9                 | 16.2                |
|                       | permutation_bonf | 9.4                 | 5.7                 | 16.0                | 9.1                 | 6.4                 | 14.2                | 9.7                 | 6.7                 | 15.3                |
| Weib shape discrete   | asymptotic       | 10.4                | 7.1                 | 20.2                | 11.2                | 7.0                 | 18.4                | 11.5                | 7.3                 | 19.7                |
|                       | asymptotic_bonf  | 10.2                | 6.5                 | 19.8                | 11.0                | 6.8                 | 18.1                | 11.1                | 7.2                 | 19.3                |
|                       | permutation_bonf | 10.6                | 6.8                 | 20.0                | 10.5                | 7.2                 | 17.3                | 10.7                | 7.3                 | 19.1                |

Table S45: Rejection rates in percent for the 2-by-2 design with  $\delta = 1.5$  and balanced small sample sizes under unequal, high censoring.

| Distribution          | Method           | $\mathcal{H}_{0,4}$ | $\mathcal{H}_{0,5}$ | $\mathcal{H}_{0,6}$ | $\mathcal{H}_{0,1}$ | $\mathcal{H}_{0,2}$ | $\mathcal{H}_{0,3}$ | $\mathcal{H}_{0,7}$ | $\mathcal{H}_{0,8}$ | $\mathcal{H}_{0,9}$ |
|-----------------------|------------------|---------------------|---------------------|---------------------|---------------------|---------------------|---------------------|---------------------|---------------------|---------------------|
| exp early continuous  | asymptotic       | 1.3                 | 1.1                 | 1.9                 | 2.0                 | 1.0                 | 1.7                 | 1.5                 | 1.5                 | 1.5                 |
|                       | asymptotic_bonf  | 1.3                 | 1.1                 | 1.7                 | 2.0                 | 1.0                 | 1.7                 | 1.4                 | 1.3                 | 1.4                 |
|                       | permutation_bonf | 1.2                 | 1.1                 | 1.7                 | 1.6                 | 0.5                 | 1.0                 | 1.1                 | 1.3                 | 1.2                 |
| exp early discrete    | asymptotic       | 1.5                 | 1.0                 | 1.7                 | 0.7                 | 1.2                 | 1.5                 | 1.1                 | 1.1                 | 2.1                 |
|                       | asymptotic_bonf  | 1.4                 | 0.9                 | 1.3                 | 0.7                 | 1.2                 | 1.3                 | 1.1                 | 1.1                 | 2.1                 |
|                       | permutation_bonf | 1.3                 | 1.0                 | 1.4                 | 0.9                 | 1.1                 | 1.0                 | 1.0                 | 0.9                 | 1.3                 |
| exp late continuous   | asymptotic       | 1.1                 | 1.1                 | 2.2                 | 2.1                 | 0.9                 | 1.3                 | 2.2                 | 1.4                 | 1.8                 |
|                       | asymptotic_bonf  | 1.1                 | 1.1                 | 2.1                 | 2.0                 | 0.9                 | 1.3                 | 2.0                 | 1.3                 | 1.7                 |
|                       | permutation_bonf | 1.1                 | 1.0                 | 1.9                 | 1.7                 | 0.5                 | 1.1                 | 1.6                 | 1.0                 | 1.4                 |
| exp late discrete     | asymptotic       | 1.5                 | 1.4                 | 2.3                 | 2.2                 | 1.0                 | 1.7                 | 1.6                 | 0.8                 | 1.6                 |
|                       | asymptotic_bonf  | 1.2                 | 1.0                 | 2.3                 | 2.2                 | 1.0                 | 1.6                 | 1.6                 | 0.7                 | 1.4                 |
|                       | permutation_bonf | 0.9                 | 1.2                 | 1.7                 | 1.8                 | 1.0                 | 1.3                 | 1.3                 | 0.6                 | 1.3                 |
| exp prop continuous   | asymptotic       | 2.0                 | 1.3                 | 2.0                 | 1.0                 | 1.0                 | 1.6                 | 1.1                 | 0.7                 | 1.9                 |
|                       | asymptotic_bonf  | 1.9                 | 1.3                 | 2.0                 | 0.9                 | 1.0                 | 1.5                 | 1.1                 | 0.6                 | 1.7                 |
|                       | permutation_bonf | 1.8                 | 1.0                 | 1.6                 | 0.9                 | 0.6                 | 1.2                 | 1.0                 | 0.6                 | 1.1                 |
| exp prop discrete     | asymptotic       | 1.3                 | 0.7                 | 2.6                 | 1.0                 | 0.7                 | 1.8                 | 1.4                 | 1.4                 | 2.1                 |
|                       | asymptotic_bonf  | 1.3                 | 0.7                 | 2.6                 | 1.0                 | 0.7                 | 1.7                 | 1.4                 | 1.4                 | 2.1                 |
|                       | permutation_bonf | 1.4                 | 0.5                 | 2.3                 | 0.9                 | 0.5                 | 1.6                 | 0.7                 | 1.3                 | 1.6                 |
| logn continuous       | asymptotic       | 2.4                 | 1.5                 | 3.3                 | 3.0                 | 2.4                 | 4.1                 | 2.6                 | 1.6                 | 3.7                 |
|                       | asymptotic_bonf  | 2.4                 | 1.4                 | 3.2                 | 2.8                 | 2.4                 | 4.0                 | 2.5                 | 1.6                 | 3.6                 |
|                       | permutation_bonf | 2.5                 | 1.4                 | 3.2                 | 2.6                 | 1.9                 | 2.7                 | 1.9                 | 1.5                 | 3.2                 |
| logn discrete         | asymptotic       | 2.7                 | 1.7                 | 4.1                 | 3.6                 | 3.5                 | 5.3                 | 2.9                 | 2.1                 | 3.7                 |
|                       | asymptotic_bonf  | 2.7                 | 1.7                 | 3.8                 | 3.5                 | 3.3                 | 5.3                 | 2.7                 | 2.0                 | 3.7                 |
|                       | permutation_bonf | 2.9                 | 1.6                 | 3.6                 | 3.3                 | 2.9                 | 4.1                 | 2.3                 | 1.8                 | 3.2                 |
| pwExp continuous      | asymptotic       | 1.3                 | 1.3                 | 1.7                 | 1.7                 | 1.0                 | 1.4                 | 2.1                 | 1.4                 | 1.6                 |
|                       | asymptotic_bonf  | 1.2                 | 1.1                 | 1.7                 | 1.6                 | 1.0                 | 1.3                 | 2.1                 | 1.3                 | 1.6                 |
|                       | permutation_bonf | 1.1                 | 1.2                 | 1.8                 | 1.5                 | 0.7                 | 1.0                 | 1.7                 | 1.1                 | 1.6                 |
| pwExp discrete        | asymptotic       | 1.5                 | 1.3                 | 2.2                 | 2.0                 | 1.1                 | 1.4                 | 2.0                 | 1.6                 | 1.5                 |
|                       | asymptotic_bonf  | 1.5                 | 1.3                 | 2.0                 | 1.9                 | 1.1                 | 1.1                 | 1.8                 | 1.3                 | 1.5                 |
|                       | permutation_bonf | 0.9                 | 1.2                 | 2.1                 | 1.6                 | 0.9                 | 1.0                 | 1.2                 | 0.8                 | 1.2                 |
| Weib late continuous  | asymptotic       | 2.2                 | 2.2                 | 3.3                 | 2.1                 | 2.1                 | 2.8                 | 3.1                 | 2.2                 | 4.1                 |
|                       | asymptotic_bonf  | 2.2                 | 2.2                 | 3.2                 | 2.1                 | 2.1                 | 2.8                 | 3.1                 | 2.2                 | 4.0                 |
|                       | permutation_bonf | 1.8                 | 2.3                 | 2.9                 | 1.6                 | 1.9                 | 2.0                 | 2.5                 | 2.2                 | 3.2                 |
| Weib late discrete    | asymptotic       | 2.1                 | 2.6                 | 3.6                 | 1.8                 | 2.8                 | 3.2                 | 3.5                 | 2.5                 | 4.1                 |
|                       | asymptotic_bonf  | 2.1                 | 2.5                 | 3.4                 | 1.7                 | 2.8                 | 3.0                 | 3.4                 | 2.3                 | 3.8                 |
|                       | permutation_bonf | 2.0                 | 2.5                 | 3.2                 | 1.9                 | 2.1                 | 2.6                 | 3.1                 | 2.1                 | 3.1                 |
| Weib prop continuous  | asymptotic       | 2.5                 | 1.8                 | 3.1                 | 2.1                 | 2.3                 | 2.7                 | 2.9                 | 2.2                 | 3.8                 |
|                       | asymptotic_bonf  | 2.5                 | 1.8                 | 3.1                 | 2.1                 | 2.2                 | 2.3                 | 2.9                 | 2.2                 | 3.8                 |
|                       | permutation_bonf | 1.9                 | 2.2                 | 3.0                 | 1.9                 | 1.9                 | 2.0                 | 2.6                 | 2.2                 | 3.5                 |
| Weib prop discrete    | asymptotic       | 2.3                 | 2.4                 | 4.1                 | 1.9                 | 2.6                 | 3.1                 | 3.3                 | 2.3                 | 3.7                 |
|                       | asymptotic_bonf  | 2.1                 | 2.3                 | 4.0                 | 1.8                 | 2.5                 | 3.1                 | 3.2                 | 2.2                 | 3.6                 |
|                       | permutation_bonf | 1.9                 | 2.3                 | 3.5                 | 1.7                 | 2.1                 | 2.5                 | 3.2                 | 2.0                 | 3.3                 |
| Weib scale continuous | asymptotic       | 1.6                 | 1.8                 | 3.1                 | 2.0                 | 2.3                 | 2.3                 | 2.9                 | 2.4                 | 2.6                 |
|                       | asymptotic_bonf  | 1.5                 | 1.8                 | 3.0                 | 1.9                 | 2.2                 | 2.1                 | 2.8                 | 2.0                 | 2.4                 |
|                       | permutation_bonf | 1.4                 | 1.7                 | 2.4                 | 1.5                 | 2.0                 | 1.9                 | 2.3                 | 1.8                 | 2.1                 |
| Weib scale discrete   | asymptotic       | 1.6                 | 2.1                 | 3.9                 | 1.7                 | 2.6                 | 2.7                 | 2.9                 | 2.0                 | 3.1                 |
|                       | asymptotic_bonf  | 1.5                 | 1.8                 | 3.6                 | 1.7                 | 2.6                 | 2.7                 | 2.9                 | 1.9                 | 3.1                 |
|                       | permutation_bonf | 1.6                 | 1.7                 | 3.1                 | 1.6                 | 2.0                 | 2.3                 | 2.4                 | 1.9                 | 2.4                 |
| Weib shape continuous | asymptotic       | 1.2                 | 1.6                 | 2.9                 | 1.1                 | 1.8                 | 1.9                 | 2.6                 | 1.8                 | 2.9                 |
|                       | asymptotic_bonf  | 1.2                 | 1.6                 | 2.9                 | 1.1                 | 1.8                 | 1.9                 | 2.4                 | 1.5                 | 2.8                 |
|                       | permutation_bonf | 1.2                 | 1.2                 | 2.4                 | 1.2                 | 1.6                 | 1.6                 | 2.1                 | 1.6                 | 2.3                 |
| Weib shape discrete   | asymptotic       | 1.5                 | 1.9                 | 3.5                 | 1.3                 | 2.2                 | 2.1                 | 2.8                 | 1.9                 | 2.9                 |
|                       | asymptotic_bonf  | 1.4                 | 1.9                 | 3.3                 | 1.3                 | 2.2                 | 2.0                 | 2.8                 | 1.8                 | 2.9                 |
|                       | permutation_bonf | 1.1                 | 1.9                 | 2.8                 | 1.3                 | 2.1                 | 1.8                 | 2.3                 | 1.8                 | 2.2                 |

Table S46: Rejection rates in percent for the 2-by-2 design with  $\delta = 1.5$  and unbalanced large sample sizes under unequal, high censoring.

| Distribution          | Method           | $\mathcal{H}_{0,4}$ | $\mathcal{H}_{0,5}$ | $\mathcal{H}_{0,6}$ | $\mathcal{H}_{0,1}$ | $\mathcal{H}_{0,2}$ | $\mathcal{H}_{0,3}$ | $\mathcal{H}_{0,7}$ | $\mathcal{H}_{0,8}$ | $\mathcal{H}_{0,9}$ |
|-----------------------|------------------|---------------------|---------------------|---------------------|---------------------|---------------------|---------------------|---------------------|---------------------|---------------------|
| exp early continuous  | asymptotic       | 18.8                | 10.8                | 29.9                | 17.8                | 9.9                 | 31.3                | 18.3                | 10.7                | 29.0                |
|                       | asymptotic_bonf  | 18.0                | 10.2                | 28.7                | 17.1                | 9.1                 | 29.2                | 17.3                | 9.5                 | 27.8                |
|                       | permutation_bonf | 17.7                | 9.6                 | 29.8                | 16.7                | 9.1                 | 27.9                | 17.1                | 9.1                 | 27.0                |
| exp early discrete    | asymptotic       | 20.6                | 12.1                | 34.5                | 18.7                | 11.7                | 32.2                | 20.7                | 12.0                | 30.9                |
|                       | asymptotic_bonf  | 19.3                | 11.6                | 32.9                | 17.5                | 11.1                | 30.9                | 19.5                | 11.1                | 29.6                |
|                       | permutation_bonf | 19.4                | 10.9                | 32.8                | 17.0                | 10.2                | 30.3                | 18.8                | 10.4                | 29.3                |
| exp late continuous   | asymptotic       | 18.9                | 11.7                | 32.4                | 18.8                | 11.2                | 31.5                | 18.9                | 10.8                | 30.8                |
|                       | asymptotic_bonf  | 18.3                | 10.9                | 31.2                | 17.5                | 10.6                | 30.1                | 17.9                | 9.6                 | 29.5                |
|                       | permutation_bonf | 18.5                | 10.3                | 30.7                | 16.6                | 10.2                | 29.2                | 18.2                | 9.0                 | 30.0                |
| exp late discrete     | asymptotic       | 21.4                | 12.4                | 37.4                | 20.6                | 12.8                | 34.4                | 21.1                | 12.8                | 32.6                |
|                       | asymptotic_bonf  | 19.7                | 11.6                | 35.8                | 19.2                | 12.1                | 32.9                | 19.5                | 11.6                | 30.5                |
|                       | permutation_bonf | 19.7                | 10.5                | 35.1                | 18.5                | 11.3                | 32.9                | 20.2                | 11.4                | 30.5                |
| exp prop continuous   | asymptotic       | 19.5                | 12.4                | 26.1                | 16.8                | 10.2                | 29.8                | 19.1                | 12.8                | 28.3                |
|                       | asymptotic_bonf  | 18.4                | 11.2                | 24.7                | 15.3                | 9.1                 | 28.5                | 17.9                | 12.0                | 26.8                |
|                       | permutation_bonf | 19.0                | 10.1                | 23.8                | 15.2                | 8.5                 | 28.0                | 17.1                | 11.0                | 26.0                |
| exp prop discrete     | asymptotic       | 21.4                | 15.1                | 30.4                | 18.0                | 11.0                | 34.1                | 20.3                | 14.1                | 30.1                |
|                       | asymptotic_bonf  | 20.6                | 13.8                | 28.6                | 16.8                | 10.3                | 32.1                | 19.5                | 13.9                | 28.9                |
|                       | permutation_bonf | 19.9                | 13.2                | 27.6                | 17.5                | 10.0                | 31.2                | 19.4                | 12.6                | 28.5                |
| logn continuous       | asymptotic       | 49.8                | 29.3                | 61.5                | 48.5                | 32.8                | 63.7                | 47.1                | 32.3                | 62.1                |
|                       | asymptotic_bonf  | 48.2                | 27.0                | 59.7                | 46.5                | 30.8                | 61.5                | 45.0                | 30.2                | 60.3                |
|                       | permutation_bonf | 46.3                | 26.6                | 58.1                | 45.4                | 29.4                | 60.3                | 44.5                | 29.3                | 60.0                |
| logn discrete         | asymptotic       | 58.5                | 35.9                | 69.4                | 55.1                | 39.5                | 70.5                | 53.0                | 36.1                | 70.0                |
|                       | asymptotic_bonf  | 56.1                | 34.2                | 67.2                | 54.0                | 37.3                | 69.4                | 51.6                | 34.7                | 68.7                |
|                       | permutation_bonf | 54.7                | 31.3                | 66.5                | 51.5                | 35.4                | 68.4                | 50.4                | 32.9                | 67.0                |
| pwExp continuous      | asymptotic       | 16.4                | 9.8                 | 29.9                | 17.4                | 9.2                 | 31.5                | 17.3                | 10.7                | 30.1                |
|                       | asymptotic_bonf  | 15.9                | 9.1                 | 28.1                | 16.2                | 7.9                 | 30.4                | 16.0                | 9.9                 | 28.1                |
|                       | permutation_bonf | 16.0                | 9.2                 | 29.1                | 17.0                | 9.3                 | 29.6                | 16.0                | 9.2                 | 27.5                |
| pwExp discrete        | asymptotic       | 20.2                | 10.8                | 33.7                | 18.8                | 11.8                | 32.7                | 18.5                | 11.0                | 32.1                |
|                       | asymptotic_bonf  | 19.1                | 10.2                | 32.5                | 17.3                | 10.0                | 31.5                | 17.6                | 10.1                | 30.4                |
|                       | permutation_bonf | 17.8                | 9.6                 | 31.4                | 16.9                | 9.9                 | 31.2                | 17.5                | 9.5                 | 30.5                |
| Weib late continuous  | asymptotic       | 47.8                | 31.5                | 65.3                | 48.6                | 29.4                | 67.2                | 46.5                | 28.5                | 65.8                |
|                       | asymptotic_bonf  | 46.1                | 29.3                | 63.5                | 47.5                | 27.8                | 65.6                | 44.7                | 27.5                | 64.0                |
|                       | permutation_bonf | 44.9                | 26.3                | 62.1                | 45.3                | 26.0                | 64.6                | 42.6                | 27.0                | 63.0                |
| Weib late discrete    | asymptotic       | 53.8                | 34.5                | 72.2                | 52.6                | 33.5                | 71.9                | 53.8                | 33.2                | 70.4                |
|                       | asymptotic_bonf  | 51.3                | 32.7                | 71.3                | 50.9                | 32.0                | 70.5                | 52.0                | 31.2                | 68.4                |
|                       | permutation_bonf | 49.8                | 31.2                | 69.2                | 48.6                | 30.3                | 69.8                | 50.8                | 30.7                | 68.2                |
| Weib prop continuous  | asymptotic       | 46.2                | 28.2                | 63.9                | 46.0                | 28.2                | 65.2                | 43.6                | 28.6                | 63.3                |
|                       | asymptotic_bonf  | 43.8                | 26.9                | 61.1                | 44.5                | 25.8                | 63.1                | 41.5                | 27.1                | 61.2                |
|                       | permutation_bonf | 42.7                | 25.0                | 59.4                | 43.7                | 25.3                | 60.9                | 41.8                | 26.7                | 61.0                |
| Weib prop discrete    | asymptotic       | 53.8                | 33.6                | 72.6                | 53.1                | 34.7                | 72.2                | 53.9                | 33.9                | 71.1                |
|                       | asymptotic_bonf  | 51.6                | 31.6                | 71.1                | 51.8                | 33.1                | 71.2                | 50.9                | 32.2                | 69.6                |
|                       | permutation_bonf | 50.1                | 30.6                | 69.2                | 49.4                | 30.7                | 70.8                | 48.8                | 30.6                | 68.9                |
| Weib scale continuous | asymptotic       | 40.2                | 25.9                | 57.2                | 41.9                | 25.0                | 60.0                | 39.8                | 25.8                | 56.9                |
|                       | asymptotic_bonf  | 37.2                | 23.6                | 55.2                | 40.3                | 23.3                | 58.2                | 37.4                | 24.0                | 54.8                |
|                       | permutation_bonf | 36.7                | 22.6                | 54.1                | 37.8                | 21.2                | 56.3                | 36.7                | 22.4                | 54.7                |
| Weib scale discrete   | asymptotic       | 46.7                | 29.9                | 65.3                | 48.2                | 30.4                | 66.5                | 46.5                | 29.9                | 64.1                |
|                       | asymptotic_bonf  | 44.6                | 27.5                | 63.4                | 45.9                | 28.6                | 64.6                | 43.6                | 28.6                | 61.7                |
|                       | permutation_bonf | 43.4                | 25.3                | 61.5                | 43.7                | 27.0                | 62.4                | 43.4                | 27.3                | 61.3                |
| Weib shape continuous | asymptotic       | 35.1                | 22.3                | 50.5                | 36.0                | 21.5                | 53.2                | 33.6                | 22.9                | 50.7                |
|                       | asymptotic_bonf  | 33.2                | 20.5                | 48.0                | 33.7                | 19.8                | 50.8                | 31.3                | 20.5                | 49.0                |
|                       | permutation_bonf | 32.0                | 20.0                | 47.2                | 31.8                | 18.9                | 50.4                | 30.4                | 19.3                | 47.9                |
| Weib shape discrete   | asymptotic       | 41.0                | 26.0                | 58.3                | 42.4                | 26.4                | 59.3                | 41.4                | 25.6                | 58.0                |
|                       | asymptotic_bonf  | 38.6                | 23.7                | 55.9                | 40.0                | 25.1                | 57.2                | 38.7                | 24.4                | 55.3                |
|                       | permutation_bonf | 37.3                | 22.7                | 54.7                | 37.3                | 23.5                | 56.6                | 37.3                | 23.9                | 55.4                |

Table S47: Rejection rates in percent for the 2-by-2 design with  $\delta = 1.5$  and unbalanced medium sample sizes under unequal, high censoring.

| Distribution          | Method           | $\mathcal{H}_{0,4}$ | $\mathcal{H}_{0,5}$ | $\mathcal{H}_{0,6}$ | $\mathcal{H}_{0,1}$ | $\mathcal{H}_{0,2}$ | $\mathcal{H}_{0,3}$ | $\mathcal{H}_{0,7}$ | $\mathcal{H}_{0,8}$ | $\mathcal{H}_{0,9}$ |
|-----------------------|------------------|---------------------|---------------------|---------------------|---------------------|---------------------|---------------------|---------------------|---------------------|---------------------|
| exp early continuous  | asymptotic       | 2.7                 | 1.7                 | 3.8                 | 2.6                 | 1.7                 | 3.6                 | 3.0                 | 1.3                 | 3.9                 |
|                       | asymptotic_bonf  | 2.2                 | 1.4                 | 3.5                 | 2.4                 | 1.2                 | 3.2                 | 2.7                 | 1.3                 | 3.7                 |
|                       | permutation_bonf | 1.6                 | 1.2                 | 3.1                 | 1.8                 | 0.9                 | 2.3                 | 2.0                 | 1.3                 | 3.1                 |
| exp early discrete    | asymptotic       | 3.1                 | 1.7                 | 4.5                 | 2.3                 | 1.4                 | 4.2                 | 2.7                 | 1.4                 | 4.1                 |
|                       | asymptotic_bonf  | 2.9                 | 1.4                 | 3.8                 | 2.2                 | 1.4                 | 4.0                 | 2.6                 | 1.3                 | 3.7                 |
|                       | permutation_bonf | 2.0                 | 1.0                 | 3.2                 | 1.4                 | 0.6                 | 3.1                 | 1.9                 | 1.0                 | 3.5                 |
| exp late continuous   | asymptotic       | 2.2                 | 2.3                 | 4.0                 | 2.6                 | 1.5                 | 3.5                 | 3.2                 | 1.8                 | 3.7                 |
|                       | asymptotic_bonf  | 1.8                 | 2.0                 | 3.7                 | 2.5                 | 1.3                 | 3.4                 | 3.0                 | 1.6                 | 3.5                 |
|                       | permutation_bonf | 1.0                 | 1.6                 | 3.1                 | 1.7                 | 1.1                 | 2.5                 | 2.8                 | 0.8                 | 2.9                 |
| exp late discrete     | asymptotic       | 3.0                 | 2.0                 | 3.8                 | 2.2                 | 1.7                 | 4.7                 | 3.3                 | 1.5                 | 4.3                 |
|                       | asymptotic_bonf  | 2.9                 | 1.8                 | 3.7                 | 2.1                 | 1.4                 | 3.6                 | 2.8                 | 1.2                 | 3.9                 |
|                       | permutation_bonf | 2.0                 | 1.1                 | 3.3                 | 2.0                 | 0.8                 | 3.4                 | 2.1                 | 1.1                 | 4.1                 |
| exp prop continuous   | asymptotic       | 2.7                 | 2.3                 | 3.0                 | 2.2                 | 1.5                 | 3.4                 | 2.5                 | 2.0                 | 3.3                 |
|                       | asymptotic_bonf  | 2.5                 | 2.0                 | 2.7                 | 1.7                 | 1.5                 | 3.3                 | 2.2                 | 1.8                 | 3.2                 |
|                       | permutation_bonf | 2.2                 | 1.3                 | 2.3                 | 1.4                 | 0.6                 | 2.8                 | 1.7                 | 1.0                 | 2.8                 |
| exp prop discrete     | asymptotic       | 3.2                 | 2.3                 | 3.9                 | 2.3                 | 1.4                 | 3.8                 | 2.9                 | 2.8                 | 4.1                 |
|                       | asymptotic_bonf  | 2.8                 | 2.2                 | 3.7                 | 2.1                 | 1.3                 | 3.4                 | 2.5                 | 2.4                 | 3.7                 |
|                       | permutation_bonf | 2.4                 | 1.1                 | 2.8                 | 1.9                 | 0.7                 | 2.9                 | 2.1                 | 1.8                 | 3.0                 |
| logn continuous       | asymptotic       | 5.2                 | 3.4                 | 8.2                 | 3.7                 | 3.4                 | 7.2                 | 5.2                 | 3.8                 | 8.9                 |
|                       | asymptotic_bonf  | 4.8                 | 3.2                 | 7.3                 | 3.5                 | 3.1                 | 6.7                 | 4.1                 | 3.6                 | 8.4                 |
|                       | permutation_bonf | 3.8                 | 1.8                 | 5.0                 | 2.5                 | 1.2                 | 4.8                 | 3.6                 | 2.8                 | 6.7                 |
| logn discrete         | asymptotic       | 6.4                 | 3.8                 | 9.0                 | 5.5                 | 3.4                 | 8.5                 | 5.6                 | 4.4                 | 10.4                |
|                       | asymptotic_bonf  | 6.1                 | 3.6                 | 7.9                 | 4.4                 | 3.0                 | 7.6                 | 4.4                 | 3.7                 | 9.2                 |
|                       | permutation_bonf | 4.1                 | 1.8                 | 6.0                 | 2.7                 | 1.3                 | 5.9                 | 3.6                 | 2.4                 | 7.3                 |
| pwExp continuous      | asymptotic       | 1.4                 | 1.9                 | 4.0                 | 2.6                 | 1.2                 | 3.3                 | 2.2                 | 2.0                 | 3.5                 |
|                       | asymptotic_bonf  | 1.3                 | 1.8                 | 3.9                 | 2.3                 | 1.0                 | 3.0                 | 1.9                 | 1.7                 | 3.1                 |
|                       | permutation_bonf | 1.0                 | 1.5                 | 3.3                 | 1.8                 | 0.7                 | 2.1                 | 1.9                 | 1.2                 | 2.8                 |
| pwExp discrete        | asymptotic       | 2.1                 | 1.9                 | 4.1                 | 2.4                 | 1.4                 | 3.7                 | 2.9                 | 2.2                 | 3.8                 |
|                       | asymptotic_bonf  | 2.0                 | 1.9                 | 3.9                 | 2.2                 | 1.3                 | 3.2                 | 2.6                 | 2.0                 | 3.3                 |
|                       | permutation_bonf | 1.3                 | 1.3                 | 3.6                 | 1.7                 | 0.8                 | 2.8                 | 2.0                 | 1.0                 | 3.1                 |
| Weib late continuous  | asymptotic       | 5.6                 | 3.1                 | 7.8                 | 4.3                 | 2.5                 | 8.5                 | 6.3                 | 3.6                 | 8.0                 |
|                       | asymptotic_bonf  | 4.8                 | 2.6                 | 6.9                 | 3.6                 | 2.3                 | 7.9                 | 5.5                 | 3.2                 | 7.7                 |
|                       | permutation_bonf | 3.7                 | 0.9                 | 5.1                 | 2.2                 | 0.7                 | 6.4                 | 4.3                 | 1.9                 | 6.4                 |
| Weib late discrete    | asymptotic       | 6.6                 | 3.8                 | 9.7                 | 4.6                 | 3.3                 | 10.7                | 6.5                 | 3.5                 | 9.9                 |
|                       | asymptotic_bonf  | 5.9                 | 2.9                 | 8.5                 | 3.9                 | 3.2                 | 9.2                 | 6.0                 | 2.9                 | 8.8                 |
|                       | permutation_bonf | 3.8                 | 1.7                 | 6.0                 | 2.6                 | 1.3                 | 7.1                 | 4.2                 | 1.9                 | 7.8                 |
| Weib prop continuous  | asymptotic       | 4.7                 | 2.7                 | 6.9                 | 4.1                 | 2.5                 | 8.0                 | 5.4                 | 3.0                 | 8.2                 |
|                       | asymptotic_bonf  | 4.3                 | 2.0                 | 6.4                 | 3.5                 | 2.2                 | 7.1                 | 5.0                 | 2.9                 | 7.1                 |
|                       | permutation_bonf | 3.0                 | 0.8                 | 5.0                 | 2.2                 | 0.7                 | 5.6                 | 4.1                 | 1.8                 | 6.0                 |
| Weib prop discrete    | asymptotic       | 5.9                 | 2.9                 | 9.3                 | 4.5                 | 3.3                 | 8.9                 | 6.5                 | 3.4                 | 8.6                 |
|                       | asymptotic_bonf  | 5.3                 | 2.5                 | 8.9                 | 4.0                 | 2.9                 | 8.6                 | 5.6                 | 2.8                 | 8.3                 |
|                       | permutation_bonf | 4.0                 | 0.8                 | 6.2                 | 2.8                 | 0.7                 | 6.0                 | 4.0                 | 1.6                 | 7.0                 |
| Weib scale continuous | asymptotic       | 3.7                 | 2.2                 | 6.0                 | 3.4                 | 2.5                 | 5.7                 | 4.1                 | 2.5                 | 5.7                 |
|                       | asymptotic_bonf  | 3.2                 | 1.9                 | 5.4                 | 2.9                 | 2.1                 | 4.7                 | 3.5                 | 2.2                 | 5.1                 |
|                       | permutation_bonf | 2.7                 | 1.1                 | 3.8                 | 1.8                 | 0.6                 | 3.1                 | 2.8                 | 1.9                 | 4.3                 |
| Weib scale discrete   | asymptotic       | 5.7                 | 2.6                 | 6.4                 | 4.1                 | 2.3                 | 6.8                 | 5.0                 | 2.6                 | 6.8                 |
|                       | asymptotic_bonf  | 4.9                 | 2.3                 | 6.0                 | 3.6                 | 2.0                 | 5.9                 | 4.7                 | 2.4                 | 5.9                 |
|                       | permutation_bonf | 3.3                 | 1.0                 | 3.8                 | 1.9                 | 0.6                 | 3.7                 | 2.9                 | 1.8                 | 5.2                 |
| Weib shape continuous | asymptotic       | 3.8                 | 1.9                 | 4.7                 | 2.8                 | 1.8                 | 4.2                 | 3.3                 | 1.4                 | 4.5                 |
|                       | asymptotic_bonf  | 3.3                 | 1.4                 | 4.5                 | 2.0                 | 1.5                 | 3.8                 | 2.7                 | 1.4                 | 3.7                 |
|                       | permutation_bonf | 2.1                 | 0.7                 | 3.3                 | 1.6                 | 0.6                 | 2.7                 | 2.2                 | 1.0                 | 3.0                 |
| Weib shape discrete   | asymptotic       | 3.7                 | 2.1                 | 4.9                 | 3.1                 | 2.4                 | 5.0                 | 4.4                 | 1.9                 | 4.9                 |
|                       | asymptotic_bonf  | 3.4                 | 1.8                 | 4.1                 | 2.6                 | 1.8                 | 4.8                 | 4.0                 | 1.5                 | 4.2                 |
|                       | permutation_bonf | 2.3                 | 1.0                 | 2.3                 | 1.8                 | 0.5                 | 2.6                 | 2.7                 | 1.2                 | 3.7                 |

Table S48: Rejection rates in percent for the 2-by-2 design with  $\delta = 1.5$  and unbalanced small sample sizes under unequal, high censoring.

| Distribution          | Method           | $\mathcal{H}_{0,4}$ | $\mathcal{H}_{0,5}$ | $\mathcal{H}_{0,6}$ | $\mathcal{H}_{0,1}$ | $\mathcal{H}_{0,2}$ | $\mathcal{H}_{0,3}$ | $\mathcal{H}_{0,7}$ | $\mathcal{H}_{0,8}$ | $\mathcal{H}_{0,9}$ |
|-----------------------|------------------|---------------------|---------------------|---------------------|---------------------|---------------------|---------------------|---------------------|---------------------|---------------------|
| exp early continuous  | asymptotic       | 1.4                 | 1.1                 | 1.9                 | 1.0                 | 1.7                 | 1.0                 | 1.1                 | 1.2                 | 2.1                 |
|                       | asymptotic_bonf  | 1.3                 | 1.1                 | 1.7                 | 1.0                 | 1.4                 | 1.0                 | 1.0                 | 1.1                 | 2.0                 |
|                       | permutation_bonf | 0.1                 | 0.2                 | 0.5                 | 0.1                 | 0.3                 | 0.0                 | 0.2                 | 0.4                 | 0.6                 |
| exp early discrete    | asymptotic       | 1.7                 | 1.3                 | 1.6                 | 1.0                 | 1.7                 | 1.2                 | 1.2                 | 1.4                 | 1.8                 |
|                       | asymptotic_bonf  | 1.3                 | 1.1                 | 1.2                 | 0.9                 | 1.7                 | 1.0                 | 1.2                 | 1.2                 | 1.8                 |
|                       | permutation_bonf | 0.3                 | 0.2                 | 0.2                 | 0.2                 | 0.4                 | 0.2                 | 0.3                 | 0.5                 | 0.6                 |
| exp late continuous   | asymptotic       | 1.9                 | 1.0                 | 1.7                 | 1.2                 | 1.6                 | 1.1                 | 0.8                 | 1.2                 | 1.8                 |
|                       | asymptotic_bonf  | 1.6                 | 0.9                 | 1.4                 | 1.2                 | 1.3                 | 0.8                 | 0.8                 | 1.2                 | 1.6                 |
|                       | permutation_bonf | 0.1                 | 0.2                 | 0.3                 | 0.3                 | 0.1                 | 0.1                 | 0.2                 | 0.5                 | 0.4                 |
| exp late discrete     | asymptotic       | 1.8                 | 1.0                 | 1.7                 | 1.4                 | 1.3                 | 1.2                 | 1.6                 | 1.4                 | 2.3                 |
|                       | asymptotic_bonf  | 1.6                 | 0.8                 | 1.5                 | 1.3                 | 1.2                 | 1.1                 | 1.5                 | 1.3                 | 1.9                 |
|                       | permutation_bonf | 0.2                 | 0.0                 | 0.3                 | 0.3                 | 0.3                 | 0.2                 | 0.3                 | 0.5                 | 0.3                 |
| exp prop continuous   | asymptotic       | 1.2                 | 1.5                 | 2.3                 | 1.4                 | 1.4                 | 1.7                 | 1.4                 | 1.0                 | 1.6                 |
|                       | asymptotic_bonf  | 1.2                 | 1.4                 | 2.1                 | 1.2                 | 1.2                 | 1.6                 | 1.2                 | 1.0                 | 1.5                 |
|                       | permutation_bonf | 0.5                 | 0.4                 | 0.4                 | 0.3                 | 0.0                 | 0.4                 | 0.3                 | 0.5                 | 0.8                 |
| exp prop discrete     | asymptotic       | 1.7                 | 1.6                 | 1.6                 | 1.4                 | 1.4                 | 1.4                 | 1.6                 | 1.1                 | 1.6                 |
|                       | asymptotic_bonf  | 1.6                 | 1.4                 | 1.5                 | 1.3                 | 1.3                 | 1.4                 | 1.5                 | 1.1                 | 1.4                 |
|                       | permutation_bonf | 0.5                 | 0.3                 | 0.7                 | 0.4                 | 0.0                 | 0.6                 | 0.5                 | 0.5                 | 0.4                 |
| logn continuous       | asymptotic       | 1.6                 | 1.7                 | 1.7                 | 2.3                 | 2.6                 | 2.0                 | 1.8                 | 1.3                 | 2.8                 |
|                       | asymptotic_bonf  | 1.3                 | 1.4                 | 1.4                 | 2.1                 | 2.3                 | 2.0                 | 1.7                 | 1.0                 | 2.5                 |
|                       | permutation_bonf | 0.5                 | 0.5                 | 0.4                 | 0.3                 | 0.8                 | 0.8                 | 0.6                 | 0.5                 | 0.6                 |
| logn discrete         | asymptotic       | 1.9                 | 2.1                 | 2.0                 | 2.6                 | 2.3                 | 2.4                 | 1.9                 | 1.4                 | 3.4                 |
|                       | asymptotic_bonf  | 1.8                 | 1.9                 | 1.7                 | 2.0                 | 2.0                 | 2.1                 | 1.7                 | 1.4                 | 3.0                 |
|                       | permutation_bonf | 0.5                 | 0.5                 | 0.5                 | 0.3                 | 0.6                 | 0.8                 | 0.7                 | 0.7                 | 0.9                 |
| pwExp continuous      | asymptotic       | 1.0                 | 1.1                 | 1.8                 | 1.2                 | 0.9                 | 1.3                 | 0.7                 | 0.6                 | 2.1                 |
|                       | asymptotic_bonf  | 0.9                 | 1.0                 | 1.7                 | 1.2                 | 0.7                 | 1.1                 | 0.7                 | 0.6                 | 1.8                 |
|                       | permutation_bonf | 0.2                 | 0.3                 | 0.3                 | 0.4                 | 0.1                 | 0.2                 | 0.2                 | 0.3                 | 0.3                 |
| pwExp discrete        | asymptotic       | 1.2                 | 1.3                 | 2.0                 | 1.0                 | 1.1                 | 1.4                 | 1.2                 | 0.9                 | 2.1                 |
|                       | asymptotic_bonf  | 0.8                 | 1.3                 | 1.6                 | 1.0                 | 1.0                 | 1.3                 | 1.2                 | 0.8                 | 1.9                 |
|                       | permutation_bonf | 0.3                 | 0.3                 | 0.4                 | 0.2                 | 0.2                 | 0.2                 | 0.5                 | 0.5                 | 0.3                 |
| Weib late continuous  | asymptotic       | 2.3                 | 1.6                 | 2.6                 | 2.2                 | 2.4                 | 2.8                 | 2.2                 | 1.0                 | 2.5                 |
|                       | asymptotic_bonf  | 2.0                 | 1.4                 | 2.2                 | 1.9                 | 2.3                 | 2.6                 | 1.9                 | 1.0                 | 2.2                 |
|                       | permutation_bonf | 0.2                 | 0.2                 | 0.7                 | 0.4                 | 0.4                 | 0.8                 | 0.6                 | 0.4                 | 0.7                 |
| Weib late discrete    | asymptotic       | 2.2                 | 1.7                 | 3.3                 | 2.3                 | 2.3                 | 3.0                 | 2.7                 | 1.4                 | 2.3                 |
|                       | asymptotic_bonf  | 2.1                 | 1.5                 | 2.8                 | 2.0                 | 1.9                 | 3.0                 | 2.4                 | 1.4                 | 2.1                 |
|                       | permutation_bonf | 0.1                 | 0.3                 | 0.6                 | 0.4                 | 0.4                 | 0.8                 | 0.6                 | 0.9                 | 0.7                 |
| Weib prop continuous  | asymptotic       | 2.0                 | 1.6                 | 2.4                 | 2.0                 | 2.2                 | 2.5                 | 2.0                 | 1.2                 | 1.9                 |
|                       | asymptotic_bonf  | 1.5                 | 1.5                 | 2.1                 | 1.7                 | 2.2                 | 2.1                 | 1.7                 | 1.1                 | 1.8                 |
|                       | permutation_bonf | 0.2                 | 0.3                 | 0.5                 | 0.3                 | 0.5                 | 0.7                 | 0.4                 | 0.3                 | 0.8                 |
| Weib prop discrete    | asymptotic       | 1.8                 | 1.7                 | 3.1                 | 2.2                 | 2.2                 | 2.5                 | 2.4                 | 0.8                 | 2.1                 |
|                       | asymptotic_bonf  | 1.6                 | 1.6                 | 2.5                 | 1.9                 | 1.7                 | 2.3                 | 2.2                 | 0.7                 | 1.8                 |
|                       | permutation_bonf | 0.2                 | 0.4                 | 0.7                 | 0.4                 | 0.5                 | 0.8                 | 0.4                 | 0.3                 | 0.9                 |
| Weib scale continuous | asymptotic       | 1.7                 | 2.3                 | 2.4                 | 2.0                 | 2.5                 | 2.5                 | 1.4                 | 1.6                 | 1.6                 |
|                       | asymptotic_bonf  | 1.2                 | 2.1                 | 2.2                 | 1.8                 | 2.3                 | 2.2                 | 1.1                 | 1.4                 | 1.4                 |
|                       | permutation_bonf | 0.2                 | 0.4                 | 0.3                 | 0.3                 | 0.5                 | 0.7                 | 0.5                 | 0.5                 | 0.7                 |
| Weib scale discrete   | asymptotic       | 1.9                 | 2.0                 | 2.2                 | 2.4                 | 1.8                 | 2.3                 | 2.0                 | 1.3                 | 1.1                 |
|                       | asymptotic_bonf  | 1.8                 | 1.8                 | 1.9                 | 1.7                 | 1.4                 | 2.0                 | 1.7                 | 1.1                 | 1.1                 |
|                       | permutation_bonf | 0.3                 | 0.6                 | 0.4                 | 0.5                 | 0.3                 | 0.5                 | 0.5                 | 0.5                 | 0.4                 |
| Weib shape continuous | asymptotic       | 2.0                 | 1.6                 | 2.0                 | 1.6                 | 3.0                 | 2.5                 | 1.1                 | 0.8                 | 1.1                 |
|                       | asymptotic_bonf  | 1.7                 | 1.5                 | 1.8                 | 1.4                 | 2.5                 | 1.9                 | 0.9                 | 0.6                 | 0.9                 |
|                       | permutation_bonf | 0.4                 | 0.3                 | 0.5                 | 0.0                 | 0.5                 | 0.8                 | 0.4                 | 0.3                 | 0.5                 |
| Weib shape discrete   | asymptotic       | 2.1                 | 2.0                 | 2.6                 | 2.0                 | 1.8                 | 2.4                 | 1.5                 | 1.0                 | 1.0                 |
|                       | asymptotic_bonf  | 2.1                 | 1.5                 | 2.1                 | 1.7                 | 1.5                 | 2.2                 | 1.2                 | 0.7                 | 0.9                 |
|                       | permutation_bonf | 0.3                 | 0.4                 | 0.6                 | 0.1                 | 0.5                 | 0.5                 | 0.4                 | 0.4                 | 0.4                 |

Table S49: Rejection rates in percent for the 2-by-2 design with  $\delta = 1.5$  and balanced large sample sizes under unequal, low censoring.

| Distribution          | Method           | $\mathcal{H}_{0,4}$ | $\mathcal{H}_{0,5}$ | $\mathcal{H}_{0,6}$ | $\mathcal{H}_{0,1}$ | $\mathcal{H}_{0,2}$ | $\mathcal{H}_{0,3}$ | $\mathcal{H}_{0,7}$ | $\mathcal{H}_{0,8}$ | $\mathcal{H}_{0,9}$ |
|-----------------------|------------------|---------------------|---------------------|---------------------|---------------------|---------------------|---------------------|---------------------|---------------------|---------------------|
| exp early continuous  | asymptotic       | 49.5                | 31.2                | 67.4                | 47.7                | 32.9                | 68.2                | 47.5                | 30.7                | 68.3                |
|                       | asymptotic_bonf  | 48.5                | 30.3                | 66.7                | 46.9                | 32.1                | 67.6                | 46.3                | 29.8                | 67.3                |
|                       | permutation_bonf | 48.3                | 29.2                | 66.4                | 46.4                | 31.0                | 67.9                | 46.5                | 29.8                | 66.4                |
| exp early discrete    | asymptotic       | 56.5                | 36.4                | 73.5                | 54.7                | 36.0                | 75.1                | 54.1                | 35.7                | 75.7                |
|                       | asymptotic_bonf  | 56.0                | 35.5                | 73.4                | 53.5                | 35.5                | 74.7                | 53.6                | 35.0                | 74.9                |
|                       | permutation_bonf | 54.7                | 34.6                | 71.9                | 53.1                | 34.8                | 74.3                | 53.1                | 34.6                | 74.5                |
| exp late continuous   | asymptotic       | 51.9                | 33.1                | 70.2                | 50.2                | 34.1                | 71.1                | 48.8                | 31.8                | 70.9                |
|                       | asymptotic_bonf  | 51.3                | 32.4                | 69.7                | 49.2                | 33.4                | 70.7                | 48.6                | 31.5                | 69.9                |
|                       | permutation_bonf | 51.1                | 31.1                | 68.6                | 47.9                | 32.2                | 69.1                | 48.2                | 30.8                | 70.8                |
| exp late discrete     | asymptotic       | 59.0                | 39.6                | 76.2                | 56.2                | 38.2                | 77.9                | 55.6                | 37.9                | 78.1                |
|                       | asymptotic_bonf  | 58.5                | 38.9                | 75.7                | 55.5                | 37.2                | 77.2                | 54.9                | 36.4                | 77.6                |
|                       | permutation_bonf | 57.2                | 37.5                | 74.9                | 54.6                | 36.0                | 76.1                | 55.0                | 35.3                | 76.8                |
| exp prop continuous   | asymptotic       | 50.1                | 34.1                | 68.6                | 49.9                | 33.2                | 68.6                | 48.5                | 34.3                | 69.2                |
|                       | asymptotic_bonf  | 49.1                | 32.9                | 67.6                | 49.3                | 32.9                | 68.0                | 47.6                | 33.4                | 68.1                |
|                       | permutation_bonf | 50.1                | 32.7                | 67.9                | 48.7                | 32.7                | 68.0                | 48.4                | 32.9                | 68.2                |
| exp prop discrete     | asymptotic       | 55.4                | 40.3                | 74.8                | 56.0                | 37.0                | 75.1                | 56.4                | 38.7                | 76.7                |
|                       | asymptotic_bonf  | 54.8                | 39.4                | 74.2                | 55.4                | 36.5                | 74.8                | 55.2                | 37.8                | 76.1                |
|                       | permutation_bonf | 55.0                | 38.1                | 74.2                | 55.4                | 36.5                | 74.1                | 55.6                | 38.3                | 75.2                |
| logn continuous       | asymptotic       | 94.3                | 81.0                | 98.9                | 93.3                | 81.6                | 99.7                | 93.9                | 83.9                | 98.7                |
|                       | asymptotic_bonf  | 94.1                | 80.7                | 98.8                | 93.3                | 81.4                | 99.7                | 93.9                | 83.6                | 98.5                |
|                       | permutation_bonf | 94.5                | 81.3                | 98.5                | 93.6                | 80.8                | 99.5                | 93.3                | 82.7                | 98.3                |
| logn discrete         | asymptotic       | 97.2                | 88.0                | 99.9                | 97.0                | 89.1                | 99.8                | 97.0                | 90.7                | 99.6                |
|                       | asymptotic_bonf  | 97.1                | 87.5                | 99.9                | 97.0                | 89.0                | 99.8                | 97.0                | 90.5                | 99.6                |
|                       | permutation_bonf | 96.9                | 87.9                | 99.9                | 96.6                | 88.4                | 99.8                | 96.8                | 89.6                | 99.5                |
| pwExp continuous      | asymptotic       | 48.4                | 30.9                | 66.6                | 47.0                | 32.1                | 68.3                | 45.9                | 29.9                | 67.7                |
|                       | asymptotic_bonf  | 47.6                | 30.3                | 66.2                | 46.3                | 31.7                | 67.7                | 45.6                | 29.4                | 67.1                |
|                       | permutation_bonf | 47.7                | 30.5                | 66.5                | 45.7                | 32.5                | 67.7                | 45.6                | 29.7                | 66.4                |
| pwExp discrete        | asymptotic       | 55.0                | 37.0                | 73.5                | 53.9                | 35.8                | 74.7                | 52.7                | 34.6                | 74.9                |
|                       | asymptotic_bonf  | 54.1                | 36.4                | 72.9                | 52.9                | 35.4                | 74.2                | 52.4                | 33.9                | 74.4                |
|                       | permutation_bonf | 54.6                | 37.6                | 72.0                | 53.7                | 35.8                | 72.9                | 52.5                | 33.6                | 73.3                |
| Weib late continuous  | asymptotic       | 94.4                | 78.5                | 98.8                | 94.1                | 80.4                | 98.8                | 94.3                | 82.2                | 99.1                |
|                       | asymptotic_bonf  | 94.4                | 77.7                | 98.8                | 94.0                | 80.0                | 98.7                | 94.3                | 82.0                | 99.0                |
|                       | permutation_bonf | 94.8                | 78.6                | 98.5                | 94.6                | 79.9                | 98.5                | 94.2                | 81.3                | 98.7                |
| Weib late discrete    | asymptotic       | 97.4                | 86.8                | 99.7                | 97.8                | 88.6                | 99.9                | 97.3                | 88.8                | 99.6                |
|                       | asymptotic_bonf  | 97.3                | 86.6                | 99.7                | 97.8                | 88.5                | 99.9                | 97.1                | 88.5                | 99.5                |
|                       | permutation_bonf | 97.4                | 87.2                | 99.7                | 97.8                | 88.7                | 99.8                | 96.4                | 88.7                | 99.4                |
| Weib prop continuous  | asymptotic       | 94.1                | 77.8                | 98.6                | 93.6                | 79.4                | 98.7                | 93.5                | 81.0                | 98.8                |
|                       | asymptotic_bonf  | 94.0                | 77.2                | 98.6                | 93.6                | 78.9                | 98.7                | 93.4                | 80.3                | 98.8                |
|                       | permutation_bonf | 94.0                | 77.4                | 98.4                | 94.0                | 78.5                | 98.6                | 93.3                | 80.7                | 98.7                |
| Weib prop discrete    | asymptotic       | 97.3                | 85.8                | 99.6                | 97.2                | 87.7                | 99.7                | 96.7                | 88.1                | 99.5                |
|                       | asymptotic_bonf  | 97.3                | 85.2                | 99.5                | 97.1                | 87.4                | 99.7                | 96.6                | 87.9                | 99.4                |
|                       | permutation_bonf | 97.1                | 85.8                | 99.8                | 96.9                | 87.0                | 99.7                | 96.2                | 87.6                | 99.4                |
| Weib scale continuous | asymptotic       | 91.1                | 74.6                | 97.8                | 91.6                | 75.8                | 97.8                | 90.8                | 77.1                | 98.4                |
|                       | asymptotic_bonf  | 90.8                | 74.1                | 97.8                | 91.4                | 75.1                | 97.7                | 90.6                | 76.3                | 98.4                |
|                       | permutation_bonf | 90.8                | 73.5                | 97.6                | 91.7                | 74.9                | 97.3                | 90.3                | 76.4                | 98.3                |
| Weib scale discrete   | asymptotic       | 95.3                | 82.7                | 99.0                | 95.6                | 83.7                | 99.2                | 95.0                | 83.9                | 99.2                |
|                       | asymptotic_bonf  | 95.2                | 82.3                | 99.0                | 95.5                | 83.5                | 99.1                | 94.8                | 83.8                | 99.1                |
|                       | permutation_bonf | 94.9                | 82.0                | 99.1                | 95.4                | 83.8                | 98.8                | 94.8                | 82.7                | 99.3                |
| Weib shape continuous | asymptotic       | 85.7                | 67.5                | 96.0                | 87.1                | 69.3                | 95.1                | 85.9                | 70.6                | 95.8                |
|                       | asymptotic_bonf  | 85.3                | 67.3                | 95.9                | 87.0                | 68.6                | 94.7                | 85.7                | 70.5                | 95.8                |
|                       | permutation_bonf | 85.5                | 67.6                | 96.0                | 86.4                | 68.9                | 94.9                | 86.1                | 70.1                | 95.8                |
| Weib shape discrete   | asymptotic       | 92.6                | 78.2                | 97.8                | 92.9                | 78.3                | 98.0                | 92.0                | 80.1                | 98.7                |
|                       | asymptotic_bonf  | 92.4                | 77.6                | 97.8                | 92.8                | 78.1                | 97.8                | 91.7                | 79.9                | 98.7                |
|                       | permutation_bonf | 92.4                | 77.5                | 97.6                | 92.9                | 78.0                | 97.8                | 91.7                | 79.4                | 98.5                |



Table S50: Rejection rates in percent for the 2-by-2 design with  $\delta = 1.5$  and balanced medium sample sizes under unequal, low censoring.

| Distribution          | Method           | $\mathcal{H}_{0,4}$ | $\mathcal{H}_{0,5}$ | $\mathcal{H}_{0,6}$ | $\mathcal{H}_{0,1}$ | $\mathcal{H}_{0,2}$ | $\mathcal{H}_{0,3}$ | $\mathcal{H}_{0,7}$ | $\mathcal{H}_{0,8}$ | $\mathcal{H}_{0,9}$ |
|-----------------------|------------------|---------------------|---------------------|---------------------|---------------------|---------------------|---------------------|---------------------|---------------------|---------------------|
| exp early continuous  | asymptotic       | 5.6                 | 5.4                 | 9.2                 | 6.9                 | 3.1                 | 8.9                 | 6.5                 | 2.7                 | 9.8                 |
|                       | asymptotic_bonf  | 5.5                 | 5.4                 | 8.9                 | 6.5                 | 3.0                 | 8.8                 | 6.2                 | 2.7                 | 9.6                 |
|                       | permutation_bonf | 6.0                 | 5.7                 | 8.7                 | 6.7                 | 2.9                 | 9.1                 | 6.3                 | 2.8                 | 9.3                 |
| exp early discrete    | asymptotic       | 7.1                 | 6.3                 | 10.6                | 7.4                 | 3.6                 | 11.7                | 6.7                 | 3.1                 | 11.3                |
|                       | asymptotic_bonf  | 7.0                 | 6.2                 | 10.2                | 7.1                 | 3.5                 | 11.5                | 6.6                 | 3.1                 | 11.1                |
|                       | permutation_bonf | 7.9                 | 6.0                 | 10.1                | 7.1                 | 3.9                 | 11.2                | 6.7                 | 2.7                 | 10.8                |
| exp late continuous   | asymptotic       | 5.8                 | 5.9                 | 9.9                 | 7.5                 | 3.3                 | 9.9                 | 7.6                 | 3.4                 | 10.4                |
|                       | asymptotic_bonf  | 5.7                 | 5.8                 | 9.9                 | 7.0                 | 3.1                 | 9.8                 | 7.3                 | 3.2                 | 10.0                |
|                       | permutation_bonf | 6.0                 | 6.0                 | 9.3                 | 7.1                 | 3.7                 | 9.7                 | 6.6                 | 2.7                 | 9.1                 |
| exp late discrete     | asymptotic       | 7.6                 | 6.0                 | 11.0                | 8.3                 | 4.0                 | 12.1                | 7.7                 | 3.5                 | 11.9                |
|                       | asymptotic_bonf  | 7.2                 | 6.0                 | 10.7                | 8.0                 | 3.6                 | 11.9                | 7.6                 | 3.5                 | 11.5                |
|                       | permutation_bonf | 7.6                 | 5.6                 | 11.1                | 7.6                 | 4.1                 | 11.9                | 7.1                 | 3.1                 | 12.1                |
| exp prop continuous   | asymptotic       | 7.3                 | 4.7                 | 9.0                 | 6.0                 | 4.8                 | 8.7                 | 6.6                 | 4.8                 | 9.7                 |
|                       | asymptotic_bonf  | 7.2                 | 4.7                 | 8.8                 | 5.9                 | 4.6                 | 8.5                 | 6.4                 | 4.5                 | 9.2                 |
|                       | permutation_bonf | 6.9                 | 4.3                 | 9.5                 | 6.1                 | 4.3                 | 8.3                 | 6.4                 | 4.9                 | 9.5                 |
| exp prop discrete     | asymptotic       | 7.6                 | 5.1                 | 10.2                | 6.9                 | 5.1                 | 9.2                 | 7.0                 | 5.3                 | 11.1                |
|                       | asymptotic_bonf  | 7.4                 | 5.1                 | 9.8                 | 6.8                 | 5.0                 | 9.2                 | 6.9                 | 5.1                 | 10.5                |
|                       | permutation_bonf | 7.8                 | 5.6                 | 10.0                | 6.4                 | 4.6                 | 8.9                 | 7.6                 | 5.2                 | 9.5                 |
| logn continuous       | asymptotic       | 18.9                | 12.3                | 30.3                | 21.0                | 13.9                | 32.8                | 21.6                | 12.7                | 32.0                |
|                       | asymptotic_bonf  | 18.8                | 11.9                | 30.0                | 20.5                | 13.8                | 32.8                | 20.9                | 12.3                | 31.6                |
|                       | permutation_bonf | 18.7                | 12.2                | 30.2                | 19.9                | 13.8                | 31.3                | 20.9                | 12.1                | 31.4                |
| logn discrete         | asymptotic       | 23.9                | 15.1                | 40.8                | 27.0                | 18.5                | 38.0                | 25.9                | 16.6                | 38.2                |
|                       | asymptotic_bonf  | 23.3                | 14.7                | 39.7                | 26.8                | 18.3                | 37.7                | 25.3                | 16.3                | 37.9                |
|                       | permutation_bonf | 23.3                | 15.1                | 39.8                | 26.4                | 17.7                | 37.3                | 25.6                | 16.3                | 37.8                |
| pwExp continuous      | asymptotic       | 5.8                 | 5.5                 | 9.2                 | 6.9                 | 4.0                 | 8.9                 | 6.6                 | 2.6                 | 8.9                 |
|                       | asymptotic_bonf  | 5.6                 | 5.4                 | 8.8                 | 6.3                 | 3.8                 | 8.8                 | 6.4                 | 2.5                 | 8.8                 |
|                       | permutation_bonf | 6.2                 | 5.3                 | 8.9                 | 6.2                 | 3.9                 | 8.8                 | 6.6                 | 2.7                 | 9.2                 |
| pwExp discrete        | asymptotic       | 6.9                 | 5.8                 | 11.1                | 6.8                 | 4.6                 | 11.0                | 7.2                 | 3.5                 | 10.9                |
|                       | asymptotic_bonf  | 6.7                 | 5.4                 | 10.8                | 6.8                 | 4.3                 | 10.8                | 7.0                 | 3.3                 | 10.7                |
|                       | permutation_bonf | 6.9                 | 5.6                 | 10.7                | 6.6                 | 4.2                 | 11.2                | 6.5                 | 3.1                 | 11.0                |
| Weib late continuous  | asymptotic       | 18.8                | 12.7                | 33.4                | 20.4                | 13.5                | 30.0                | 20.9                | 11.9                | 32.6                |
|                       | asymptotic_bonf  | 18.5                | 12.3                | 32.8                | 20.0                | 13.3                | 29.5                | 20.6                | 11.4                | 32.4                |
|                       | permutation_bonf | 18.1                | 12.6                | 33.6                | 20.9                | 13.6                | 29.3                | 19.8                | 11.2                | 33.0                |
| Weib late discrete    | asymptotic       | 22.6                | 16.1                | 40.4                | 25.8                | 16.2                | 36.0                | 26.4                | 15.3                | 39.5                |
|                       | asymptotic_bonf  | 22.1                | 15.6                | 39.4                | 24.9                | 15.6                | 35.6                | 25.7                | 14.6                | 38.9                |
|                       | permutation_bonf | 22.3                | 16.5                | 38.8                | 25.0                | 15.3                | 35.2                | 26.0                | 15.2                | 38.3                |
| Weib prop continuous  | asymptotic       | 17.8                | 12.4                | 32.5                | 19.4                | 12.8                | 29.6                | 20.1                | 11.3                | 31.6                |
|                       | asymptotic_bonf  | 17.2                | 12.2                | 32.2                | 19.2                | 12.4                | 29.2                | 19.9                | 10.9                | 31.2                |
|                       | permutation_bonf | 17.0                | 12.7                | 32.5                | 19.4                | 12.6                | 28.4                | 19.4                | 10.8                | 31.0                |
| Weib prop discrete    | asymptotic       | 22.4                | 15.5                | 39.0                | 25.4                | 15.9                | 35.9                | 26.4                | 14.6                | 38.4                |
|                       | asymptotic_bonf  | 22.0                | 15.0                | 38.4                | 24.8                | 15.6                | 35.5                | 26.1                | 14.2                | 37.7                |
|                       | permutation_bonf | 22.4                | 15.0                | 38.6                | 24.9                | 16.3                | 35.6                | 25.4                | 14.2                | 38.5                |
| Weib scale continuous | asymptotic       | 15.9                | 11.2                | 28.7                | 16.9                | 11.0                | 25.9                | 18.1                | 9.7                 | 27.9                |
|                       | asymptotic_bonf  | 15.7                | 11.0                | 28.2                | 16.7                | 10.8                | 25.1                | 17.7                | 9.5                 | 27.8                |
|                       | permutation_bonf | 16.1                | 11.2                | 27.9                | 16.8                | 11.3                | 25.6                | 17.3                | 9.2                 | 26.4                |
| Weib scale discrete   | asymptotic       | 20.2                | 13.7                | 34.7                | 21.8                | 13.6                | 31.6                | 23.2                | 12.9                | 33.3                |
|                       | asymptotic_bonf  | 19.6                | 13.7                | 34.1                | 21.5                | 13.1                | 31.1                | 22.9                | 12.3                | 32.8                |
|                       | permutation_bonf | 19.4                | 13.4                | 34.6                | 22.3                | 13.4                | 31.9                | 22.8                | 12.6                | 32.5                |
| Weib shape continuous | asymptotic       | 12.8                | 9.0                 | 24.6                | 14.5                | 9.5                 | 20.5                | 14.2                | 8.1                 | 23.8                |
|                       | asymptotic_bonf  | 12.6                | 8.7                 | 24.0                | 13.7                | 9.3                 | 20.1                | 13.8                | 8.0                 | 23.4                |
|                       | permutation_bonf | 13.3                | 8.3                 | 23.4                | 14.1                | 9.5                 | 20.0                | 13.4                | 7.7                 | 23.5                |
| Weib shape discrete   | asymptotic       | 16.7                | 11.8                | 29.0                | 18.1                | 11.3                | 27.5                | 19.0                | 11.4                | 27.2                |
|                       | asymptotic_bonf  | 16.4                | 11.6                | 28.4                | 17.3                | 10.9                | 27.1                | 18.3                | 11.0                | 26.7                |
|                       | permutation_bonf | 16.5                | 11.2                | 28.8                | 17.8                | 11.4                | 27.6                | 18.7                | 11.1                | 27.7                |

Table S51: Rejection rates in percent for the 2-by-2 design with  $\delta = 1.5$  and balanced small sample sizes under unequal, low censoring.

| Distribution          | Method           | $\mathcal{H}_{0,4}$ | $\mathcal{H}_{0,5}$ | $\mathcal{H}_{0,6}$ | $\mathcal{H}_{0,1}$ | $\mathcal{H}_{0,2}$ | $\mathcal{H}_{0,3}$ | $\mathcal{H}_{0,7}$ | $\mathcal{H}_{0,8}$ | $\mathcal{H}_{0,9}$ |
|-----------------------|------------------|---------------------|---------------------|---------------------|---------------------|---------------------|---------------------|---------------------|---------------------|---------------------|
| exp early continuous  | asymptotic       | 2.1                 | 1.2                 | 1.4                 | 1.7                 | 0.8                 | 1.8                 | 1.7                 | 1.6                 | 1.4                 |
|                       | asymptotic_bonf  | 1.8                 | 1.2                 | 1.4                 | 1.6                 | 0.8                 | 1.7                 | 1.6                 | 1.4                 | 1.3                 |
|                       | permutation_bonf | 1.7                 | 1.0                 | 1.2                 | 1.4                 | 0.9                 | 1.6                 | 1.1                 | 1.6                 | 1.3                 |
| exp early discrete    | asymptotic       | 2.1                 | 1.5                 | 1.4                 | 1.2                 | 1.6                 | 1.6                 | 2.3                 | 1.0                 | 1.9                 |
|                       | asymptotic_bonf  | 1.9                 | 1.5                 | 1.2                 | 1.0                 | 1.5                 | 1.4                 | 2.3                 | 1.0                 | 1.8                 |
|                       | permutation_bonf | 1.6                 | 1.2                 | 1.3                 | 1.0                 | 1.3                 | 1.4                 | 1.8                 | 0.6                 | 1.5                 |
| exp late continuous   | asymptotic       | 1.5                 | 1.4                 | 1.6                 | 1.9                 | 0.9                 | 1.7                 | 1.9                 | 1.8                 | 1.5                 |
|                       | asymptotic_bonf  | 1.3                 | 1.3                 | 1.4                 | 1.9                 | 0.9                 | 1.6                 | 1.8                 | 1.6                 | 1.5                 |
|                       | permutation_bonf | 1.6                 | 1.1                 | 1.2                 | 1.6                 | 1.2                 | 1.4                 | 1.6                 | 1.6                 | 1.2                 |
| exp late discrete     | asymptotic       | 1.6                 | 1.4                 | 1.6                 | 1.8                 | 1.3                 | 2.1                 | 2.4                 | 1.7                 | 1.9                 |
|                       | asymptotic_bonf  | 1.5                 | 1.2                 | 1.4                 | 1.7                 | 1.3                 | 2.0                 | 2.0                 | 1.6                 | 1.9                 |
|                       | permutation_bonf | 1.6                 | 0.9                 | 1.6                 | 1.6                 | 1.4                 | 1.9                 | 1.9                 | 1.7                 | 1.4                 |
| exp prop continuous   | asymptotic       | 1.3                 | 1.3                 | 2.0                 | 1.6                 | 1.5                 | 2.0                 | 1.1                 | 1.3                 | 1.8                 |
|                       | asymptotic_bonf  | 1.2                 | 1.1                 | 2.0                 | 1.5                 | 1.4                 | 2.0                 | 1.1                 | 1.2                 | 1.7                 |
|                       | permutation_bonf | 1.1                 | 0.9                 | 1.8                 | 1.5                 | 1.4                 | 1.8                 | 0.9                 | 1.6                 | 1.6                 |
| exp prop discrete     | asymptotic       | 2.2                 | 0.7                 | 2.3                 | 1.4                 | 1.1                 | 2.6                 | 1.1                 | 1.1                 | 2.4                 |
|                       | asymptotic_bonf  | 2.1                 | 0.7                 | 2.2                 | 1.3                 | 0.9                 | 2.5                 | 1.1                 | 1.1                 | 2.3                 |
|                       | permutation_bonf | 1.9                 | 1.0                 | 1.9                 | 1.4                 | 1.1                 | 1.9                 | 1.1                 | 0.6                 | 2.2                 |
| logn continuous       | asymptotic       | 3.9                 | 2.0                 | 4.3                 | 3.5                 | 4.1                 | 6.2                 | 3.1                 | 1.0                 | 4.4                 |
|                       | asymptotic_bonf  | 3.9                 | 2.0                 | 4.2                 | 3.4                 | 3.9                 | 6.0                 | 3.0                 | 1.0                 | 4.3                 |
|                       | permutation_bonf | 3.9                 | 1.7                 | 4.0                 | 2.8                 | 3.6                 | 5.4                 | 2.9                 | 1.0                 | 4.0                 |
| logn discrete         | asymptotic       | 4.8                 | 2.4                 | 4.9                 | 4.4                 | 4.3                 | 7.3                 | 3.8                 | 1.4                 | 4.8                 |
|                       | asymptotic_bonf  | 4.5                 | 2.3                 | 4.8                 | 4.4                 | 4.1                 | 7.3                 | 3.8                 | 1.2                 | 4.8                 |
|                       | permutation_bonf | 4.7                 | 2.4                 | 4.4                 | 4.0                 | 4.1                 | 7.1                 | 3.8                 | 1.2                 | 4.7                 |
| pwExp continuous      | asymptotic       | 1.6                 | 1.2                 | 1.3                 | 1.7                 | 0.9                 | 1.9                 | 1.9                 | 1.6                 | 1.3                 |
|                       | asymptotic_bonf  | 1.5                 | 1.2                 | 1.2                 | 1.6                 | 0.9                 | 1.7                 | 1.9                 | 1.6                 | 1.3                 |
|                       | permutation_bonf | 1.5                 | 1.1                 | 1.2                 | 1.0                 | 0.9                 | 1.5                 | 1.0                 | 1.7                 | 1.2                 |
| pwExp discrete        | asymptotic       | 2.0                 | 1.3                 | 1.4                 | 1.8                 | 1.1                 | 2.1                 | 1.9                 | 1.6                 | 1.9                 |
|                       | asymptotic_bonf  | 1.7                 | 1.3                 | 1.3                 | 1.8                 | 1.0                 | 2.0                 | 1.7                 | 1.5                 | 1.9                 |
|                       | permutation_bonf | 1.9                 | 1.3                 | 1.6                 | 1.3                 | 1.2                 | 1.9                 | 1.0                 | 1.9                 | 1.6                 |
| Weib late continuous  | asymptotic       | 3.5                 | 2.4                 | 4.6                 | 2.9                 | 3.6                 | 4.1                 | 3.4                 | 3.1                 | 5.0                 |
|                       | asymptotic_bonf  | 3.4                 | 2.4                 | 4.5                 | 2.9                 | 3.4                 | 4.1                 | 3.3                 | 3.1                 | 4.9                 |
|                       | permutation_bonf | 3.4                 | 2.3                 | 4.4                 | 2.4                 | 3.1                 | 3.7                 | 3.2                 | 2.9                 | 5.2                 |
| Weib late discrete    | asymptotic       | 3.8                 | 3.1                 | 5.5                 | 2.9                 | 3.6                 | 5.0                 | 4.3                 | 3.5                 | 5.8                 |
|                       | asymptotic_bonf  | 3.6                 | 3.0                 | 5.4                 | 2.9                 | 3.5                 | 4.8                 | 4.2                 | 3.3                 | 5.6                 |
|                       | permutation_bonf | 3.3                 | 2.3                 | 4.8                 | 2.9                 | 3.4                 | 4.7                 | 3.7                 | 3.1                 | 5.3                 |
| Weib prop continuous  | asymptotic       | 3.6                 | 2.3                 | 4.5                 | 2.7                 | 3.2                 | 3.9                 | 3.2                 | 3.3                 | 4.8                 |
|                       | asymptotic_bonf  | 3.6                 | 2.3                 | 4.3                 | 2.6                 | 3.0                 | 3.9                 | 3.1                 | 3.3                 | 4.6                 |
|                       | permutation_bonf | 3.0                 | 2.1                 | 4.2                 | 2.2                 | 2.9                 | 3.7                 | 3.0                 | 3.0                 | 5.1                 |
| Weib prop discrete    | asymptotic       | 4.0                 | 2.6                 | 5.6                 | 3.2                 | 3.3                 | 4.8                 | 4.2                 | 3.2                 | 5.7                 |
|                       | asymptotic_bonf  | 3.8                 | 2.6                 | 5.4                 | 3.2                 | 3.2                 | 4.5                 | 4.0                 | 3.2                 | 5.6                 |
|                       | permutation_bonf | 3.5                 | 2.4                 | 5.4                 | 2.9                 | 3.5                 | 4.3                 | 3.5                 | 2.9                 | 5.3                 |
| Weib scale continuous | asymptotic       | 2.6                 | 2.0                 | 4.3                 | 2.3                 | 2.7                 | 3.5                 | 2.6                 | 2.4                 | 4.3                 |
|                       | asymptotic_bonf  | 2.6                 | 1.9                 | 4.1                 | 2.2                 | 2.7                 | 3.5                 | 2.6                 | 2.3                 | 4.2                 |
|                       | permutation_bonf | 2.3                 | 2.0                 | 3.6                 | 1.8                 | 2.2                 | 3.2                 | 2.3                 | 2.5                 | 4.0                 |
| Weib scale discrete   | asymptotic       | 2.7                 | 2.2                 | 4.8                 | 2.3                 | 3.2                 | 4.1                 | 3.0                 | 2.5                 | 4.8                 |
|                       | asymptotic_bonf  | 2.6                 | 2.2                 | 4.6                 | 2.2                 | 2.9                 | 3.8                 | 2.8                 | 2.1                 | 4.7                 |
|                       | permutation_bonf | 2.7                 | 2.3                 | 4.6                 | 2.2                 | 2.7                 | 3.6                 | 2.7                 | 2.4                 | 4.5                 |
| Weib shape continuous | asymptotic       | 2.0                 | 1.4                 | 3.1                 | 1.1                 | 2.0                 | 2.6                 | 1.9                 | 1.9                 | 3.6                 |
|                       | asymptotic_bonf  | 1.9                 | 1.4                 | 2.9                 | 1.1                 | 1.9                 | 2.5                 | 1.8                 | 1.8                 | 3.4                 |
|                       | permutation_bonf | 1.8                 | 1.7                 | 2.8                 | 0.9                 | 1.8                 | 2.1                 | 2.2                 | 1.7                 | 3.4                 |
| Weib shape discrete   | asymptotic       | 2.3                 | 1.8                 | 3.5                 | 1.4                 | 2.3                 | 3.3                 | 2.1                 | 2.1                 | 4.2                 |
|                       | asymptotic_bonf  | 1.9                 | 1.7                 | 3.4                 | 1.4                 | 2.1                 | 3.2                 | 1.9                 | 2.0                 | 3.9                 |
|                       | permutation_bonf | 2.1                 | 1.6                 | 3.4                 | 1.3                 | 2.1                 | 3.0                 | 2.0                 | 1.9                 | 3.6                 |

Table S52: Rejection rates in percent for the 2-by-2 design with  $\delta = 1.5$  and unbalanced large sample sizes under unequal, low censoring.

| Distribution          | Method           | $\mathcal{H}_{0,4}$ | $\mathcal{H}_{0,5}$ | $\mathcal{H}_{0,6}$ | $\mathcal{H}_{0,1}$ | $\mathcal{H}_{0,2}$ | $\mathcal{H}_{0,3}$ | $\mathcal{H}_{0,7}$ | $\mathcal{H}_{0,8}$ | $\mathcal{H}_{0,9}$ |
|-----------------------|------------------|---------------------|---------------------|---------------------|---------------------|---------------------|---------------------|---------------------|---------------------|---------------------|
| exp early continuous  | asymptotic       | 24.2                | 13.3                | 39.7                | 23.5                | 13.1                | 37.4                | 24.2                | 13.0                | 37.8                |
|                       | asymptotic.bonf  | 22.7                | 12.5                | 38.4                | 22.7                | 12.0                | 35.9                | 22.7                | 12.2                | 35.5                |
|                       | permutation.bonf | 22.2                | 11.7                | 37.7                | 21.4                | 11.7                | 34.8                | 22.4                | 12.7                | 35.8                |
| exp early discrete    | asymptotic       | 27.5                | 15.7                | 44.8                | 27.5                | 15.1                | 44.9                | 28.6                | 15.6                | 43.8                |
|                       | asymptotic.bonf  | 25.6                | 14.6                | 42.7                | 25.7                | 14.2                | 42.8                | 27.1                | 14.1                | 41.8                |
|                       | permutation.bonf | 26.2                | 13.8                | 42.3                | 25.9                | 13.1                | 42.9                | 26.8                | 14.8                | 40.4                |
| exp late continuous   | asymptotic       | 26.1                | 14.5                | 45.9                | 26.5                | 14.5                | 44.1                | 26.8                | 14.6                | 41.8                |
|                       | asymptotic.bonf  | 25.0                | 13.3                | 44.2                | 24.4                | 13.3                | 42.3                | 25.0                | 13.2                | 40.1                |
|                       | permutation.bonf | 25.0                | 13.3                | 42.6                | 24.2                | 12.5                | 40.5                | 25.6                | 13.8                | 39.4                |
| exp late discrete     | asymptotic       | 30.3                | 17.5                | 51.8                | 31.2                | 17.8                | 50.4                | 31.5                | 17.6                | 50.0                |
|                       | asymptotic.bonf  | 28.8                | 16.5                | 49.2                | 29.6                | 16.4                | 48.9                | 30.1                | 16.3                | 47.4                |
|                       | permutation.bonf | 29.4                | 15.7                | 48.2                | 28.2                | 16.0                | 49.2                | 28.9                | 16.7                | 46.2                |
| exp prop continuous   | asymptotic       | 28.2                | 16.5                | 37.5                | 25.5                | 14.9                | 39.6                | 26.5                | 15.0                | 36.4                |
|                       | asymptotic.bonf  | 26.3                | 14.8                | 35.7                | 23.6                | 14.0                | 37.5                | 24.2                | 14.3                | 34.8                |
|                       | permutation.bonf | 26.7                | 14.4                | 34.3                | 23.0                | 13.0                | 36.6                | 23.6                | 14.6                | 33.9                |
| exp prop discrete     | asymptotic       | 31.2                | 20.0                | 42.6                | 28.4                | 18.0                | 44.5                | 30.1                | 17.9                | 43.5                |
|                       | asymptotic.bonf  | 29.4                | 18.1                | 41.0                | 26.7                | 16.5                | 42.8                | 28.7                | 17.0                | 40.8                |
|                       | permutation.bonf | 29.0                | 18.0                | 39.4                | 26.5                | 15.1                | 43.3                | 28.1                | 16.2                | 39.4                |
| logn continuous       | asymptotic       | 72.5                | 49.2                | 84.8                | 70.1                | 52.3                | 84.0                | 69.4                | 50.4                | 84.3                |
|                       | asymptotic.bonf  | 70.3                | 47.1                | 84.0                | 68.2                | 50.3                | 82.6                | 68.0                | 48.3                | 83.0                |
|                       | permutation.bonf | 69.4                | 46.0                | 82.6                | 67.0                | 48.2                | 82.7                | 67.4                | 47.3                | 82.5                |
| logn discrete         | asymptotic       | 80.5                | 58.2                | 91.2                | 78.3                | 61.6                | 89.7                | 78.1                | 59.7                | 89.9                |
|                       | asymptotic.bonf  | 79.1                | 56.2                | 90.2                | 76.9                | 59.5                | 88.4                | 76.8                | 57.3                | 89.0                |
|                       | permutation.bonf | 78.1                | 54.3                | 89.1                | 75.2                | 57.4                | 88.0                | 76.5                | 55.9                | 88.9                |
| pwExp continuous      | asymptotic       | 22.4                | 13.8                | 39.4                | 22.9                | 12.7                | 36.6                | 22.5                | 12.4                | 36.5                |
|                       | asymptotic.bonf  | 20.6                | 12.4                | 37.4                | 21.0                | 11.8                | 34.7                | 21.6                | 11.3                | 35.0                |
|                       | permutation.bonf | 21.2                | 11.2                | 37.0                | 20.5                | 11.4                | 34.7                | 21.3                | 11.0                | 35.5                |
| pwExp discrete        | asymptotic       | 26.6                | 15.3                | 45.4                | 26.1                | 15.2                | 43.9                | 26.1                | 14.9                | 43.3                |
|                       | asymptotic.bonf  | 25.3                | 14.6                | 43.4                | 25.0                | 13.5                | 42.1                | 25.1                | 14.0                | 41.1                |
|                       | permutation.bonf | 25.0                | 14.6                | 43.3                | 24.0                | 13.8                | 41.6                | 25.4                | 13.4                | 41.4                |
| Weib late continuous  | asymptotic       | 72.0                | 50.3                | 88.6                | 70.9                | 47.6                | 88.9                | 72.5                | 50.1                | 88.2                |
|                       | asymptotic.bonf  | 70.3                | 48.3                | 87.3                | 69.4                | 46.0                | 88.0                | 71.1                | 48.6                | 87.2                |
|                       | permutation.bonf | 69.4                | 47.8                | 85.8                | 68.5                | 44.0                | 87.8                | 70.6                | 47.8                | 87.3                |
| Weib late discrete    | asymptotic       | 81.1                | 58.1                | 92.3                | 79.1                | 58.1                | 93.6                | 80.0                | 58.1                | 93.3                |
|                       | asymptotic.bonf  | 80.0                | 56.3                | 91.8                | 77.8                | 55.8                | 93.0                | 78.7                | 56.3                | 93.2                |
|                       | permutation.bonf | 78.5                | 55.1                | 90.7                | 76.7                | 54.8                | 92.7                | 79.1                | 55.3                | 92.8                |
| Weib prop continuous  | asymptotic       | 68.9                | 47.6                | 86.6                | 68.3                | 45.4                | 86.6                | 70.9                | 48.5                | 85.8                |
|                       | asymptotic.bonf  | 67.1                | 45.4                | 85.0                | 67.2                | 44.1                | 86.0                | 69.2                | 46.6                | 84.9                |
|                       | permutation.bonf | 66.2                | 44.0                | 83.4                | 65.9                | 42.0                | 85.4                | 67.9                | 45.2                | 84.8                |
| Weib prop discrete    | asymptotic       | 79.3                | 55.6                | 91.5                | 76.9                | 55.6                | 93.1                | 78.2                | 55.2                | 92.5                |
|                       | asymptotic.bonf  | 77.2                | 53.9                | 90.9                | 75.8                | 53.3                | 92.3                | 77.1                | 53.4                | 91.5                |
|                       | permutation.bonf | 77.0                | 53.5                | 89.8                | 74.5                | 52.1                | 92.1                | 76.6                | 52.8                | 90.7                |
| Weib scale continuous | asymptotic       | 58.6                | 38.8                | 77.4                | 60.4                | 39.0                | 78.2                | 59.4                | 38.6                | 76.8                |
|                       | asymptotic.bonf  | 56.8                | 36.9                | 74.5                | 58.2                | 36.7                | 76.6                | 57.1                | 36.3                | 75.0                |
|                       | permutation.bonf | 56.1                | 35.3                | 74.5                | 56.8                | 35.1                | 76.0                | 57.1                | 35.7                | 74.1                |
| Weib scale discrete   | asymptotic       | 68.1                | 46.2                | 86.1                | 67.5                | 45.9                | 86.0                | 69.1                | 46.7                | 85.3                |
|                       | asymptotic.bonf  | 66.7                | 44.7                | 84.9                | 66.0                | 44.1                | 84.7                | 67.3                | 44.5                | 84.3                |
|                       | permutation.bonf | 65.3                | 43.2                | 83.2                | 65.2                | 43.6                | 84.2                | 65.3                | 43.4                | 83.8                |
| Weib shape continuous | asymptotic       | 45.3                | 28.3                | 61.8                | 46.3                | 29.1                | 63.6                | 45.1                | 28.9                | 64.3                |
|                       | asymptotic.bonf  | 41.7                | 25.2                | 59.3                | 43.7                | 26.6                | 61.1                | 41.9                | 27.2                | 61.3                |
|                       | permutation.bonf | 41.5                | 24.6                | 58.0                | 43.8                | 25.0                | 60.2                | 41.0                | 25.8                | 61.1                |
| Weib shape discrete   | asymptotic       | 54.7                | 36.2                | 72.7                | 57.0                | 37.1                | 74.5                | 55.4                | 36.7                | 74.0                |
|                       | asymptotic.bonf  | 51.9                | 34.4                | 70.2                | 53.7                | 34.5                | 72.0                | 51.7                | 34.7                | 71.4                |
|                       | permutation.bonf | 51.8                | 32.2                | 69.2                | 53.6                | 32.8                | 71.0                | 52.3                | 33.3                | 71.1                |

Table S53: Rejection rates in percent for the 2-by-2 design with  $\delta = 1.5$  and unbalanced medium sample sizes under unequal, low censoring.

| Distribution          | Method           | $\mathcal{H}_{0,4}$ | $\mathcal{H}_{0,5}$ | $\mathcal{H}_{0,6}$ | $\mathcal{H}_{0,1}$ | $\mathcal{H}_{0,2}$ | $\mathcal{H}_{0,3}$ | $\mathcal{H}_{0,7}$ | $\mathcal{H}_{0,8}$ | $\mathcal{H}_{0,9}$ |
|-----------------------|------------------|---------------------|---------------------|---------------------|---------------------|---------------------|---------------------|---------------------|---------------------|---------------------|
| exp early continuous  | asymptotic       | 2.6                 | 1.7                 | 4.6                 | 2.9                 | 1.5                 | 3.7                 | 2.7                 | 2.0                 | 4.4                 |
|                       | asymptotic_bonf  | 2.2                 | 1.5                 | 4.3                 | 2.9                 | 1.3                 | 3.3                 | 2.3                 | 1.8                 | 3.8                 |
|                       | permutation_bonf | 1.6                 | 1.1                 | 3.3                 | 2.2                 | 1.0                 | 2.9                 | 2.2                 | 1.7                 | 3.0                 |
| exp early discrete    | asymptotic       | 3.0                 | 1.9                 | 4.8                 | 3.5                 | 1.8                 | 4.7                 | 3.5                 | 2.2                 | 5.0                 |
|                       | asymptotic_bonf  | 2.9                 | 1.5                 | 4.4                 | 3.4                 | 1.4                 | 4.0                 | 2.8                 | 2.1                 | 4.5                 |
|                       | permutation_bonf | 1.7                 | 1.6                 | 4.0                 | 2.4                 | 1.2                 | 3.7                 | 2.3                 | 1.6                 | 4.5                 |
| exp late continuous   | asymptotic       | 2.6                 | 2.2                 | 4.7                 | 3.7                 | 1.7                 | 4.4                 | 3.2                 | 2.2                 | 5.0                 |
|                       | asymptotic_bonf  | 2.2                 | 1.9                 | 4.1                 | 3.4                 | 1.5                 | 3.9                 | 2.9                 | 2.1                 | 4.4                 |
|                       | permutation_bonf | 1.9                 | 1.5                 | 3.8                 | 2.7                 | 1.0                 | 3.1                 | 3.0                 | 1.8                 | 3.5                 |
| exp late discrete     | asymptotic       | 3.4                 | 2.0                 | 5.1                 | 4.0                 | 2.3                 | 5.0                 | 3.3                 | 2.5                 | 6.1                 |
|                       | asymptotic_bonf  | 3.0                 | 2.0                 | 4.4                 | 3.7                 | 2.1                 | 4.7                 | 3.2                 | 2.3                 | 5.4                 |
|                       | permutation_bonf | 1.8                 | 1.7                 | 4.3                 | 2.9                 | 1.5                 | 3.8                 | 2.7                 | 1.9                 | 4.9                 |
| exp prop continuous   | asymptotic       | 3.6                 | 2.5                 | 3.8                 | 2.5                 | 1.9                 | 4.6                 | 2.8                 | 2.3                 | 5.3                 |
|                       | asymptotic_bonf  | 3.1                 | 2.3                 | 3.4                 | 2.2                 | 1.7                 | 4.1                 | 2.3                 | 2.2                 | 4.9                 |
|                       | permutation_bonf | 2.4                 | 1.6                 | 3.3                 | 1.3                 | 1.2                 | 3.1                 | 2.4                 | 1.7                 | 4.2                 |
| exp prop discrete     | asymptotic       | 3.7                 | 2.9                 | 4.6                 | 3.3                 | 2.1                 | 5.2                 | 3.2                 | 2.3                 | 5.5                 |
|                       | asymptotic_bonf  | 3.5                 | 2.3                 | 4.1                 | 2.7                 | 1.9                 | 4.6                 | 2.8                 | 2.2                 | 5.0                 |
|                       | permutation_bonf | 3.5                 | 1.8                 | 3.2                 | 2.6                 | 1.3                 | 3.6                 | 2.6                 | 2.0                 | 4.8                 |
| logn continuous       | asymptotic       | 8.1                 | 5.9                 | 13.7                | 7.2                 | 5.1                 | 12.6                | 7.4                 | 6.2                 | 13.4                |
|                       | asymptotic_bonf  | 7.3                 | 5.3                 | 12.4                | 6.5                 | 4.6                 | 11.8                | 6.6                 | 5.8                 | 12.9                |
|                       | permutation_bonf | 5.7                 | 3.6                 | 10.4                | 5.2                 | 3.2                 | 10.5                | 5.5                 | 4.5                 | 11.1                |
| logn discrete         | asymptotic       | 10.3                | 6.8                 | 17.5                | 8.7                 | 5.7                 | 16.0                | 9.3                 | 6.9                 | 16.9                |
|                       | asymptotic_bonf  | 9.3                 | 6.0                 | 16.2                | 7.8                 | 5.1                 | 14.7                | 8.6                 | 6.6                 | 16.3                |
|                       | permutation_bonf | 7.0                 | 4.3                 | 12.7                | 6.2                 | 3.5                 | 12.4                | 7.2                 | 4.7                 | 13.4                |
| pwExp continuous      | asymptotic       | 1.9                 | 2.2                 | 4.5                 | 2.8                 | 1.6                 | 3.5                 | 2.6                 | 1.7                 | 4.7                 |
|                       | asymptotic_bonf  | 1.8                 | 1.6                 | 4.0                 | 2.3                 | 1.5                 | 3.0                 | 2.4                 | 1.6                 | 4.1                 |
|                       | permutation_bonf | 1.4                 | 1.8                 | 3.5                 | 1.8                 | 0.9                 | 2.5                 | 1.8                 | 1.0                 | 3.4                 |
| pwExp discrete        | asymptotic       | 2.2                 | 2.3                 | 4.4                 | 3.3                 | 2.3                 | 4.4                 | 2.9                 | 1.9                 | 5.3                 |
|                       | asymptotic_bonf  | 1.8                 | 1.9                 | 4.1                 | 2.8                 | 2.0                 | 3.8                 | 2.7                 | 1.9                 | 4.8                 |
|                       | permutation_bonf | 1.5                 | 1.7                 | 3.9                 | 2.2                 | 1.6                 | 3.3                 | 1.9                 | 1.3                 | 3.9                 |
| Weib late continuous  | asymptotic       | 9.9                 | 5.1                 | 13.8                | 8.0                 | 5.6                 | 14.0                | 10.4                | 4.9                 | 16.1                |
|                       | asymptotic_bonf  | 9.2                 | 4.2                 | 12.5                | 7.7                 | 5.0                 | 13.1                | 9.2                 | 4.8                 | 14.7                |
|                       | permutation_bonf | 7.2                 | 2.9                 | 11.2                | 5.6                 | 2.3                 | 11.1                | 8.0                 | 4.4                 | 13.0                |
| Weib late discrete    | asymptotic       | 12.1                | 6.2                 | 17.0                | 10.3                | 6.3                 | 17.9                | 14.1                | 5.9                 | 19.1                |
|                       | asymptotic_bonf  | 11.0                | 5.6                 | 15.9                | 9.4                 | 5.5                 | 16.8                | 12.8                | 5.1                 | 17.7                |
|                       | permutation_bonf | 7.5                 | 3.3                 | 13.1                | 7.3                 | 3.7                 | 14.3                | 9.9                 | 4.1                 | 14.8                |
| Weib prop continuous  | asymptotic       | 8.9                 | 4.1                 | 11.9                | 7.5                 | 5.2                 | 12.5                | 9.2                 | 4.0                 | 14.3                |
|                       | asymptotic_bonf  | 8.2                 | 3.8                 | 11.1                | 6.8                 | 4.5                 | 11.4                | 8.3                 | 3.8                 | 13.2                |
|                       | permutation_bonf | 6.7                 | 2.7                 | 9.8                 | 5.1                 | 1.9                 | 9.1                 | 7.1                 | 3.7                 | 11.5                |
| Weib prop discrete    | asymptotic       | 11.0                | 5.1                 | 14.9                | 10.1                | 5.7                 | 16.2                | 11.4                | 5.1                 | 17.3                |
|                       | asymptotic_bonf  | 10.0                | 4.6                 | 13.9                | 9.0                 | 5.0                 | 14.7                | 10.5                | 4.5                 | 15.8                |
|                       | permutation_bonf | 7.9                 | 2.9                 | 12.3                | 6.1                 | 2.4                 | 11.8                | 8.9                 | 3.8                 | 13.5                |
| Weib scale continuous | asymptotic       | 6.5                 | 2.8                 | 8.7                 | 4.9                 | 3.7                 | 8.4                 | 7.2                 | 3.4                 | 9.7                 |
|                       | asymptotic_bonf  | 5.9                 | 2.3                 | 8.1                 | 4.2                 | 3.2                 | 7.5                 | 6.1                 | 2.8                 | 8.9                 |
|                       | permutation_bonf | 5.0                 | 1.5                 | 7.2                 | 3.3                 | 1.8                 | 6.1                 | 5.0                 | 2.4                 | 7.9                 |
| Weib scale discrete   | asymptotic       | 8.3                 | 3.5                 | 10.5                | 6.9                 | 4.4                 | 10.7                | 8.6                 | 3.9                 | 11.9                |
|                       | asymptotic_bonf  | 7.5                 | 3.0                 | 8.9                 | 5.9                 | 3.8                 | 9.7                 | 7.8                 | 3.3                 | 10.6                |
|                       | permutation_bonf | 5.9                 | 1.9                 | 7.8                 | 4.1                 | 1.7                 | 7.5                 | 6.3                 | 2.4                 | 9.4                 |
| Weib shape continuous | asymptotic       | 4.2                 | 1.3                 | 5.9                 | 3.4                 | 2.2                 | 5.3                 | 4.3                 | 2.6                 | 6.0                 |
|                       | asymptotic_bonf  | 3.3                 | 0.9                 | 5.1                 | 2.6                 | 1.7                 | 4.6                 | 3.4                 | 1.7                 | 4.8                 |
|                       | permutation_bonf | 2.2                 | 0.5                 | 4.0                 | 1.9                 | 0.9                 | 4.0                 | 2.6                 | 1.7                 | 3.8                 |
| Weib shape discrete   | asymptotic       | 5.8                 | 2.1                 | 7.3                 | 4.5                 | 3.3                 | 6.9                 | 6.0                 | 3.3                 | 8.2                 |
|                       | asymptotic_bonf  | 4.6                 | 1.7                 | 6.3                 | 3.9                 | 2.5                 | 6.2                 | 4.7                 | 2.5                 | 6.8                 |
|                       | permutation_bonf | 3.2                 | 0.5                 | 5.1                 | 2.0                 | 0.8                 | 4.3                 | 3.7                 | 2.1                 | 5.1                 |

Table S54: Rejection rates in percent for the 2-by-2 design with  $\delta = 1.5$  and unbalanced small sample sizes under unequal, low censoring.

| Distribution          | Method           | $\mathcal{H}_{0,4}$ | $\mathcal{H}_{0,5}$ | $\mathcal{H}_{0,6}$ | $\mathcal{H}_{0,1}$ | $\mathcal{H}_{0,2}$ | $\mathcal{H}_{0,3}$ | $\mathcal{H}_{0,7}$ | $\mathcal{H}_{0,8}$ | $\mathcal{H}_{0,9}$ |
|-----------------------|------------------|---------------------|---------------------|---------------------|---------------------|---------------------|---------------------|---------------------|---------------------|---------------------|
| exp early continuous  | asymptotic       | 1.4                 | 0.8                 | 2.1                 | 1.5                 | 1.3                 | 0.8                 | 0.7                 | 1.2                 | 1.6                 |
|                       | asymptotic_bonf  | 1.2                 | 0.8                 | 1.6                 | 1.2                 | 1.2                 | 0.7                 | 0.6                 | 1.0                 | 1.6                 |
|                       | permutation_bonf | 0.1                 | 0.3                 | 0.6                 | 0.1                 | 0.6                 | 0.3                 | 0.2                 | 0.5                 | 1.1                 |
| exp early discrete    | asymptotic       | 1.4                 | 0.9                 | 1.9                 | 1.0                 | 1.2                 | 1.0                 | 0.6                 | 1.4                 | 1.8                 |
|                       | asymptotic_bonf  | 1.1                 | 0.8                 | 1.7                 | 1.0                 | 1.2                 | 1.0                 | 0.6                 | 1.1                 | 1.6                 |
|                       | permutation_bonf | 0.2                 | 0.2                 | 0.7                 | 0.1                 | 0.3                 | 0.5                 | 0.2                 | 0.5                 | 0.7                 |
| exp late continuous   | asymptotic       | 1.4                 | 0.7                 | 1.9                 | 1.0                 | 1.1                 | 1.1                 | 0.9                 | 1.1                 | 2.1                 |
|                       | asymptotic_bonf  | 1.2                 | 0.7                 | 1.2                 | 0.9                 | 1.0                 | 1.0                 | 0.7                 | 0.9                 | 1.7                 |
|                       | permutation_bonf | 0.0                 | 0.2                 | 0.3                 | 0.3                 | 0.3                 | 0.3                 | 0.2                 | 0.4                 | 1.4                 |
| exp late discrete     | asymptotic       | 1.5                 | 1.0                 | 1.6                 | 1.3                 | 1.0                 | 1.6                 | 0.9                 | 1.2                 | 2.1                 |
|                       | asymptotic_bonf  | 1.1                 | 0.6                 | 1.2                 | 1.1                 | 0.9                 | 1.4                 | 0.9                 | 1.0                 | 2.1                 |
|                       | permutation_bonf | 0.2                 | 0.1                 | 0.5                 | 0.2                 | 0.1                 | 0.5                 | 0.2                 | 0.4                 | 1.0                 |
| exp prop continuous   | asymptotic       | 1.5                 | 1.2                 | 1.8                 | 0.9                 | 0.9                 | 2.1                 | 1.2                 | 1.0                 | 1.6                 |
|                       | asymptotic_bonf  | 1.3                 | 1.1                 | 1.7                 | 0.9                 | 0.7                 | 2.1                 | 1.0                 | 1.0                 | 1.4                 |
|                       | permutation_bonf | 0.3                 | 0.4                 | 1.3                 | 0.2                 | 0.0                 | 0.9                 | 0.6                 | 0.2                 | 0.6                 |
| exp prop discrete     | asymptotic       | 1.5                 | 1.3                 | 2.0                 | 0.8                 | 0.8                 | 2.3                 | 1.1                 | 1.2                 | 1.6                 |
|                       | asymptotic_bonf  | 1.4                 | 1.3                 | 1.8                 | 0.7                 | 0.7                 | 1.9                 | 0.9                 | 1.1                 | 1.5                 |
|                       | permutation_bonf | 0.4                 | 0.5                 | 1.0                 | 0.2                 | 0.0                 | 0.7                 | 0.5                 | 0.2                 | 0.6                 |
| logn continuous       | asymptotic       | 1.3                 | 1.1                 | 2.4                 | 1.4                 | 1.4                 | 2.1                 | 2.0                 | 0.9                 | 2.0                 |
|                       | asymptotic_bonf  | 1.2                 | 1.0                 | 2.3                 | 1.2                 | 1.3                 | 1.7                 | 1.7                 | 0.8                 | 1.8                 |
|                       | permutation_bonf | 0.1                 | 0.2                 | 0.6                 | 0.2                 | 0.4                 | 0.5                 | 0.5                 | 0.4                 | 0.8                 |
| logn discrete         | asymptotic       | 1.2                 | 1.4                 | 2.4                 | 1.6                 | 1.2                 | 2.2                 | 2.1                 | 1.2                 | 2.4                 |
|                       | asymptotic_bonf  | 1.0                 | 1.3                 | 2.2                 | 1.5                 | 1.2                 | 2.1                 | 1.9                 | 0.9                 | 2.3                 |
|                       | permutation_bonf | 0.1                 | 0.3                 | 0.4                 | 0.1                 | 0.3                 | 0.3                 | 0.7                 | 0.4                 | 0.8                 |
| pwExp continuous      | asymptotic       | 1.0                 | 1.1                 | 1.9                 | 0.8                 | 0.8                 | 1.5                 | 0.8                 | 1.0                 | 2.0                 |
|                       | asymptotic_bonf  | 0.7                 | 1.0                 | 1.7                 | 0.5                 | 0.7                 | 1.2                 | 0.4                 | 1.0                 | 1.6                 |
|                       | permutation_bonf | 0.1                 | 0.3                 | 0.6                 | 0.2                 | 0.3                 | 0.3                 | 0.3                 | 0.2                 | 0.9                 |
| pwExp discrete        | asymptotic       | 0.9                 | 1.4                 | 1.9                 | 0.7                 | 0.6                 | 1.6                 | 0.7                 | 1.1                 | 2.2                 |
|                       | asymptotic_bonf  | 0.7                 | 1.2                 | 1.7                 | 0.7                 | 0.5                 | 1.4                 | 0.6                 | 0.9                 | 1.5                 |
|                       | permutation_bonf | 0.0                 | 0.3                 | 0.6                 | 0.1                 | 0.2                 | 0.5                 | 0.2                 | 0.4                 | 0.9                 |
| Weib late continuous  | asymptotic       | 1.9                 | 1.1                 | 3.3                 | 1.9                 | 1.6                 | 2.7                 | 1.1                 | 1.4                 | 3.0                 |
|                       | asymptotic_bonf  | 1.6                 | 1.1                 | 3.0                 | 1.7                 | 1.5                 | 2.6                 | 1.0                 | 1.1                 | 2.9                 |
|                       | permutation_bonf | 0.4                 | 0.2                 | 0.9                 | 0.2                 | 0.0                 | 0.7                 | 0.2                 | 0.5                 | 1.2                 |
| Weib late discrete    | asymptotic       | 2.3                 | 1.0                 | 3.7                 | 2.1                 | 1.7                 | 3.2                 | 2.0                 | 1.7                 | 2.8                 |
|                       | asymptotic_bonf  | 2.1                 | 0.8                 | 3.3                 | 2.0                 | 1.4                 | 2.7                 | 1.5                 | 1.3                 | 2.5                 |
|                       | permutation_bonf | 0.4                 | 0.3                 | 1.2                 | 0.3                 | 0.2                 | 0.7                 | 0.4                 | 0.5                 | 1.3                 |
| Weib prop continuous  | asymptotic       | 1.5                 | 1.2                 | 2.8                 | 1.7                 | 1.7                 | 2.4                 | 0.9                 | 1.3                 | 2.8                 |
|                       | asymptotic_bonf  | 1.3                 | 1.1                 | 2.6                 | 1.5                 | 1.4                 | 2.0                 | 0.8                 | 1.1                 | 2.2                 |
|                       | permutation_bonf | 0.2                 | 0.3                 | 0.9                 | 0.2                 | 0.1                 | 0.7                 | 0.3                 | 0.3                 | 1.1                 |
| Weib prop discrete    | asymptotic       | 1.7                 | 1.1                 | 3.2                 | 1.8                 | 1.7                 | 2.7                 | 1.4                 | 1.2                 | 2.5                 |
|                       | asymptotic_bonf  | 1.6                 | 0.9                 | 2.7                 | 1.7                 | 1.4                 | 2.5                 | 1.1                 | 1.0                 | 2.4                 |
|                       | permutation_bonf | 0.4                 | 0.1                 | 1.1                 | 0.2                 | 0.1                 | 0.6                 | 0.3                 | 0.3                 | 1.3                 |
| Weib scale continuous | asymptotic       | 1.1                 | 1.1                 | 1.7                 | 1.5                 | 1.4                 | 2.1                 | 0.9                 | 0.6                 | 1.7                 |
|                       | asymptotic_bonf  | 0.8                 | 0.9                 | 1.5                 | 1.2                 | 1.3                 | 2.1                 | 0.7                 | 0.6                 | 1.4                 |
|                       | permutation_bonf | 0.3                 | 0.3                 | 0.6                 | 0.2                 | 0.2                 | 0.5                 | 0.5                 | 0.3                 | 0.6                 |
| Weib scale discrete   | asymptotic       | 1.2                 | 1.1                 | 2.0                 | 1.6                 | 1.3                 | 2.2                 | 0.9                 | 0.8                 | 1.8                 |
|                       | asymptotic_bonf  | 1.1                 | 0.9                 | 1.8                 | 1.1                 | 1.3                 | 1.8                 | 0.8                 | 0.6                 | 1.5                 |
|                       | permutation_bonf | 0.4                 | 0.3                 | 0.7                 | 0.2                 | 0.1                 | 0.4                 | 0.4                 | 0.3                 | 0.5                 |
| Weib shape continuous | asymptotic       | 2.5                 | 1.6                 | 2.1                 | 2.0                 | 2.2                 | 1.7                 | 1.9                 | 1.1                 | 1.7                 |
|                       | asymptotic_bonf  | 2.2                 | 1.4                 | 1.7                 | 1.7                 | 2.0                 | 1.7                 | 1.9                 | 1.0                 | 1.7                 |
|                       | permutation_bonf | 0.5                 | 0.5                 | 0.7                 | 0.2                 | 0.5                 | 0.7                 | 0.8                 | 0.7                 | 1.0                 |
| Weib shape discrete   | asymptotic       | 2.9                 | 1.6                 | 2.2                 | 1.5                 | 2.1                 | 2.0                 | 1.9                 | 1.3                 | 1.9                 |
|                       | asymptotic_bonf  | 2.4                 | 1.4                 | 2.1                 | 1.3                 | 1.9                 | 1.9                 | 1.5                 | 1.2                 | 1.6                 |
|                       | permutation_bonf | 0.7                 | 0.5                 | 0.7                 | 0.3                 | 0.4                 | 0.4                 | 0.7                 | 0.6                 | 0.8                 |

Table S55: Rejection rates in percent for the Dunnett-type contrast matrix with  $\delta = 1.5$  and balanced large sample sizes under equal censoring.

| Distribution          | Method           | $\mathcal{H}_{0,7}$ | $\mathcal{H}_{0,8}$ | $\mathcal{H}_{0,9}$ |
|-----------------------|------------------|---------------------|---------------------|---------------------|
| exp early continuous  | asymptotic       | 85.6                | 65.4                | 94.9                |
|                       | asymptotic.bonf  | 84.4                | 63.7                | 94.6                |
|                       | permutation.bonf | 83.1                | 63.6                | 94.2                |
| exp early discrete    | asymptotic       | 90.7                | 71.9                | 97.3                |
|                       | asymptotic.bonf  | 89.9                | 69.9                | 97.0                |
|                       | permutation.bonf | 89.7                | 69.1                | 96.5                |
| exp late continuous   | asymptotic       | 88.2                | 68.9                | 96.3                |
|                       | asymptotic.bonf  | 87.3                | 66.9                | 96.0                |
|                       | permutation.bonf | 86.7                | 66.9                | 96.0                |
| exp late discrete     | asymptotic       | 92.7                | 74.8                | 98.1                |
|                       | asymptotic.bonf  | 91.7                | 73.6                | 98.0                |
|                       | permutation.bonf | 91.9                | 73.4                | 98.0                |
| exp prop continuous   | asymptotic       | 86.8                | 69.9                | 96.4                |
|                       | asymptotic.bonf  | 85.8                | 68.7                | 96.0                |
|                       | permutation.bonf | 84.9                | 67.5                | 96.1                |
| exp prop discrete     | asymptotic       | 90.3                | 76.5                | 97.7                |
|                       | asymptotic.bonf  | 90.0                | 75.5                | 97.6                |
|                       | permutation.bonf | 89.6                | 75.9                | 97.6                |
| logn continuous       | asymptotic       | 100.0               | 98.9                | 100.0               |
|                       | asymptotic.bonf  | 100.0               | 98.9                | 100.0               |
|                       | permutation.bonf | 100.0               | 98.8                | 100.0               |
| logn discrete         | asymptotic       | 100.0               | 99.6                | 100.0               |
|                       | asymptotic.bonf  | 100.0               | 99.5                | 100.0               |
|                       | permutation.bonf | 100.0               | 99.5                | 100.0               |
| pwExp continuous      | asymptotic       | 84.0                | 61.9                | 95.2                |
|                       | asymptotic.bonf  | 82.7                | 61.2                | 94.5                |
|                       | permutation.bonf | 83.0                | 61.9                | 94.4                |
| pwExp discrete        | asymptotic       | 89.0                | 69.7                | 96.9                |
|                       | asymptotic.bonf  | 88.4                | 68.2                | 96.8                |
|                       | permutation.bonf | 87.9                | 67.6                | 96.4                |
| Weib late continuous  | asymptotic       | 99.9                | 99.2                | 100.0               |
|                       | asymptotic.bonf  | 99.9                | 99.1                | 100.0               |
|                       | permutation.bonf | 99.9                | 98.9                | 100.0               |
| Weib late discrete    | asymptotic       | 100.0               | 99.5                | 100.0               |
|                       | asymptotic.bonf  | 100.0               | 99.5                | 100.0               |
|                       | permutation.bonf | 100.0               | 99.5                | 100.0               |
| Weib prop continuous  | asymptotic       | 99.9                | 98.7                | 100.0               |
|                       | asymptotic.bonf  | 99.9                | 98.7                | 100.0               |
|                       | permutation.bonf | 99.9                | 98.5                | 100.0               |
| Weib prop discrete    | asymptotic       | 100.0               | 99.6                | 100.0               |
|                       | asymptotic.bonf  | 100.0               | 99.4                | 100.0               |
|                       | permutation.bonf | 100.0               | 99.4                | 100.0               |
| Weib scale continuous | asymptotic       | 99.5                | 97.7                | 100.0               |
|                       | asymptotic.bonf  | 99.4                | 97.3                | 100.0               |
|                       | permutation.bonf | 99.4                | 97.3                | 100.0               |
| Weib scale discrete   | asymptotic       | 99.9                | 98.9                | 100.0               |
|                       | asymptotic.bonf  | 99.9                | 98.9                | 100.0               |
|                       | permutation.bonf | 99.9                | 98.8                | 100.0               |
| Weib shape continuous | asymptotic       | 98.7                | 94.1                | 99.7                |
|                       | asymptotic.bonf  | 98.7                | 93.4                | 99.7                |
|                       | permutation.bonf | 98.7                | 92.8                | 99.9                |
| Weib shape discrete   | asymptotic       | 99.8                | 97.2                | 100.0               |
|                       | asymptotic.bonf  | 99.7                | 97.1                | 100.0               |
|                       | permutation.bonf | 99.6                | 97.0                | 100.0               |

Table S56: Rejection rates in percent for the Dunnett-type contrast matrix with  $\delta = 1.5$  and balanced medium sample sizes under equal censoring.

| Distribution          | Method           | $\mathcal{H}_{0,7}$ | $\mathcal{H}_{0,8}$ | $\mathcal{H}_{0,9}$ |
|-----------------------|------------------|---------------------|---------------------|---------------------|
| exp early continuous  | asymptotic       | 15.5                | 10.0                | 22.0                |
|                       | asymptotic.bonf  | 14.4                | 9.5                 | 20.6                |
|                       | permutation.bonf | 14.2                | 9.2                 | 20.1                |
| exp early discrete    | asymptotic       | 18.7                | 11.3                | 26.5                |
|                       | asymptotic.bonf  | 17.5                | 10.7                | 24.6                |
|                       | permutation.bonf | 17.9                | 11.0                | 23.9                |
| exp late continuous   | asymptotic       | 17.2                | 11.4                | 23.7                |
|                       | asymptotic.bonf  | 15.6                | 10.3                | 22.2                |
|                       | permutation.bonf | 15.5                | 10.3                | 22.6                |
| exp late discrete     | asymptotic       | 20.7                | 13.3                | 29.1                |
|                       | asymptotic.bonf  | 18.8                | 12.4                | 27.8                |
|                       | permutation.bonf | 19.8                | 12.4                | 27.6                |
| exp prop continuous   | asymptotic       | 17.4                | 11.6                | 22.1                |
|                       | asymptotic.bonf  | 16.5                | 10.7                | 20.8                |
|                       | permutation.bonf | 15.7                | 11.3                | 20.0                |
| exp prop discrete     | asymptotic       | 19.5                | 13.0                | 25.5                |
|                       | asymptotic.bonf  | 18.2                | 11.8                | 24.2                |
|                       | permutation.bonf | 17.3                | 12.0                | 23.2                |
| logn continuous       | asymptotic       | 44.5                | 30.5                | 65.4                |
|                       | asymptotic.bonf  | 43.1                | 29.6                | 64.3                |
|                       | permutation.bonf | 43.8                | 29.0                | 64.3                |
| logn discrete         | asymptotic       | 51.8                | 38.0                | 71.7                |
|                       | asymptotic.bonf  | 50.4                | 36.5                | 70.9                |
|                       | permutation.bonf | 51.4                | 36.2                | 70.5                |
| pwExp continuous      | asymptotic       | 15.1                | 10.2                | 21.5                |
|                       | asymptotic.bonf  | 14.3                | 9.4                 | 20.7                |
|                       | permutation.bonf | 14.0                | 9.5                 | 20.5                |
| pwExp discrete        | asymptotic       | 17.8                | 11.9                | 25.4                |
|                       | asymptotic.bonf  | 16.6                | 11.3                | 23.7                |
|                       | permutation.bonf | 15.9                | 10.8                | 23.5                |
| Weib late continuous  | asymptotic       | 45.3                | 31.4                | 65.7                |
|                       | asymptotic.bonf  | 43.6                | 29.8                | 64.3                |
|                       | permutation.bonf | 42.5                | 29.3                | 63.1                |
| Weib late discrete    | asymptotic       | 51.9                | 36.2                | 71.1                |
|                       | asymptotic.bonf  | 50.3                | 35.0                | 69.7                |
|                       | permutation.bonf | 50.2                | 34.5                | 69.1                |
| Weib prop continuous  | asymptotic       | 41.9                | 28.1                | 62.6                |
|                       | asymptotic.bonf  | 41.0                | 27.2                | 61.9                |
|                       | permutation.bonf | 39.7                | 27.6                | 61.1                |
| Weib prop discrete    | asymptotic       | 51.8                | 35.9                | 71.0                |
|                       | asymptotic.bonf  | 50.5                | 34.3                | 70.1                |
|                       | permutation.bonf | 50.5                | 34.6                | 68.5                |
| Weib scale continuous | asymptotic       | 35.8                | 23.8                | 53.7                |
|                       | asymptotic.bonf  | 33.9                | 22.8                | 52.4                |
|                       | permutation.bonf | 33.7                | 24.4                | 52.6                |
| Weib scale discrete   | asymptotic       | 44.6                | 29.4                | 61.4                |
|                       | asymptotic.bonf  | 43.5                | 28.5                | 59.5                |
|                       | permutation.bonf | 42.4                | 28.5                | 59.3                |
| Weib shape continuous | asymptotic       | 27.1                | 17.1                | 41.2                |
|                       | asymptotic.bonf  | 25.7                | 16.3                | 40.1                |
|                       | permutation.bonf | 24.2                | 17.5                | 38.6                |
| Weib shape discrete   | asymptotic       | 33.3                | 22.9                | 50.3                |
|                       | asymptotic.bonf  | 32.5                | 21.8                | 48.9                |
|                       | permutation.bonf | 32.6                | 21.9                | 47.5                |

Table S57: Rejection rates in percent for the Dunnett-type contrast matrix with  $\delta = 1.5$  and balanced small sample sizes under equal censoring.

| Distribution          | Method           | $\mathcal{H}_{0,7}$ | $\mathcal{H}_{0,8}$ | $\mathcal{H}_{0,9}$ |
|-----------------------|------------------|---------------------|---------------------|---------------------|
| exp early continuous  | asymptotic       | 3.1                 | 1.3                 | 3.2                 |
|                       | asymptotic.bonf  | 2.7                 | 1.2                 | 3.0                 |
|                       | permutation.bonf | 2.4                 | 1.0                 | 2.2                 |
| exp early discrete    | asymptotic       | 3.0                 | 2.3                 | 2.6                 |
|                       | asymptotic.bonf  | 2.8                 | 2.2                 | 2.5                 |
|                       | permutation.bonf | 2.6                 | 1.5                 | 2.6                 |
| exp late continuous   | asymptotic       | 3.4                 | 1.6                 | 3.6                 |
|                       | asymptotic.bonf  | 3.0                 | 1.6                 | 3.1                 |
|                       | permutation.bonf | 2.6                 | 1.0                 | 2.6                 |
| exp late discrete     | asymptotic       | 3.6                 | 1.6                 | 4.1                 |
|                       | asymptotic.bonf  | 3.5                 | 1.1                 | 3.8                 |
|                       | permutation.bonf | 2.9                 | 1.4                 | 3.3                 |
| exp prop continuous   | asymptotic       | 2.0                 | 1.8                 | 3.2                 |
|                       | asymptotic.bonf  | 1.9                 | 1.7                 | 3.1                 |
|                       | permutation.bonf | 1.4                 | 1.3                 | 2.5                 |
| exp prop discrete     | asymptotic       | 2.8                 | 1.6                 | 4.9                 |
|                       | asymptotic.bonf  | 2.5                 | 1.5                 | 4.5                 |
|                       | permutation.bonf | 2.2                 | 1.4                 | 4.0                 |
| logn continuous       | asymptotic       | 6.4                 | 4.6                 | 11.0                |
|                       | asymptotic.bonf  | 6.0                 | 4.1                 | 10.4                |
|                       | permutation.bonf | 6.2                 | 3.5                 | 9.0                 |
| logn discrete         | asymptotic       | 8.4                 | 5.3                 | 12.7                |
|                       | asymptotic.bonf  | 7.9                 | 5.1                 | 11.6                |
|                       | permutation.bonf | 7.2                 | 4.4                 | 10.7                |
| pwExp continuous      | asymptotic       | 2.5                 | 1.3                 | 3.1                 |
|                       | asymptotic.bonf  | 2.5                 | 1.3                 | 2.5                 |
|                       | permutation.bonf | 1.9                 | 0.9                 | 1.7                 |
| pwExp discrete        | asymptotic       | 2.6                 | 1.3                 | 3.6                 |
|                       | asymptotic.bonf  | 2.4                 | 1.2                 | 3.4                 |
|                       | permutation.bonf | 2.2                 | 1.0                 | 2.3                 |
| Weib late continuous  | asymptotic       | 5.8                 | 5.7                 | 8.9                 |
|                       | asymptotic.bonf  | 5.5                 | 5.4                 | 8.3                 |
|                       | permutation.bonf | 5.1                 | 5.1                 | 7.0                 |
| Weib late discrete    | asymptotic       | 7.1                 | 6.7                 | 10.7                |
|                       | asymptotic.bonf  | 6.8                 | 6.1                 | 9.7                 |
|                       | permutation.bonf | 6.4                 | 5.4                 | 8.5                 |
| Weib prop continuous  | asymptotic       | 5.5                 | 5.5                 | 8.0                 |
|                       | asymptotic.bonf  | 5.2                 | 5.4                 | 7.6                 |
|                       | permutation.bonf | 5.0                 | 4.4                 | 6.0                 |
| Weib prop discrete    | asymptotic       | 6.3                 | 6.3                 | 9.5                 |
|                       | asymptotic.bonf  | 6.1                 | 5.8                 | 9.0                 |
|                       | permutation.bonf | 5.6                 | 5.2                 | 7.3                 |
| Weib scale continuous | asymptotic       | 4.3                 | 3.7                 | 5.8                 |
|                       | asymptotic.bonf  | 4.2                 | 3.5                 | 5.2                 |
|                       | permutation.bonf | 3.3                 | 3.4                 | 4.0                 |
| Weib scale discrete   | asymptotic       | 4.1                 | 4.5                 | 5.9                 |
|                       | asymptotic.bonf  | 3.8                 | 4.1                 | 5.3                 |
|                       | permutation.bonf | 3.9                 | 4.2                 | 5.2                 |
| Weib shape continuous | asymptotic       | 1.7                 | 2.8                 | 3.6                 |
|                       | asymptotic.bonf  | 1.7                 | 2.4                 | 3.3                 |
|                       | permutation.bonf | 1.6                 | 2.4                 | 3.2                 |
| Weib shape discrete   | asymptotic       | 2.7                 | 3.1                 | 4.3                 |
|                       | asymptotic.bonf  | 2.3                 | 3.0                 | 3.9                 |
|                       | permutation.bonf | 2.0                 | 3.1                 | 3.1                 |



Table S58: Rejection rates in percent for the Dunnett-type contrast matrix with  $\delta = 1.5$  and unbalanced large sample sizes under equal censoring.

| Distribution          | Method           | $\mathcal{H}_{0,7}$ | $\mathcal{H}_{0,8}$ | $\mathcal{H}_{0,9}$ |
|-----------------------|------------------|---------------------|---------------------|---------------------|
| exp early continuous  | asymptotic       | 36.8                | 20.8                | 59.5                |
|                       | asymptotic.bonf  | 36.1                | 20.1                | 58.4                |
|                       | permutation.bonf | 32.4                | 18.1                | 57.2                |
| exp early discrete    | asymptotic       | 42.7                | 25.5                | 65.7                |
|                       | asymptotic.bonf  | 41.8                | 24.5                | 64.5                |
|                       | permutation.bonf | 38.4                | 22.0                | 64.2                |
| exp late continuous   | asymptotic       | 44.5                | 25.3                | 67.9                |
|                       | asymptotic.bonf  | 42.6                | 24.2                | 67.3                |
|                       | permutation.bonf | 39.0                | 21.4                | 66.5                |
| exp late discrete     | asymptotic       | 51.1                | 30.4                | 74.1                |
|                       | asymptotic.bonf  | 50.0                | 29.1                | 73.5                |
|                       | permutation.bonf | 46.6                | 25.0                | 71.0                |
| exp prop continuous   | asymptotic       | 42.0                | 25.2                | 60.8                |
|                       | asymptotic.bonf  | 41.4                | 24.7                | 60.0                |
|                       | permutation.bonf | 39.0                | 22.2                | 58.1                |
| exp prop discrete     | asymptotic       | 48.8                | 30.6                | 68.2                |
|                       | asymptotic.bonf  | 47.8                | 29.8                | 67.5                |
|                       | permutation.bonf | 45.6                | 26.7                | 65.1                |
| logn continuous       | asymptotic       | 88.4                | 68.3                | 95.5                |
|                       | asymptotic.bonf  | 88.3                | 67.3                | 95.4                |
|                       | permutation.bonf | 85.9                | 64.2                | 94.9                |
| logn discrete         | asymptotic       | 92.7                | 76.6                | 98.0                |
|                       | asymptotic.bonf  | 92.5                | 75.9                | 97.8                |
|                       | permutation.bonf | 90.2                | 71.5                | 97.1                |
| pwExp continuous      | asymptotic       | 34.7                | 19.8                | 59.6                |
|                       | asymptotic.bonf  | 33.8                | 19.1                | 58.6                |
|                       | permutation.bonf | 32.5                | 17.0                | 57.0                |
| pwExp discrete        | asymptotic       | 42.0                | 23.7                | 66.1                |
|                       | asymptotic.bonf  | 40.9                | 23.3                | 65.3                |
|                       | permutation.bonf | 38.6                | 20.8                | 64.1                |
| Weib late continuous  | asymptotic       | 88.1                | 67.8                | 97.4                |
|                       | asymptotic.bonf  | 87.8                | 67.1                | 97.3                |
|                       | permutation.bonf | 85.6                | 62.5                | 96.8                |
| Weib late discrete    | asymptotic       | 89.9                | 73.2                | 97.1                |
|                       | asymptotic.bonf  | 89.7                | 72.9                | 97.1                |
|                       | permutation.bonf | 88.2                | 69.4                | 96.4                |
| Weib prop continuous  | asymptotic       | 85.6                | 64.5                | 96.2                |
|                       | asymptotic.bonf  | 85.2                | 63.4                | 95.9                |
|                       | permutation.bonf | 83.3                | 58.8                | 95.6                |
| Weib prop discrete    | asymptotic       | 90.3                | 72.6                | 97.9                |
|                       | asymptotic.bonf  | 90.0                | 72.3                | 97.8                |
|                       | permutation.bonf | 87.8                | 67.9                | 97.8                |
| Weib scale continuous | asymptotic       | 74.8                | 53.2                | 89.5                |
|                       | asymptotic.bonf  | 74.4                | 52.3                | 89.2                |
|                       | permutation.bonf | 72.4                | 47.1                | 87.4                |
| Weib scale discrete   | asymptotic       | 81.7                | 60.4                | 95.2                |
|                       | asymptotic.bonf  | 81.7                | 60.0                | 95.1                |
|                       | permutation.bonf | 78.4                | 55.7                | 93.2                |
| Weib shape continuous | asymptotic       | 60.0                | 34.8                | 76.9                |
|                       | asymptotic.bonf  | 59.1                | 34.5                | 76.4                |
|                       | permutation.bonf | 53.5                | 27.9                | 73.6                |
| Weib shape discrete   | asymptotic       | 70.5                | 47.1                | 85.1                |
|                       | asymptotic.bonf  | 70.0                | 46.1                | 85.1                |
|                       | permutation.bonf | 65.2                | 39.3                | 83.4                |

Table S59: Rejection rates in percent for the Dunnett-type contrast matrix with  $\delta = 1.5$  and unbalanced medium sample sizes under equal censoring.

| Distribution          | Method           | $\mathcal{H}_{0,7}$ | $\mathcal{H}_{0,8}$ | $\mathcal{H}_{0,9}$ |
|-----------------------|------------------|---------------------|---------------------|---------------------|
| exp early continuous  | asymptotic       | 3.1                 | 2.3                 | 5.2                 |
|                       | asymptotic.bonf  | 3.0                 | 2.3                 | 5.0                 |
|                       | permutation.bonf | 1.3                 | 0.9                 | 3.1                 |
| exp early discrete    | asymptotic       | 3.6                 | 2.6                 | 6.3                 |
|                       | asymptotic.bonf  | 3.3                 | 2.3                 | 6.1                 |
|                       | permutation.bonf | 1.7                 | 0.8                 | 4.1                 |
| exp late continuous   | asymptotic       | 4.2                 | 2.2                 | 7.1                 |
|                       | asymptotic.bonf  | 3.6                 | 2.2                 | 6.9                 |
|                       | permutation.bonf | 2.0                 | 0.9                 | 4.5                 |
| exp late discrete     | asymptotic       | 5.2                 | 2.6                 | 7.7                 |
|                       | asymptotic.bonf  | 4.6                 | 2.6                 | 7.1                 |
|                       | permutation.bonf | 2.5                 | 1.1                 | 5.3                 |
| exp prop continuous   | asymptotic       | 4.3                 | 2.4                 | 5.2                 |
|                       | asymptotic.bonf  | 4.1                 | 2.0                 | 4.8                 |
|                       | permutation.bonf | 2.4                 | 1.0                 | 3.2                 |
| exp prop discrete     | asymptotic       | 4.9                 | 2.6                 | 6.2                 |
|                       | asymptotic.bonf  | 4.6                 | 2.4                 | 6.1                 |
|                       | permutation.bonf | 2.4                 | 0.7                 | 3.7                 |
| logn continuous       | asymptotic       | 9.9                 | 6.3                 | 18.2                |
|                       | asymptotic.bonf  | 9.5                 | 6.3                 | 17.9                |
|                       | permutation.bonf | 3.8                 | 0.7                 | 10.2                |
| logn discrete         | asymptotic       | 12.1                | 7.1                 | 21.5                |
|                       | asymptotic.bonf  | 11.7                | 7.0                 | 20.9                |
|                       | permutation.bonf | 3.9                 | 0.7                 | 11.3                |
| pwExp continuous      | asymptotic       | 3.1                 | 2.1                 | 4.3                 |
|                       | asymptotic.bonf  | 2.8                 | 2.1                 | 4.3                 |
|                       | permutation.bonf | 1.3                 | 0.8                 | 3.3                 |
| pwExp discrete        | asymptotic       | 3.9                 | 2.2                 | 5.9                 |
|                       | asymptotic.bonf  | 3.6                 | 2.1                 | 5.6                 |
|                       | permutation.bonf | 1.6                 | 0.8                 | 3.9                 |
| Weib late continuous  | asymptotic       | 12.1                | 5.8                 | 22.1                |
|                       | asymptotic.bonf  | 11.6                | 5.5                 | 21.3                |
|                       | permutation.bonf | 5.0                 | 0.7                 | 13.2                |
| Weib late discrete    | asymptotic       | 14.0                | 7.2                 | 26.6                |
|                       | asymptotic.bonf  | 13.6                | 6.4                 | 25.8                |
|                       | permutation.bonf | 6.4                 | 0.9                 | 15.9                |
| Weib prop continuous  | asymptotic       | 10.3                | 4.8                 | 19.5                |
|                       | asymptotic.bonf  | 9.8                 | 4.6                 | 18.9                |
|                       | permutation.bonf | 4.3                 | 0.5                 | 10.8                |
| Weib prop discrete    | asymptotic       | 11.6                | 5.9                 | 22.9                |
|                       | asymptotic.bonf  | 11.2                | 5.9                 | 22.5                |
|                       | permutation.bonf | 4.5                 | 0.5                 | 11.8                |
| Weib scale continuous | asymptotic       | 7.7                 | 2.7                 | 11.6                |
|                       | asymptotic.bonf  | 7.6                 | 2.4                 | 11.1                |
|                       | permutation.bonf | 2.0                 | 0.2                 | 6.5                 |
| Weib scale discrete   | asymptotic       | 8.6                 | 3.9                 | 13.3                |
|                       | asymptotic.bonf  | 8.4                 | 3.7                 | 12.9                |
|                       | permutation.bonf | 2.0                 | 0.2                 | 7.3                 |
| Weib shape continuous | asymptotic       | 3.7                 | 1.2                 | 5.5                 |
|                       | asymptotic.bonf  | 3.5                 | 1.2                 | 5.3                 |
|                       | permutation.bonf | 0.9                 | 0.1                 | 2.6                 |
| Weib shape discrete   | asymptotic       | 4.3                 | 1.9                 | 7.5                 |
|                       | asymptotic.bonf  | 4.2                 | 1.8                 | 7.1                 |
|                       | permutation.bonf | 0.8                 | 0.0                 | 3.0                 |

Table S60: Rejection rates in percent for the Dunnett-type contrast matrix with  $\delta = 1.5$  and unbalanced small sample sizes under equal censoring.

| Distribution          | Method           | $\mathcal{H}_{0,7}$ | $\mathcal{H}_{0,8}$ | $\mathcal{H}_{0,9}$ |
|-----------------------|------------------|---------------------|---------------------|---------------------|
| exp early continuous  | asymptotic       | 1.1                 | 3.3                 | 2.3                 |
|                       | asymptotic.bonf  | 1.0                 | 3.2                 | 2.3                 |
|                       | permutation.bonf | 0.2                 | 0.2                 | 0.2                 |
| exp early discrete    | asymptotic       | 1.2                 | 3.1                 | 2.4                 |
|                       | asymptotic.bonf  | 1.1                 | 3.1                 | 2.3                 |
|                       | permutation.bonf | 0.1                 | 0.3                 | 0.2                 |
| exp late continuous   | asymptotic       | 1.7                 | 2.2                 | 2.9                 |
|                       | asymptotic.bonf  | 1.4                 | 2.2                 | 2.7                 |
|                       | permutation.bonf | 0.1                 | 0.1                 | 0.1                 |
| exp late discrete     | asymptotic       | 1.8                 | 2.2                 | 3.2                 |
|                       | asymptotic.bonf  | 1.7                 | 2.1                 | 3.0                 |
|                       | permutation.bonf | 0.0                 | 0.2                 | 0.2                 |
| exp prop continuous   | asymptotic       | 1.8                 | 2.1                 | 2.5                 |
|                       | asymptotic.bonf  | 1.6                 | 2.1                 | 2.3                 |
|                       | permutation.bonf | 0.2                 | 0.3                 | 0.4                 |
| exp prop discrete     | asymptotic       | 1.8                 | 2.6                 | 2.6                 |
|                       | asymptotic.bonf  | 1.7                 | 2.6                 | 2.6                 |
|                       | permutation.bonf | 0.1                 | 0.3                 | 0.4                 |
| logn continuous       | asymptotic       | 3.4                 | 4.8                 | 3.1                 |
|                       | asymptotic.bonf  | 3.3                 | 4.7                 | 3.1                 |
|                       | permutation.bonf | 0.3                 | 0.3                 | 0.2                 |
| logn discrete         | asymptotic       | 3.5                 | 5.3                 | 3.0                 |
|                       | asymptotic.bonf  | 3.4                 | 5.3                 | 3.0                 |
|                       | permutation.bonf | 0.2                 | 0.2                 | 0.1                 |
| pwExp continuous      | asymptotic       | 1.4                 | 2.4                 | 2.3                 |
|                       | asymptotic.bonf  | 1.2                 | 2.4                 | 2.0                 |
|                       | permutation.bonf | 0.1                 | 0.1                 | 0.3                 |
| pwExp discrete        | asymptotic       | 1.3                 | 2.6                 | 2.5                 |
|                       | asymptotic.bonf  | 1.3                 | 2.6                 | 2.4                 |
|                       | permutation.bonf | 0.1                 | 0.1                 | 0.4                 |
| Weib late continuous  | asymptotic       | 2.8                 | 2.2                 | 3.2                 |
|                       | asymptotic.bonf  | 2.7                 | 2.2                 | 3.2                 |
|                       | permutation.bonf | 0.1                 | 0.1                 | 0.3                 |
| Weib late discrete    | asymptotic       | 2.9                 | 3.2                 | 4.0                 |
|                       | asymptotic.bonf  | 2.8                 | 3.2                 | 3.8                 |
|                       | permutation.bonf | 0.0                 | 0.1                 | 0.2                 |
| Weib prop continuous  | asymptotic       | 2.5                 | 3.3                 | 3.2                 |
|                       | asymptotic.bonf  | 2.5                 | 3.3                 | 3.0                 |
|                       | permutation.bonf | 0.1                 | 0.1                 | 0.3                 |
| Weib prop discrete    | asymptotic       | 2.8                 | 3.7                 | 3.4                 |
|                       | asymptotic.bonf  | 2.6                 | 3.6                 | 3.4                 |
|                       | permutation.bonf | 0.1                 | 0.1                 | 0.2                 |
| Weib scale continuous | asymptotic       | 3.3                 | 4.6                 | 2.5                 |
|                       | asymptotic.bonf  | 3.3                 | 4.5                 | 2.5                 |
|                       | permutation.bonf | 0.2                 | 0.4                 | 0.5                 |
| Weib scale discrete   | asymptotic       | 3.5                 | 5.7                 | 2.9                 |
|                       | asymptotic.bonf  | 3.5                 | 5.7                 | 2.9                 |
|                       | permutation.bonf | 0.2                 | 0.5                 | 0.3                 |
| Weib shape continuous | asymptotic       | 6.2                 | 9.3                 | 3.5                 |
|                       | asymptotic.bonf  | 6.1                 | 9.3                 | 3.3                 |
|                       | permutation.bonf | 1.3                 | 1.0                 | 1.2                 |
| Weib shape discrete   | asymptotic       | 6.3                 | 9.5                 | 3.7                 |
|                       | asymptotic.bonf  | 6.3                 | 9.5                 | 3.5                 |
|                       | permutation.bonf | 0.7                 | 1.0                 | 1.0                 |

Table S61: Rejection rates in percent for the Dunnett-type contrast matrix with  $\delta = 1.5$  and balanced large sample sizes under unequal, high censoring.

| Distribution          | Method           | $\mathcal{H}_{0,7}$ | $\mathcal{H}_{0,8}$ | $\mathcal{H}_{0,9}$ |
|-----------------------|------------------|---------------------|---------------------|---------------------|
| exp early continuous  | asymptotic       | 74.9                | 56.0                | 89.5                |
|                       | asymptotic.bonf  | 73.2                | 54.1                | 88.8                |
|                       | permutation.bonf | 72.8                | 52.6                | 88.5                |
| exp early discrete    | asymptotic       | 78.5                | 59.2                | 91.4                |
|                       | asymptotic.bonf  | 77.1                | 57.0                | 91.0                |
|                       | permutation.bonf | 77.1                | 56.9                | 90.5                |
| exp late continuous   | asymptotic       | 77.3                | 57.1                | 90.3                |
|                       | asymptotic.bonf  | 75.3                | 54.6                | 89.5                |
|                       | permutation.bonf | 73.8                | 53.5                | 89.5                |
| exp late discrete     | asymptotic       | 79.7                | 60.8                | 92.1                |
|                       | asymptotic.bonf  | 78.5                | 59.5                | 91.6                |
|                       | permutation.bonf | 78.4                | 58.5                | 91.5                |
| exp prop continuous   | asymptotic       | 75.1                | 57.2                | 89.7                |
|                       | asymptotic.bonf  | 74.0                | 55.5                | 89.3                |
|                       | permutation.bonf | 73.5                | 54.6                | 89.0                |
| exp prop discrete     | asymptotic       | 79.3                | 61.5                | 92.6                |
|                       | asymptotic.bonf  | 78.2                | 59.2                | 91.6                |
|                       | permutation.bonf | 78.5                | 58.7                | 92.0                |
| logn continuous       | asymptotic       | 99.2                | 93.3                | 99.8                |
|                       | asymptotic.bonf  | 98.7                | 92.9                | 99.8                |
|                       | permutation.bonf | 98.7                | 92.8                | 99.7                |
| logn discrete         | asymptotic       | 99.6                | 96.5                | 100.0               |
|                       | asymptotic.bonf  | 99.5                | 96.1                | 100.0               |
|                       | permutation.bonf | 99.8                | 96.4                | 100.0               |
| pwExp continuous      | asymptotic       | 73.2                | 53.7                | 89.2                |
|                       | asymptotic.bonf  | 71.1                | 51.3                | 88.5                |
|                       | permutation.bonf | 70.4                | 51.7                | 88.2                |
| pwExp discrete        | asymptotic       | 77.8                | 57.8                | 91.6                |
|                       | asymptotic.bonf  | 75.7                | 56.6                | 90.6                |
|                       | permutation.bonf | 75.1                | 55.4                | 90.7                |
| Weib late continuous  | asymptotic       | 98.9                | 93.1                | 100.0               |
|                       | asymptotic.bonf  | 98.8                | 92.7                | 100.0               |
|                       | permutation.bonf | 98.6                | 92.3                | 100.0               |
| Weib late discrete    | asymptotic       | 99.7                | 96.4                | 100.0               |
|                       | asymptotic.bonf  | 99.6                | 96.4                | 100.0               |
|                       | permutation.bonf | 99.5                | 96.1                | 99.9                |
| Weib prop continuous  | asymptotic       | 98.5                | 92.3                | 100.0               |
|                       | asymptotic.bonf  | 98.3                | 91.8                | 100.0               |
|                       | permutation.bonf | 98.4                | 91.9                | 100.0               |
| Weib prop discrete    | asymptotic       | 99.5                | 95.9                | 100.0               |
|                       | asymptotic.bonf  | 99.5                | 95.9                | 100.0               |
|                       | permutation.bonf | 99.5                | 95.6                | 100.0               |
| Weib scale continuous | asymptotic       | 98.2                | 89.4                | 99.8                |
|                       | asymptotic.bonf  | 97.9                | 88.9                | 99.8                |
|                       | permutation.bonf | 97.5                | 89.1                | 99.8                |
| Weib scale discrete   | asymptotic       | 99.2                | 94.5                | 100.0               |
|                       | asymptotic.bonf  | 99.0                | 93.9                | 100.0               |
|                       | permutation.bonf | 98.9                | 94.1                | 100.0               |
| Weib shape continuous | asymptotic       | 97.0                | 85.8                | 99.4                |
|                       | asymptotic.bonf  | 96.4                | 85.0                | 99.3                |
|                       | permutation.bonf | 96.3                | 85.0                | 99.3                |
| Weib shape discrete   | asymptotic       | 98.5                | 92.0                | 99.8                |
|                       | asymptotic.bonf  | 98.4                | 91.2                | 99.8                |
|                       | permutation.bonf | 97.9                | 90.8                | 99.7                |

Table S62: Rejection rates in percent for the Dunnett-type contrast matrix with  $\delta = 1.5$  and balanced medium sample sizes under unequal, high censoring.

| Distribution          | Method           | $\mathcal{H}_{0,7}$ | $\mathcal{H}_{0,8}$ | $\mathcal{H}_{0,9}$ |
|-----------------------|------------------|---------------------|---------------------|---------------------|
| exp early continuous  | asymptotic       | 13.0                | 7.7                 | 16.4                |
|                       | asymptotic.bonf  | 12.3                | 6.9                 | 15.2                |
|                       | permutation.bonf | 11.9                | 6.8                 | 14.6                |
| exp early discrete    | asymptotic       | 13.9                | 7.4                 | 18.6                |
|                       | asymptotic.bonf  | 13.3                | 6.7                 | 17.5                |
|                       | permutation.bonf | 13.3                | 7.1                 | 17.3                |
| exp late continuous   | asymptotic       | 12.0                | 8.2                 | 17.7                |
|                       | asymptotic.bonf  | 11.5                | 7.8                 | 16.9                |
|                       | permutation.bonf | 11.2                | 7.5                 | 16.6                |
| exp late discrete     | asymptotic       | 15.1                | 7.6                 | 19.7                |
|                       | asymptotic.bonf  | 13.8                | 7.0                 | 18.4                |
|                       | permutation.bonf | 13.6                | 7.0                 | 18.5                |
| exp prop continuous   | asymptotic       | 13.2                | 9.2                 | 17.7                |
|                       | asymptotic.bonf  | 12.4                | 8.6                 | 16.1                |
|                       | permutation.bonf | 11.9                | 8.7                 | 16.2                |
| exp prop discrete     | asymptotic       | 14.9                | 9.7                 | 19.0                |
|                       | asymptotic.bonf  | 14.1                | 9.1                 | 17.9                |
|                       | permutation.bonf | 14.2                | 8.7                 | 17.6                |
| logn continuous       | asymptotic       | 27.6                | 18.6                | 46.1                |
|                       | asymptotic.bonf  | 26.2                | 17.2                | 45.5                |
|                       | permutation.bonf | 26.0                | 16.6                | 44.0                |
| logn discrete         | asymptotic       | 33.6                | 21.4                | 54.5                |
|                       | asymptotic.bonf  | 32.3                | 20.8                | 53.2                |
|                       | permutation.bonf | 32.0                | 20.9                | 51.3                |
| pwExp continuous      | asymptotic       | 11.6                | 7.4                 | 17.1                |
|                       | asymptotic.bonf  | 10.5                | 7.1                 | 16.4                |
|                       | permutation.bonf | 10.2                | 7.0                 | 15.3                |
| pwExp discrete        | asymptotic       | 14.0                | 7.7                 | 18.9                |
|                       | asymptotic.bonf  | 13.1                | 7.4                 | 17.8                |
|                       | permutation.bonf | 13.7                | 7.5                 | 17.7                |
| Weib late continuous  | asymptotic       | 30.2                | 18.5                | 46.3                |
|                       | asymptotic.bonf  | 29.1                | 17.9                | 44.7                |
|                       | permutation.bonf | 27.9                | 17.3                | 45.0                |
| Weib late discrete    | asymptotic       | 34.5                | 22.2                | 50.8                |
|                       | asymptotic.bonf  | 33.1                | 20.7                | 49.5                |
|                       | permutation.bonf | 32.5                | 19.8                | 48.2                |
| Weib prop continuous  | asymptotic       | 29.6                | 17.2                | 43.9                |
|                       | asymptotic.bonf  | 28.4                | 16.1                | 43.0                |
|                       | permutation.bonf | 26.1                | 17.1                | 41.8                |
| Weib prop discrete    | asymptotic       | 34.7                | 21.8                | 52.6                |
|                       | asymptotic.bonf  | 33.1                | 20.4                | 51.8                |
|                       | permutation.bonf | 32.4                | 20.9                | 50.7                |
| Weib scale continuous | asymptotic       | 24.4                | 15.3                | 39.6                |
|                       | asymptotic.bonf  | 23.2                | 14.7                | 38.7                |
|                       | permutation.bonf | 22.7                | 14.2                | 38.4                |
| Weib scale discrete   | asymptotic       | 29.6                | 18.6                | 47.8                |
|                       | asymptotic.bonf  | 28.4                | 18.1                | 46.2                |
|                       | permutation.bonf | 27.8                | 18.0                | 46.0                |
| Weib shape continuous | asymptotic       | 20.5                | 13.0                | 34.0                |
|                       | asymptotic.bonf  | 19.8                | 11.6                | 33.0                |
|                       | permutation.bonf | 18.5                | 12.3                | 31.4                |
| Weib shape discrete   | asymptotic       | 24.8                | 15.1                | 39.1                |
|                       | asymptotic.bonf  | 24.2                | 14.5                | 38.3                |
|                       | permutation.bonf | 23.2                | 14.4                | 38.2                |

Table S63: Rejection rates in percent for the Dunnett-type contrast matrix with  $\delta = 1.5$  and balanced small sample sizes under unequal, high censoring.

| Distribution          | Method           | $\mathcal{H}_{0,7}$ | $\mathcal{H}_{0,8}$ | $\mathcal{H}_{0,9}$ |
|-----------------------|------------------|---------------------|---------------------|---------------------|
| exp early continuous  | asymptotic       | 3.0                 | 1.7                 | 3.6                 |
|                       | asymptotic.bonf  | 2.6                 | 1.7                 | 3.4                 |
|                       | permutation.bonf | 2.3                 | 1.4                 | 3.0                 |
| exp early discrete    | asymptotic       | 2.3                 | 1.9                 | 2.2                 |
|                       | asymptotic.bonf  | 2.1                 | 1.7                 | 2.0                 |
|                       | permutation.bonf | 1.9                 | 1.6                 | 1.7                 |
| exp late continuous   | asymptotic       | 2.8                 | 2.1                 | 4.4                 |
|                       | asymptotic.bonf  | 2.7                 | 1.7                 | 3.9                 |
|                       | permutation.bonf | 2.0                 | 1.6                 | 2.7                 |
| exp late discrete     | asymptotic       | 3.3                 | 1.7                 | 3.8                 |
|                       | asymptotic.bonf  | 3.1                 | 1.6                 | 3.5                 |
|                       | permutation.bonf | 2.5                 | 1.3                 | 2.9                 |
| exp prop continuous   | asymptotic       | 1.8                 | 2.0                 | 3.7                 |
|                       | asymptotic.bonf  | 1.6                 | 2.0                 | 3.5                 |
|                       | permutation.bonf | 1.0                 | 1.9                 | 2.3                 |
| exp prop discrete     | asymptotic       | 2.6                 | 1.7                 | 3.8                 |
|                       | asymptotic.bonf  | 2.4                 | 1.3                 | 3.5                 |
|                       | permutation.bonf | 1.6                 | 1.2                 | 2.9                 |
| logn continuous       | asymptotic       | 4.7                 | 3.1                 | 8.0                 |
|                       | asymptotic.bonf  | 4.5                 | 2.7                 | 7.6                 |
|                       | permutation.bonf | 4.4                 | 2.3                 | 6.5                 |
| logn discrete         | asymptotic       | 5.6                 | 3.9                 | 8.2                 |
|                       | asymptotic.bonf  | 5.4                 | 3.5                 | 8.0                 |
|                       | permutation.bonf | 4.5                 | 3.5                 | 6.5                 |
| pwExp continuous      | asymptotic       | 2.3                 | 1.8                 | 3.7                 |
|                       | asymptotic.bonf  | 2.2                 | 1.8                 | 3.4                 |
|                       | permutation.bonf | 1.7                 | 1.5                 | 2.2                 |
| pwExp discrete        | asymptotic       | 2.8                 | 1.9                 | 4.2                 |
|                       | asymptotic.bonf  | 2.6                 | 1.9                 | 4.0                 |
|                       | permutation.bonf | 2.1                 | 1.6                 | 3.0                 |
| Weib late continuous  | asymptotic       | 3.7                 | 4.4                 | 7.6                 |
|                       | asymptotic.bonf  | 3.5                 | 4.3                 | 7.2                 |
|                       | permutation.bonf | 2.1                 | 3.5                 | 5.7                 |
| Weib late discrete    | asymptotic       | 4.4                 | 5.4                 | 9.0                 |
|                       | asymptotic.bonf  | 4.0                 | 5.2                 | 8.6                 |
|                       | permutation.bonf | 2.6                 | 4.6                 | 7.3                 |
| Weib prop continuous  | asymptotic       | 3.2                 | 4.5                 | 7.5                 |
|                       | asymptotic.bonf  | 2.9                 | 4.4                 | 6.9                 |
|                       | permutation.bonf | 2.5                 | 3.2                 | 5.1                 |
| Weib prop discrete    | asymptotic       | 4.1                 | 5.0                 | 8.6                 |
|                       | asymptotic.bonf  | 3.7                 | 4.8                 | 8.4                 |
|                       | permutation.bonf | 2.6                 | 3.7                 | 6.4                 |
| Weib scale continuous | asymptotic       | 2.1                 | 3.4                 | 4.9                 |
|                       | asymptotic.bonf  | 2.0                 | 3.3                 | 4.8                 |
|                       | permutation.bonf | 1.5                 | 3.2                 | 3.7                 |
| Weib scale discrete   | asymptotic       | 2.3                 | 4.1                 | 5.5                 |
|                       | asymptotic.bonf  | 2.1                 | 3.7                 | 5.1                 |
|                       | permutation.bonf | 1.6                 | 3.5                 | 4.3                 |
| Weib shape continuous | asymptotic       | 1.6                 | 2.3                 | 3.8                 |
|                       | asymptotic.bonf  | 1.5                 | 2.1                 | 3.6                 |
|                       | permutation.bonf | 1.4                 | 1.8                 | 2.8                 |
| Weib shape discrete   | asymptotic       | 1.3                 | 2.7                 | 4.4                 |
|                       | asymptotic.bonf  | 1.3                 | 2.4                 | 4.0                 |
|                       | permutation.bonf | 1.0                 | 2.2                 | 3.7                 |

Table S64: Rejection rates in percent for the Dunnett-type contrast matrix with  $\delta = 1.5$  and unbalanced large sample sizes under unequal, high censoring.

| Distribution          | Method           | $\mathcal{H}_{0,7}$ | $\mathcal{H}_{0,8}$ | $\mathcal{H}_{0,9}$ |
|-----------------------|------------------|---------------------|---------------------|---------------------|
| exp early continuous  | asymptotic       | 30.9                | 17.7                | 53.0                |
|                       | asymptotic.bonf  | 30.1                | 16.9                | 52.0                |
|                       | permutation.bonf | 28.0                | 14.3                | 50.3                |
| exp early discrete    | asymptotic       | 34.0                | 19.8                | 56.3                |
|                       | asymptotic.bonf  | 33.2                | 19.0                | 55.8                |
|                       | permutation.bonf | 31.5                | 17.4                | 54.0                |
| exp late continuous   | asymptotic       | 32.8                | 18.7                | 57.5                |
|                       | asymptotic.bonf  | 31.7                | 17.6                | 56.0                |
|                       | permutation.bonf | 30.2                | 15.5                | 54.3                |
| exp late discrete     | asymptotic       | 37.0                | 20.5                | 61.1                |
|                       | asymptotic.bonf  | 36.3                | 19.9                | 60.2                |
|                       | permutation.bonf | 33.6                | 16.9                | 57.9                |
| exp prop continuous   | asymptotic       | 32.2                | 20.4                | 49.3                |
|                       | asymptotic.bonf  | 31.1                | 19.5                | 48.4                |
|                       | permutation.bonf | 28.8                | 18.3                | 46.8                |
| exp prop discrete     | asymptotic       | 35.5                | 22.7                | 54.1                |
|                       | asymptotic.bonf  | 34.5                | 22.5                | 53.1                |
|                       | permutation.bonf | 32.1                | 18.7                | 50.7                |
| logn continuous       | asymptotic       | 71.7                | 47.6                | 84.4                |
|                       | asymptotic.bonf  | 70.9                | 47.1                | 84.0                |
|                       | permutation.bonf | 66.3                | 39.0                | 81.9                |
| logn discrete         | asymptotic       | 77.1                | 54.7                | 90.7                |
|                       | asymptotic.bonf  | 76.7                | 53.9                | 90.6                |
|                       | permutation.bonf | 71.6                | 44.2                | 86.6                |
| pwExp continuous      | asymptotic       | 28.7                | 16.6                | 51.4                |
|                       | asymptotic.bonf  | 28.0                | 15.5                | 50.7                |
|                       | permutation.bonf | 26.5                | 13.4                | 49.0                |
| pwExp discrete        | asymptotic       | 33.3                | 18.2                | 56.5                |
|                       | asymptotic.bonf  | 32.5                | 17.6                | 55.6                |
|                       | permutation.bonf | 30.0                | 14.4                | 54.6                |
| Weib late continuous  | asymptotic       | 71.7                | 48.6                | 87.7                |
|                       | asymptotic.bonf  | 70.6                | 47.5                | 87.1                |
|                       | permutation.bonf | 65.2                | 38.8                | 85.9                |
| Weib late discrete    | asymptotic       | 74.6                | 52.4                | 89.3                |
|                       | asymptotic.bonf  | 74.2                | 51.7                | 88.9                |
|                       | permutation.bonf | 68.4                | 42.3                | 87.3                |
| Weib prop continuous  | asymptotic       | 68.0                | 46.1                | 85.1                |
|                       | asymptotic.bonf  | 67.3                | 44.9                | 85.0                |
|                       | permutation.bonf | 62.5                | 36.0                | 83.2                |
| Weib prop discrete    | asymptotic       | 75.6                | 51.9                | 90.5                |
|                       | asymptotic.bonf  | 74.8                | 50.9                | 90.2                |
|                       | permutation.bonf | 69.9                | 42.7                | 88.3                |
| Weib scale continuous | asymptotic       | 60.8                | 39.0                | 78.0                |
|                       | asymptotic.bonf  | 59.9                | 38.4                | 77.2                |
|                       | permutation.bonf | 55.8                | 30.8                | 74.1                |
| Weib scale discrete   | asymptotic       | 67.2                | 44.2                | 83.5                |
|                       | asymptotic.bonf  | 66.7                | 43.4                | 83.2                |
|                       | permutation.bonf | 60.4                | 35.2                | 80.3                |
| Weib shape continuous | asymptotic       | 50.9                | 30.2                | 69.3                |
|                       | asymptotic.bonf  | 50.6                | 29.6                | 68.8                |
|                       | permutation.bonf | 45.1                | 22.7                | 64.2                |
| Weib shape discrete   | asymptotic       | 58.4                | 36.5                | 75.6                |
|                       | asymptotic.bonf  | 57.7                | 36.0                | 74.6                |
|                       | permutation.bonf | 50.1                | 26.3                | 70.7                |

Table S65: Rejection rates in percent for the Dunnett-type contrast matrix with  $\delta = 1.5$  and unbalanced medium sample sizes under unequal, high censoring.

| Distribution          | Method           | $\mathcal{H}_{0,7}$ | $\mathcal{H}_{0,8}$ | $\mathcal{H}_{0,9}$ |
|-----------------------|------------------|---------------------|---------------------|---------------------|
| exp early continuous  | asymptotic       | 2.8                 | 2.3                 | 4.4                 |
|                       | asymptotic.bonf  | 2.6                 | 2.2                 | 4.3                 |
|                       | permutation.bonf | 0.6                 | 0.4                 | 2.7                 |
| exp early discrete    | asymptotic       | 3.1                 | 1.7                 | 5.3                 |
|                       | asymptotic.bonf  | 3.1                 | 1.6                 | 4.9                 |
|                       | permutation.bonf | 0.7                 | 0.3                 | 2.9                 |
| exp late continuous   | asymptotic       | 3.7                 | 2.1                 | 4.4                 |
|                       | asymptotic.bonf  | 3.6                 | 2.0                 | 4.3                 |
|                       | permutation.bonf | 0.7                 | 0.4                 | 3.0                 |
| exp late discrete     | asymptotic       | 3.3                 | 1.8                 | 5.6                 |
|                       | asymptotic.bonf  | 3.1                 | 1.7                 | 5.1                 |
|                       | permutation.bonf | 1.2                 | 0.3                 | 3.3                 |
| exp prop continuous   | asymptotic       | 3.1                 | 2.1                 | 3.9                 |
|                       | asymptotic.bonf  | 2.8                 | 1.9                 | 3.9                 |
|                       | permutation.bonf | 1.4                 | 0.5                 | 2.5                 |
| exp prop discrete     | asymptotic       | 3.6                 | 2.4                 | 4.8                 |
|                       | asymptotic.bonf  | 3.4                 | 2.2                 | 4.5                 |
|                       | permutation.bonf | 1.5                 | 0.3                 | 2.2                 |
| logn continuous       | asymptotic       | 5.4                 | 4.0                 | 10.9                |
|                       | asymptotic.bonf  | 5.2                 | 3.9                 | 10.6                |
|                       | permutation.bonf | 1.1                 | 0.0                 | 3.4                 |
| logn discrete         | asymptotic       | 6.4                 | 4.2                 | 12.6                |
|                       | asymptotic.bonf  | 6.2                 | 4.2                 | 12.1                |
|                       | permutation.bonf | 0.8                 | 0.0                 | 3.4                 |
| pwExp continuous      | asymptotic       | 2.4                 | 1.8                 | 4.8                 |
|                       | asymptotic.bonf  | 2.3                 | 1.8                 | 4.3                 |
|                       | permutation.bonf | 0.5                 | 0.6                 | 2.5                 |
| pwExp discrete        | asymptotic       | 2.5                 | 1.5                 | 5.2                 |
|                       | asymptotic.bonf  | 2.4                 | 1.5                 | 4.6                 |
|                       | permutation.bonf | 0.8                 | 0.4                 | 3.1                 |
| Weib late continuous  | asymptotic       | 7.3                 | 3.3                 | 12.8                |
|                       | asymptotic.bonf  | 6.6                 | 3.0                 | 12.4                |
|                       | permutation.bonf | 1.4                 | 0.0                 | 4.2                 |
| Weib late discrete    | asymptotic       | 7.7                 | 3.2                 | 16.6                |
|                       | asymptotic.bonf  | 7.6                 | 3.1                 | 15.4                |
|                       | permutation.bonf | 0.7                 | 0.1                 | 5.3                 |
| Weib prop continuous  | asymptotic       | 6.8                 | 2.2                 | 11.4                |
|                       | asymptotic.bonf  | 6.7                 | 2.0                 | 11.3                |
|                       | permutation.bonf | 1.2                 | 0.0                 | 4.0                 |
| Weib prop discrete    | asymptotic       | 7.8                 | 2.9                 | 14.6                |
|                       | asymptotic.bonf  | 7.3                 | 2.5                 | 14.1                |
|                       | permutation.bonf | 1.0                 | 0.1                 | 3.7                 |
| Weib scale continuous | asymptotic       | 5.0                 | 1.9                 | 7.6                 |
|                       | asymptotic.bonf  | 4.7                 | 1.7                 | 7.6                 |
|                       | permutation.bonf | 0.8                 | 0.1                 | 1.9                 |
| Weib scale discrete   | asymptotic       | 5.3                 | 1.7                 | 9.1                 |
|                       | asymptotic.bonf  | 5.2                 | 1.6                 | 8.5                 |
|                       | permutation.bonf | 0.5                 | 0.1                 | 1.5                 |
| Weib shape continuous | asymptotic       | 3.1                 | 1.8                 | 5.3                 |
|                       | asymptotic.bonf  | 3.0                 | 1.8                 | 4.9                 |
|                       | permutation.bonf | 0.4                 | 0.0                 | 1.6                 |
| Weib shape discrete   | asymptotic       | 3.6                 | 1.9                 | 5.9                 |
|                       | asymptotic.bonf  | 3.6                 | 1.9                 | 5.6                 |
|                       | permutation.bonf | 0.3                 | 0.0                 | 1.2                 |



Table S66: Rejection rates in percent for the Dunnett-type contrast matrix with  $\delta = 1.5$  and unbalanced small sample sizes under unequal, high censoring.

| Distribution          | Method           | $\mathcal{H}_{0,7}$ | $\mathcal{H}_{0,8}$ | $\mathcal{H}_{0,9}$ |
|-----------------------|------------------|---------------------|---------------------|---------------------|
| exp early continuous  | asymptotic       | 1.3                 | 4.5                 | 2.0                 |
|                       | asymptotic.bonf  | 1.3                 | 4.3                 | 1.9                 |
|                       | permutation.bonf | 0.2                 | 0.2                 | 0.1                 |
| exp early discrete    | asymptotic       | 2.2                 | 5.5                 | 2.1                 |
|                       | asymptotic.bonf  | 2.2                 | 5.5                 | 2.0                 |
|                       | permutation.bonf | 0.3                 | 0.1                 | 0.1                 |
| exp late continuous   | asymptotic       | 1.8                 | 4.1                 | 2.0                 |
|                       | asymptotic.bonf  | 1.7                 | 4.0                 | 1.9                 |
|                       | permutation.bonf | 0.2                 | 0.1                 | 0.1                 |
| exp late discrete     | asymptotic       | 2.1                 | 4.5                 | 2.7                 |
|                       | asymptotic.bonf  | 2.0                 | 4.3                 | 2.5                 |
|                       | permutation.bonf | 0.3                 | 0.0                 | 0.1                 |
| exp prop continuous   | asymptotic       | 2.0                 | 4.8                 | 2.6                 |
|                       | asymptotic.bonf  | 2.0                 | 4.6                 | 2.6                 |
|                       | permutation.bonf | 0.3                 | 0.4                 | 0.2                 |
| exp prop discrete     | asymptotic       | 2.8                 | 5.2                 | 2.7                 |
|                       | asymptotic.bonf  | 2.8                 | 5.2                 | 2.7                 |
|                       | permutation.bonf | 0.4                 | 0.2                 | 0.2                 |
| logn continuous       | asymptotic       | 5.5                 | 11.5                | 3.9                 |
|                       | asymptotic.bonf  | 5.5                 | 11.2                | 3.9                 |
|                       | permutation.bonf | 0.5                 | 0.6                 | 0.2                 |
| logn discrete         | asymptotic       | 6.1                 | 12.1                | 4.6                 |
|                       | asymptotic.bonf  | 6.0                 | 12.1                | 4.4                 |
|                       | permutation.bonf | 0.4                 | 0.8                 | 0.2                 |
| pwExp continuous      | asymptotic       | 1.5                 | 4.0                 | 2.0                 |
|                       | asymptotic.bonf  | 1.4                 | 3.9                 | 1.8                 |
|                       | permutation.bonf | 0.0                 | 0.2                 | 0.2                 |
| pwExp discrete        | asymptotic       | 1.8                 | 4.8                 | 2.0                 |
|                       | asymptotic.bonf  | 1.7                 | 4.8                 | 1.9                 |
|                       | permutation.bonf | 0.0                 | 0.1                 | 0.1                 |
| Weib late continuous  | asymptotic       | 5.2                 | 6.9                 | 4.1                 |
|                       | asymptotic.bonf  | 5.2                 | 6.8                 | 3.6                 |
|                       | permutation.bonf | 0.2                 | 0.2                 | 0.5                 |
| Weib late discrete    | asymptotic       | 7.0                 | 7.9                 | 4.9                 |
|                       | asymptotic.bonf  | 6.9                 | 7.5                 | 4.8                 |
|                       | permutation.bonf | 0.2                 | 0.4                 | 0.4                 |
| Weib prop continuous  | asymptotic       | 5.9                 | 7.3                 | 3.5                 |
|                       | asymptotic.bonf  | 5.5                 | 7.3                 | 3.3                 |
|                       | permutation.bonf | 0.3                 | 0.1                 | 0.5                 |
| Weib prop discrete    | asymptotic       | 7.2                 | 9.0                 | 5.0                 |
|                       | asymptotic.bonf  | 7.1                 | 8.6                 | 4.8                 |
|                       | permutation.bonf | 0.3                 | 0.2                 | 0.6                 |
| Weib scale continuous | asymptotic       | 6.8                 | 10.5                | 4.4                 |
|                       | asymptotic.bonf  | 6.8                 | 10.5                | 4.4                 |
|                       | permutation.bonf | 0.4                 | 0.4                 | 0.4                 |
| Weib scale discrete   | asymptotic       | 8.4                 | 11.5                | 4.5                 |
|                       | asymptotic.bonf  | 8.2                 | 11.4                | 4.4                 |
|                       | permutation.bonf | 0.2                 | 0.2                 | 0.5                 |
| Weib shape continuous | asymptotic       | 7.7                 | 12.4                | 4.0                 |
|                       | asymptotic.bonf  | 7.7                 | 12.4                | 4.0                 |
|                       | permutation.bonf | 0.9                 | 0.4                 | 0.4                 |
| Weib shape discrete   | asymptotic       | 9.3                 | 14.1                | 5.3                 |
|                       | asymptotic.bonf  | 9.3                 | 14.0                | 5.2                 |
|                       | permutation.bonf | 0.7                 | 0.5                 | 1.1                 |

Table S67: Rejection rates in percent for the Dunnett-type contrast matrix with  $\delta = 1.5$  and balanced large sample sizes under unequal, low censoring.

| Distribution          | Method           | $\mathcal{H}_{0,7}$ | $\mathcal{H}_{0,8}$ | $\mathcal{H}_{0,9}$ |
|-----------------------|------------------|---------------------|---------------------|---------------------|
| exp early continuous  | asymptotic       | 84.3                | 64.0                | 94.3                |
|                       | asymptotic.bonf  | 83.7                | 61.8                | 94.0                |
|                       | permutation.bonf | 83.0                | 62.4                | 93.6                |
| exp early discrete    | asymptotic       | 89.0                | 71.3                | 96.4                |
|                       | asymptotic.bonf  | 88.2                | 69.5                | 96.1                |
|                       | permutation.bonf | 88.1                | 69.6                | 95.6                |
| exp late continuous   | asymptotic       | 86.6                | 68.1                | 95.9                |
|                       | asymptotic.bonf  | 85.9                | 66.0                | 95.6                |
|                       | permutation.bonf | 85.5                | 65.4                | 95.8                |
| exp late discrete     | asymptotic       | 91.5                | 74.7                | 97.7                |
|                       | asymptotic.bonf  | 90.7                | 72.6                | 97.5                |
|                       | permutation.bonf | 89.9                | 73.0                | 97.4                |
| exp prop continuous   | asymptotic       | 85.3                | 69.1                | 96.1                |
|                       | asymptotic.bonf  | 84.2                | 67.4                | 95.6                |
|                       | permutation.bonf | 82.8                | 67.1                | 95.7                |
| exp prop discrete     | asymptotic       | 90.0                | 75.5                | 97.9                |
|                       | asymptotic.bonf  | 89.4                | 74.5                | 97.6                |
|                       | permutation.bonf | 88.7                | 74.5                | 97.6                |
| logn continuous       | asymptotic       | 100.0               | 98.7                | 100.0               |
|                       | asymptotic.bonf  | 100.0               | 98.4                | 100.0               |
|                       | permutation.bonf | 100.0               | 98.3                | 100.0               |
| logn discrete         | asymptotic       | 100.0               | 99.8                | 100.0               |
|                       | asymptotic.bonf  | 100.0               | 99.7                | 100.0               |
|                       | permutation.bonf | 100.0               | 99.8                | 100.0               |
| pwExp continuous      | asymptotic       | 83.7                | 62.2                | 94.7                |
|                       | asymptotic.bonf  | 82.4                | 60.2                | 94.1                |
|                       | permutation.bonf | 81.6                | 59.9                | 93.9                |
| pwExp discrete        | asymptotic       | 87.6                | 69.6                | 96.2                |
|                       | asymptotic.bonf  | 86.9                | 68.3                | 96.0                |
|                       | permutation.bonf | 86.6                | 68.7                | 96.2                |
| Weib late continuous  | asymptotic       | 100.0               | 99.4                | 100.0               |
|                       | asymptotic.bonf  | 100.0               | 99.2                | 100.0               |
|                       | permutation.bonf | 100.0               | 99.2                | 100.0               |
| Weib late discrete    | asymptotic       | 100.0               | 99.8                | 100.0               |
|                       | asymptotic.bonf  | 100.0               | 99.8                | 100.0               |
|                       | permutation.bonf | 100.0               | 99.8                | 100.0               |
| Weib prop continuous  | asymptotic       | 100.0               | 99.0                | 100.0               |
|                       | asymptotic.bonf  | 99.9                | 98.8                | 100.0               |
|                       | permutation.bonf | 99.9                | 98.6                | 100.0               |
| Weib prop discrete    | asymptotic       | 100.0               | 99.8                | 100.0               |
|                       | asymptotic.bonf  | 100.0               | 99.8                | 100.0               |
|                       | permutation.bonf | 100.0               | 99.8                | 100.0               |
| Weib scale continuous | asymptotic       | 99.6                | 97.8                | 100.0               |
|                       | asymptotic.bonf  | 99.6                | 97.7                | 100.0               |
|                       | permutation.bonf | 99.6                | 97.6                | 100.0               |
| Weib scale discrete   | asymptotic       | 100.0               | 99.3                | 100.0               |
|                       | asymptotic.bonf  | 99.9                | 99.3                | 100.0               |
|                       | permutation.bonf | 99.8                | 99.1                | 100.0               |
| Weib shape continuous | asymptotic       | 98.9                | 92.7                | 99.8                |
|                       | asymptotic.bonf  | 98.6                | 92.4                | 99.8                |
|                       | permutation.bonf | 98.5                | 91.9                | 99.7                |
| Weib shape discrete   | asymptotic       | 99.6                | 97.4                | 100.0               |
|                       | asymptotic.bonf  | 99.4                | 97.2                | 100.0               |
|                       | permutation.bonf | 99.6                | 97.4                | 100.0               |

Table S68: Rejection rates in percent for the Dunnett-type contrast matrix with  $\delta = 1.5$  and balanced medium sample sizes under unequal, low censoring.

| Distribution          | Method           | $\mathcal{H}_{0,7}$ | $\mathcal{H}_{0,8}$ | $\mathcal{H}_{0,9}$ |
|-----------------------|------------------|---------------------|---------------------|---------------------|
| exp early continuous  | asymptotic       | 14.6                | 10.3                | 21.0                |
|                       | asymptotic.bonf  | 13.5                | 9.5                 | 19.0                |
|                       | permutation.bonf | 13.8                | 9.6                 | 19.9                |
| exp early discrete    | asymptotic       | 17.6                | 12.0                | 25.6                |
|                       | asymptotic.bonf  | 16.3                | 10.9                | 24.1                |
|                       | permutation.bonf | 17.6                | 11.0                | 23.1                |
| exp late continuous   | asymptotic       | 15.9                | 11.1                | 23.8                |
|                       | asymptotic.bonf  | 15.0                | 10.7                | 21.9                |
|                       | permutation.bonf | 15.5                | 11.0                | 22.2                |
| exp late discrete     | asymptotic       | 19.9                | 12.6                | 28.3                |
|                       | asymptotic.bonf  | 18.5                | 12.0                | 26.6                |
|                       | permutation.bonf | 19.2                | 12.3                | 26.7                |
| exp prop continuous   | asymptotic       | 16.2                | 10.9                | 21.1                |
|                       | asymptotic.bonf  | 15.3                | 10.2                | 19.9                |
|                       | permutation.bonf | 15.3                | 10.8                | 19.9                |
| exp prop discrete     | asymptotic       | 18.1                | 12.5                | 24.8                |
|                       | asymptotic.bonf  | 17.7                | 11.7                | 23.7                |
|                       | permutation.bonf | 16.6                | 11.3                | 23.2                |
| logn continuous       | asymptotic       | 45.0                | 32.4                | 66.6                |
|                       | asymptotic.bonf  | 42.6                | 31.2                | 64.5                |
|                       | permutation.bonf | 43.7                | 30.5                | 64.4                |
| logn discrete         | asymptotic       | 53.5                | 39.1                | 72.9                |
|                       | asymptotic.bonf  | 52.2                | 37.5                | 71.9                |
|                       | permutation.bonf | 52.5                | 37.1                | 71.5                |
| pwExp continuous      | asymptotic       | 14.8                | 10.5                | 21.9                |
|                       | asymptotic.bonf  | 13.9                | 9.7                 | 20.9                |
|                       | permutation.bonf | 13.8                | 10.2                | 20.4                |
| pwExp discrete        | asymptotic       | 17.6                | 12.5                | 24.9                |
|                       | asymptotic.bonf  | 16.7                | 11.5                | 23.4                |
|                       | permutation.bonf | 16.5                | 11.2                | 23.4                |
| Weib late continuous  | asymptotic       | 47.2                | 33.4                | 66.4                |
|                       | asymptotic.bonf  | 44.5                | 31.6                | 65.4                |
|                       | permutation.bonf | 44.6                | 32.1                | 63.5                |
| Weib late discrete    | asymptotic       | 54.9                | 40.2                | 73.7                |
|                       | asymptotic.bonf  | 53.3                | 39.1                | 72.7                |
|                       | permutation.bonf | 52.5                | 38.5                | 71.7                |
| Weib prop continuous  | asymptotic       | 44.1                | 31.3                | 64.0                |
|                       | asymptotic.bonf  | 42.8                | 30.5                | 62.4                |
|                       | permutation.bonf | 43.0                | 30.1                | 61.0                |
| Weib prop discrete    | asymptotic       | 52.9                | 38.3                | 71.7                |
|                       | asymptotic.bonf  | 51.8                | 36.8                | 70.5                |
|                       | permutation.bonf | 51.8                | 36.9                | 69.2                |
| Weib scale continuous | asymptotic       | 37.5                | 25.4                | 54.6                |
|                       | asymptotic.bonf  | 36.0                | 24.6                | 53.5                |
|                       | permutation.bonf | 34.7                | 23.9                | 52.9                |
| Weib scale discrete   | asymptotic       | 46.2                | 30.8                | 62.9                |
|                       | asymptotic.bonf  | 44.5                | 30.1                | 61.6                |
|                       | permutation.bonf | 44.5                | 29.0                | 60.9                |
| Weib shape continuous | asymptotic       | 25.6                | 18.0                | 39.9                |
|                       | asymptotic.bonf  | 25.0                | 16.7                | 38.9                |
|                       | permutation.bonf | 24.4                | 17.7                | 39.3                |
| Weib shape discrete   | asymptotic       | 34.7                | 23.2                | 51.2                |
|                       | asymptotic.bonf  | 33.0                | 22.7                | 49.6                |
|                       | permutation.bonf | 32.7                | 22.5                | 48.9                |

Table S69: Rejection rates in percent for the Dunnett-type contrast matrix with  $\delta = 1.5$  and balanced small sample sizes under unequal, low censoring.

| Distribution          | Method           | $\mathcal{H}_{0,7}$ | $\mathcal{H}_{0,8}$ | $\mathcal{H}_{0,9}$ |
|-----------------------|------------------|---------------------|---------------------|---------------------|
| exp early continuous  | asymptotic       | 3.3                 | 1.3                 | 3.2                 |
|                       | asymptotic.bonf  | 3.1                 | 1.3                 | 2.8                 |
|                       | permutation.bonf | 2.7                 | 1.3                 | 2.5                 |
| exp early discrete    | asymptotic       | 3.0                 | 2.4                 | 2.8                 |
|                       | asymptotic.bonf  | 2.8                 | 2.0                 | 2.3                 |
|                       | permutation.bonf | 2.3                 | 1.9                 | 2.1                 |
| exp late continuous   | asymptotic       | 3.3                 | 1.7                 | 3.5                 |
|                       | asymptotic.bonf  | 3.1                 | 1.4                 | 3.3                 |
|                       | permutation.bonf | 2.5                 | 1.7                 | 2.5                 |
| exp late discrete     | asymptotic       | 3.7                 | 2.0                 | 4.2                 |
|                       | asymptotic.bonf  | 3.4                 | 1.8                 | 3.8                 |
|                       | permutation.bonf | 3.2                 | 1.8                 | 3.0                 |
| exp prop continuous   | asymptotic       | 1.9                 | 1.8                 | 3.4                 |
|                       | asymptotic.bonf  | 1.6                 | 1.5                 | 3.3                 |
|                       | permutation.bonf | 1.4                 | 1.3                 | 2.9                 |
| exp prop discrete     | asymptotic       | 3.1                 | 1.7                 | 4.4                 |
|                       | asymptotic.bonf  | 3.1                 | 1.6                 | 4.0                 |
|                       | permutation.bonf | 2.6                 | 1.4                 | 3.2                 |
| logn continuous       | asymptotic       | 7.5                 | 4.9                 | 11.5                |
|                       | asymptotic.bonf  | 7.0                 | 4.6                 | 10.8                |
|                       | permutation.bonf | 6.2                 | 4.4                 | 9.1                 |
| logn discrete         | asymptotic       | 9.0                 | 6.1                 | 13.2                |
|                       | asymptotic.bonf  | 8.3                 | 5.6                 | 12.2                |
|                       | permutation.bonf | 7.9                 | 5.7                 | 11.4                |
| pwExp continuous      | asymptotic       | 2.2                 | 1.6                 | 3.0                 |
|                       | asymptotic.bonf  | 2.0                 | 1.3                 | 2.5                 |
|                       | permutation.bonf | 1.8                 | 1.5                 | 1.9                 |
| pwExp discrete        | asymptotic       | 2.8                 | 1.5                 | 3.8                 |
|                       | asymptotic.bonf  | 2.6                 | 1.5                 | 3.3                 |
|                       | permutation.bonf | 2.4                 | 1.6                 | 2.4                 |
| Weib late continuous  | asymptotic       | 7.2                 | 6.6                 | 11.1                |
|                       | asymptotic.bonf  | 7.0                 | 6.2                 | 10.5                |
|                       | permutation.bonf | 5.7                 | 5.5                 | 9.0                 |
| Weib late discrete    | asymptotic       | 8.2                 | 7.4                 | 13.2                |
|                       | asymptotic.bonf  | 8.1                 | 7.0                 | 12.4                |
|                       | permutation.bonf | 7.0                 | 6.1                 | 11.2                |
| Weib prop continuous  | asymptotic       | 6.6                 | 6.4                 | 9.8                 |
|                       | asymptotic.bonf  | 6.3                 | 5.4                 | 9.1                 |
|                       | permutation.bonf | 5.5                 | 5.3                 | 8.1                 |
| Weib prop discrete    | asymptotic       | 8.2                 | 6.9                 | 12.4                |
|                       | asymptotic.bonf  | 7.5                 | 6.3                 | 11.4                |
|                       | permutation.bonf | 7.3                 | 6.0                 | 9.7                 |
| Weib scale continuous | asymptotic       | 4.2                 | 4.1                 | 7.1                 |
|                       | asymptotic.bonf  | 3.9                 | 3.7                 | 6.4                 |
|                       | permutation.bonf | 3.4                 | 4.2                 | 5.5                 |
| Weib scale discrete   | asymptotic       | 5.1                 | 4.8                 | 8.1                 |
|                       | asymptotic.bonf  | 4.9                 | 4.5                 | 7.2                 |
|                       | permutation.bonf | 4.6                 | 4.4                 | 6.4                 |
| Weib shape continuous | asymptotic       | 1.7                 | 2.5                 | 3.9                 |
|                       | asymptotic.bonf  | 1.6                 | 2.1                 | 3.5                 |
|                       | permutation.bonf | 1.7                 | 2.4                 | 3.4                 |
| Weib shape discrete   | asymptotic       | 2.3                 | 2.8                 | 4.7                 |
|                       | asymptotic.bonf  | 2.2                 | 2.8                 | 4.5                 |
|                       | permutation.bonf | 2.3                 | 3.1                 | 4.5                 |

Table S70: Rejection rates in percent for the Dunnett-type contrast matrix with  $\delta = 1.5$  and unbalanced large sample sizes under unequal, low censoring.

| Distribution          | Method           | $\mathcal{H}_{0,7}$ | $\mathcal{H}_{0,8}$ | $\mathcal{H}_{0,9}$ |
|-----------------------|------------------|---------------------|---------------------|---------------------|
| exp early continuous  | asymptotic       | 37.4                | 21.4                | 59.5                |
|                       | asymptotic.bonf  | 36.4                | 20.5                | 58.0                |
|                       | permutation.bonf | 34.4                | 18.2                | 58.2                |
| exp early discrete    | asymptotic       | 44.0                | 26.0                | 66.6                |
|                       | asymptotic.bonf  | 43.1                | 25.0                | 65.4                |
|                       | permutation.bonf | 39.6                | 22.3                | 64.2                |
| exp late continuous   | asymptotic       | 44.7                | 25.4                | 68.7                |
|                       | asymptotic.bonf  | 43.5                | 24.7                | 68.0                |
|                       | permutation.bonf | 40.9                | 21.9                | 67.6                |
| exp late discrete     | asymptotic       | 51.7                | 30.6                | 75.9                |
|                       | asymptotic.bonf  | 51.3                | 29.6                | 75.3                |
|                       | permutation.bonf | 47.7                | 25.8                | 73.7                |
| exp prop continuous   | asymptotic       | 43.3                | 25.0                | 61.9                |
|                       | asymptotic.bonf  | 42.3                | 24.2                | 61.2                |
|                       | permutation.bonf | 40.9                | 22.2                | 59.7                |
| exp prop discrete     | asymptotic       | 48.6                | 30.9                | 68.7                |
|                       | asymptotic.bonf  | 48.0                | 29.7                | 68.1                |
|                       | permutation.bonf | 46.2                | 27.0                | 65.9                |
| logn continuous       | asymptotic       | 90.7                | 73.1                | 97.2                |
|                       | asymptotic.bonf  | 90.4                | 72.2                | 97.2                |
|                       | permutation.bonf | 88.7                | 66.7                | 96.2                |
| logn discrete         | asymptotic       | 94.5                | 81.9                | 99.0                |
|                       | asymptotic.bonf  | 94.4                | 81.7                | 98.8                |
|                       | permutation.bonf | 92.7                | 75.8                | 98.5                |
| pwExp continuous      | asymptotic       | 34.9                | 20.2                | 58.6                |
|                       | asymptotic.bonf  | 34.2                | 19.1                | 57.9                |
|                       | permutation.bonf | 33.5                | 17.5                | 56.0                |
| pwExp discrete        | asymptotic       | 41.2                | 24.2                | 66.5                |
|                       | asymptotic.bonf  | 40.8                | 23.9                | 66.2                |
|                       | permutation.bonf | 38.3                | 21.4                | 64.5                |
| Weib late continuous  | asymptotic       | 91.3                | 73.3                | 98.6                |
|                       | asymptotic.bonf  | 91.2                | 72.7                | 98.5                |
|                       | permutation.bonf | 89.7                | 68.1                | 98.1                |
| Weib late discrete    | asymptotic       | 95.4                | 81.4                | 99.3                |
|                       | asymptotic.bonf  | 95.2                | 80.4                | 99.3                |
|                       | permutation.bonf | 93.5                | 76.1                | 99.0                |
| Weib prop continuous  | asymptotic       | 88.7                | 68.8                | 97.7                |
|                       | asymptotic.bonf  | 88.5                | 67.8                | 97.6                |
|                       | permutation.bonf | 86.1                | 64.1                | 96.7                |
| Weib prop discrete    | asymptotic       | 94.2                | 78.5                | 99.1                |
|                       | asymptotic.bonf  | 93.9                | 77.8                | 99.1                |
|                       | permutation.bonf | 91.8                | 72.8                | 98.4                |
| Weib scale continuous | asymptotic       | 77.9                | 55.2                | 91.5                |
|                       | asymptotic.bonf  | 77.4                | 54.6                | 91.2                |
|                       | permutation.bonf | 74.6                | 48.3                | 89.1                |
| Weib scale discrete   | asymptotic       | 85.4                | 64.6                | 95.3                |
|                       | asymptotic.bonf  | 85.1                | 63.8                | 95.2                |
|                       | permutation.bonf | 81.6                | 58.4                | 94.2                |
| Weib shape continuous | asymptotic       | 59.8                | 35.5                | 77.1                |
|                       | asymptotic.bonf  | 59.5                | 35.0                | 76.7                |
|                       | permutation.bonf | 54.6                | 28.0                | 74.5                |
| Weib shape discrete   | asymptotic       | 69.7                | 48.0                | 86.4                |
|                       | asymptotic.bonf  | 69.1                | 47.1                | 86.1                |
|                       | permutation.bonf | 65.5                | 38.2                | 83.2                |

Table S71: Rejection rates in percent for the Dunnett-type contrast matrix with  $\delta = 1.5$  and unbalanced medium sample sizes under unequal, low censoring.

| Distribution          | Method           | $\mathcal{H}_{0,7}$ | $\mathcal{H}_{0,8}$ | $\mathcal{H}_{0,9}$ |
|-----------------------|------------------|---------------------|---------------------|---------------------|
| exp early continuous  | asymptotic       | 3.5                 | 2.4                 | 5.2                 |
|                       | asymptotic.bonf  | 3.1                 | 2.3                 | 5.1                 |
|                       | permutation.bonf | 1.4                 | 0.5                 | 3.9                 |
| exp early discrete    | asymptotic       | 4.1                 | 2.7                 | 6.9                 |
|                       | asymptotic.bonf  | 3.6                 | 2.6                 | 6.4                 |
|                       | permutation.bonf | 1.6                 | 0.8                 | 4.7                 |
| exp late continuous   | asymptotic       | 4.2                 | 2.4                 | 6.6                 |
|                       | asymptotic.bonf  | 4.2                 | 2.4                 | 6.2                 |
|                       | permutation.bonf | 2.1                 | 0.8                 | 4.2                 |
| exp late discrete     | asymptotic       | 5.4                 | 2.5                 | 7.9                 |
|                       | asymptotic.bonf  | 4.9                 | 2.5                 | 7.4                 |
|                       | permutation.bonf | 2.5                 | 1.1                 | 5.1                 |
| exp prop continuous   | asymptotic       | 4.2                 | 2.3                 | 4.9                 |
|                       | asymptotic.bonf  | 4.0                 | 2.3                 | 4.3                 |
|                       | permutation.bonf | 2.3                 | 0.9                 | 3.1                 |
| exp prop discrete     | asymptotic       | 5.4                 | 2.8                 | 6.0                 |
|                       | asymptotic.bonf  | 4.7                 | 2.7                 | 5.5                 |
|                       | permutation.bonf | 2.3                 | 0.8                 | 3.5                 |
| logn continuous       | asymptotic       | 11.3                | 6.9                 | 20.9                |
|                       | asymptotic.bonf  | 10.9                | 6.4                 | 20.5                |
|                       | permutation.bonf | 3.4                 | 0.9                 | 10.4                |
| logn discrete         | asymptotic       | 13.4                | 8.2                 | 23.9                |
|                       | asymptotic.bonf  | 13.1                | 7.8                 | 23.8                |
|                       | permutation.bonf | 4.2                 | 0.7                 | 12.7                |
| pwExp continuous      | asymptotic       | 3.3                 | 2.1                 | 5.2                 |
|                       | asymptotic.bonf  | 3.0                 | 1.9                 | 4.9                 |
|                       | permutation.bonf | 1.4                 | 0.7                 | 3.0                 |
| pwExp discrete        | asymptotic       | 3.9                 | 2.3                 | 5.8                 |
|                       | asymptotic.bonf  | 3.8                 | 2.1                 | 5.4                 |
|                       | permutation.bonf | 2.2                 | 0.6                 | 3.2                 |
| Weib late continuous  | asymptotic       | 13.6                | 6.7                 | 25.9                |
|                       | asymptotic.bonf  | 13.3                | 6.2                 | 25.1                |
|                       | permutation.bonf | 5.5                 | 0.7                 | 14.7                |
| Weib late discrete    | asymptotic       | 16.7                | 8.5                 | 30.1                |
|                       | asymptotic.bonf  | 16.1                | 8.3                 | 29.5                |
|                       | permutation.bonf | 6.3                 | 0.8                 | 17.3                |
| Weib prop continuous  | asymptotic       | 12.3                | 6.0                 | 21.7                |
|                       | asymptotic.bonf  | 11.8                | 5.7                 | 21.4                |
|                       | permutation.bonf | 4.4                 | 0.3                 | 11.1                |
| Weib prop discrete    | asymptotic       | 15.0                | 7.0                 | 26.7                |
|                       | asymptotic.bonf  | 14.4                | 7.0                 | 25.9                |
|                       | permutation.bonf | 4.6                 | 0.4                 | 12.9                |
| Weib scale continuous | asymptotic       | 7.6                 | 3.2                 | 12.0                |
|                       | asymptotic.bonf  | 7.5                 | 2.8                 | 11.8                |
|                       | permutation.bonf | 1.9                 | 0.0                 | 5.4                 |
| Weib scale discrete   | asymptotic       | 9.3                 | 4.1                 | 14.2                |
|                       | asymptotic.bonf  | 9.0                 | 3.6                 | 13.9                |
|                       | permutation.bonf | 1.8                 | 0.1                 | 6.4                 |
| Weib shape continuous | asymptotic       | 3.7                 | 1.1                 | 5.4                 |
|                       | asymptotic.bonf  | 3.6                 | 1.1                 | 5.2                 |
|                       | permutation.bonf | 0.7                 | 0.0                 | 2.6                 |
| Weib shape discrete   | asymptotic       | 4.7                 | 1.8                 | 7.9                 |
|                       | asymptotic.bonf  | 4.5                 | 1.6                 | 7.7                 |
|                       | permutation.bonf | 0.6                 | 0.0                 | 3.0                 |

Table S72: Rejection rates in percent for the Dunnett-type contrast matrix with  $\delta = 1.5$  and unbalanced small sample sizes under unequal, low censoring.

| Distribution          | Method           | $\mathcal{H}_{0,7}$ | $\mathcal{H}_{0,8}$ | $\mathcal{H}_{0,9}$ |
|-----------------------|------------------|---------------------|---------------------|---------------------|
| exp early continuous  | asymptotic       | 1.1                 | 3.3                 | 2.2                 |
|                       | asymptotic.bonf  | 1.1                 | 3.3                 | 2.2                 |
|                       | permutation.bonf | 0.1                 | 0.0                 | 0.1                 |
| exp early discrete    | asymptotic       | 1.2                 | 3.5                 | 2.2                 |
|                       | asymptotic.bonf  | 1.0                 | 3.3                 | 2.2                 |
|                       | permutation.bonf | 0.1                 | 0.0                 | 0.1                 |
| exp late continuous   | asymptotic       | 1.3                 | 2.3                 | 2.7                 |
|                       | asymptotic.bonf  | 1.2                 | 2.3                 | 2.7                 |
|                       | permutation.bonf | 0.1                 | 0.0                 | 0.2                 |
| exp late discrete     | asymptotic       | 1.3                 | 2.5                 | 3.0                 |
|                       | asymptotic.bonf  | 1.2                 | 2.3                 | 2.7                 |
|                       | permutation.bonf | 0.0                 | 0.0                 | 0.1                 |
| exp prop continuous   | asymptotic       | 1.8                 | 2.3                 | 2.5                 |
|                       | asymptotic.bonf  | 1.6                 | 2.3                 | 2.4                 |
|                       | permutation.bonf | 0.1                 | 0.3                 | 0.4                 |
| exp prop discrete     | asymptotic       | 1.8                 | 2.3                 | 2.4                 |
|                       | asymptotic.bonf  | 1.8                 | 2.2                 | 2.3                 |
|                       | permutation.bonf | 0.0                 | 0.3                 | 0.4                 |
| logn continuous       | asymptotic       | 2.2                 | 3.5                 | 2.9                 |
|                       | asymptotic.bonf  | 2.2                 | 3.4                 | 2.8                 |
|                       | permutation.bonf | 0.2                 | 0.1                 | 0.1                 |
| logn discrete         | asymptotic       | 2.2                 | 3.7                 | 3.0                 |
|                       | asymptotic.bonf  | 2.2                 | 3.7                 | 3.0                 |
|                       | permutation.bonf | 0.2                 | 0.1                 | 0.1                 |
| pwExp continuous      | asymptotic       | 1.6                 | 2.3                 | 1.9                 |
|                       | asymptotic.bonf  | 1.5                 | 2.3                 | 1.9                 |
|                       | permutation.bonf | 0.0                 | 0.0                 | 0.2                 |
| pwExp discrete        | asymptotic       | 1.8                 | 2.5                 | 2.0                 |
|                       | asymptotic.bonf  | 1.5                 | 2.5                 | 1.8                 |
|                       | permutation.bonf | 0.0                 | 0.0                 | 0.2                 |
| Weib late continuous  | asymptotic       | 2.0                 | 2.2                 | 3.9                 |
|                       | asymptotic.bonf  | 2.0                 | 2.1                 | 3.7                 |
|                       | permutation.bonf | 0.0                 | 0.0                 | 0.0                 |
| Weib late discrete    | asymptotic       | 2.4                 | 2.4                 | 4.0                 |
|                       | asymptotic.bonf  | 2.4                 | 2.4                 | 3.9                 |
|                       | permutation.bonf | 0.0                 | 0.0                 | 0.0                 |
| Weib prop continuous  | asymptotic       | 2.0                 | 2.4                 | 2.9                 |
|                       | asymptotic.bonf  | 1.9                 | 2.4                 | 2.8                 |
|                       | permutation.bonf | 0.0                 | 0.0                 | 0.0                 |
| Weib prop discrete    | asymptotic       | 1.7                 | 2.9                 | 3.6                 |
|                       | asymptotic.bonf  | 1.7                 | 2.9                 | 3.4                 |
|                       | permutation.bonf | 0.0                 | 0.0                 | 0.0                 |
| Weib scale continuous | asymptotic       | 2.9                 | 4.0                 | 2.8                 |
|                       | asymptotic.bonf  | 2.9                 | 3.9                 | 2.8                 |
|                       | permutation.bonf | 0.2                 | 0.1                 | 0.1                 |
| Weib scale discrete   | asymptotic       | 3.2                 | 4.1                 | 2.7                 |
|                       | asymptotic.bonf  | 3.0                 | 4.1                 | 2.6                 |
|                       | permutation.bonf | 0.2                 | 0.0                 | 0.1                 |
| Weib shape continuous | asymptotic       | 6.2                 | 9.1                 | 3.5                 |
|                       | asymptotic.bonf  | 6.2                 | 9.1                 | 3.5                 |
|                       | permutation.bonf | 0.7                 | 0.8                 | 0.8                 |
| Weib shape discrete   | asymptotic       | 6.1                 | 9.2                 | 3.5                 |
|                       | asymptotic.bonf  | 6.1                 | 9.2                 | 3.5                 |
|                       | permutation.bonf | 0.8                 | 0.5                 | 0.7                 |

Table S73: Rejection rates in percent for the Tukey-type contrast matrix with  $\delta = 1.5$  and balanced large sample sizes under equal censoring.

| Distribution          | Method           | $\mathcal{H}_{0,7}$ | $\mathcal{H}_{0,8}$ | $\mathcal{H}_{0,9}$ | $\mathcal{H}_{0,13}$ | $\mathcal{H}_{0,14}$ | $\mathcal{H}_{0,15}$ | $\mathcal{H}_{0,16}$ | $\mathcal{H}_{0,17}$ | $\mathcal{H}_{0,18}$ |
|-----------------------|------------------|---------------------|---------------------|---------------------|----------------------|----------------------|----------------------|----------------------|----------------------|----------------------|
| exp early continuous  | asymptotic       | 79.3                | 57.0                | 92.4                | 78.5                 | 57.8                 | 92.5                 | 77.7                 | 56.0                 | 95.3                 |
|                       | asymptotic_bonf  | 77.5                | 54.6                | 91.4                | 76.8                 | 54.8                 | 91.8                 | 76.1                 | 54.9                 | 94.4                 |
|                       | permutation_bonf | 75.6                | 53.5                | 90.8                | 75.3                 | 53.2                 | 91.2                 | 74.6                 | 52.6                 | 93.6                 |
| exp early discrete    | asymptotic       | 86.3                | 65.3                | 95.4                | 84.4                 | 64.7                 | 95.3                 | 85.0                 | 64.1                 | 97.2                 |
|                       | asymptotic_bonf  | 84.8                | 62.7                | 95.3                | 83.1                 | 63.1                 | 94.8                 | 83.4                 | 61.2                 | 97.0                 |
|                       | permutation_bonf | 83.2                | 60.5                | 94.0                | 82.3                 | 61.0                 | 94.0                 | 81.5                 | 59.8                 | 96.3                 |
| exp late continuous   | asymptotic       | 84.2                | 61.6                | 95.1                | 81.9                 | 61.6                 | 94.8                 | 82.6                 | 61.0                 | 96.8                 |
|                       | asymptotic_bonf  | 82.9                | 59.0                | 94.8                | 80.1                 | 59.6                 | 94.3                 | 80.3                 | 58.5                 | 96.4                 |
|                       | permutation_bonf | 80.7                | 57.5                | 94.2                | 79.3                 | 58.1                 | 93.4                 | 79.2                 | 57.0                 | 95.8                 |
| exp late discrete     | asymptotic       | 89.2                | 67.6                | 96.9                | 89.5                 | 68.7                 | 97.2                 | 88.8                 | 68.9                 | 98.6                 |
|                       | asymptotic_bonf  | 87.6                | 66.1                | 96.4                | 87.4                 | 66.9                 | 96.7                 | 87.3                 | 67.2                 | 98.1                 |
|                       | permutation_bonf | 87.2                | 64.5                | 96.6                | 86.5                 | 65.8                 | 96.8                 | 85.7                 | 65.2                 | 98.0                 |
| exp prop continuous   | asymptotic       | 80.8                | 62.1                | 94.6                | 81.7                 | 62.1                 | 95.0                 | 80.3                 | 63.0                 | 95.6                 |
|                       | asymptotic_bonf  | 78.3                | 59.2                | 94.1                | 79.7                 | 60.6                 | 94.6                 | 78.6                 | 60.2                 | 95.0                 |
|                       | permutation_bonf | 77.9                | 58.4                | 93.2                | 78.0                 | 58.4                 | 93.8                 | 77.6                 | 59.2                 | 94.5                 |
| exp prop discrete     | asymptotic       | 86.9                | 70.2                | 96.7                | 88.2                 | 69.0                 | 97.4                 | 86.3                 | 68.5                 | 98.2                 |
|                       | asymptotic_bonf  | 86.0                | 68.3                | 96.2                | 86.8                 | 66.8                 | 96.8                 | 84.5                 | 67.0                 | 97.9                 |
|                       | permutation_bonf | 85.0                | 67.4                | 96.4                | 85.3                 | 66.1                 | 96.4                 | 83.9                 | 66.9                 | 96.8                 |
| logn continuous       | asymptotic       | 99.9                | 98.6                | 99.9                | 99.7                 | 98.6                 | 100.0                | 99.8                 | 98.1                 | 100.0                |
|                       | asymptotic_bonf  | 99.9                | 98.3                | 99.9                | 99.6                 | 97.5                 | 100.0                | 99.8                 | 97.9                 | 100.0                |
|                       | permutation_bonf | 100.0               | 97.0                | 99.9                | 99.6                 | 97.3                 | 100.0                | 99.8                 | 97.4                 | 100.0                |
| logn discrete         | asymptotic       | 100.0               | 99.2                | 100.0               | 99.9                 | 99.4                 | 100.0                | 99.9                 | 99.4                 | 100.0                |
|                       | asymptotic_bonf  | 100.0               | 99.2                | 100.0               | 99.9                 | 99.4                 | 100.0                | 99.9                 | 99.4                 | 100.0                |
|                       | permutation_bonf | 100.0               | 99.2                | 100.0               | 99.9                 | 99.0                 | 100.0                | 99.9                 | 99.4                 | 100.0                |
| pwExp continuous      | asymptotic       | 78.8                | 55.3                | 92.3                | 76.9                 | 56.3                 | 91.9                 | 76.7                 | 55.1                 | 94.6                 |
|                       | asymptotic_bonf  | 76.5                | 52.7                | 91.6                | 75.8                 | 54.0                 | 90.8                 | 75.1                 | 53.2                 | 93.6                 |
|                       | permutation_bonf | 74.8                | 51.5                | 90.9                | 73.9                 | 53.9                 | 89.8                 | 74.0                 | 52.7                 | 93.4                 |
| pwExp discrete        | asymptotic       | 85.5                | 62.0                | 95.9                | 84.4                 | 64.0                 | 95.4                 | 84.1                 | 64.4                 | 97.3                 |
|                       | asymptotic_bonf  | 83.3                | 60.0                | 94.8                | 83.3                 | 61.9                 | 94.9                 | 82.2                 | 62.7                 | 96.6                 |
|                       | permutation_bonf | 82.6                | 58.8                | 94.3                | 81.9                 | 60.4                 | 94.7                 | 81.1                 | 61.8                 | 96.5                 |
| Weib late continuous  | asymptotic       | 99.9                | 98.3                | 100.0               | 99.7                 | 98.4                 | 100.0                | 99.8                 | 97.6                 | 100.0                |
|                       | asymptotic_bonf  | 99.9                | 98.2                | 100.0               | 99.7                 | 98.2                 | 100.0                | 99.8                 | 97.2                 | 100.0                |
|                       | permutation_bonf | 99.8                | 97.4                | 100.0               | 99.4                 | 98.2                 | 100.0                | 99.8                 | 96.6                 | 100.0                |
| Weib late discrete    | asymptotic       | 100.0               | 99.3                | 100.0               | 100.0                | 99.3                 | 100.0                | 100.0                | 99.1                 | 100.0                |
|                       | asymptotic_bonf  | 99.9                | 99.2                | 100.0               | 99.9                 | 99.3                 | 100.0                | 100.0                | 98.8                 | 100.0                |
|                       | permutation_bonf | 99.9                | 99.3                | 100.0               | 100.0                | 99.3                 | 100.0                | 100.0                | 98.9                 | 100.0                |
| Weib prop continuous  | asymptotic       | 99.7                | 98.2                | 100.0               | 99.5                 | 97.9                 | 100.0                | 99.8                 | 97.0                 | 100.0                |
|                       | asymptotic_bonf  | 99.7                | 98.0                | 100.0               | 99.4                 | 97.4                 | 100.0                | 99.8                 | 96.7                 | 100.0                |
|                       | permutation_bonf | 99.7                | 97.2                | 100.0               | 99.4                 | 97.6                 | 100.0                | 99.8                 | 96.3                 | 100.0                |
| Weib prop discrete    | asymptotic       | 100.0               | 99.0                | 100.0               | 99.9                 | 99.2                 | 100.0                | 99.9                 | 98.8                 | 100.0                |
|                       | asymptotic_bonf  | 100.0               | 99.0                | 100.0               | 99.9                 | 99.1                 | 100.0                | 99.9                 | 98.6                 | 100.0                |
|                       | permutation_bonf | 100.0               | 98.9                | 100.0               | 99.9                 | 99.2                 | 100.0                | 99.9                 | 98.3                 | 100.0                |
| Weib scale continuous | asymptotic       | 99.2                | 96.4                | 100.0               | 98.9                 | 95.4                 | 100.0                | 99.4                 | 95.3                 | 100.0                |
|                       | asymptotic_bonf  | 99.0                | 95.7                | 100.0               | 98.8                 | 95.2                 | 99.9                 | 99.3                 | 94.6                 | 100.0                |
|                       | permutation_bonf | 99.0                | 95.4                | 100.0               | 98.9                 | 94.8                 | 100.0                | 98.9                 | 94.2                 | 100.0                |
| Weib scale discrete   | asymptotic       | 99.9                | 98.5                | 100.0               | 99.6                 | 98.1                 | 100.0                | 99.9                 | 97.3                 | 100.0                |
|                       | asymptotic_bonf  | 99.9                | 98.5                | 100.0               | 99.4                 | 98.0                 | 100.0                | 99.9                 | 97.2                 | 100.0                |
|                       | permutation_bonf | 99.7                | 98.3                | 100.0               | 99.3                 | 97.5                 | 100.0                | 99.8                 | 96.9                 | 100.0                |
| Weib shape continuous | asymptotic       | 98.4                | 90.2                | 99.7                | 97.7                 | 90.6                 | 99.5                 | 98.0                 | 90.0                 | 99.7                 |
|                       | asymptotic_bonf  | 98.2                | 89.5                | 99.7                | 97.2                 | 89.3                 | 99.4                 | 97.8                 | 89.2                 | 99.7                 |
|                       | permutation_bonf | 98.0                | 88.5                | 99.5                | 97.1                 | 88.9                 | 99.5                 | 97.2                 | 88.1                 | 99.6                 |
| Weib shape discrete   | asymptotic       | 99.3                | 95.5                | 100.0               | 99.3                 | 95.9                 | 99.8                 | 99.4                 | 95.0                 | 100.0                |
|                       | asymptotic_bonf  | 99.2                | 94.8                | 100.0               | 99.1                 | 95.3                 | 99.8                 | 99.2                 | 94.7                 | 100.0                |
|                       | permutation_bonf | 99.3                | 94.3                | 99.9                | 98.8                 | 94.5                 | 99.7                 | 99.0                 | 93.6                 | 99.9                 |



Table S74: Rejection rates in percent for the Tukey-type contrast matrix with  $\delta = 1.5$  and balanced medium sample sizes under equal censoring.

| Distribution          | Method           | $\mathcal{H}_{0,7}$ | $\mathcal{H}_{0,8}$ | $\mathcal{H}_{0,9}$ | $\mathcal{H}_{0,13}$ | $\mathcal{H}_{0,14}$ | $\mathcal{H}_{0,15}$ | $\mathcal{H}_{0,16}$ | $\mathcal{H}_{0,17}$ | $\mathcal{H}_{0,18}$ |
|-----------------------|------------------|---------------------|---------------------|---------------------|----------------------|----------------------|----------------------|----------------------|----------------------|----------------------|
| exp early continuous  | asymptotic       | 11.1                | 6.9                 | 16.2                | 11.7                 | 6.4                  | 18.6                 | 11.2                 | 4.4                  | 18.4                 |
|                       | asymptotic_bonf  | 10.1                | 5.8                 | 14.5                | 10.6                 | 6.0                  | 17.1                 | 10.2                 | 3.6                  | 16.5                 |
|                       | permutation_bonf | 10.0                | 6.1                 | 15.1                | 10.3                 | 5.5                  | 16.7                 | 9.6                  | 3.9                  | 16.6                 |
| exp early discrete    | asymptotic       | 13.3                | 8.1                 | 19.5                | 13.3                 | 7.9                  | 22.1                 | 14.1                 | 5.7                  | 22.9                 |
|                       | asymptotic_bonf  | 12.2                | 7.1                 | 17.6                | 12.4                 | 7.2                  | 20.1                 | 12.9                 | 5.0                  | 21.0                 |
|                       | permutation_bonf | 12.8                | 6.9                 | 17.1                | 11.8                 | 7.1                  | 19.1                 | 11.8                 | 5.1                  | 19.3                 |
| exp late continuous   | asymptotic       | 12.0                | 7.3                 | 17.8                | 12.8                 | 6.9                  | 21.7                 | 12.3                 | 5.4                  | 22.2                 |
|                       | asymptotic_bonf  | 10.5                | 6.0                 | 16.8                | 11.7                 | 5.9                  | 20.6                 | 11.5                 | 4.7                  | 20.2                 |
|                       | permutation_bonf | 10.2                | 6.1                 | 16.6                | 11.2                 | 6.4                  | 19.4                 | 10.4                 | 4.9                  | 20.6                 |
| exp late discrete     | asymptotic       | 14.4                | 9.1                 | 21.9                | 14.2                 | 8.2                  | 25.5                 | 14.6                 | 6.3                  | 26.4                 |
|                       | asymptotic_bonf  | 13.1                | 7.7                 | 19.7                | 13.4                 | 7.8                  | 23.5                 | 13.5                 | 5.8                  | 24.2                 |
|                       | permutation_bonf | 13.2                | 8.1                 | 19.2                | 13.1                 | 8.1                  | 22.6                 | 13.6                 | 6.0                  | 23.2                 |
| exp prop continuous   | asymptotic       | 13.1                | 7.9                 | 15.8                | 12.1                 | 6.6                  | 16.6                 | 11.4                 | 6.4                  | 18.0                 |
|                       | asymptotic_bonf  | 11.8                | 6.5                 | 14.1                | 11.1                 | 6.3                  | 15.5                 | 10.2                 | 5.9                  | 17.0                 |
|                       | permutation_bonf | 11.6                | 7.6                 | 14.8                | 10.2                 | 5.8                  | 14.9                 | 10.1                 | 6.0                  | 15.0                 |
| exp prop discrete     | asymptotic       | 15.2                | 9.6                 | 18.6                | 13.7                 | 7.8                  | 19.6                 | 13.6                 | 8.0                  | 21.1                 |
|                       | asymptotic_bonf  | 13.7                | 8.4                 | 17.5                | 12.7                 | 7.0                  | 18.4                 | 12.9                 | 6.9                  | 19.2                 |
|                       | permutation_bonf | 12.1                | 9.1                 | 17.9                | 12.3                 | 6.1                  | 16.6                 | 12.1                 | 6.7                  | 17.7                 |
| logn continuous       | asymptotic       | 37.6                | 23.7                | 58.4                | 37.0                 | 25.0                 | 58.0                 | 38.2                 | 24.3                 | 56.9                 |
|                       | asymptotic_bonf  | 35.6                | 21.9                | 55.9                | 35.6                 | 22.9                 | 55.5                 | 36.9                 | 21.9                 | 53.9                 |
|                       | permutation_bonf | 34.2                | 21.5                | 54.7                | 33.9                 | 22.1                 | 52.4                 | 35.5                 | 19.8                 | 51.9                 |
| logn discrete         | asymptotic       | 45.5                | 29.6                | 66.7                | 44.2                 | 30.4                 | 65.0                 | 45.6                 | 29.1                 | 67.5                 |
|                       | asymptotic_bonf  | 43.4                | 26.8                | 64.6                | 42.0                 | 28.7                 | 63.3                 | 44.1                 | 26.8                 | 65.1                 |
|                       | permutation_bonf | 41.7                | 26.8                | 63.7                | 41.3                 | 28.4                 | 62.3                 | 41.9                 | 26.3                 | 62.3                 |
| pwExp continuous      | asymptotic       | 10.9                | 6.7                 | 16.5                | 11.0                 | 5.7                  | 19.2                 | 11.5                 | 4.9                  | 18.8                 |
|                       | asymptotic_bonf  | 10.0                | 5.6                 | 15.2                | 10.1                 | 5.1                  | 17.0                 | 9.8                  | 4.3                  | 16.5                 |
|                       | permutation_bonf | 9.5                 | 5.5                 | 14.3                | 9.6                  | 5.3                  | 16.0                 | 9.7                  | 4.7                  | 15.5                 |
| pwExp discrete        | asymptotic       | 13.2                | 8.2                 | 20.2                | 13.2                 | 6.7                  | 22.3                 | 12.7                 | 6.1                  | 22.4                 |
|                       | asymptotic_bonf  | 12.1                | 6.7                 | 18.3                | 11.8                 | 6.2                  | 21.1                 | 11.8                 | 5.2                  | 20.6                 |
|                       | permutation_bonf | 11.7                | 7.6                 | 18.1                | 11.7                 | 6.1                  | 20.0                 | 11.6                 | 5.6                  | 18.8                 |
| Weib late continuous  | asymptotic       | 37.1                | 24.4                | 57.4                | 36.3                 | 23.2                 | 60.2                 | 41.7                 | 23.6                 | 56.7                 |
|                       | asymptotic_bonf  | 34.9                | 22.8                | 55.4                | 34.8                 | 22.0                 | 58.5                 | 39.6                 | 22.1                 | 55.3                 |
|                       | permutation_bonf | 34.7                | 22.1                | 53.3                | 35.0                 | 20.4                 | 56.9                 | 36.9                 | 21.1                 | 52.6                 |
| Weib late discrete    | asymptotic       | 44.0                | 28.5                | 64.3                | 44.6                 | 27.4                 | 65.8                 | 47.6                 | 29.6                 | 63.2                 |
|                       | asymptotic_bonf  | 41.8                | 26.9                | 61.3                | 42.0                 | 25.6                 | 63.5                 | 46.1                 | 26.3                 | 60.8                 |
|                       | permutation_bonf | 40.5                | 25.1                | 59.7                | 42.2                 | 24.4                 | 62.0                 | 44.4                 | 26.5                 | 58.5                 |
| Weib prop continuous  | asymptotic       | 34.4                | 23.4                | 55.1                | 35.4                 | 21.1                 | 57.2                 | 38.9                 | 22.5                 | 54.3                 |
|                       | asymptotic_bonf  | 33.0                | 21.2                | 52.9                | 33.5                 | 20.1                 | 54.8                 | 36.9                 | 20.1                 | 52.0                 |
|                       | permutation_bonf | 31.3                | 20.7                | 51.8                | 33.7                 | 20.0                 | 53.9                 | 35.0                 | 20.5                 | 50.6                 |
| Weib prop discrete    | asymptotic       | 43.9                | 28.7                | 63.6                | 42.9                 | 26.8                 | 65.1                 | 47.6                 | 28.3                 | 61.7                 |
|                       | asymptotic_bonf  | 41.5                | 26.8                | 61.8                | 41.0                 | 24.3                 | 63.7                 | 45.6                 | 26.2                 | 60.0                 |
|                       | permutation_bonf | 39.7                | 25.5                | 59.5                | 39.2                 | 24.5                 | 61.3                 | 44.5                 | 26.2                 | 57.9                 |
| Weib scale continuous | asymptotic       | 28.5                | 18.7                | 46.1                | 29.7                 | 16.4                 | 47.1                 | 32.0                 | 18.1                 | 44.8                 |
|                       | asymptotic_bonf  | 26.4                | 16.9                | 44.5                | 27.9                 | 15.4                 | 45.0                 | 29.1                 | 16.5                 | 42.6                 |
|                       | permutation_bonf | 25.7                | 16.9                | 43.1                | 25.7                 | 15.0                 | 43.4                 | 27.8                 | 16.3                 | 40.1                 |
| Weib scale discrete   | asymptotic       | 36.2                | 23.9                | 54.1                | 36.3                 | 21.7                 | 55.7                 | 40.1                 | 22.8                 | 52.6                 |
|                       | asymptotic_bonf  | 33.8                | 22.1                | 52.3                | 33.4                 | 19.9                 | 53.8                 | 37.9                 | 21.2                 | 50.1                 |
|                       | permutation_bonf | 31.9                | 21.9                | 50.2                | 32.6                 | 19.5                 | 52.2                 | 36.4                 | 21.2                 | 48.1                 |
| Weib shape continuous | asymptotic       | 19.5                | 12.1                | 33.5                | 20.7                 | 12.9                 | 36.2                 | 22.8                 | 12.3                 | 33.0                 |
|                       | asymptotic_bonf  | 17.5                | 11.7                | 31.9                | 18.9                 | 11.2                 | 34.4                 | 20.5                 | 10.9                 | 30.8                 |
|                       | permutation_bonf | 17.7                | 11.8                | 30.4                | 18.2                 | 10.8                 | 32.7                 | 19.8                 | 10.5                 | 29.2                 |
| Weib shape discrete   | asymptotic       | 26.7                | 16.3                | 41.3                | 28.6                 | 16.6                 | 44.5                 | 30.3                 | 16.5                 | 42.2                 |
|                       | asymptotic_bonf  | 25.0                | 14.7                | 39.6                | 25.7                 | 15.2                 | 42.1                 | 28.3                 | 15.1                 | 39.5                 |
|                       | permutation_bonf | 23.1                | 15.5                | 37.7                | 24.0                 | 14.8                 | 41.5                 | 26.5                 | 15.1                 | 38.0                 |

Table S75: Rejection rates in percent for the Tukey-type contrast matrix with  $\delta = 1.5$  and balanced small sample sizes under equal censoring.

| Distribution          | Method           | $\mathcal{H}_{0,7}$ | $\mathcal{H}_{0,8}$ | $\mathcal{H}_{0,9}$ | $\mathcal{H}_{0,13}$ | $\mathcal{H}_{0,14}$ | $\mathcal{H}_{0,15}$ | $\mathcal{H}_{0,16}$ | $\mathcal{H}_{0,17}$ | $\mathcal{H}_{0,18}$ |
|-----------------------|------------------|---------------------|---------------------|---------------------|----------------------|----------------------|----------------------|----------------------|----------------------|----------------------|
| exp early continuous  | asymptotic       | 2.2                 | 0.9                 | 2.1                 | 1.5                  | 1.2                  | 2.2                  | 1.7                  | 0.7                  | 2.4                  |
|                       | asymptotic_bonf  | 2.0                 | 0.5                 | 1.9                 | 1.2                  | 1.0                  | 1.7                  | 1.4                  | 0.6                  | 2.3                  |
|                       | permutation_bonf | 1.6                 | 0.6                 | 1.0                 | 0.8                  | 0.6                  | 1.4                  | 1.1                  | 0.6                  | 2.0                  |
| exp early discrete    | asymptotic       | 2.2                 | 1.5                 | 1.7                 | 1.9                  | 0.9                  | 2.3                  | 1.7                  | 0.9                  | 1.9                  |
|                       | asymptotic_bonf  | 1.9                 | 1.3                 | 1.4                 | 1.6                  | 0.9                  | 2.0                  | 1.5                  | 0.7                  | 1.5                  |
|                       | permutation_bonf | 1.5                 | 1.1                 | 1.1                 | 1.5                  | 0.7                  | 1.6                  | 1.1                  | 0.5                  | 1.3                  |
| exp late continuous   | asymptotic       | 2.1                 | 1.0                 | 2.3                 | 1.9                  | 1.6                  | 2.6                  | 2.5                  | 1.2                  | 3.1                  |
|                       | asymptotic_bonf  | 2.0                 | 1.0                 | 1.9                 | 1.7                  | 1.5                  | 2.3                  | 2.2                  | 1.2                  | 2.7                  |
|                       | permutation_bonf | 1.9                 | 0.8                 | 1.6                 | 1.2                  | 0.8                  | 2.0                  | 1.6                  | 1.0                  | 2.2                  |
| exp late discrete     | asymptotic       | 2.4                 | 0.9                 | 2.8                 | 1.8                  | 1.7                  | 3.0                  | 2.8                  | 1.3                  | 2.9                  |
|                       | asymptotic_bonf  | 2.3                 | 0.8                 | 2.3                 | 1.7                  | 1.5                  | 2.7                  | 2.2                  | 1.2                  | 2.5                  |
|                       | permutation_bonf | 2.0                 | 0.9                 | 1.6                 | 1.4                  | 1.4                  | 2.1                  | 2.4                  | 0.7                  | 2.4                  |
| exp prop continuous   | asymptotic       | 1.1                 | 0.9                 | 2.0                 | 1.8                  | 1.0                  | 2.4                  | 1.2                  | 0.9                  | 2.4                  |
|                       | asymptotic_bonf  | 1.1                 | 0.7                 | 1.9                 | 1.7                  | 0.9                  | 1.9                  | 0.7                  | 0.9                  | 2.2                  |
|                       | permutation_bonf | 0.8                 | 0.6                 | 1.8                 | 1.6                  | 0.9                  | 1.6                  | 0.6                  | 0.9                  | 1.5                  |
| exp prop discrete     | asymptotic       | 1.6                 | 1.1                 | 3.4                 | 1.9                  | 0.5                  | 3.2                  | 1.7                  | 1.0                  | 3.0                  |
|                       | asymptotic_bonf  | 1.6                 | 0.9                 | 3.0                 | 1.6                  | 0.3                  | 2.7                  | 1.5                  | 0.9                  | 2.7                  |
|                       | permutation_bonf | 1.2                 | 0.9                 | 2.2                 | 1.2                  | 0.5                  | 2.3                  | 1.2                  | 0.7                  | 2.4                  |
| logn continuous       | asymptotic       | 4.9                 | 2.6                 | 7.6                 | 4.5                  | 2.2                  | 5.7                  | 4.4                  | 2.7                  | 7.6                  |
|                       | asymptotic_bonf  | 4.3                 | 2.3                 | 7.0                 | 3.6                  | 1.6                  | 5.1                  | 3.9                  | 2.6                  | 6.9                  |
|                       | permutation_bonf | 3.6                 | 2.0                 | 5.6                 | 3.4                  | 1.6                  | 4.6                  | 3.8                  | 2.3                  | 5.8                  |
| logn discrete         | asymptotic       | 5.7                 | 3.4                 | 9.4                 | 5.6                  | 2.7                  | 7.1                  | 5.4                  | 3.2                  | 9.1                  |
|                       | asymptotic_bonf  | 4.7                 | 2.9                 | 8.3                 | 5.1                  | 2.3                  | 6.2                  | 4.8                  | 2.5                  | 8.1                  |
|                       | permutation_bonf | 4.3                 | 2.3                 | 7.3                 | 4.2                  | 1.9                  | 5.1                  | 4.9                  | 2.3                  | 7.0                  |
| pwExp continuous      | asymptotic       | 1.6                 | 1.0                 | 1.4                 | 1.6                  | 1.3                  | 2.0                  | 1.8                  | 0.8                  | 2.1                  |
|                       | asymptotic_bonf  | 1.5                 | 0.8                 | 1.2                 | 1.2                  | 1.1                  | 1.9                  | 1.5                  | 0.7                  | 1.9                  |
|                       | permutation_bonf | 1.2                 | 0.5                 | 1.0                 | 0.9                  | 0.4                  | 1.6                  | 1.4                  | 0.6                  | 1.6                  |
| pwExp discrete        | asymptotic       | 1.8                 | 1.1                 | 2.0                 | 1.7                  | 1.4                  | 2.5                  | 2.1                  | 0.9                  | 2.5                  |
|                       | asymptotic_bonf  | 1.7                 | 0.7                 | 1.4                 | 1.5                  | 1.1                  | 2.0                  | 1.8                  | 0.7                  | 2.2                  |
|                       | permutation_bonf | 1.3                 | 0.5                 | 1.2                 | 1.2                  | 0.6                  | 1.8                  | 1.5                  | 0.4                  | 1.8                  |
| Weib late continuous  | asymptotic       | 4.3                 | 4.3                 | 6.1                 | 4.9                  | 2.9                  | 7.4                  | 4.4                  | 3.5                  | 7.2                  |
|                       | asymptotic_bonf  | 4.1                 | 3.5                 | 5.6                 | 4.4                  | 2.6                  | 6.9                  | 3.9                  | 2.8                  | 6.3                  |
|                       | permutation_bonf | 3.0                 | 3.2                 | 4.6                 | 4.0                  | 2.5                  | 5.2                  | 2.7                  | 2.9                  | 4.6                  |
| Weib late discrete    | asymptotic       | 5.1                 | 4.4                 | 7.4                 | 5.7                  | 3.5                  | 8.1                  | 5.5                  | 3.9                  | 7.9                  |
|                       | asymptotic_bonf  | 4.5                 | 4.1                 | 6.5                 | 5.2                  | 3.0                  | 7.2                  | 5.0                  | 3.4                  | 7.1                  |
|                       | permutation_bonf | 3.9                 | 3.7                 | 5.0                 | 4.2                  | 2.9                  | 6.6                  | 3.6                  | 3.1                  | 5.3                  |
| Weib prop continuous  | asymptotic       | 4.0                 | 3.5                 | 5.2                 | 4.5                  | 2.6                  | 6.6                  | 4.0                  | 3.1                  | 6.1                  |
|                       | asymptotic_bonf  | 3.7                 | 3.2                 | 4.5                 | 4.0                  | 2.4                  | 6.0                  | 3.7                  | 2.7                  | 5.3                  |
|                       | permutation_bonf | 2.5                 | 3.0                 | 4.1                 | 3.6                  | 2.1                  | 5.0                  | 2.4                  | 2.7                  | 4.0                  |
| Weib prop discrete    | asymptotic       | 4.6                 | 3.9                 | 5.8                 | 5.2                  | 3.0                  | 8.1                  | 5.2                  | 3.3                  | 6.8                  |
|                       | asymptotic_bonf  | 3.9                 | 3.4                 | 4.9                 | 4.7                  | 2.6                  | 7.5                  | 4.1                  | 2.9                  | 6.2                  |
|                       | permutation_bonf | 3.6                 | 3.8                 | 4.3                 | 4.4                  | 2.8                  | 6.2                  | 3.4                  | 2.9                  | 5.1                  |
| Weib scale continuous | asymptotic       | 2.4                 | 2.4                 | 3.0                 | 2.6                  | 2.0                  | 5.0                  | 1.8                  | 2.1                  | 4.1                  |
|                       | asymptotic_bonf  | 1.9                 | 2.2                 | 2.9                 | 2.1                  | 1.9                  | 4.5                  | 1.4                  | 1.7                  | 3.2                  |
|                       | permutation_bonf | 1.4                 | 2.5                 | 2.5                 | 1.8                  | 1.6                  | 3.5                  | 1.6                  | 1.4                  | 2.3                  |
| Weib scale discrete   | asymptotic       | 3.1                 | 2.9                 | 3.8                 | 3.9                  | 2.1                  | 5.5                  | 1.9                  | 2.1                  | 5.3                  |
|                       | asymptotic_bonf  | 2.4                 | 2.4                 | 3.3                 | 2.9                  | 2.0                  | 5.3                  | 1.3                  | 1.8                  | 4.4                  |
|                       | permutation_bonf | 1.8                 | 2.1                 | 3.0                 | 2.4                  | 1.5                  | 4.3                  | 1.6                  | 1.7                  | 3.4                  |
| Weib shape continuous | asymptotic       | 1.3                 | 1.3                 | 1.7                 | 1.3                  | 1.0                  | 3.0                  | 1.0                  | 1.0                  | 2.2                  |
|                       | asymptotic_bonf  | 1.0                 | 1.3                 | 1.7                 | 1.0                  | 0.6                  | 2.4                  | 0.8                  | 0.8                  | 1.6                  |
|                       | permutation_bonf | 0.7                 | 1.4                 | 2.0                 | 1.0                  | 1.0                  | 2.2                  | 0.7                  | 1.0                  | 1.5                  |
| Weib shape discrete   | asymptotic       | 1.5                 | 1.7                 | 2.6                 | 1.6                  | 1.0                  | 3.3                  | 1.0                  | 1.0                  | 2.8                  |
|                       | asymptotic_bonf  | 1.1                 | 1.3                 | 2.4                 | 1.5                  | 1.0                  | 2.9                  | 0.8                  | 0.9                  | 2.2                  |
|                       | permutation_bonf | 1.0                 | 1.6                 | 2.0                 | 1.3                  | 1.0                  | 2.8                  | 0.8                  | 0.8                  | 2.0                  |

Table S76: Rejection rates in percent for the Tukey-type contrast matrix with  $\delta = 1.5$  and unbalanced large sample sizes under equal censoring.

| Distribution          | Method           | $\mathcal{H}_{0,7}$ | $\mathcal{H}_{0,8}$ | $\mathcal{H}_{0,9}$ | $\mathcal{H}_{0,13}$ | $\mathcal{H}_{0,14}$ | $\mathcal{H}_{0,15}$ | $\mathcal{H}_{0,16}$ | $\mathcal{H}_{0,17}$ | $\mathcal{H}_{0,18}$ |
|-----------------------|------------------|---------------------|---------------------|---------------------|----------------------|----------------------|----------------------|----------------------|----------------------|----------------------|
| exp early continuous  | asymptotic       | 31.3                | 16.0                | 53.4                | 27.3                 | 12.3                 | 42.7                 | 27.1                 | 13.2                 | 45.8                 |
|                       | asymptotic_bonf  | 27.3                | 13.7                | 50.6                | 23.9                 | 11.2                 | 39.4                 | 23.3                 | 11.7                 | 41.3                 |
|                       | permutation_bonf | 24.4                | 11.3                | 47.7                | 21.7                 | 9.9                  | 36.8                 | 22.4                 | 11.0                 | 38.8                 |
| exp early discrete    | asymptotic       | 36.9                | 19.3                | 59.6                | 30.7                 | 15.7                 | 48.3                 | 32.2                 | 17.1                 | 51.7                 |
|                       | asymptotic_bonf  | 33.0                | 17.0                | 57.0                | 28.4                 | 13.7                 | 45.2                 | 29.1                 | 14.4                 | 47.7                 |
|                       | permutation_bonf | 29.1                | 13.4                | 53.4                | 24.8                 | 12.6                 | 45.3                 | 26.7                 | 13.4                 | 46.1                 |
| exp late continuous   | asymptotic       | 36.4                | 20.4                | 62.6                | 30.4                 | 15.0                 | 50.2                 | 31.8                 | 15.7                 | 53.2                 |
|                       | asymptotic_bonf  | 33.0                | 17.4                | 59.6                | 26.8                 | 13.0                 | 46.5                 | 28.9                 | 13.7                 | 49.4                 |
|                       | permutation_bonf | 29.0                | 14.4                | 57.1                | 25.1                 | 11.7                 | 45.2                 | 26.3                 | 13.1                 | 46.6                 |
| exp late discrete     | asymptotic       | 44.3                | 23.9                | 69.1                | 35.5                 | 19.0                 | 57.5                 | 37.8                 | 18.9                 | 59.1                 |
|                       | asymptotic_bonf  | 39.4                | 21.4                | 65.7                | 31.5                 | 16.4                 | 54.3                 | 34.3                 | 16.4                 | 56.2                 |
|                       | permutation_bonf | 35.3                | 16.6                | 63.2                | 28.9                 | 14.4                 | 52.5                 | 33.0                 | 15.7                 | 54.4                 |
| exp prop continuous   | asymptotic       | 35.9                | 20.0                | 54.2                | 29.8                 | 16.9                 | 42.7                 | 28.0                 | 16.1                 | 46.7                 |
|                       | asymptotic_bonf  | 32.5                | 17.7                | 50.4                | 26.5                 | 14.3                 | 38.8                 | 25.7                 | 14.2                 | 42.9                 |
|                       | permutation_bonf | 30.0                | 14.6                | 47.4                | 25.1                 | 12.7                 | 37.2                 | 23.8                 | 12.6                 | 41.3                 |
| exp prop discrete     | asymptotic       | 41.7                | 24.8                | 62.3                | 34.3                 | 20.3                 | 49.3                 | 35.4                 | 19.6                 | 54.9                 |
|                       | asymptotic_bonf  | 37.8                | 21.9                | 57.8                | 31.1                 | 17.7                 | 46.0                 | 31.0                 | 17.3                 | 51.4                 |
|                       | permutation_bonf | 35.1                | 17.6                | 55.2                | 29.8                 | 15.3                 | 42.8                 | 28.6                 | 14.7                 | 48.5                 |
| logn continuous       | asymptotic       | 84.8                | 63.0                | 94.1                | 74.7                 | 51.8                 | 88.9                 | 75.6                 | 56.4                 | 90.3                 |
|                       | asymptotic_bonf  | 82.1                | 59.7                | 93.1                | 72.5                 | 48.0                 | 86.5                 | 73.4                 | 52.8                 | 88.6                 |
|                       | permutation_bonf | 75.4                | 50.1                | 89.9                | 69.7                 | 43.1                 | 83.8                 | 68.9                 | 48.1                 | 85.9                 |
| logn discrete         | asymptotic       | 91.0                | 71.0                | 97.3                | 81.3                 | 62.2                 | 93.4                 | 84.0                 | 65.5                 | 94.1                 |
|                       | asymptotic_bonf  | 89.0                | 67.4                | 96.5                | 79.4                 | 57.7                 | 92.2                 | 82.4                 | 62.2                 | 93.5                 |
|                       | permutation_bonf | 82.6                | 59.6                | 94.3                | 76.0                 | 52.2                 | 90.4                 | 77.4                 | 56.0                 | 91.3                 |
| pwExp continuous      | asymptotic       | 29.2                | 15.3                | 52.1                | 24.1                 | 12.5                 | 42.5                 | 25.7                 | 13.6                 | 43.1                 |
|                       | asymptotic_bonf  | 26.7                | 13.1                | 47.7                | 21.7                 | 10.5                 | 39.1                 | 22.8                 | 11.5                 | 39.9                 |
|                       | permutation_bonf | 24.2                | 10.4                | 45.0                | 19.7                 | 9.1                  | 37.2                 | 21.1                 | 11.8                 | 37.6                 |
| pwExp discrete        | asymptotic       | 34.8                | 19.2                | 60.8                | 29.3                 | 15.3                 | 49.2                 | 30.8                 | 16.9                 | 50.7                 |
|                       | asymptotic_bonf  | 32.0                | 15.9                | 57.0                | 25.8                 | 13.3                 | 45.7                 | 27.6                 | 14.2                 | 47.3                 |
|                       | permutation_bonf | 28.9                | 12.3                | 51.8                | 25.5                 | 11.9                 | 44.6                 | 25.6                 | 13.6                 | 44.7                 |
| Weib late continuous  | asymptotic       | 84.8                | 62.0                | 96.4                | 78.6                 | 52.7                 | 91.7                 | 78.2                 | 55.2                 | 94.3                 |
|                       | asymptotic_bonf  | 83.2                | 58.2                | 95.6                | 75.2                 | 49.8                 | 90.7                 | 75.4                 | 51.1                 | 93.3                 |
|                       | permutation_bonf | 80.2                | 49.2                | 94.2                | 73.2                 | 44.7                 | 88.3                 | 71.9                 | 46.0                 | 91.2                 |
| Weib late discrete    | asymptotic       | 87.8                | 69.5                | 95.9                | 81.1                 | 59.8                 | 93.3                 | 80.8                 | 60.5                 | 96.0                 |
|                       | asymptotic_bonf  | 86.2                | 66.0                | 95.8                | 79.3                 | 56.1                 | 92.1                 | 78.6                 | 58.8                 | 95.0                 |
|                       | permutation_bonf | 81.6                | 57.1                | 94.8                | 77.2                 | 52.6                 | 91.3                 | 75.8                 | 52.7                 | 93.4                 |
| Weib prop continuous  | asymptotic       | 82.1                | 58.0                | 95.1                | 75.5                 | 50.6                 | 90.1                 | 75.2                 | 52.2                 | 91.9                 |
|                       | asymptotic_bonf  | 80.3                | 55.1                | 94.4                | 72.6                 | 46.3                 | 88.0                 | 73.1                 | 47.7                 | 90.1                 |
|                       | permutation_bonf | 75.4                | 46.1                | 92.6                | 69.7                 | 42.0                 | 86.7                 | 69.3                 | 44.1                 | 87.8                 |
| Weib prop discrete    | asymptotic       | 87.9                | 68.2                | 97.4                | 82.4                 | 59.4                 | 94.7                 | 82.4                 | 60.6                 | 95.9                 |
|                       | asymptotic_bonf  | 85.8                | 65.0                | 96.7                | 80.3                 | 55.5                 | 93.8                 | 80.8                 | 57.4                 | 95.0                 |
|                       | permutation_bonf | 82.8                | 54.9                | 95.9                | 77.6                 | 51.4                 | 92.5                 | 77.9                 | 52.5                 | 93.3                 |
| Weib scale continuous | asymptotic       | 69.7                | 46.9                | 86.6                | 63.0                 | 39.7                 | 80.3                 | 63.4                 | 42.3                 | 82.1                 |
|                       | asymptotic_bonf  | 67.4                | 42.7                | 84.9                | 59.3                 | 35.8                 | 77.8                 | 59.9                 | 38.8                 | 79.8                 |
|                       | permutation_bonf | 61.5                | 35.1                | 81.3                | 55.0                 | 31.5                 | 74.8                 | 56.4                 | 33.5                 | 76.8                 |
| Weib scale discrete   | asymptotic       | 77.2                | 54.7                | 92.3                | 72.0                 | 48.7                 | 88.5                 | 72.5                 | 50.0                 | 88.5                 |
|                       | asymptotic_bonf  | 74.4                | 50.8                | 90.7                | 69.1                 | 44.6                 | 86.4                 | 68.9                 | 46.7                 | 87.6                 |
|                       | permutation_bonf | 69.1                | 42.6                | 86.8                | 65.2                 | 39.7                 | 83.7                 | 64.9                 | 41.1                 | 84.6                 |
| Weib shape continuous | asymptotic       | 52.9                | 29.0                | 71.2                | 45.8                 | 27.3                 | 65.3                 | 47.9                 | 28.5                 | 67.8                 |
|                       | asymptotic_bonf  | 48.2                | 24.3                | 67.8                | 42.6                 | 23.3                 | 61.1                 | 43.6                 | 24.5                 | 63.7                 |
|                       | permutation_bonf | 41.2                | 18.8                | 62.9                | 37.8                 | 20.4                 | 58.3                 | 39.6                 | 20.6                 | 59.6                 |
| Weib shape discrete   | asymptotic       | 64.7                | 40.1                | 81.5                | 56.2                 | 35.0                 | 75.2                 | 57.1                 | 35.9                 | 77.6                 |
|                       | asymptotic_bonf  | 59.9                | 35.0                | 79.1                | 52.1                 | 32.4                 | 71.9                 | 54.6                 | 32.7                 | 74.6                 |
|                       | permutation_bonf | 51.7                | 25.6                | 73.9                | 48.8                 | 27.2                 | 70.3                 | 50.7                 | 28.0                 | 70.4                 |

Table S77: Rejection rates in percent for the Tukey-type contrast matrix with  $\delta = 1.5$  and unbalanced medium sample sizes under equal censoring.

| Distribution          | Method           | $\mathcal{H}_{0,7}$ | $\mathcal{H}_{0,8}$ | $\mathcal{H}_{0,9}$ | $\mathcal{H}_{0,13}$ | $\mathcal{H}_{0,14}$ | $\mathcal{H}_{0,15}$ | $\mathcal{H}_{0,16}$ | $\mathcal{H}_{0,17}$ | $\mathcal{H}_{0,18}$ |
|-----------------------|------------------|---------------------|---------------------|---------------------|----------------------|----------------------|----------------------|----------------------|----------------------|----------------------|
| exp early continuous  | asymptotic       | 1.6                 | 1.5                 | 3.8                 | 1.6                  | 1.1                  | 3.5                  | 2.7                  | 1.1                  | 4.2                  |
|                       | asymptotic_bonf  | 1.5                 | 0.9                 | 3.2                 | 1.2                  | 0.9                  | 3.0                  | 2.5                  | 0.9                  | 3.4                  |
|                       | permutation_bonf | 0.5                 | 0.2                 | 1.6                 | 0.6                  | 0.3                  | 2.3                  | 1.8                  | 0.5                  | 2.5                  |
| exp early discrete    | asymptotic       | 2.4                 | 1.8                 | 4.4                 | 1.9                  | 1.4                  | 3.9                  | 3.5                  | 1.2                  | 4.4                  |
|                       | asymptotic_bonf  | 2.0                 | 1.3                 | 3.9                 | 1.6                  | 1.1                  | 3.6                  | 2.8                  | 0.8                  | 3.9                  |
|                       | permutation_bonf | 0.7                 | 0.2                 | 2.4                 | 0.8                  | 0.6                  | 2.3                  | 1.7                  | 0.5                  | 2.7                  |
| exp late continuous   | asymptotic       | 2.4                 | 1.7                 | 5.2                 | 1.8                  | 1.4                  | 4.1                  | 3.1                  | 1.4                  | 4.8                  |
|                       | asymptotic_bonf  | 2.0                 | 1.5                 | 3.9                 | 1.2                  | 1.2                  | 3.4                  | 2.6                  | 0.8                  | 3.9                  |
|                       | permutation_bonf | 0.8                 | 0.2                 | 1.8                 | 0.8                  | 0.5                  | 2.7                  | 2.0                  | 0.4                  | 3.0                  |
| exp late discrete     | asymptotic       | 2.8                 | 1.8                 | 5.9                 | 2.2                  | 1.6                  | 4.4                  | 3.8                  | 1.2                  | 5.2                  |
|                       | asymptotic_bonf  | 2.2                 | 1.7                 | 5.1                 | 1.8                  | 1.5                  | 4.0                  | 3.3                  | 1.1                  | 4.3                  |
|                       | permutation_bonf | 0.9                 | 0.6                 | 2.8                 | 0.9                  | 0.8                  | 2.9                  | 1.9                  | 0.5                  | 3.3                  |
| exp prop continuous   | asymptotic       | 3.2                 | 1.4                 | 3.2                 | 2.6                  | 1.2                  | 3.5                  | 2.2                  | 1.8                  | 2.9                  |
|                       | asymptotic_bonf  | 2.2                 | 1.0                 | 3.0                 | 2.2                  | 0.8                  | 2.6                  | 1.9                  | 1.2                  | 2.3                  |
|                       | permutation_bonf | 1.2                 | 0.4                 | 1.7                 | 1.5                  | 0.3                  | 1.7                  | 1.0                  | 0.3                  | 1.9                  |
| exp prop discrete     | asymptotic       | 3.4                 | 1.5                 | 4.3                 | 3.0                  | 1.2                  | 4.4                  | 2.7                  | 1.9                  | 4.0                  |
|                       | asymptotic_bonf  | 2.9                 | 1.0                 | 3.4                 | 2.5                  | 0.9                  | 3.3                  | 2.5                  | 1.7                  | 3.4                  |
|                       | permutation_bonf | 1.3                 | 0.3                 | 2.1                 | 1.6                  | 0.6                  | 2.3                  | 1.7                  | 0.4                  | 2.0                  |
| logn continuous       | asymptotic       | 7.1                 | 4.6                 | 13.7                | 7.3                  | 4.5                  | 13.0                 | 6.3                  | 4.5                  | 12.5                 |
|                       | asymptotic_bonf  | 5.9                 | 4.0                 | 12.0                | 5.7                  | 3.7                  | 11.5                 | 5.1                  | 3.3                  | 10.6                 |
|                       | permutation_bonf | 1.2                 | 0.2                 | 5.3                 | 2.5                  | 1.0                  | 7.1                  | 3.3                  | 1.0                  | 6.3                  |
| logn discrete         | asymptotic       | 8.9                 | 5.5                 | 16.7                | 8.6                  | 5.2                  | 16.5                 | 8.0                  | 3.9                  | 15.6                 |
|                       | asymptotic_bonf  | 7.1                 | 4.4                 | 15.0                | 7.4                  | 4.0                  | 13.3                 | 6.5                  | 3.6                  | 13.0                 |
|                       | permutation_bonf | 1.2                 | 0.2                 | 5.5                 | 3.1                  | 1.0                  | 8.5                  | 3.1                  | 1.5                  | 9.0                  |
| pwExp continuous      | asymptotic       | 2.1                 | 1.5                 | 3.5                 | 1.2                  | 1.3                  | 3.4                  | 2.3                  | 1.3                  | 3.5                  |
|                       | asymptotic_bonf  | 1.5                 | 1.4                 | 3.3                 | 0.7                  | 1.2                  | 2.9                  | 1.8                  | 1.0                  | 2.7                  |
|                       | permutation_bonf | 0.3                 | 0.4                 | 1.5                 | 0.4                  | 0.6                  | 2.4                  | 1.2                  | 0.3                  | 1.9                  |
| pwExp discrete        | asymptotic       | 2.7                 | 2.0                 | 4.0                 | 1.8                  | 1.4                  | 4.4                  | 2.5                  | 1.5                  | 4.2                  |
|                       | asymptotic_bonf  | 2.1                 | 1.5                 | 3.6                 | 1.4                  | 1.2                  | 3.1                  | 2.1                  | 1.1                  | 3.5                  |
|                       | permutation_bonf | 0.5                 | 0.4                 | 1.5                 | 0.6                  | 0.7                  | 2.7                  | 1.3                  | 0.2                  | 2.4                  |
| Weib late continuous  | asymptotic       | 8.5                 | 4.0                 | 17.3                | 8.5                  | 4.0                  | 14.1                 | 8.0                  | 4.1                  | 16.0                 |
|                       | asymptotic_bonf  | 6.7                 | 2.8                 | 14.3                | 6.9                  | 2.7                  | 11.8                 | 6.6                  | 3.0                  | 13.9                 |
|                       | permutation_bonf | 2.1                 | 0.2                 | 7.3                 | 4.1                  | 1.0                  | 8.0                  | 2.7                  | 0.5                  | 8.6                  |
| Weib late discrete    | asymptotic       | 10.4                | 4.6                 | 21.4                | 9.7                  | 4.9                  | 17.5                 | 10.2                 | 4.0                  | 19.9                 |
|                       | asymptotic_bonf  | 9.2                 | 3.6                 | 18.7                | 7.5                  | 3.5                  | 15.8                 | 8.6                  | 3.2                  | 17.1                 |
|                       | permutation_bonf | 2.0                 | 0.1                 | 8.4                 | 4.7                  | 1.2                  | 10.8                 | 3.3                  | 0.7                  | 11.1                 |
| Weib prop continuous  | asymptotic       | 7.6                 | 3.4                 | 14.7                | 6.7                  | 3.3                  | 11.8                 | 6.6                  | 3.5                  | 12.8                 |
|                       | asymptotic_bonf  | 5.9                 | 2.6                 | 12.4                | 5.8                  | 2.5                  | 10.1                 | 5.3                  | 2.3                  | 11.4                 |
|                       | permutation_bonf | 1.5                 | 0.1                 | 5.4                 | 3.9                  | 0.9                  | 6.8                  | 2.7                  | 0.4                  | 6.7                  |
| Weib prop discrete    | asymptotic       | 9.4                 | 3.8                 | 17.2                | 8.0                  | 3.8                  | 14.8                 | 8.0                  | 4.5                  | 16.6                 |
|                       | asymptotic_bonf  | 7.9                 | 2.8                 | 14.6                | 6.5                  | 2.7                  | 12.9                 | 6.8                  | 2.9                  | 14.0                 |
|                       | permutation_bonf | 1.7                 | 0.1                 | 5.7                 | 4.3                  | 0.6                  | 8.3                  | 2.6                  | 0.0                  | 7.9                  |
| Weib scale continuous | asymptotic       | 4.6                 | 1.6                 | 9.4                 | 4.8                  | 1.7                  | 8.0                  | 4.4                  | 1.8                  | 8.6                  |
|                       | asymptotic_bonf  | 3.4                 | 1.3                 | 7.9                 | 4.1                  | 1.1                  | 6.8                  | 3.1                  | 1.6                  | 6.9                  |
|                       | permutation_bonf | 0.6                 | 0.0                 | 2.3                 | 2.3                  | 0.6                  | 3.6                  | 1.3                  | 0.1                  | 3.8                  |
| Weib scale discrete   | asymptotic       | 5.8                 | 2.0                 | 10.1                | 5.5                  | 2.3                  | 9.6                  | 5.6                  | 2.5                  | 10.1                 |
|                       | asymptotic_bonf  | 4.3                 | 1.4                 | 9.2                 | 4.8                  | 1.8                  | 8.4                  | 4.3                  | 1.8                  | 8.4                  |
|                       | permutation_bonf | 0.9                 | 0.0                 | 3.4                 | 3.0                  | 0.5                  | 4.7                  | 1.3                  | 0.1                  | 4.6                  |
| Weib shape continuous | asymptotic       | 2.3                 | 1.1                 | 4.3                 | 2.8                  | 1.1                  | 4.0                  | 2.5                  | 1.0                  | 3.9                  |
|                       | asymptotic_bonf  | 1.7                 | 0.7                 | 3.2                 | 2.5                  | 0.5                  | 3.2                  | 1.8                  | 0.7                  | 2.6                  |
|                       | permutation_bonf | 0.2                 | 0.0                 | 1.1                 | 1.1                  | 0.2                  | 1.9                  | 0.8                  | 0.1                  | 1.3                  |
| Weib shape discrete   | asymptotic       | 3.3                 | 1.1                 | 5.2                 | 3.4                  | 1.0                  | 5.4                  | 3.2                  | 1.2                  | 5.7                  |
|                       | asymptotic_bonf  | 2.3                 | 1.0                 | 4.6                 | 2.9                  | 0.9                  | 4.0                  | 2.6                  | 0.9                  | 4.1                  |
|                       | permutation_bonf | 0.1                 | 0.0                 | 1.1                 | 1.0                  | 0.2                  | 2.8                  | 0.5                  | 0.0                  | 2.2                  |

Table S78: Rejection rates in percent for the Tukey-type contrast matrix with  $\delta = 1.5$  and unbalanced small sample sizes under equal censoring.

| Distribution          | Method           | $\mathcal{H}_{0,7}$ | $\mathcal{H}_{0,8}$ | $\mathcal{H}_{0,9}$ | $\mathcal{H}_{0,13}$ | $\mathcal{H}_{0,14}$ | $\mathcal{H}_{0,15}$ | $\mathcal{H}_{0,16}$ | $\mathcal{H}_{0,17}$ | $\mathcal{H}_{0,18}$ |
|-----------------------|------------------|---------------------|---------------------|---------------------|----------------------|----------------------|----------------------|----------------------|----------------------|----------------------|
| exp early continuous  | asymptotic       | 0.8                 | 3.0                 | 1.7                 | 0.8                  | 1.7                  | 1.5                  | 0.6                  | 2.2                  | 1.7                  |
|                       | asymptotic_bonf  | 0.7                 | 3.0                 | 1.6                 | 0.6                  | 1.7                  | 1.3                  | 0.6                  | 2.0                  | 1.5                  |
|                       | permutation_bonf | 0.1                 | 0.1                 | 0.2                 | 0.1                  | 0.1                  | 0.1                  | 0.0                  | 0.4                  | 0.4                  |
| exp early discrete    | asymptotic       | 0.9                 | 2.9                 | 2.0                 | 0.9                  | 1.5                  | 1.7                  | 0.7                  | 2.1                  | 1.7                  |
|                       | asymptotic_bonf  | 0.6                 | 2.7                 | 1.7                 | 0.7                  | 1.5                  | 1.6                  | 0.7                  | 1.7                  | 1.4                  |
|                       | permutation_bonf | 0.1                 | 0.2                 | 0.1                 | 0.1                  | 0.3                  | 0.3                  | 0.0                  | 0.3                  | 0.2                  |
| exp late continuous   | asymptotic       | 1.0                 | 1.9                 | 2.2                 | 0.6                  | 1.0                  | 1.9                  | 1.0                  | 1.7                  | 1.7                  |
|                       | asymptotic_bonf  | 0.7                 | 1.9                 | 1.7                 | 0.5                  | 1.0                  | 1.6                  | 0.6                  | 1.5                  | 1.5                  |
|                       | permutation_bonf | 0.0                 | 0.1                 | 0.0                 | 0.0                  | 0.1                  | 0.0                  | 0.0                  | 0.3                  | 0.2                  |
| exp late discrete     | asymptotic       | 1.1                 | 2.0                 | 2.6                 | 1.0                  | 0.9                  | 2.2                  | 0.9                  | 1.9                  | 1.9                  |
|                       | asymptotic_bonf  | 0.9                 | 2.0                 | 2.0                 | 0.6                  | 0.8                  | 1.5                  | 0.8                  | 1.6                  | 1.6                  |
|                       | permutation_bonf | 0.0                 | 0.1                 | 0.0                 | 0.0                  | 0.2                  | 0.2                  | 0.0                  | 0.2                  | 0.1                  |
| exp prop continuous   | asymptotic       | 1.0                 | 2.0                 | 1.9                 | 1.5                  | 1.6                  | 1.7                  | 1.1                  | 1.4                  | 2.1                  |
|                       | asymptotic_bonf  | 1.0                 | 1.8                 | 1.5                 | 1.1                  | 1.2                  | 1.3                  | 0.9                  | 1.3                  | 1.7                  |
|                       | permutation_bonf | 0.2                 | 0.3                 | 0.3                 | 0.0                  | 0.1                  | 0.2                  | 0.2                  | 0.0                  | 0.3                  |
| exp prop discrete     | asymptotic       | 1.2                 | 2.3                 | 2.1                 | 1.3                  | 1.6                  | 2.2                  | 1.0                  | 1.5                  | 2.0                  |
|                       | asymptotic_bonf  | 1.0                 | 2.2                 | 1.9                 | 1.1                  | 1.2                  | 1.6                  | 0.6                  | 1.4                  | 1.6                  |
|                       | permutation_bonf | 0.1                 | 0.1                 | 0.3                 | 0.0                  | 0.1                  | 0.3                  | 0.2                  | 0.0                  | 0.3                  |
| logn continuous       | asymptotic       | 2.7                 | 4.6                 | 2.3                 | 2.0                  | 1.4                  | 2.4                  | 1.7                  | 2.1                  | 2.2                  |
|                       | asymptotic_bonf  | 2.2                 | 4.5                 | 2.1                 | 1.6                  | 1.0                  | 2.3                  | 1.1                  | 1.7                  | 2.0                  |
|                       | permutation_bonf | 0.3                 | 0.1                 | 0.1                 | 0.2                  | 0.0                  | 0.4                  | 0.1                  | 0.1                  | 0.1                  |
| logn discrete         | asymptotic       | 2.9                 | 5.1                 | 2.9                 | 2.6                  | 1.1                  | 2.5                  | 2.2                  | 1.7                  | 2.7                  |
|                       | asymptotic_bonf  | 2.7                 | 5.0                 | 2.4                 | 2.1                  | 1.0                  | 2.2                  | 1.7                  | 1.3                  | 2.2                  |
|                       | permutation_bonf | 0.1                 | 0.1                 | 0.1                 | 0.3                  | 0.1                  | 0.3                  | 0.1                  | 0.0                  | 0.0                  |
| pwExp continuous      | asymptotic       | 1.1                 | 2.4                 | 1.8                 | 0.7                  | 1.4                  | 1.5                  | 0.7                  | 1.7                  | 1.7                  |
|                       | asymptotic_bonf  | 0.9                 | 2.4                 | 1.6                 | 0.5                  | 1.3                  | 1.1                  | 0.4                  | 1.4                  | 1.4                  |
|                       | permutation_bonf | 0.1                 | 0.1                 | 0.2                 | 0.0                  | 0.1                  | 0.3                  | 0.0                  | 0.3                  | 0.3                  |
| pwExp discrete        | asymptotic       | 1.1                 | 2.5                 | 1.6                 | 0.7                  | 1.2                  | 1.9                  | 0.8                  | 1.7                  | 1.9                  |
|                       | asymptotic_bonf  | 1.0                 | 2.4                 | 1.5                 | 0.6                  | 1.0                  | 1.3                  | 0.3                  | 1.2                  | 1.8                  |
|                       | permutation_bonf | 0.1                 | 0.0                 | 0.2                 | 0.0                  | 0.1                  | 0.4                  | 0.0                  | 0.2                  | 0.2                  |
| Weib late continuous  | asymptotic       | 1.6                 | 2.1                 | 2.6                 | 1.3                  | 0.7                  | 2.1                  | 1.7                  | 1.0                  | 2.0                  |
|                       | asymptotic_bonf  | 1.5                 | 1.9                 | 2.3                 | 1.2                  | 0.6                  | 1.8                  | 1.6                  | 0.8                  | 1.6                  |
|                       | permutation_bonf | 0.1                 | 0.0                 | 0.2                 | 0.2                  | 0.1                  | 0.3                  | 0.1                  | 0.0                  | 0.1                  |
| Weib late discrete    | asymptotic       | 2.4                 | 2.9                 | 2.8                 | 1.9                  | 1.1                  | 2.5                  | 1.7                  | 1.0                  | 2.3                  |
|                       | asymptotic_bonf  | 2.0                 | 2.7                 | 2.2                 | 1.5                  | 1.0                  | 2.2                  | 1.6                  | 0.7                  | 1.9                  |
|                       | permutation_bonf | 0.0                 | 0.0                 | 0.1                 | 0.2                  | 0.2                  | 0.1                  | 0.3                  | 0.0                  | 0.1                  |
| Weib prop continuous  | asymptotic       | 1.9                 | 3.0                 | 2.4                 | 1.1                  | 0.8                  | 1.9                  | 1.6                  | 1.7                  | 1.9                  |
|                       | asymptotic_bonf  | 1.7                 | 2.6                 | 1.9                 | 1.0                  | 0.7                  | 1.7                  | 1.5                  | 1.3                  | 1.8                  |
|                       | permutation_bonf | 0.1                 | 0.1                 | 0.2                 | 0.2                  | 0.1                  | 0.0                  | 0.1                  | 0.0                  | 0.0                  |
| Weib prop discrete    | asymptotic       | 2.2                 | 3.4                 | 2.4                 | 1.6                  | 0.9                  | 2.2                  | 1.6                  | 1.3                  | 1.7                  |
|                       | asymptotic_bonf  | 2.1                 | 3.3                 | 2.1                 | 1.1                  | 0.7                  | 2.0                  | 1.3                  | 1.1                  | 1.5                  |
|                       | permutation_bonf | 0.0                 | 0.1                 | 0.2                 | 0.1                  | 0.0                  | 0.0                  | 0.2                  | 0.0                  | 0.0                  |
| Weib scale continuous | asymptotic       | 2.9                 | 4.3                 | 1.9                 | 2.3                  | 1.1                  | 1.7                  | 2.3                  | 2.2                  | 1.9                  |
|                       | asymptotic_bonf  | 2.9                 | 4.2                 | 1.9                 | 1.9                  | 1.0                  | 1.4                  | 1.8                  | 1.8                  | 1.7                  |
|                       | permutation_bonf | 0.1                 | 0.1                 | 0.3                 | 0.2                  | 0.2                  | 0.0                  | 0.1                  | 0.0                  | 0.0                  |
| Weib scale discrete   | asymptotic       | 3.4                 | 5.5                 | 2.5                 | 1.9                  | 1.8                  | 1.8                  | 2.1                  | 1.9                  | 2.1                  |
|                       | asymptotic_bonf  | 3.2                 | 5.5                 | 2.4                 | 1.5                  | 1.2                  | 1.5                  | 1.9                  | 1.7                  | 1.6                  |
|                       | permutation_bonf | 0.0                 | 0.1                 | 0.3                 | 0.2                  | 0.2                  | 0.0                  | 0.3                  | 0.1                  | 0.0                  |
| Weib shape continuous | asymptotic       | 6.1                 | 9.3                 | 3.0                 | 4.6                  | 3.3                  | 2.7                  | 5.2                  | 5.1                  | 2.9                  |
|                       | asymptotic_bonf  | 5.9                 | 9.0                 | 2.6                 | 4.1                  | 3.0                  | 2.5                  | 4.6                  | 4.6                  | 2.5                  |
|                       | permutation_bonf | 0.5                 | 0.5                 | 0.7                 | 0.8                  | 0.6                  | 0.3                  | 0.5                  | 0.3                  | 0.6                  |
| Weib shape discrete   | asymptotic       | 6.3                 | 9.4                 | 3.3                 | 3.9                  | 2.6                  | 2.3                  | 4.5                  | 4.1                  | 3.0                  |
|                       | asymptotic_bonf  | 6.1                 | 9.1                 | 3.0                 | 3.4                  | 2.2                  | 2.2                  | 4.2                  | 3.7                  | 2.5                  |
|                       | permutation_bonf | 0.1                 | 0.3                 | 0.6                 | 0.8                  | 0.4                  | 0.1                  | 0.3                  | 0.2                  | 0.3                  |

Table S79: Rejection rates in percent for the Tukey-type contrast matrix with  $\delta = 1.5$  and balanced large sample sizes under unequal, high censoring.

| Distribution          | Method           | $\mathcal{H}_{0,7}$ | $\mathcal{H}_{0,8}$ | $\mathcal{H}_{0,9}$ | $\mathcal{H}_{0,13}$ | $\mathcal{H}_{0,14}$ | $\mathcal{H}_{0,15}$ | $\mathcal{H}_{0,16}$ | $\mathcal{H}_{0,17}$ | $\mathcal{H}_{0,18}$ |
|-----------------------|------------------|---------------------|---------------------|---------------------|----------------------|----------------------|----------------------|----------------------|----------------------|----------------------|
| exp early continuous  | asymptotic       | 67.1                | 46.9                | 85.6                | 65.1                 | 43.0                 | 85.2                 | 68.7                 | 45.8                 | 90.2                 |
|                       | asymptotic_bonf  | 65.3                | 44.7                | 84.3                | 63.2                 | 40.9                 | 83.9                 | 67.2                 | 43.6                 | 88.9                 |
|                       | permutation_bonf | 62.6                | 43.0                | 83.7                | 60.7                 | 39.3                 | 82.5                 | 64.8                 | 43.2                 | 86.4                 |
| exp early discrete    | asymptotic       | 71.6                | 50.9                | 88.1                | 69.7                 | 46.3                 | 87.9                 | 72.9                 | 51.5                 | 92.4                 |
|                       | asymptotic_bonf  | 69.9                | 49.0                | 87.0                | 68.1                 | 44.4                 | 86.3                 | 70.7                 | 49.4                 | 90.9                 |
|                       | permutation_bonf | 68.3                | 48.1                | 86.5                | 66.6                 | 41.6                 | 85.2                 | 69.5                 | 47.8                 | 89.6                 |
| exp late continuous   | asymptotic       | 68.7                | 48.2                | 86.9                | 66.2                 | 44.0                 | 86.7                 | 70.9                 | 49.0                 | 91.4                 |
|                       | asymptotic_bonf  | 66.9                | 45.8                | 86.0                | 64.0                 | 41.2                 | 85.2                 | 69.1                 | 46.1                 | 90.6                 |
|                       | permutation_bonf | 66.0                | 44.9                | 85.2                | 63.2                 | 41.2                 | 84.2                 | 67.3                 | 45.1                 | 88.9                 |
| exp late discrete     | asymptotic       | 73.9                | 53.2                | 89.4                | 71.9                 | 47.2                 | 89.1                 | 74.9                 | 52.1                 | 93.2                 |
|                       | asymptotic_bonf  | 72.3                | 50.5                | 88.9                | 69.6                 | 45.4                 | 87.4                 | 73.3                 | 50.2                 | 92.7                 |
|                       | permutation_bonf | 71.2                | 48.5                | 87.0                | 68.9                 | 44.0                 | 87.2                 | 72.7                 | 48.4                 | 91.1                 |
| exp prop continuous   | asymptotic       | 69.1                | 49.0                | 87.8                | 67.0                 | 47.7                 | 86.7                 | 69.3                 | 52.0                 | 89.1                 |
|                       | asymptotic_bonf  | 67.5                | 47.5                | 86.4                | 65.1                 | 46.1                 | 85.8                 | 67.9                 | 49.8                 | 88.2                 |
|                       | permutation_bonf | 66.2                | 46.0                | 84.7                | 63.1                 | 44.7                 | 84.9                 | 66.7                 | 48.6                 | 87.5                 |
| exp prop discrete     | asymptotic       | 74.0                | 52.9                | 89.3                | 72.0                 | 51.7                 | 89.4                 | 75.0                 | 55.6                 | 91.0                 |
|                       | asymptotic_bonf  | 72.3                | 50.9                | 88.4                | 70.4                 | 49.8                 | 88.4                 | 72.4                 | 53.5                 | 90.0                 |
|                       | permutation_bonf | 70.3                | 49.6                | 87.3                | 68.4                 | 47.0                 | 86.1                 | 70.8                 | 52.5                 | 90.4                 |
| logn continuous       | asymptotic       | 98.0                | 89.6                | 99.8                | 96.7                 | 87.5                 | 99.3                 | 98.0                 | 88.4                 | 99.8                 |
|                       | asymptotic_bonf  | 97.6                | 88.1                | 99.7                | 96.4                 | 86.8                 | 99.3                 | 97.9                 | 87.1                 | 99.8                 |
|                       | permutation_bonf | 97.7                | 86.9                | 99.6                | 96.2                 | 84.2                 | 99.1                 | 97.2                 | 87.4                 | 99.9                 |
| logn discrete         | asymptotic       | 99.1                | 94.8                | 100.0               | 98.4                 | 92.6                 | 99.7                 | 99.2                 | 93.5                 | 100.0                |
|                       | asymptotic_bonf  | 99.0                | 93.9                | 100.0               | 98.2                 | 92.0                 | 99.7                 | 99.1                 | 92.6                 | 100.0                |
|                       | permutation_bonf | 99.0                | 93.6                | 99.9                | 98.0                 | 90.8                 | 99.5                 | 98.4                 | 92.9                 | 99.9                 |
| pwExp continuous      | asymptotic       | 65.5                | 44.9                | 84.6                | 65.1                 | 41.7                 | 85.8                 | 66.7                 | 45.3                 | 89.1                 |
|                       | asymptotic_bonf  | 63.5                | 42.3                | 83.2                | 62.4                 | 39.7                 | 84.7                 | 65.4                 | 43.2                 | 87.8                 |
|                       | permutation_bonf | 60.9                | 41.9                | 83.7                | 61.9                 | 39.4                 | 82.9                 | 65.2                 | 43.1                 | 86.3                 |
| pwExp discrete        | asymptotic       | 70.7                | 49.6                | 87.8                | 69.9                 | 44.8                 | 88.0                 | 70.9                 | 50.2                 | 91.6                 |
|                       | asymptotic_bonf  | 68.9                | 47.2                | 87.1                | 68.2                 | 43.1                 | 86.8                 | 69.5                 | 48.2                 | 91.0                 |
|                       | permutation_bonf | 66.7                | 46.5                | 86.8                | 66.3                 | 42.4                 | 86.6                 | 68.4                 | 47.1                 | 89.2                 |
| Weib late continuous  | asymptotic       | 98.1                | 90.1                | 100.0               | 96.5                 | 89.2                 | 99.7                 | 97.0                 | 89.4                 | 99.8                 |
|                       | asymptotic_bonf  | 98.0                | 89.1                | 100.0               | 96.3                 | 87.7                 | 99.7                 | 96.9                 | 88.6                 | 99.7                 |
|                       | permutation_bonf | 97.5                | 88.3                | 99.6                | 95.4                 | 86.9                 | 99.6                 | 96.0                 | 87.3                 | 99.2                 |
| Weib late discrete    | asymptotic       | 99.2                | 94.8                | 99.9                | 98.2                 | 92.8                 | 99.9                 | 98.4                 | 92.9                 | 99.8                 |
|                       | asymptotic_bonf  | 99.0                | 94.1                | 99.9                | 98.0                 | 91.7                 | 99.9                 | 98.2                 | 92.2                 | 99.8                 |
|                       | permutation_bonf | 98.9                | 93.5                | 99.8                | 97.6                 | 91.0                 | 99.9                 | 98.1                 | 91.6                 | 99.6                 |
| Weib prop continuous  | asymptotic       | 97.7                | 88.9                | 100.0               | 96.5                 | 88.7                 | 99.7                 | 96.7                 | 88.9                 | 99.5                 |
|                       | asymptotic_bonf  | 97.3                | 87.4                | 100.0               | 95.9                 | 87.2                 | 99.6                 | 96.4                 | 87.7                 | 99.3                 |
|                       | permutation_bonf | 97.0                | 87.7                | 99.7                | 95.2                 | 86.5                 | 99.7                 | 96.0                 | 87.3                 | 99.3                 |
| Weib prop discrete    | asymptotic       | 99.0                | 94.0                | 100.0               | 97.9                 | 92.2                 | 99.9                 | 98.5                 | 93.0                 | 99.9                 |
|                       | asymptotic_bonf  | 98.9                | 93.4                | 100.0               | 97.7                 | 91.6                 | 99.9                 | 98.2                 | 92.3                 | 99.8                 |
|                       | permutation_bonf | 99.0                | 92.9                | 99.9                | 97.5                 | 90.8                 | 99.9                 | 97.9                 | 91.7                 | 99.6                 |
| Weib scale continuous | asymptotic       | 96.4                | 86.0                | 99.8                | 95.2                 | 84.0                 | 99.3                 | 95.9                 | 85.2                 | 99.0                 |
|                       | asymptotic_bonf  | 96.0                | 84.6                | 99.7                | 94.4                 | 82.1                 | 99.2                 | 95.0                 | 84.2                 | 98.9                 |
|                       | permutation_bonf | 95.2                | 83.1                | 99.3                | 93.2                 | 79.8                 | 98.9                 | 93.7                 | 82.2                 | 98.7                 |
| Weib scale discrete   | asymptotic       | 98.3                | 91.0                | 100.0               | 97.0                 | 89.3                 | 99.7                 | 98.1                 | 90.4                 | 99.4                 |
|                       | asymptotic_bonf  | 98.2                | 90.3                | 99.8                | 96.9                 | 88.4                 | 99.7                 | 97.8                 | 89.1                 | 99.4                 |
|                       | permutation_bonf | 97.4                | 90.6                | 99.7                | 96.7                 | 88.0                 | 99.4                 | 97.2                 | 88.1                 | 99.2                 |
| Weib shape continuous | asymptotic       | 94.6                | 81.3                | 98.9                | 92.8                 | 78.5                 | 98.2                 | 93.4                 | 80.8                 | 97.9                 |
|                       | asymptotic_bonf  | 94.0                | 79.7                | 98.8                | 92.1                 | 77.0                 | 97.7                 | 92.8                 | 79.2                 | 97.7                 |
|                       | permutation_bonf | 93.3                | 77.8                | 98.3                | 91.0                 | 76.0                 | 97.3                 | 92.6                 | 77.4                 | 97.3                 |
| Weib shape discrete   | asymptotic       | 97.1                | 87.6                | 99.7                | 95.9                 | 85.4                 | 99.5                 | 96.0                 | 85.5                 | 99.0                 |
|                       | asymptotic_bonf  | 96.5                | 86.4                | 99.7                | 95.4                 | 83.7                 | 99.2                 | 95.9                 | 84.9                 | 98.9                 |
|                       | permutation_bonf | 96.5                | 86.2                | 99.1                | 94.3                 | 82.5                 | 99.2                 | 95.2                 | 84.2                 | 98.5                 |

Table S80: Rejection rates in percent for the Tukey-type contrast matrix with  $\delta = 1.5$  and balanced medium sample sizes under unequal, high censoring.

| Distribution          | Method           | $\mathcal{H}_{0,7}$ | $\mathcal{H}_{0,8}$ | $\mathcal{H}_{0,9}$ | $\mathcal{H}_{0,13}$ | $\mathcal{H}_{0,14}$ | $\mathcal{H}_{0,15}$ | $\mathcal{H}_{0,16}$ | $\mathcal{H}_{0,17}$ | $\mathcal{H}_{0,18}$ |
|-----------------------|------------------|---------------------|---------------------|---------------------|----------------------|----------------------|----------------------|----------------------|----------------------|----------------------|
| exp early continuous  | asymptotic       | 9.4                 | 5.5                 | 11.4                | 9.1                  | 5.5                  | 12.0                 | 9.0                  | 3.8                  | 13.5                 |
|                       | asymptotic_bonf  | 8.6                 | 4.7                 | 10.5                | 8.1                  | 4.7                  | 10.4                 | 8.4                  | 3.6                  | 12.3                 |
|                       | permutation_bonf | 8.3                 | 4.4                 | 11.0                | 8.2                  | 3.7                  | 10.0                 | 7.7                  | 3.9                  | 11.3                 |
| exp early discrete    | asymptotic       | 11.1                | 5.1                 | 12.9                | 10.4                 | 4.4                  | 14.8                 | 9.9                  | 5.0                  | 15.4                 |
|                       | asymptotic_bonf  | 10.2                | 4.6                 | 12.1                | 9.4                  | 4.0                  | 13.1                 | 8.9                  | 4.2                  | 13.7                 |
|                       | permutation_bonf | 9.6                 | 4.4                 | 12.4                | 9.1                  | 3.9                  | 12.9                 | 8.6                  | 3.8                  | 13.0                 |
| exp late continuous   | asymptotic       | 9.7                 | 5.5                 | 13.6                | 9.9                  | 5.1                  | 13.6                 | 10.5                 | 4.4                  | 14.3                 |
|                       | asymptotic_bonf  | 8.6                 | 4.7                 | 12.6                | 9.3                  | 4.5                  | 12.7                 | 9.8                  | 3.7                  | 12.8                 |
|                       | permutation_bonf | 8.0                 | 4.7                 | 11.9                | 8.6                  | 4.0                  | 11.0                 | 8.8                  | 3.3                  | 13.1                 |
| exp late discrete     | asymptotic       | 11.0                | 5.4                 | 14.5                | 11.0                 | 5.5                  | 15.0                 | 10.8                 | 4.9                  | 17.6                 |
|                       | asymptotic_bonf  | 10.1                | 4.9                 | 13.3                | 9.8                  | 4.9                  | 13.9                 | 9.8                  | 4.4                  | 15.4                 |
|                       | permutation_bonf | 9.8                 | 4.2                 | 12.4                | 9.5                  | 4.8                  | 12.8                 | 9.8                  | 4.4                  | 15.1                 |
| exp prop continuous   | asymptotic       | 10.0                | 6.4                 | 11.5                | 8.3                  | 6.4                  | 13.1                 | 9.1                  | 5.8                  | 13.8                 |
|                       | asymptotic_bonf  | 8.6                 | 5.9                 | 10.0                | 7.3                  | 5.8                  | 12.0                 | 8.3                  | 4.8                  | 12.6                 |
|                       | permutation_bonf | 8.0                 | 5.6                 | 10.6                | 6.6                  | 6.2                  | 11.1                 | 7.6                  | 4.7                  | 11.6                 |
| exp prop discrete     | asymptotic       | 10.8                | 7.4                 | 13.2                | 9.2                  | 6.7                  | 14.4                 | 10.7                 | 6.2                  | 15.1                 |
|                       | asymptotic_bonf  | 10.0                | 6.3                 | 11.9                | 8.2                  | 5.6                  | 13.3                 | 9.8                  | 5.3                  | 14.2                 |
|                       | permutation_bonf | 9.7                 | 5.2                 | 11.5                | 7.6                  | 5.6                  | 12.5                 | 9.1                  | 4.9                  | 13.4                 |
| logn continuous       | asymptotic       | 21.7                | 13.4                | 39.2                | 20.6                 | 13.2                 | 36.2                 | 23.8                 | 12.3                 | 35.7                 |
|                       | asymptotic_bonf  | 20.5                | 12.4                | 37.5                | 18.9                 | 12.5                 | 34.4                 | 22.3                 | 10.5                 | 33.5                 |
|                       | permutation_bonf | 19.1                | 11.8                | 35.3                | 18.3                 | 11.4                 | 32.0                 | 21.5                 | 10.5                 | 31.8                 |
| logn discrete         | asymptotic       | 27.1                | 17.4                | 46.2                | 24.2                 | 17.2                 | 42.3                 | 28.9                 | 15.5                 | 41.9                 |
|                       | asymptotic_bonf  | 24.7                | 16.1                | 44.0                | 22.9                 | 16.0                 | 40.6                 | 27.2                 | 13.7                 | 39.6                 |
|                       | permutation_bonf | 24.2                | 15.6                | 42.7                | 22.3                 | 16.3                 | 40.3                 | 25.9                 | 14.2                 | 37.2                 |
| pwExp continuous      | asymptotic       | 8.1                 | 5.5                 | 12.6                | 8.3                  | 5.0                  | 12.0                 | 8.4                  | 3.6                  | 13.2                 |
|                       | asymptotic_bonf  | 7.7                 | 4.8                 | 12.2                | 7.9                  | 4.3                  | 11.0                 | 7.9                  | 3.1                  | 12.0                 |
|                       | permutation_bonf | 6.8                 | 4.5                 | 11.3                | 8.4                  | 3.9                  | 10.9                 | 7.0                  | 3.3                  | 12.0                 |
| pwExp discrete        | asymptotic       | 10.1                | 5.5                 | 14.9                | 9.7                  | 4.4                  | 14.5                 | 9.3                  | 4.5                  | 14.8                 |
|                       | asymptotic_bonf  | 8.9                 | 5.2                 | 13.8                | 8.9                  | 4.0                  | 13.5                 | 8.5                  | 4.2                  | 14.0                 |
|                       | permutation_bonf | 8.8                 | 4.4                 | 12.5                | 9.0                  | 4.2                  | 12.8                 | 7.6                  | 4.2                  | 12.8                 |
| Weib late continuous  | asymptotic       | 24.1                | 13.8                | 39.0                | 21.2                 | 12.5                 | 38.1                 | 24.5                 | 15.0                 | 37.8                 |
|                       | asymptotic_bonf  | 21.8                | 12.8                | 37.0                | 20.1                 | 11.4                 | 35.8                 | 23.0                 | 13.5                 | 36.0                 |
|                       | permutation_bonf | 20.1                | 12.0                | 35.8                | 17.9                 | 10.2                 | 33.3                 | 20.8                 | 12.7                 | 33.3                 |
| Weib late discrete    | asymptotic       | 26.8                | 16.3                | 43.9                | 25.0                 | 14.5                 | 40.8                 | 28.4                 | 16.6                 | 41.8                 |
|                       | asymptotic_bonf  | 25.2                | 14.5                | 42.4                | 22.5                 | 13.5                 | 39.2                 | 26.4                 | 15.3                 | 39.9                 |
|                       | permutation_bonf | 23.5                | 14.5                | 39.8                | 21.3                 | 12.6                 | 37.4                 | 25.3                 | 15.5                 | 38.0                 |
| Weib prop continuous  | asymptotic       | 21.7                | 13.1                | 36.7                | 20.6                 | 12.4                 | 35.8                 | 23.6                 | 15.0                 | 35.6                 |
|                       | asymptotic_bonf  | 19.9                | 12.2                | 35.3                | 19.1                 | 11.7                 | 33.2                 | 22.7                 | 13.7                 | 34.3                 |
|                       | permutation_bonf | 19.7                | 11.2                | 33.7                | 17.8                 | 10.4                 | 31.1                 | 20.1                 | 12.8                 | 32.4                 |
| Weib prop discrete    | asymptotic       | 28.4                | 16.1                | 44.2                | 24.5                 | 15.1                 | 41.4                 | 27.8                 | 16.5                 | 40.8                 |
|                       | asymptotic_bonf  | 26.7                | 14.7                | 42.5                | 23.7                 | 14.3                 | 39.9                 | 26.3                 | 14.9                 | 39.1                 |
|                       | permutation_bonf | 24.9                | 13.9                | 39.5                | 22.5                 | 13.9                 | 39.1                 | 24.9                 | 14.9                 | 38.8                 |
| Weib scale continuous | asymptotic       | 18.6                | 11.9                | 32.0                | 17.6                 | 10.4                 | 30.5                 | 20.0                 | 11.8                 | 28.9                 |
|                       | asymptotic_bonf  | 16.9                | 10.9                | 30.1                | 16.2                 | 9.6                  | 29.0                 | 18.0                 | 11.1                 | 27.3                 |
|                       | permutation_bonf | 16.3                | 10.1                | 28.1                | 15.8                 | 9.2                  | 27.4                 | 17.1                 | 10.7                 | 26.2                 |
| Weib scale discrete   | asymptotic       | 22.9                | 13.4                | 39.2                | 21.2                 | 13.3                 | 36.4                 | 24.3                 | 14.8                 | 34.8                 |
|                       | asymptotic_bonf  | 21.4                | 12.3                | 37.8                | 19.4                 | 11.8                 | 34.3                 | 22.8                 | 13.4                 | 33.3                 |
|                       | permutation_bonf | 19.5                | 12.2                | 35.7                | 19.4                 | 12.4                 | 32.8                 | 21.4                 | 12.6                 | 32.3                 |
| Weib shape continuous | asymptotic       | 15.6                | 9.7                 | 26.6                | 15.8                 | 9.4                  | 26.1                 | 16.8                 | 10.8                 | 24.5                 |
|                       | asymptotic_bonf  | 14.4                | 8.6                 | 24.7                | 14.0                 | 8.4                  | 25.0                 | 14.6                 | 9.1                  | 23.0                 |
|                       | permutation_bonf | 13.5                | 9.3                 | 23.2                | 13.4                 | 8.3                  | 23.3                 | 15.7                 | 9.7                  | 21.3                 |
| Weib shape discrete   | asymptotic       | 18.1                | 10.9                | 32.9                | 18.9                 | 11.9                 | 32.1                 | 20.4                 | 12.4                 | 28.1                 |
|                       | asymptotic_bonf  | 16.7                | 10.0                | 30.0                | 17.3                 | 10.4                 | 29.8                 | 19.7                 | 11.3                 | 26.6                 |
|                       | permutation_bonf | 15.6                | 10.5                | 27.8                | 15.8                 | 10.0                 | 28.3                 | 18.0                 | 10.5                 | 24.6                 |

Table S81: Rejection rates in percent for the Tukey-type contrast matrix with  $\delta = 1.5$  and balanced small sample sizes under unequal, high censoring.

| Distribution          | Method           | $\mathcal{H}_{0,7}$ | $\mathcal{H}_{0,8}$ | $\mathcal{H}_{0,9}$ | $\mathcal{H}_{0,13}$ | $\mathcal{H}_{0,14}$ | $\mathcal{H}_{0,15}$ | $\mathcal{H}_{0,16}$ | $\mathcal{H}_{0,17}$ | $\mathcal{H}_{0,18}$ |
|-----------------------|------------------|---------------------|---------------------|---------------------|----------------------|----------------------|----------------------|----------------------|----------------------|----------------------|
| exp early continuous  | asymptotic       | 2.1                 | 1.2                 | 2.2                 | 1.7                  | 1.4                  | 2.4                  | 2.1                  | 0.7                  | 2.1                  |
|                       | asymptotic_bonf  | 1.9                 | 0.9                 | 1.8                 | 1.3                  | 1.1                  | 2.2                  | 1.8                  | 0.4                  | 1.6                  |
|                       | permutation_bonf | 1.3                 | 0.8                 | 1.5                 | 1.2                  | 1.3                  | 1.9                  | 1.1                  | 0.5                  | 1.5                  |
| exp early discrete    | asymptotic       | 1.5                 | 1.3                 | 1.2                 | 1.6                  | 1.2                  | 2.7                  | 1.6                  | 1.0                  | 2.6                  |
|                       | asymptotic_bonf  | 1.3                 | 1.2                 | 1.0                 | 1.3                  | 1.1                  | 2.6                  | 1.3                  | 0.6                  | 2.0                  |
|                       | permutation_bonf | 1.2                 | 1.0                 | 1.0                 | 0.9                  | 0.9                  | 1.9                  | 1.0                  | 0.7                  | 1.6                  |
| exp late continuous   | asymptotic       | 2.0                 | 1.3                 | 2.6                 | 2.1                  | 1.2                  | 2.5                  | 2.2                  | 0.8                  | 2.4                  |
|                       | asymptotic_bonf  | 1.4                 | 0.9                 | 2.0                 | 1.9                  | 1.0                  | 2.2                  | 2.1                  | 0.6                  | 2.3                  |
|                       | permutation_bonf | 1.1                 | 0.7                 | 1.5                 | 1.3                  | 1.1                  | 1.7                  | 1.3                  | 0.5                  | 1.7                  |
| exp late discrete     | asymptotic       | 2.3                 | 1.1                 | 2.4                 | 2.2                  | 1.1                  | 2.5                  | 2.7                  | 1.0                  | 2.4                  |
|                       | asymptotic_bonf  | 2.0                 | 0.9                 | 2.3                 | 2.1                  | 1.1                  | 2.2                  | 2.1                  | 0.8                  | 2.2                  |
|                       | permutation_bonf | 1.4                 | 0.4                 | 1.5                 | 1.6                  | 1.0                  | 1.4                  | 1.4                  | 0.5                  | 1.5                  |
| exp prop continuous   | asymptotic       | 0.8                 | 1.3                 | 2.6                 | 1.9                  | 0.6                  | 1.6                  | 1.0                  | 1.3                  | 2.1                  |
|                       | asymptotic_bonf  | 0.6                 | 1.3                 | 2.2                 | 1.8                  | 0.6                  | 1.4                  | 0.9                  | 1.1                  | 1.9                  |
|                       | permutation_bonf | 0.5                 | 1.0                 | 1.5                 | 1.1                  | 0.5                  | 1.3                  | 0.5                  | 0.8                  | 1.6                  |
| exp prop discrete     | asymptotic       | 1.9                 | 0.8                 | 2.4                 | 1.4                  | 1.5                  | 2.8                  | 1.1                  | 0.8                  | 2.9                  |
|                       | asymptotic_bonf  | 1.5                 | 0.7                 | 2.2                 | 1.4                  | 1.2                  | 2.6                  | 0.9                  | 0.7                  | 2.2                  |
|                       | permutation_bonf | 0.9                 | 0.6                 | 1.4                 | 0.7                  | 1.1                  | 1.6                  | 0.7                  | 0.5                  | 1.6                  |
| logn continuous       | asymptotic       | 3.4                 | 1.9                 | 6.0                 | 3.6                  | 1.7                  | 4.7                  | 3.0                  | 1.9                  | 5.2                  |
|                       | asymptotic_bonf  | 3.0                 | 1.5                 | 5.3                 | 3.2                  | 1.5                  | 4.3                  | 2.3                  | 1.7                  | 4.6                  |
|                       | permutation_bonf | 2.5                 | 1.6                 | 4.3                 | 2.4                  | 1.1                  | 3.9                  | 1.8                  | 1.7                  | 3.2                  |
| logn discrete         | asymptotic       | 3.9                 | 2.3                 | 6.3                 | 4.1                  | 2.5                  | 5.2                  | 4.0                  | 2.8                  | 6.1                  |
|                       | asymptotic_bonf  | 3.6                 | 1.8                 | 5.8                 | 3.6                  | 2.3                  | 4.7                  | 3.6                  | 2.4                  | 5.2                  |
|                       | permutation_bonf | 3.0                 | 1.8                 | 4.5                 | 2.8                  | 1.9                  | 3.6                  | 2.6                  | 2.4                  | 3.8                  |
| pwExp continuous      | asymptotic       | 1.5                 | 1.3                 | 2.1                 | 1.4                  | 1.4                  | 2.4                  | 2.0                  | 0.6                  | 1.8                  |
|                       | asymptotic_bonf  | 1.1                 | 1.3                 | 1.8                 | 1.2                  | 1.3                  | 2.0                  | 1.7                  | 0.6                  | 1.5                  |
|                       | permutation_bonf | 0.9                 | 0.6                 | 1.0                 | 0.7                  | 1.1                  | 1.3                  | 1.3                  | 0.4                  | 1.4                  |
| pwExp discrete        | asymptotic       | 1.8                 | 1.5                 | 2.4                 | 2.0                  | 1.0                  | 3.0                  | 2.6                  | 0.6                  | 2.4                  |
|                       | asymptotic_bonf  | 1.6                 | 1.1                 | 2.1                 | 1.7                  | 0.9                  | 2.3                  | 2.3                  | 0.5                  | 1.9                  |
|                       | permutation_bonf | 1.1                 | 0.8                 | 2.1                 | 1.2                  | 0.5                  | 1.9                  | 1.7                  | 0.5                  | 1.6                  |
| Weib late continuous  | asymptotic       | 2.1                 | 3.6                 | 5.4                 | 2.7                  | 2.9                  | 5.9                  | 3.3                  | 2.9                  | 5.2                  |
|                       | asymptotic_bonf  | 2.0                 | 3.2                 | 4.4                 | 2.3                  | 2.6                  | 5.2                  | 3.0                  | 2.6                  | 4.5                  |
|                       | permutation_bonf | 1.3                 | 2.7                 | 3.1                 | 1.8                  | 2.0                  | 3.7                  | 2.0                  | 1.6                  | 3.1                  |
| Weib late discrete    | asymptotic       | 2.7                 | 4.3                 | 6.4                 | 3.2                  | 3.0                  | 6.3                  | 3.9                  | 3.2                  | 5.4                  |
|                       | asymptotic_bonf  | 2.4                 | 3.8                 | 5.6                 | 2.8                  | 2.7                  | 5.8                  | 3.6                  | 3.2                  | 4.8                  |
|                       | permutation_bonf | 1.4                 | 3.2                 | 4.1                 | 2.2                  | 2.3                  | 3.8                  | 2.7                  | 2.7                  | 3.9                  |
| Weib prop continuous  | asymptotic       | 2.0                 | 3.3                 | 5.0                 | 2.5                  | 2.7                  | 5.5                  | 2.8                  | 2.8                  | 4.6                  |
|                       | asymptotic_bonf  | 1.8                 | 2.8                 | 3.8                 | 2.0                  | 2.5                  | 4.8                  | 2.7                  | 2.0                  | 4.4                  |
|                       | permutation_bonf | 1.2                 | 2.2                 | 3.3                 | 1.8                  | 1.6                  | 3.5                  | 1.9                  | 1.6                  | 2.7                  |
| Weib prop discrete    | asymptotic       | 2.3                 | 3.4                 | 5.7                 | 2.6                  | 2.8                  | 6.0                  | 3.3                  | 3.1                  | 4.9                  |
|                       | asymptotic_bonf  | 1.8                 | 3.2                 | 5.2                 | 2.3                  | 2.5                  | 5.8                  | 2.8                  | 2.8                  | 4.6                  |
|                       | permutation_bonf | 1.9                 | 2.5                 | 3.5                 | 1.8                  | 1.9                  | 3.9                  | 2.1                  | 2.0                  | 3.5                  |
| Weib scale continuous | asymptotic       | 1.2                 | 2.3                 | 3.1                 | 1.4                  | 1.9                  | 4.2                  | 1.8                  | 2.0                  | 3.6                  |
|                       | asymptotic_bonf  | 0.8                 | 2.2                 | 2.9                 | 1.2                  | 1.4                  | 2.8                  | 1.5                  | 1.8                  | 2.8                  |
|                       | permutation_bonf | 0.7                 | 1.7                 | 2.7                 | 1.0                  | 1.0                  | 2.0                  | 1.0                  | 1.4                  | 2.2                  |
| Weib scale discrete   | asymptotic       | 1.4                 | 2.4                 | 3.8                 | 1.7                  | 1.7                  | 4.6                  | 2.2                  | 2.0                  | 3.6                  |
|                       | asymptotic_bonf  | 1.1                 | 2.1                 | 3.4                 | 1.5                  | 1.2                  | 3.8                  | 1.8                  | 1.4                  | 3.0                  |
|                       | permutation_bonf | 0.8                 | 1.9                 | 2.7                 | 1.4                  | 1.0                  | 3.1                  | 1.2                  | 1.6                  | 2.0                  |
| Weib shape continuous | asymptotic       | 1.1                 | 1.5                 | 2.4                 | 1.2                  | 1.1                  | 2.6                  | 1.2                  | 1.5                  | 2.2                  |
|                       | asymptotic_bonf  | 0.7                 | 1.3                 | 2.4                 | 1.0                  | 0.9                  | 2.5                  | 0.9                  | 1.1                  | 1.9                  |
|                       | permutation_bonf | 0.6                 | 1.1                 | 1.8                 | 0.6                  | 0.9                  | 1.8                  | 0.8                  | 1.0                  | 1.8                  |
| Weib shape discrete   | asymptotic       | 0.8                 | 1.7                 | 2.9                 | 1.4                  | 1.3                  | 3.4                  | 1.4                  | 1.7                  | 2.5                  |
|                       | asymptotic_bonf  | 0.8                 | 1.5                 | 2.6                 | 1.2                  | 0.8                  | 3.1                  | 1.2                  | 1.6                  | 2.1                  |
|                       | permutation_bonf | 0.7                 | 1.2                 | 1.9                 | 1.2                  | 1.1                  | 2.9                  | 0.8                  | 1.3                  | 1.8                  |



Table S82: Rejection rates in percent for the Tukey-type contrast matrix with  $\delta = 1.5$  and unbalanced large sample sizes under unequal, high censoring.

| Distribution          | Method           | $\mathcal{H}_{0,7}$ | $\mathcal{H}_{0,8}$ | $\mathcal{H}_{0,9}$ | $\mathcal{H}_{0,13}$ | $\mathcal{H}_{0,14}$ | $\mathcal{H}_{0,15}$ | $\mathcal{H}_{0,16}$ | $\mathcal{H}_{0,17}$ | $\mathcal{H}_{0,18}$ |
|-----------------------|------------------|---------------------|---------------------|---------------------|----------------------|----------------------|----------------------|----------------------|----------------------|----------------------|
| exp early continuous  | asymptotic       | 24.4                | 12.2                | 46.6                | 20.1                 | 11.2                 | 34.4                 | 21.2                 | 10.6                 | 38.4                 |
|                       | asymptotic_bonf  | 22.2                | 10.6                | 43.6                | 17.4                 | 9.4                  | 30.8                 | 18.9                 | 8.7                  | 35.3                 |
|                       | permutation_bonf | 18.9                | 8.4                 | 38.9                | 16.0                 | 7.9                  | 29.0                 | 17.7                 | 7.1                  | 32.3                 |
| exp early discrete    | asymptotic       | 28.3                | 14.5                | 50.3                | 22.3                 | 11.4                 | 37.0                 | 23.8                 | 12.1                 | 41.0                 |
|                       | asymptotic_bonf  | 24.9                | 12.7                | 47.0                | 20.1                 | 9.7                  | 34.0                 | 21.1                 | 10.2                 | 37.7                 |
|                       | permutation_bonf | 22.4                | 9.2                 | 41.4                | 19.3                 | 8.5                  | 32.3                 | 19.1                 | 8.2                  | 35.5                 |
| exp late continuous   | asymptotic       | 27.8                | 13.8                | 50.6                | 20.8                 | 12.0                 | 36.4                 | 22.9                 | 10.7                 | 41.1                 |
|                       | asymptotic_bonf  | 24.2                | 12.2                | 47.6                | 18.7                 | 10.1                 | 33.4                 | 20.2                 | 9.0                  | 38.1                 |
|                       | permutation_bonf | 21.1                | 9.7                 | 42.0                | 17.5                 | 8.4                  | 31.6                 | 18.9                 | 7.7                  | 35.2                 |
| exp late discrete     | asymptotic       | 31.6                | 16.0                | 55.1                | 23.1                 | 12.0                 | 39.8                 | 25.3                 | 13.2                 | 45.0                 |
|                       | asymptotic_bonf  | 26.7                | 14.2                | 52.0                | 20.9                 | 9.7                  | 36.5                 | 22.9                 | 11.4                 | 40.8                 |
|                       | permutation_bonf | 23.6                | 11.1                | 46.5                | 19.8                 | 9.3                  | 34.9                 | 21.6                 | 9.4                  | 39.4                 |
| exp prop continuous   | asymptotic       | 26.7                | 15.2                | 43.6                | 21.5                 | 12.8                 | 30.8                 | 20.7                 | 12.0                 | 38.0                 |
|                       | asymptotic_bonf  | 23.8                | 13.9                | 40.5                | 19.0                 | 10.8                 | 28.1                 | 18.7                 | 10.6                 | 34.5                 |
|                       | permutation_bonf | 20.1                | 10.1                | 36.5                | 18.2                 | 9.4                  | 26.2                 | 16.1                 | 9.7                  | 32.9                 |
| exp prop discrete     | asymptotic       | 28.7                | 18.1                | 48.6                | 23.3                 | 14.5                 | 35.3                 | 23.4                 | 14.9                 | 41.4                 |
|                       | asymptotic_bonf  | 25.5                | 15.9                | 44.0                | 20.9                 | 12.7                 | 32.7                 | 20.8                 | 13.0                 | 38.2                 |
|                       | permutation_bonf | 22.7                | 12.3                | 41.1                | 18.9                 | 11.3                 | 31.0                 | 18.1                 | 10.8                 | 36.6                 |
| logn continuous       | asymptotic       | 64.7                | 40.9                | 80.7                | 54.4                 | 32.2                 | 68.2                 | 56.4                 | 35.3                 | 73.4                 |
|                       | asymptotic_bonf  | 61.6                | 37.0                | 77.3                | 50.0                 | 28.8                 | 64.3                 | 52.6                 | 32.2                 | 70.1                 |
|                       | permutation_bonf | 52.6                | 24.1                | 70.9                | 46.4                 | 24.6                 | 61.4                 | 45.4                 | 27.1                 | 65.9                 |
| logn discrete         | asymptotic       | 72.7                | 48.4                | 86.9                | 61.9                 | 39.3                 | 77.1                 | 63.4                 | 41.6                 | 81.1                 |
|                       | asymptotic_bonf  | 69.6                | 43.6                | 84.3                | 57.5                 | 35.4                 | 73.5                 | 60.3                 | 38.6                 | 78.4                 |
|                       | permutation_bonf | 59.2                | 29.3                | 77.9                | 54.8                 | 30.6                 | 69.7                 | 53.8                 | 32.2                 | 75.0                 |
| pwExp continuous      | asymptotic       | 24.0                | 11.9                | 46.1                | 18.3                 | 9.9                  | 35.1                 | 21.8                 | 11.4                 | 36.6                 |
|                       | asymptotic_bonf  | 22.6                | 9.9                 | 42.9                | 16.1                 | 8.8                  | 31.5                 | 19.5                 | 9.4                  | 33.7                 |
|                       | permutation_bonf | 19.1                | 8.2                 | 38.1                | 15.3                 | 7.3                  | 29.7                 | 17.1                 | 7.4                  | 31.0                 |
| pwExp discrete        | asymptotic       | 27.5                | 14.0                | 50.7                | 20.7                 | 11.1                 | 37.3                 | 23.6                 | 11.7                 | 40.8                 |
|                       | asymptotic_bonf  | 24.8                | 11.9                | 47.5                | 18.8                 | 9.4                  | 34.2                 | 21.3                 | 10.3                 | 37.3                 |
|                       | permutation_bonf | 21.0                | 9.6                 | 42.3                | 18.5                 | 8.3                  | 33.0                 | 19.8                 | 8.3                  | 33.4                 |
| Weib late continuous  | asymptotic       | 65.2                | 40.7                | 84.4                | 53.6                 | 32.9                 | 74.6                 | 55.2                 | 34.8                 | 78.2                 |
|                       | asymptotic_bonf  | 61.2                | 36.7                | 83.2                | 49.4                 | 29.9                 | 71.2                 | 51.9                 | 31.0                 | 75.2                 |
|                       | permutation_bonf | 51.6                | 26.2                | 77.9                | 44.9                 | 25.8                 | 68.3                 | 47.7                 | 25.3                 | 70.6                 |
| Weib late discrete    | asymptotic       | 70.0                | 45.0                | 86.6                | 60.9                 | 37.2                 | 77.3                 | 62.2                 | 39.0                 | 81.6                 |
|                       | asymptotic_bonf  | 66.6                | 42.9                | 84.6                | 58.0                 | 34.0                 | 75.2                 | 59.7                 | 35.7                 | 78.9                 |
|                       | permutation_bonf | 57.4                | 30.2                | 80.4                | 52.3                 | 29.5                 | 71.6                 | 53.0                 | 30.6                 | 75.0                 |
| Weib prop continuous  | asymptotic       | 62.9                | 38.8                | 82.9                | 51.0                 | 29.8                 | 71.4                 | 54.4                 | 32.3                 | 74.5                 |
|                       | asymptotic_bonf  | 58.9                | 34.2                | 80.5                | 47.1                 | 28.2                 | 68.0                 | 50.6                 | 29.7                 | 71.8                 |
|                       | permutation_bonf | 50.7                | 24.1                | 75.0                | 43.2                 | 23.4                 | 64.9                 | 46.0                 | 24.1                 | 67.0                 |
| Weib prop discrete    | asymptotic       | 69.9                | 45.7                | 87.2                | 60.7                 | 35.7                 | 79.6                 | 62.4                 | 38.6                 | 81.9                 |
|                       | asymptotic_bonf  | 66.7                | 42.3                | 85.5                | 56.2                 | 32.8                 | 76.7                 | 58.1                 | 34.9                 | 79.9                 |
|                       | permutation_bonf | 56.8                | 28.6                | 80.8                | 51.7                 | 28.6                 | 73.2                 | 52.0                 | 30.1                 | 75.3                 |
| Weib scale continuous | asymptotic       | 54.2                | 32.8                | 72.4                | 42.9                 | 24.8                 | 62.4                 | 45.0                 | 26.4                 | 67.5                 |
|                       | asymptotic_bonf  | 49.7                | 29.3                | 70.0                | 39.4                 | 21.9                 | 59.5                 | 42.1                 | 24.9                 | 63.6                 |
|                       | permutation_bonf | 42.8                | 21.0                | 63.9                | 35.7                 | 19.1                 | 55.4                 | 37.6                 | 20.1                 | 58.9                 |
| Weib scale discrete   | asymptotic       | 61.5                | 37.5                | 79.2                | 49.3                 | 29.5                 | 69.7                 | 52.7                 | 31.6                 | 74.5                 |
|                       | asymptotic_bonf  | 57.2                | 34.1                | 76.4                | 46.0                 | 26.7                 | 66.4                 | 48.0                 | 28.9                 | 71.1                 |
|                       | permutation_bonf | 48.3                | 23.6                | 70.9                | 41.6                 | 21.7                 | 62.8                 | 44.0                 | 24.0                 | 67.0                 |
| Weib shape continuous | asymptotic       | 44.2                | 23.9                | 62.6                | 35.5                 | 22.3                 | 53.7                 | 39.6                 | 22.1                 | 58.7                 |
|                       | asymptotic_bonf  | 41.2                | 20.8                | 58.8                | 31.3                 | 18.7                 | 50.2                 | 35.1                 | 19.0                 | 54.7                 |
|                       | permutation_bonf | 32.6                | 13.0                | 51.4                | 28.8                 | 15.8                 | 46.4                 | 29.6                 | 14.6                 | 48.3                 |
| Weib shape discrete   | asymptotic       | 51.6                | 30.0                | 70.0                | 42.7                 | 25.5                 | 61.1                 | 45.5                 | 26.8                 | 64.3                 |
|                       | asymptotic_bonf  | 46.6                | 26.2                | 66.3                | 38.9                 | 22.4                 | 57.6                 | 40.7                 | 22.8                 | 61.4                 |
|                       | permutation_bonf | 36.1                | 15.2                | 57.8                | 34.5                 | 18.1                 | 52.5                 | 35.1                 | 17.7                 | 55.5                 |

Table S83: Rejection rates in percent for the Tukey-type contrast matrix with  $\delta = 1.5$  and unbalanced medium sample sizes under unequal, high censoring.

| Distribution          | Method           | $\mathcal{H}_{0,7}$ | $\mathcal{H}_{0,8}$ | $\mathcal{H}_{0,9}$ | $\mathcal{H}_{0,13}$ | $\mathcal{H}_{0,14}$ | $\mathcal{H}_{0,15}$ | $\mathcal{H}_{0,16}$ | $\mathcal{H}_{0,17}$ | $\mathcal{H}_{0,18}$ |
|-----------------------|------------------|---------------------|---------------------|---------------------|----------------------|----------------------|----------------------|----------------------|----------------------|----------------------|
| exp early continuous  | asymptotic       | 1.6                 | 1.5                 | 3.4                 | 1.0                  | 0.9                  | 2.8                  | 2.1                  | 0.8                  | 3.4                  |
|                       | asymptotic_bonf  | 1.0                 | 1.0                 | 2.9                 | 0.8                  | 0.8                  | 2.5                  | 1.6                  | 0.6                  | 2.8                  |
|                       | permutation_bonf | 0.3                 | 0.1                 | 1.3                 | 0.4                  | 0.3                  | 1.5                  | 1.0                  | 0.1                  | 1.4                  |
| exp early discrete    | asymptotic       | 1.9                 | 1.2                 | 3.6                 | 1.7                  | 0.9                  | 3.4                  | 1.6                  | 0.7                  | 3.5                  |
|                       | asymptotic_bonf  | 1.2                 | 0.9                 | 3.0                 | 1.3                  | 0.7                  | 2.9                  | 1.4                  | 0.3                  | 2.8                  |
|                       | permutation_bonf | 0.5                 | 0.0                 | 1.0                 | 0.2                  | 0.5                  | 1.7                  | 0.6                  | 0.1                  | 1.7                  |
| exp late continuous   | asymptotic       | 2.4                 | 1.3                 | 3.6                 | 1.6                  | 1.1                  | 3.3                  | 2.3                  | 0.8                  | 3.9                  |
|                       | asymptotic_bonf  | 1.7                 | 1.0                 | 3.1                 | 1.1                  | 0.9                  | 2.6                  | 1.9                  | 0.5                  | 2.8                  |
|                       | permutation_bonf | 0.4                 | 0.1                 | 1.5                 | 0.4                  | 0.3                  | 1.7                  | 0.8                  | 0.1                  | 1.6                  |
| exp late discrete     | asymptotic       | 2.3                 | 1.2                 | 3.7                 | 2.1                  | 1.0                  | 3.7                  | 2.4                  | 1.2                  | 4.0                  |
|                       | asymptotic_bonf  | 1.6                 | 1.0                 | 2.9                 | 1.8                  | 1.0                  | 2.9                  | 2.1                  | 0.7                  | 3.4                  |
|                       | permutation_bonf | 0.3                 | 0.1                 | 1.6                 | 0.4                  | 0.3                  | 1.9                  | 1.0                  | 0.2                  | 1.9                  |
| exp prop continuous   | asymptotic       | 2.4                 | 1.2                 | 3.0                 | 2.1                  | 1.2                  | 2.8                  | 1.9                  | 1.5                  | 2.6                  |
|                       | asymptotic_bonf  | 1.9                 | 0.8                 | 2.5                 | 1.2                  | 0.9                  | 2.3                  | 1.6                  | 1.1                  | 2.1                  |
|                       | permutation_bonf | 0.5                 | 0.1                 | 1.2                 | 1.1                  | 0.5                  | 1.8                  | 0.8                  | 0.2                  | 1.7                  |
| exp prop discrete     | asymptotic       | 2.3                 | 1.1                 | 3.2                 | 1.8                  | 1.2                  | 3.1                  | 2.4                  | 1.6                  | 2.8                  |
|                       | asymptotic_bonf  | 2.0                 | 0.7                 | 2.4                 | 1.2                  | 1.2                  | 3.0                  | 1.8                  | 1.5                  | 2.6                  |
|                       | permutation_bonf | 0.8                 | 0.1                 | 1.2                 | 0.8                  | 0.3                  | 2.0                  | 0.8                  | 0.4                  | 1.8                  |
| logn continuous       | asymptotic       | 4.2                 | 2.3                 | 8.1                 | 4.6                  | 3.0                  | 6.9                  | 4.0                  | 2.3                  | 7.5                  |
|                       | asymptotic_bonf  | 3.4                 | 1.9                 | 6.8                 | 3.6                  | 2.7                  | 5.7                  | 3.0                  | 2.3                  | 6.7                  |
|                       | permutation_bonf | 0.4                 | 0.0                 | 1.3                 | 0.8                  | 0.4                  | 2.2                  | 1.0                  | 0.1                  | 2.8                  |
| logn discrete         | asymptotic       | 4.8                 | 2.8                 | 9.0                 | 4.8                  | 2.8                  | 8.9                  | 4.2                  | 2.6                  | 8.0                  |
|                       | asymptotic_bonf  | 4.0                 | 2.3                 | 7.8                 | 3.8                  | 2.8                  | 7.4                  | 3.6                  | 2.2                  | 7.2                  |
|                       | permutation_bonf | 0.2                 | 0.0                 | 0.7                 | 1.0                  | 0.3                  | 2.4                  | 1.0                  | 0.1                  | 3.5                  |
| pwExp continuous      | asymptotic       | 1.8                 | 1.3                 | 3.7                 | 1.0                  | 1.4                  | 3.1                  | 1.8                  | 1.1                  | 2.7                  |
|                       | asymptotic_bonf  | 1.2                 | 1.1                 | 2.7                 | 1.0                  | 1.2                  | 2.6                  | 1.6                  | 1.1                  | 2.3                  |
|                       | permutation_bonf | 0.1                 | 0.1                 | 1.0                 | 0.4                  | 0.3                  | 1.5                  | 0.7                  | 0.1                  | 1.5                  |
| pwExp discrete        | asymptotic       | 1.9                 | 1.0                 | 3.4                 | 1.2                  | 1.2                  | 3.1                  | 1.8                  | 1.2                  | 3.2                  |
|                       | asymptotic_bonf  | 1.4                 | 1.0                 | 3.0                 | 0.8                  | 1.2                  | 2.6                  | 1.3                  | 1.1                  | 2.5                  |
|                       | permutation_bonf | 0.3                 | 0.0                 | 1.3                 | 0.3                  | 0.7                  | 1.8                  | 0.6                  | 0.2                  | 1.2                  |
| Weib late continuous  | asymptotic       | 4.6                 | 1.5                 | 9.5                 | 4.5                  | 2.2                  | 6.8                  | 3.8                  | 2.5                  | 8.0                  |
|                       | asymptotic_bonf  | 3.9                 | 1.1                 | 8.1                 | 3.3                  | 1.8                  | 5.6                  | 3.0                  | 1.8                  | 7.1                  |
|                       | permutation_bonf | 0.3                 | 0.0                 | 1.7                 | 1.5                  | 0.3                  | 2.9                  | 0.9                  | 0.0                  | 3.1                  |
| Weib late discrete    | asymptotic       | 5.4                 | 1.6                 | 12.3                | 5.0                  | 2.3                  | 10.0                 | 5.2                  | 2.8                  | 10.9                 |
|                       | asymptotic_bonf  | 3.9                 | 1.3                 | 10.4                | 4.2                  | 1.9                  | 8.3                  | 3.9                  | 2.1                  | 9.4                  |
|                       | permutation_bonf | 0.0                 | 0.1                 | 2.4                 | 1.4                  | 0.2                  | 3.5                  | 0.5                  | 0.2                  | 3.5                  |
| Weib prop continuous  | asymptotic       | 4.7                 | 1.3                 | 7.8                 | 3.7                  | 1.9                  | 6.9                  | 3.7                  | 1.9                  | 8.0                  |
|                       | asymptotic_bonf  | 3.5                 | 0.9                 | 6.5                 | 3.1                  | 1.7                  | 5.9                  | 2.9                  | 1.4                  | 7.0                  |
|                       | permutation_bonf | 0.3                 | 0.0                 | 1.5                 | 1.6                  | 0.4                  | 2.7                  | 0.7                  | 0.1                  | 2.7                  |
| Weib prop discrete    | asymptotic       | 5.0                 | 1.4                 | 10.1                | 4.7                  | 2.1                  | 9.4                  | 4.4                  | 2.5                  | 9.5                  |
|                       | asymptotic_bonf  | 3.5                 | 0.8                 | 8.8                 | 3.7                  | 1.5                  | 7.5                  | 3.7                  | 1.7                  | 7.5                  |
|                       | permutation_bonf | 0.2                 | 0.0                 | 1.5                 | 1.4                  | 0.1                  | 2.8                  | 0.7                  | 0.3                  | 2.8                  |
| Weib scale continuous | asymptotic       | 2.9                 | 1.0                 | 4.9                 | 2.9                  | 1.2                  | 4.9                  | 2.8                  | 1.2                  | 5.5                  |
|                       | asymptotic_bonf  | 1.9                 | 0.8                 | 4.1                 | 2.4                  | 1.0                  | 4.1                  | 1.9                  | 0.6                  | 4.3                  |
|                       | permutation_bonf | 0.3                 | 0.0                 | 0.7                 | 0.7                  | 0.5                  | 1.5                  | 0.3                  | 0.0                  | 1.6                  |
| Weib scale discrete   | asymptotic       | 3.4                 | 1.0                 | 6.1                 | 3.4                  | 1.5                  | 5.6                  | 3.0                  | 1.3                  | 7.1                  |
|                       | asymptotic_bonf  | 3.0                 | 0.6                 | 4.6                 | 2.8                  | 1.0                  | 4.7                  | 2.1                  | 0.9                  | 5.4                  |
|                       | permutation_bonf | 0.2                 | 0.0                 | 0.4                 | 0.8                  | 0.3                  | 1.3                  | 0.4                  | 0.0                  | 2.0                  |
| Weib shape continuous | asymptotic       | 2.3                 | 1.0                 | 3.3                 | 2.8                  | 0.7                  | 3.2                  | 2.0                  | 0.8                  | 3.3                  |
|                       | asymptotic_bonf  | 1.6                 | 0.6                 | 2.8                 | 2.1                  | 0.7                  | 2.5                  | 1.5                  | 0.6                  | 2.9                  |
|                       | permutation_bonf | 0.2                 | 0.0                 | 0.5                 | 0.2                  | 0.3                  | 1.3                  | 0.3                  | 0.0                  | 1.0                  |
| Weib shape discrete   | asymptotic       | 2.2                 | 0.9                 | 3.8                 | 2.9                  | 0.8                  | 3.6                  | 2.2                  | 1.0                  | 3.8                  |
|                       | asymptotic_bonf  | 1.8                 | 0.6                 | 3.2                 | 2.1                  | 0.7                  | 3.3                  | 1.8                  | 0.5                  | 2.9                  |
|                       | permutation_bonf | 0.1                 | 0.0                 | 0.4                 | 0.4                  | 0.2                  | 1.0                  | 0.2                  | 0.0                  | 0.7                  |

Table S84: Rejection rates in percent for the Tukey-type contrast matrix with  $\delta = 1.5$  and unbalanced small sample sizes under unequal, high censoring.

| Distribution          | Method           | $\mathcal{H}_{0,7}$ | $\mathcal{H}_{0,8}$ | $\mathcal{H}_{0,9}$ | $\mathcal{H}_{0,13}$ | $\mathcal{H}_{0,14}$ | $\mathcal{H}_{0,15}$ | $\mathcal{H}_{0,16}$ | $\mathcal{H}_{0,17}$ | $\mathcal{H}_{0,18}$ |
|-----------------------|------------------|---------------------|---------------------|---------------------|----------------------|----------------------|----------------------|----------------------|----------------------|----------------------|
| exp early continuous  | asymptotic       | 0.9                 | 4.2                 | 1.3                 | 1.0                  | 1.7                  | 1.2                  | 0.9                  | 2.4                  | 1.4                  |
|                       | asymptotic_bonf  | 0.9                 | 4.1                 | 1.2                 | 0.8                  | 1.4                  | 0.9                  | 0.7                  | 2.1                  | 1.2                  |
|                       | permutation_bonf | 0.2                 | 0.1                 | 0.1                 | 0.0                  | 0.0                  | 0.1                  | 0.0                  | 0.3                  | 0.0                  |
| exp early discrete    | asymptotic       | 1.9                 | 5.1                 | 1.7                 | 1.4                  | 1.6                  | 1.2                  | 1.4                  | 2.9                  | 1.8                  |
|                       | asymptotic_bonf  | 1.9                 | 4.9                 | 1.5                 | 1.1                  | 1.4                  | 1.1                  | 1.3                  | 2.4                  | 1.3                  |
|                       | permutation_bonf | 0.2                 | 0.1                 | 0.0                 | 0.1                  | 0.1                  | 0.0                  | 0.1                  | 0.5                  | 0.0                  |
| exp late continuous   | asymptotic       | 1.1                 | 3.7                 | 1.7                 | 1.0                  | 1.6                  | 1.1                  | 0.8                  | 1.8                  | 1.5                  |
|                       | asymptotic_bonf  | 1.0                 | 3.5                 | 1.1                 | 1.0                  | 1.4                  | 0.8                  | 0.5                  | 1.5                  | 1.4                  |
|                       | permutation_bonf | 0.2                 | 0.1                 | 0.1                 | 0.0                  | 0.0                  | 0.0                  | 0.0                  | 0.2                  | 0.0                  |
| exp late discrete     | asymptotic       | 1.6                 | 4.1                 | 2.1                 | 1.6                  | 1.4                  | 1.7                  | 0.9                  | 1.7                  | 1.8                  |
|                       | asymptotic_bonf  | 1.6                 | 3.9                 | 1.9                 | 1.3                  | 1.3                  | 1.4                  | 0.8                  | 1.6                  | 1.3                  |
|                       | permutation_bonf | 0.2                 | 0.0                 | 0.0                 | 0.0                  | 0.0                  | 0.0                  | 0.1                  | 0.3                  | 0.1                  |
| exp prop continuous   | asymptotic       | 2.0                 | 4.5                 | 1.9                 | 1.3                  | 1.9                  | 1.8                  | 1.7                  | 2.1                  | 1.6                  |
|                       | asymptotic_bonf  | 1.7                 | 4.4                 | 1.7                 | 0.7                  | 1.3                  | 1.5                  | 1.5                  | 1.8                  | 1.2                  |
|                       | permutation_bonf | 0.3                 | 0.1                 | 0.0                 | 0.0                  | 0.2                  | 0.3                  | 0.2                  | 0.1                  | 0.2                  |
| exp prop discrete     | asymptotic       | 2.6                 | 5.0                 | 2.2                 | 1.6                  | 1.5                  | 2.1                  | 2.1                  | 2.1                  | 1.5                  |
|                       | asymptotic_bonf  | 2.5                 | 5.0                 | 1.8                 | 1.4                  | 1.3                  | 1.6                  | 1.8                  | 1.9                  | 1.3                  |
|                       | permutation_bonf | 0.3                 | 0.1                 | 0.0                 | 0.1                  | 0.1                  | 0.1                  | 0.1                  | 0.0                  | 0.2                  |
| logn continuous       | asymptotic       | 5.3                 | 10.5                | 3.6                 | 1.9                  | 0.8                  | 2.1                  | 2.9                  | 1.1                  | 3.0                  |
|                       | asymptotic_bonf  | 5.1                 | 10.1                | 3.5                 | 1.0                  | 0.7                  | 1.8                  | 2.5                  | 1.0                  | 2.6                  |
|                       | permutation_bonf | 0.2                 | 0.3                 | 0.2                 | 0.2                  | 0.5                  | 0.2                  | 0.1                  | 0.2                  | 0.3                  |
| logn discrete         | asymptotic       | 5.6                 | 11.3                | 4.2                 | 1.6                  | 0.8                  | 2.3                  | 2.6                  | 0.9                  | 2.9                  |
|                       | asymptotic_bonf  | 5.3                 | 9.9                 | 3.8                 | 1.0                  | 0.7                  | 1.8                  | 2.2                  | 0.7                  | 2.5                  |
|                       | permutation_bonf | 0.2                 | 0.5                 | 0.0                 | 0.4                  | 0.4                  | 0.3                  | 0.1                  | 0.3                  | 0.4                  |
| pwExp continuous      | asymptotic       | 1.2                 | 3.9                 | 1.5                 | 0.9                  | 1.4                  | 1.4                  | 0.8                  | 1.9                  | 1.3                  |
|                       | asymptotic_bonf  | 1.2                 | 3.9                 | 1.1                 | 0.7                  | 1.1                  | 1.2                  | 0.8                  | 1.7                  | 1.0                  |
|                       | permutation_bonf | 0.0                 | 0.2                 | 0.0                 | 0.0                  | 0.0                  | 0.0                  | 0.0                  | 0.1                  | 0.2                  |
| pwExp discrete        | asymptotic       | 1.3                 | 4.7                 | 1.4                 | 1.1                  | 1.3                  | 1.5                  | 1.3                  | 2.2                  | 1.8                  |
|                       | asymptotic_bonf  | 1.2                 | 4.5                 | 1.2                 | 0.9                  | 1.0                  | 1.2                  | 1.0                  | 1.8                  | 1.5                  |
|                       | permutation_bonf | 0.0                 | 0.1                 | 0.0                 | 0.0                  | 0.1                  | 0.1                  | 0.1                  | 0.2                  | 0.2                  |
| Weib late continuous  | asymptotic       | 5.0                 | 6.5                 | 3.1                 | 1.8                  | 0.7                  | 2.6                  | 2.3                  | 1.1                  | 2.4                  |
|                       | asymptotic_bonf  | 5.0                 | 6.2                 | 3.0                 | 1.5                  | 0.6                  | 2.1                  | 2.2                  | 0.9                  | 2.3                  |
|                       | permutation_bonf | 0.2                 | 0.1                 | 0.4                 | 0.2                  | 0.0                  | 0.5                  | 0.1                  | 0.1                  | 0.4                  |
| Weib late discrete    | asymptotic       | 6.5                 | 6.7                 | 4.1                 | 2.1                  | 0.5                  | 2.8                  | 2.1                  | 1.4                  | 3.3                  |
|                       | asymptotic_bonf  | 6.2                 | 6.4                 | 3.8                 | 1.8                  | 0.5                  | 2.6                  | 1.8                  | 1.1                  | 2.9                  |
|                       | permutation_bonf | 0.0                 | 0.3                 | 0.3                 | 0.2                  | 0.4                  | 0.2                  | 0.2                  | 0.3                  | 0.2                  |
| Weib prop continuous  | asymptotic       | 5.2                 | 6.9                 | 3.1                 | 1.8                  | 0.7                  | 2.2                  | 2.3                  | 1.3                  | 2.3                  |
|                       | asymptotic_bonf  | 5.0                 | 6.4                 | 2.7                 | 1.4                  | 0.7                  | 1.8                  | 2.1                  | 1.0                  | 1.9                  |
|                       | permutation_bonf | 0.2                 | 0.0                 | 0.4                 | 0.2                  | 0.0                  | 0.2                  | 0.1                  | 0.1                  | 0.2                  |
| Weib prop discrete    | asymptotic       | 6.6                 | 7.5                 | 3.8                 | 1.8                  | 0.5                  | 2.6                  | 2.3                  | 0.7                  | 2.1                  |
|                       | asymptotic_bonf  | 6.3                 | 7.1                 | 3.3                 | 1.3                  | 0.5                  | 2.0                  | 1.9                  | 0.5                  | 1.8                  |
|                       | permutation_bonf | 0.1                 | 0.1                 | 0.3                 | 0.2                  | 0.1                  | 0.1                  | 0.2                  | 0.0                  | 0.3                  |
| Weib scale continuous | asymptotic       | 6.4                 | 10.0                | 3.9                 | 2.1                  | 1.8                  | 2.2                  | 2.6                  | 2.2                  | 2.5                  |
|                       | asymptotic_bonf  | 6.2                 | 9.3                 | 3.7                 | 1.8                  | 1.6                  | 2.2                  | 2.3                  | 1.9                  | 2.4                  |
|                       | permutation_bonf | 0.2                 | 0.1                 | 0.3                 | 0.2                  | 0.0                  | 0.1                  | 0.3                  | 0.2                  | 0.2                  |
| Weib scale discrete   | asymptotic       | 7.6                 | 10.1                | 4.1                 | 2.0                  | 1.0                  | 2.0                  | 2.1                  | 1.8                  | 2.2                  |
|                       | asymptotic_bonf  | 7.5                 | 9.8                 | 3.9                 | 1.6                  | 0.8                  | 1.5                  | 2.0                  | 1.2                  | 2.0                  |
|                       | permutation_bonf | 0.1                 | 0.1                 | 0.1                 | 0.3                  | 0.1                  | 0.0                  | 0.4                  | 0.0                  | 0.2                  |
| Weib shape continuous | asymptotic       | 7.4                 | 12.2                | 3.9                 | 2.4                  | 1.3                  | 2.0                  | 3.1                  | 2.5                  | 2.4                  |
|                       | asymptotic_bonf  | 7.3                 | 11.4                | 3.9                 | 2.1                  | 1.0                  | 2.0                  | 2.3                  | 1.7                  | 2.3                  |
|                       | permutation_bonf | 0.6                 | 0.1                 | 0.3                 | 0.2                  | 0.0                  | 0.0                  | 0.4                  | 0.3                  | 0.0                  |
| Weib shape discrete   | asymptotic       | 9.1                 | 13.0                | 4.8                 | 2.3                  | 0.8                  | 1.9                  | 2.6                  | 1.8                  | 2.5                  |
|                       | asymptotic_bonf  | 8.9                 | 12.5                | 4.6                 | 1.6                  | 0.6                  | 1.6                  | 2.1                  | 1.1                  | 2.4                  |
|                       | permutation_bonf | 0.3                 | 0.2                 | 0.5                 | 0.3                  | 0.1                  | 0.1                  | 0.2                  | 0.2                  | 0.0                  |

Table S85: Rejection rates in percent for the Tukey-type contrast matrix with  $\delta = 1.5$  and balanced large sample sizes under unequal, low censoring.

| Distribution          | Method           | $\mathcal{H}_{0,7}$ | $\mathcal{H}_{0,8}$ | $\mathcal{H}_{0,9}$ | $\mathcal{H}_{0,13}$ | $\mathcal{H}_{0,14}$ | $\mathcal{H}_{0,15}$ | $\mathcal{H}_{0,16}$ | $\mathcal{H}_{0,17}$ | $\mathcal{H}_{0,18}$ |
|-----------------------|------------------|---------------------|---------------------|---------------------|----------------------|----------------------|----------------------|----------------------|----------------------|----------------------|
| exp early continuous  | asymptotic       | 79.6                | 55.9                | 92.2                | 78.6                 | 57.6                 | 92.6                 | 76.7                 | 54.9                 | 93.5                 |
|                       | asymptotic_bonf  | 77.0                | 53.9                | 91.7                | 76.7                 | 55.3                 | 92.1                 | 75.1                 | 52.8                 | 93.0                 |
|                       | permutation_bonf | 74.9                | 52.0                | 90.9                | 76.0                 | 54.1                 | 91.6                 | 72.8                 | 51.9                 | 92.0                 |
| exp early discrete    | asymptotic       | 84.4                | 63.6                | 95.1                | 84.9                 | 64.9                 | 95.6                 | 82.9                 | 61.6                 | 96.1                 |
|                       | asymptotic_bonf  | 83.6                | 61.5                | 94.8                | 83.0                 | 63.5                 | 95.0                 | 81.3                 | 59.8                 | 95.8                 |
|                       | permutation_bonf | 80.9                | 58.8                | 94.0                | 82.8                 | 62.7                 | 94.4                 | 79.9                 | 58.0                 | 94.5                 |
| exp late continuous   | asymptotic       | 82.9                | 61.0                | 94.7                | 82.6                 | 62.3                 | 94.6                 | 80.7                 | 59.5                 | 95.6                 |
|                       | asymptotic_bonf  | 81.7                | 58.2                | 94.0                | 80.9                 | 59.7                 | 93.9                 | 78.6                 | 57.2                 | 95.0                 |
|                       | permutation_bonf | 79.6                | 56.7                | 93.3                | 79.6                 | 60.3                 | 93.5                 | 77.0                 | 54.7                 | 94.5                 |
| exp late discrete     | asymptotic       | 87.4                | 68.1                | 96.5                | 89.3                 | 70.7                 | 97.2                 | 87.3                 | 65.7                 | 98.0                 |
|                       | asymptotic_bonf  | 86.2                | 66.5                | 96.2                | 88.2                 | 68.4                 | 96.8                 | 85.8                 | 63.5                 | 97.9                 |
|                       | permutation_bonf | 85.9                | 64.7                | 95.8                | 87.0                 | 66.7                 | 96.4                 | 83.9                 | 61.2                 | 97.1                 |
| exp prop continuous   | asymptotic       | 79.0                | 60.0                | 93.5                | 82.4                 | 62.0                 | 95.0                 | 79.5                 | 60.6                 | 94.1                 |
|                       | asymptotic_bonf  | 77.8                | 57.8                | 93.1                | 80.2                 | 60.2                 | 94.3                 | 77.7                 | 58.8                 | 93.4                 |
|                       | permutation_bonf | 75.7                | 56.1                | 92.6                | 79.6                 | 58.5                 | 94.4                 | 76.6                 | 57.9                 | 92.6                 |
| exp prop discrete     | asymptotic       | 85.1                | 69.5                | 96.2                | 88.6                 | 69.9                 | 98.2                 | 84.4                 | 67.6                 | 96.8                 |
|                       | asymptotic_bonf  | 83.6                | 67.6                | 95.6                | 87.6                 | 67.6                 | 97.6                 | 83.3                 | 65.0                 | 96.3                 |
|                       | permutation_bonf | 82.6                | 65.3                | 95.7                | 85.9                 | 66.7                 | 96.5                 | 81.5                 | 64.7                 | 95.3                 |
| logn continuous       | asymptotic       | 100.0               | 97.9                | 100.0               | 99.8                 | 98.4                 | 100.0                | 99.9                 | 97.8                 | 100.0                |
|                       | asymptotic_bonf  | 100.0               | 97.5                | 100.0               | 99.6                 | 98.4                 | 100.0                | 99.9                 | 97.6                 | 100.0                |
|                       | permutation_bonf | 100.0               | 97.3                | 100.0               | 99.6                 | 97.9                 | 100.0                | 99.9                 | 96.9                 | 100.0                |
| logn discrete         | asymptotic       | 100.0               | 99.5                | 100.0               | 99.9                 | 99.5                 | 100.0                | 99.9                 | 99.3                 | 100.0                |
|                       | asymptotic_bonf  | 100.0               | 99.3                | 100.0               | 99.9                 | 99.5                 | 100.0                | 99.9                 | 99.2                 | 100.0                |
|                       | permutation_bonf | 100.0               | 99.0                | 100.0               | 99.9                 | 99.1                 | 100.0                | 99.9                 | 99.4                 | 100.0                |
| pwExp continuous      | asymptotic       | 76.6                | 54.3                | 92.3                | 78.0                 | 56.6                 | 92.1                 | 74.4                 | 53.3                 | 92.6                 |
|                       | asymptotic_bonf  | 74.1                | 51.6                | 91.5                | 76.0                 | 54.5                 | 91.0                 | 72.7                 | 50.9                 | 91.6                 |
|                       | permutation_bonf | 73.7                | 51.1                | 89.9                | 75.2                 | 53.2                 | 90.2                 | 72.0                 | 49.6                 | 91.5                 |
| pwExp discrete        | asymptotic       | 83.6                | 62.2                | 95.0                | 84.7                 | 64.2                 | 95.3                 | 82.1                 | 60.2                 | 95.3                 |
|                       | asymptotic_bonf  | 82.1                | 59.8                | 94.4                | 83.4                 | 62.5                 | 94.9                 | 80.1                 | 57.6                 | 94.9                 |
|                       | permutation_bonf | 80.9                | 57.7                | 94.3                | 83.2                 | 61.2                 | 94.4                 | 79.3                 | 56.6                 | 94.2                 |
| Weib late continuous  | asymptotic       | 99.9                | 98.6                | 100.0               | 99.8                 | 99.1                 | 100.0                | 99.9                 | 97.2                 | 100.0                |
|                       | asymptotic_bonf  | 99.8                | 98.4                | 100.0               | 99.8                 | 98.9                 | 100.0                | 99.9                 | 96.8                 | 100.0                |
|                       | permutation_bonf | 99.9                | 98.1                | 100.0               | 99.7                 | 98.8                 | 100.0                | 99.4                 | 96.5                 | 100.0                |
| Weib late discrete    | asymptotic       | 100.0               | 99.8                | 100.0               | 100.0                | 99.8                 | 100.0                | 100.0                | 98.7                 | 100.0                |
|                       | asymptotic_bonf  | 100.0               | 99.7                | 100.0               | 100.0                | 99.8                 | 100.0                | 100.0                | 98.6                 | 100.0                |
|                       | permutation_bonf | 100.0               | 99.6                | 100.0               | 100.0                | 99.6                 | 100.0                | 100.0                | 98.7                 | 100.0                |
| Weib prop continuous  | asymptotic       | 99.8                | 98.0                | 100.0               | 99.7                 | 98.3                 | 100.0                | 99.8                 | 96.2                 | 100.0                |
|                       | asymptotic_bonf  | 99.7                | 97.5                | 100.0               | 99.7                 | 97.9                 | 100.0                | 99.8                 | 96.0                 | 100.0                |
|                       | permutation_bonf | 99.8                | 97.5                | 100.0               | 99.7                 | 98.3                 | 100.0                | 99.4                 | 96.2                 | 100.0                |
| Weib prop discrete    | asymptotic       | 100.0               | 99.6                | 100.0               | 100.0                | 99.7                 | 100.0                | 99.9                 | 98.4                 | 100.0                |
|                       | asymptotic_bonf  | 100.0               | 99.5                | 100.0               | 100.0                | 99.7                 | 100.0                | 99.9                 | 98.3                 | 100.0                |
|                       | permutation_bonf | 100.0               | 99.5                | 100.0               | 100.0                | 99.3                 | 100.0                | 100.0                | 98.3                 | 100.0                |
| Weib scale continuous | asymptotic       | 99.5                | 96.0                | 100.0               | 99.3                 | 96.1                 | 100.0                | 99.2                 | 94.2                 | 100.0                |
|                       | asymptotic_bonf  | 99.3                | 94.8                | 100.0               | 99.3                 | 95.5                 | 100.0                | 98.9                 | 93.5                 | 100.0                |
|                       | permutation_bonf | 99.2                | 95.3                | 100.0               | 99.1                 | 94.8                 | 99.9                 | 98.7                 | 92.9                 | 100.0                |
| Weib scale discrete   | asymptotic       | 99.8                | 98.8                | 100.0               | 99.8                 | 99.0                 | 100.0                | 99.9                 | 97.5                 | 100.0                |
|                       | asymptotic_bonf  | 99.8                | 98.5                | 100.0               | 99.7                 | 98.9                 | 100.0                | 99.9                 | 97.0                 | 100.0                |
|                       | permutation_bonf | 99.8                | 98.6                | 100.0               | 99.8                 | 98.3                 | 100.0                | 99.9                 | 96.3                 | 100.0                |
| Weib shape continuous | asymptotic       | 98.0                | 89.8                | 99.6                | 97.6                 | 90.7                 | 99.5                 | 97.6                 | 87.8                 | 99.5                 |
|                       | asymptotic_bonf  | 97.7                | 89.2                | 99.6                | 97.2                 | 89.7                 | 99.5                 | 97.2                 | 87.0                 | 99.4                 |
|                       | permutation_bonf | 97.4                | 88.0                | 99.6                | 96.9                 | 89.5                 | 99.4                 | 96.4                 | 85.3                 | 99.3                 |
| Weib shape discrete   | asymptotic       | 99.2                | 95.1                | 99.9                | 99.3                 | 96.3                 | 99.8                 | 98.9                 | 94.1                 | 99.9                 |
|                       | asymptotic_bonf  | 99.1                | 94.1                | 99.8                | 99.2                 | 95.8                 | 99.8                 | 98.8                 | 93.4                 | 99.9                 |
|                       | permutation_bonf | 99.0                | 93.8                | 99.9                | 98.9                 | 95.3                 | 99.9                 | 98.9                 | 92.8                 | 99.9                 |

Table S86: Rejection rates in percent for the Tukey-type contrast matrix with  $\delta = 1.5$  and balanced medium sample sizes under unequal, low censoring.

| Distribution          | Method           | $\mathcal{H}_{0,7}$ | $\mathcal{H}_{0,8}$ | $\mathcal{H}_{0,9}$ | $\mathcal{H}_{0,13}$ | $\mathcal{H}_{0,14}$ | $\mathcal{H}_{0,15}$ | $\mathcal{H}_{0,16}$ | $\mathcal{H}_{0,17}$ | $\mathcal{H}_{0,18}$ |
|-----------------------|------------------|---------------------|---------------------|---------------------|----------------------|----------------------|----------------------|----------------------|----------------------|----------------------|
| exp early continuous  | asymptotic       | 11.1                | 7.0                 | 15.1                | 11.7                 | 6.7                  | 18.7                 | 11.5                 | 4.2                  | 17.7                 |
|                       | asymptotic_bonf  | 10.5                | 6.3                 | 14.1                | 11.1                 | 5.9                  | 17.3                 | 10.0                 | 3.9                  | 16.4                 |
|                       | permutation_bonf | 9.9                 | 6.2                 | 14.2                | 10.2                 | 5.8                  | 16.3                 | 9.4                  | 3.6                  | 15.4                 |
| exp early discrete    | asymptotic       | 13.2                | 8.4                 | 18.6                | 14.0                 | 8.0                  | 22.9                 | 11.9                 | 6.2                  | 21.2                 |
|                       | asymptotic_bonf  | 12.0                | 6.9                 | 17.1                | 13.0                 | 7.2                  | 21.2                 | 11.2                 | 5.1                  | 19.3                 |
|                       | permutation_bonf | 12.8                | 7.1                 | 17.4                | 11.7                 | 7.0                  | 19.7                 | 10.6                 | 5.1                  | 17.4                 |
| exp late continuous   | asymptotic       | 11.4                | 8.2                 | 17.7                | 13.2                 | 7.1                  | 22.8                 | 12.7                 | 6.0                  | 20.6                 |
|                       | asymptotic_bonf  | 10.5                | 7.5                 | 16.5                | 12.2                 | 6.0                  | 20.6                 | 11.5                 | 4.8                  | 19.4                 |
|                       | permutation_bonf | 10.3                | 7.5                 | 15.3                | 11.2                 | 6.7                  | 19.2                 | 11.2                 | 5.1                  | 17.4                 |
| exp late discrete     | asymptotic       | 14.1                | 9.7                 | 21.0                | 15.3                 | 8.5                  | 25.5                 | 14.6                 | 6.2                  | 24.8                 |
|                       | asymptotic_bonf  | 12.8                | 8.9                 | 19.5                | 13.9                 | 7.7                  | 24.0                 | 13.4                 | 5.4                  | 22.2                 |
|                       | permutation_bonf | 13.7                | 8.4                 | 18.5                | 13.4                 | 7.8                  | 22.7                 | 12.4                 | 6.2                  | 20.7                 |
| exp prop continuous   | asymptotic       | 13.2                | 8.3                 | 16.3                | 12.0                 | 6.1                  | 16.3                 | 11.4                 | 6.2                  | 17.1                 |
|                       | asymptotic_bonf  | 12.3                | 7.7                 | 15.1                | 11.3                 | 5.6                  | 15.2                 | 9.8                  | 5.7                  | 15.2                 |
|                       | permutation_bonf | 10.5                | 7.2                 | 14.8                | 10.6                 | 5.8                  | 14.3                 | 9.8                  | 5.6                  | 14.4                 |
| exp prop discrete     | asymptotic       | 14.7                | 9.4                 | 19.1                | 13.6                 | 7.5                  | 20.9                 | 13.6                 | 7.6                  | 19.7                 |
|                       | asymptotic_bonf  | 13.3                | 8.5                 | 17.7                | 13.1                 | 6.6                  | 18.9                 | 12.5                 | 6.7                  | 17.9                 |
|                       | permutation_bonf | 11.8                | 8.3                 | 16.0                | 11.8                 | 6.5                  | 17.1                 | 11.5                 | 6.4                  | 17.2                 |
| logn continuous       | asymptotic       | 37.8                | 25.7                | 59.4                | 40.1                 | 26.5                 | 60.4                 | 38.4                 | 21.9                 | 54.9                 |
|                       | asymptotic_bonf  | 36.1                | 24.6                | 56.9                | 38.5                 | 24.5                 | 58.0                 | 36.2                 | 21.0                 | 52.7                 |
|                       | permutation_bonf | 34.5                | 23.6                | 54.6                | 36.3                 | 24.7                 | 56.7                 | 34.7                 | 20.3                 | 51.1                 |
| logn discrete         | asymptotic       | 45.3                | 32.5                | 66.8                | 47.5                 | 32.2                 | 69.1                 | 47.7                 | 28.9                 | 64.3                 |
|                       | asymptotic_bonf  | 43.4                | 30.3                | 64.9                | 45.2                 | 30.6                 | 67.1                 | 45.0                 | 26.7                 | 62.5                 |
|                       | permutation_bonf | 43.5                | 30.2                | 63.0                | 45.3                 | 30.7                 | 64.9                 | 44.0                 | 25.3                 | 58.8                 |
| pwExp continuous      | asymptotic       | 10.1                | 7.4                 | 16.4                | 11.3                 | 6.0                  | 19.0                 | 11.1                 | 4.8                  | 16.8                 |
|                       | asymptotic_bonf  | 9.0                 | 6.2                 | 15.2                | 10.2                 | 5.1                  | 16.8                 | 9.7                  | 4.3                  | 15.5                 |
|                       | permutation_bonf | 8.4                 | 6.7                 | 14.8                | 9.3                  | 5.1                  | 16.0                 | 9.0                  | 4.4                  | 14.4                 |
| pwExp discrete        | asymptotic       | 12.1                | 8.3                 | 19.5                | 13.1                 | 6.6                  | 22.5                 | 12.3                 | 5.8                  | 20.9                 |
|                       | asymptotic_bonf  | 11.2                | 7.5                 | 17.9                | 12.0                 | 6.2                  | 21.3                 | 10.9                 | 4.9                  | 19.2                 |
|                       | permutation_bonf | 10.3                | 7.5                 | 17.6                | 11.4                 | 6.1                  | 20.3                 | 10.3                 | 5.4                  | 17.9                 |
| Weib late continuous  | asymptotic       | 38.4                | 26.6                | 58.8                | 39.8                 | 26.3                 | 63.1                 | 40.7                 | 24.5                 | 56.9                 |
|                       | asymptotic_bonf  | 36.3                | 25.6                | 57.8                | 37.7                 | 24.3                 | 61.1                 | 37.9                 | 23.4                 | 55.2                 |
|                       | permutation_bonf | 35.3                | 24.1                | 55.2                | 36.8                 | 24.1                 | 59.8                 | 36.4                 | 21.5                 | 53.3                 |
| Weib late discrete    | asymptotic       | 47.1                | 32.2                | 67.9                | 48.1                 | 31.8                 | 71.4                 | 48.9                 | 29.2                 | 64.8                 |
|                       | asymptotic_bonf  | 44.9                | 30.5                | 65.8                | 46.2                 | 29.6                 | 69.3                 | 45.9                 | 27.8                 | 63.1                 |
|                       | permutation_bonf | 43.7                | 29.1                | 62.9                | 44.9                 | 28.6                 | 66.9                 | 45.3                 | 27.0                 | 60.3                 |
| Weib prop continuous  | asymptotic       | 36.7                | 25.3                | 56.6                | 37.6                 | 24.0                 | 60.7                 | 38.3                 | 22.9                 | 53.6                 |
|                       | asymptotic_bonf  | 35.0                | 23.3                | 54.0                | 36.1                 | 22.2                 | 58.9                 | 35.8                 | 21.6                 | 51.5                 |
|                       | permutation_bonf | 33.0                | 22.1                | 53.0                | 35.1                 | 21.9                 | 55.8                 | 33.6                 | 21.2                 | 49.1                 |
| Weib prop discrete    | asymptotic       | 45.3                | 30.7                | 65.3                | 46.5                 | 30.0                 | 68.4                 | 47.9                 | 28.2                 | 63.1                 |
|                       | asymptotic_bonf  | 43.2                | 29.1                | 62.9                | 44.2                 | 28.3                 | 66.8                 | 45.9                 | 27.2                 | 61.2                 |
|                       | permutation_bonf | 41.9                | 28.1                | 60.1                | 42.3                 | 27.4                 | 65.6                 | 43.1                 | 27.7                 | 59.7                 |
| Weib scale continuous | asymptotic       | 29.4                | 19.6                | 46.2                | 30.8                 | 18.1                 | 49.3                 | 30.2                 | 18.5                 | 42.8                 |
|                       | asymptotic_bonf  | 27.4                | 18.0                | 43.9                | 29.0                 | 16.9                 | 47.1                 | 27.8                 | 16.8                 | 41.2                 |
|                       | permutation_bonf | 25.4                | 18.0                | 43.3                | 28.2                 | 16.3                 | 45.5                 | 25.7                 | 15.6                 | 39.0                 |
| Weib scale discrete   | asymptotic       | 37.4                | 24.4                | 55.5                | 37.7                 | 23.3                 | 57.8                 | 38.8                 | 22.3                 | 51.8                 |
|                       | asymptotic_bonf  | 35.1                | 22.8                | 53.8                | 36.3                 | 21.6                 | 55.5                 | 36.6                 | 20.6                 | 49.4                 |
|                       | permutation_bonf | 32.9                | 22.0                | 52.1                | 35.2                 | 21.5                 | 53.6                 | 34.2                 | 21.0                 | 47.6                 |
| Weib shape continuous | asymptotic       | 19.5                | 12.8                | 33.6                | 21.4                 | 12.9                 | 37.1                 | 21.5                 | 11.8                 | 30.6                 |
|                       | asymptotic_bonf  | 18.3                | 11.9                | 31.7                | 19.6                 | 11.3                 | 34.7                 | 19.9                 | 10.4                 | 29.1                 |
|                       | permutation_bonf | 18.0                | 11.5                | 30.3                | 19.0                 | 11.1                 | 32.3                 | 19.2                 | 10.2                 | 27.6                 |
| Weib shape discrete   | asymptotic       | 26.5                | 17.4                | 41.1                | 28.7                 | 17.2                 | 44.6                 | 28.4                 | 16.2                 | 40.4                 |
|                       | asymptotic_bonf  | 23.5                | 15.2                | 39.7                | 26.8                 | 15.2                 | 42.5                 | 25.9                 | 14.7                 | 38.0                 |
|                       | permutation_bonf | 22.5                | 16.0                | 39.4                | 26.1                 | 14.9                 | 40.8                 | 25.9                 | 14.0                 | 35.9                 |

Table S87: Rejection rates in percent for the Tukey-type contrast matrix with  $\delta = 1.5$  and balanced small sample sizes under unequal, low censoring.

| Distribution          | Method           | $\mathcal{H}_{0,7}$ | $\mathcal{H}_{0,8}$ | $\mathcal{H}_{0,9}$ | $\mathcal{H}_{0,13}$ | $\mathcal{H}_{0,14}$ | $\mathcal{H}_{0,15}$ | $\mathcal{H}_{0,16}$ | $\mathcal{H}_{0,17}$ | $\mathcal{H}_{0,18}$ |
|-----------------------|------------------|---------------------|---------------------|---------------------|----------------------|----------------------|----------------------|----------------------|----------------------|----------------------|
| exp early continuous  | asymptotic       | 2.3                 | 0.8                 | 2.1                 | 1.7                  | 1.5                  | 2.1                  | 2.4                  | 0.6                  | 2.8                  |
|                       | asymptotic_bonf  | 2.1                 | 0.8                 | 1.9                 | 1.5                  | 1.1                  | 1.8                  | 2.1                  | 0.6                  | 2.6                  |
|                       | permutation_bonf | 1.9                 | 0.6                 | 1.2                 | 1.1                  | 0.6                  | 1.1                  | 1.8                  | 0.5                  | 1.5                  |
| exp early discrete    | asymptotic       | 2.0                 | 1.4                 | 1.7                 | 2.2                  | 1.2                  | 2.4                  | 2.1                  | 1.1                  | 1.7                  |
|                       | asymptotic_bonf  | 1.8                 | 1.2                 | 1.6                 | 1.7                  | 1.0                  | 1.9                  | 1.6                  | 1.1                  | 1.3                  |
|                       | permutation_bonf | 1.6                 | 0.8                 | 1.2                 | 1.3                  | 0.8                  | 1.8                  | 1.1                  | 1.0                  | 1.3                  |
| exp late continuous   | asymptotic       | 2.3                 | 1.2                 | 2.2                 | 1.9                  | 1.8                  | 2.7                  | 2.7                  | 1.3                  | 2.7                  |
|                       | asymptotic_bonf  | 2.0                 | 1.0                 | 2.0                 | 1.9                  | 1.6                  | 2.2                  | 2.6                  | 1.2                  | 2.6                  |
|                       | permutation_bonf | 1.6                 | 0.8                 | 1.4                 | 1.2                  | 1.0                  | 1.6                  | 1.9                  | 0.9                  | 2.3                  |
| exp late discrete     | asymptotic       | 2.4                 | 1.4                 | 2.8                 | 2.1                  | 1.7                  | 2.9                  | 2.9                  | 1.6                  | 3.3                  |
|                       | asymptotic_bonf  | 2.2                 | 1.2                 | 2.6                 | 2.0                  | 1.7                  | 2.6                  | 2.7                  | 1.1                  | 3.1                  |
|                       | permutation_bonf | 1.5                 | 0.9                 | 2.0                 | 1.6                  | 1.2                  | 1.7                  | 2.2                  | 1.1                  | 2.4                  |
| exp prop continuous   | asymptotic       | 1.3                 | 0.9                 | 2.4                 | 1.7                  | 1.2                  | 1.9                  | 1.1                  | 1.1                  | 2.4                  |
|                       | asymptotic_bonf  | 1.0                 | 0.9                 | 2.2                 | 1.6                  | 0.8                  | 1.4                  | 0.9                  | 0.8                  | 1.9                  |
|                       | permutation_bonf | 0.7                 | 0.9                 | 1.5                 | 1.2                  | 0.9                  | 1.3                  | 0.8                  | 0.7                  | 1.6                  |
| exp prop discrete     | asymptotic       | 2.3                 | 1.2                 | 3.1                 | 1.6                  | 0.5                  | 3.5                  | 1.9                  | 1.2                  | 3.1                  |
|                       | asymptotic_bonf  | 2.2                 | 0.9                 | 2.9                 | 1.4                  | 0.5                  | 3.1                  | 1.8                  | 1.0                  | 2.7                  |
|                       | permutation_bonf | 1.7                 | 0.5                 | 2.4                 | 1.0                  | 0.3                  | 2.3                  | 1.4                  | 1.0                  | 2.2                  |
| logn continuous       | asymptotic       | 5.4                 | 3.4                 | 7.9                 | 4.7                  | 2.8                  | 5.7                  | 5.0                  | 3.2                  | 7.5                  |
|                       | asymptotic_bonf  | 4.7                 | 2.8                 | 7.2                 | 4.0                  | 1.9                  | 5.3                  | 4.6                  | 2.9                  | 7.1                  |
|                       | permutation_bonf | 4.1                 | 2.6                 | 5.5                 | 3.2                  | 1.8                  | 4.4                  | 4.2                  | 2.5                  | 5.8                  |
| logn discrete         | asymptotic       | 6.8                 | 4.1                 | 10.3                | 6.5                  | 3.4                  | 7.7                  | 5.7                  | 3.4                  | 9.2                  |
|                       | asymptotic_bonf  | 6.0                 | 3.4                 | 9.0                 | 5.3                  | 2.8                  | 6.8                  | 5.2                  | 3.0                  | 8.9                  |
|                       | permutation_bonf | 4.8                 | 3.5                 | 7.9                 | 4.5                  | 2.9                  | 6.5                  | 5.1                  | 2.8                  | 7.5                  |
| pwExp continuous      | asymptotic       | 1.4                 | 1.1                 | 1.6                 | 1.4                  | 1.2                  | 2.0                  | 2.2                  | 0.9                  | 2.6                  |
|                       | asymptotic_bonf  | 1.4                 | 1.0                 | 1.4                 | 1.0                  | 1.0                  | 1.9                  | 2.2                  | 0.8                  | 2.4                  |
|                       | permutation_bonf | 1.2                 | 0.5                 | 1.0                 | 1.0                  | 0.3                  | 1.2                  | 1.8                  | 0.7                  | 1.9                  |
| pwExp discrete        | asymptotic       | 1.7                 | 1.0                 | 2.4                 | 1.6                  | 1.5                  | 2.5                  | 2.4                  | 1.1                  | 3.1                  |
|                       | asymptotic_bonf  | 1.4                 | 1.0                 | 1.6                 | 1.5                  | 1.1                  | 1.9                  | 2.4                  | 1.0                  | 2.7                  |
|                       | permutation_bonf | 1.1                 | 0.7                 | 1.1                 | 0.9                  | 0.5                  | 1.6                  | 2.0                  | 1.0                  | 2.0                  |
| Weib late continuous  | asymptotic       | 4.9                 | 4.3                 | 8.1                 | 5.9                  | 3.6                  | 8.4                  | 4.3                  | 4.1                  | 6.8                  |
|                       | asymptotic_bonf  | 4.1                 | 4.1                 | 7.1                 | 5.3                  | 3.2                  | 7.4                  | 3.9                  | 3.9                  | 6.4                  |
|                       | permutation_bonf | 3.8                 | 3.6                 | 6.0                 | 3.8                  | 2.6                  | 5.5                  | 3.0                  | 3.3                  | 5.2                  |
| Weib late discrete    | asymptotic       | 5.9                 | 4.6                 | 9.7                 | 6.9                  | 4.1                  | 9.7                  | 5.7                  | 4.6                  | 8.6                  |
|                       | asymptotic_bonf  | 5.4                 | 4.2                 | 8.3                 | 6.4                  | 3.6                  | 8.9                  | 5.1                  | 4.3                  | 8.2                  |
|                       | permutation_bonf | 4.7                 | 4.5                 | 6.6                 | 5.2                  | 3.2                  | 7.3                  | 3.5                  | 4.2                  | 7.4                  |
| Weib prop continuous  | asymptotic       | 4.6                 | 4.0                 | 6.8                 | 5.4                  | 3.2                  | 7.0                  | 3.8                  | 3.9                  | 6.2                  |
|                       | asymptotic_bonf  | 3.6                 | 3.5                 | 6.3                 | 4.5                  | 2.7                  | 6.0                  | 3.3                  | 3.6                  | 5.1                  |
|                       | permutation_bonf | 3.0                 | 3.2                 | 5.2                 | 3.6                  | 2.4                  | 4.9                  | 2.7                  | 3.0                  | 4.8                  |
| Weib prop discrete    | asymptotic       | 5.4                 | 4.8                 | 8.4                 | 6.4                  | 3.6                  | 8.8                  | 4.7                  | 4.8                  | 7.4                  |
|                       | asymptotic_bonf  | 5.0                 | 4.0                 | 7.6                 | 6.0                  | 2.9                  | 8.1                  | 4.0                  | 4.1                  | 7.2                  |
|                       | permutation_bonf | 4.2                 | 3.6                 | 5.6                 | 4.5                  | 2.6                  | 6.8                  | 3.3                  | 3.9                  | 5.9                  |
| Weib scale continuous | asymptotic       | 2.9                 | 2.6                 | 4.7                 | 2.5                  | 1.6                  | 4.9                  | 1.9                  | 1.9                  | 3.8                  |
|                       | asymptotic_bonf  | 2.7                 | 2.5                 | 4.3                 | 2.1                  | 1.5                  | 4.5                  | 1.5                  | 1.7                  | 3.4                  |
|                       | permutation_bonf | 1.7                 | 2.3                 | 3.0                 | 1.9                  | 1.3                  | 3.9                  | 1.6                  | 1.6                  | 3.0                  |
| Weib scale discrete   | asymptotic       | 3.5                 | 3.2                 | 5.3                 | 3.5                  | 2.0                  | 5.7                  | 2.2                  | 2.5                  | 5.4                  |
|                       | asymptotic_bonf  | 2.6                 | 3.2                 | 4.5                 | 3.0                  | 1.9                  | 5.3                  | 1.8                  | 2.0                  | 4.7                  |
|                       | permutation_bonf | 2.0                 | 2.4                 | 3.8                 | 2.5                  | 1.6                  | 4.8                  | 1.8                  | 1.8                  | 4.3                  |
| Weib shape continuous | asymptotic       | 1.3                 | 1.9                 | 2.0                 | 1.3                  | 1.2                  | 3.0                  | 1.0                  | 1.0                  | 2.4                  |
|                       | asymptotic_bonf  | 1.0                 | 1.6                 | 1.9                 | 1.3                  | 0.9                  | 2.4                  | 0.9                  | 0.9                  | 2.1                  |
|                       | permutation_bonf | 0.9                 | 1.4                 | 2.0                 | 0.7                  | 0.9                  | 2.4                  | 0.9                  | 0.7                  | 2.3                  |
| Weib shape discrete   | asymptotic       | 1.5                 | 2.3                 | 3.0                 | 1.7                  | 1.3                  | 3.8                  | 1.3                  | 1.4                  | 3.2                  |
|                       | asymptotic_bonf  | 1.3                 | 2.2                 | 2.4                 | 1.5                  | 1.2                  | 3.0                  | 1.1                  | 1.1                  | 3.0                  |
|                       | permutation_bonf | 1.1                 | 2.0                 | 2.2                 | 1.4                  | 1.1                  | 2.7                  | 0.9                  | 0.8                  | 2.9                  |

Table S88: Rejection rates in percent for the Tukey-type contrast matrix with  $\delta = 1.5$  and unbalanced large sample sizes under unequal, low censoring.

| Distribution          | Method           | $\mathcal{H}_{0,7}$ | $\mathcal{H}_{0,8}$ | $\mathcal{H}_{0,9}$ | $\mathcal{H}_{0,13}$ | $\mathcal{H}_{0,14}$ | $\mathcal{H}_{0,15}$ | $\mathcal{H}_{0,16}$ | $\mathcal{H}_{0,17}$ | $\mathcal{H}_{0,18}$ |
|-----------------------|------------------|---------------------|---------------------|---------------------|----------------------|----------------------|----------------------|----------------------|----------------------|----------------------|
| exp early continuous  | asymptotic       | 31.0                | 16.3                | 53.5                | 26.6                 | 12.9                 | 42.8                 | 26.9                 | 12.7                 | 44.1                 |
|                       | asymptotic_bonf  | 28.1                | 14.4                | 51.2                | 23.6                 | 11.1                 | 39.9                 | 23.9                 | 11.2                 | 40.3                 |
|                       | permutation_bonf | 24.3                | 11.7                | 48.3                | 21.1                 | 10.8                 | 37.7                 | 22.4                 | 10.3                 | 38.2                 |
| exp early discrete    | asymptotic       | 36.6                | 20.6                | 60.6                | 31.1                 | 15.4                 | 49.1                 | 31.9                 | 16.4                 | 52.0                 |
|                       | asymptotic_bonf  | 33.3                | 17.6                | 57.6                | 27.6                 | 13.8                 | 45.3                 | 28.5                 | 14.0                 | 47.7                 |
|                       | permutation_bonf | 28.8                | 14.0                | 54.7                | 26.4                 | 13.1                 | 44.5                 | 26.3                 | 12.7                 | 44.2                 |
| exp late continuous   | asymptotic       | 37.8                | 19.9                | 63.5                | 31.1                 | 15.1                 | 51.5                 | 31.4                 | 15.7                 | 52.0                 |
|                       | asymptotic_bonf  | 33.8                | 17.8                | 60.1                | 27.7                 | 13.1                 | 48.1                 | 28.4                 | 13.6                 | 47.9                 |
|                       | permutation_bonf | 30.2                | 14.6                | 58.4                | 25.6                 | 11.8                 | 46.2                 | 26.8                 | 12.9                 | 45.3                 |
| exp late discrete     | asymptotic       | 44.5                | 24.4                | 70.0                | 37.5                 | 19.1                 | 59.4                 | 38.1                 | 19.0                 | 59.8                 |
|                       | asymptotic_bonf  | 41.1                | 22.0                | 67.4                | 33.4                 | 16.7                 | 55.4                 | 34.4                 | 17.0                 | 57.5                 |
|                       | permutation_bonf | 36.7                | 17.2                | 64.5                | 31.2                 | 15.8                 | 53.5                 | 32.2                 | 15.2                 | 53.9                 |
| exp prop continuous   | asymptotic       | 36.7                | 20.0                | 54.5                | 30.0                 | 17.0                 | 43.1                 | 28.6                 | 16.2                 | 45.8                 |
|                       | asymptotic_bonf  | 33.1                | 17.8                | 50.3                | 27.3                 | 14.6                 | 39.6                 | 26.1                 | 14.3                 | 43.2                 |
|                       | permutation_bonf | 30.5                | 16.2                | 47.1                | 26.1                 | 12.1                 | 37.3                 | 23.1                 | 12.6                 | 41.8                 |
| exp prop discrete     | asymptotic       | 42.9                | 24.4                | 62.8                | 35.0                 | 20.5                 | 49.7                 | 33.9                 | 19.7                 | 53.9                 |
|                       | asymptotic_bonf  | 40.0                | 21.9                | 59.4                | 31.6                 | 18.0                 | 46.8                 | 30.3                 | 16.9                 | 50.2                 |
|                       | permutation_bonf | 36.1                | 18.0                | 56.2                | 29.8                 | 15.8                 | 45.2                 | 27.4                 | 14.8                 | 49.4                 |
| logn continuous       | asymptotic       | 87.8                | 66.7                | 95.6                | 77.5                 | 57.1                 | 91.3                 | 77.3                 | 58.8                 | 90.9                 |
|                       | asymptotic_bonf  | 85.6                | 63.8                | 94.4                | 76.4                 | 54.3                 | 89.9                 | 74.3                 | 55.5                 | 89.2                 |
|                       | permutation_bonf | 81.0                | 54.7                | 93.0                | 72.9                 | 48.3                 | 87.3                 | 71.5                 | 49.7                 | 86.9                 |
| logn discrete         | asymptotic       | 92.9                | 76.3                | 98.3                | 86.4                 | 66.4                 | 95.4                 | 86.2                 | 68.6                 | 95.2                 |
|                       | asymptotic_bonf  | 92.0                | 73.5                | 98.0                | 84.1                 | 63.3                 | 94.6                 | 84.1                 | 66.3                 | 94.1                 |
|                       | permutation_bonf | 87.1                | 62.7                | 96.8                | 81.0                 | 57.7                 | 92.6                 | 80.8                 | 60.0                 | 92.5                 |
| pwExp continuous      | asymptotic       | 29.9                | 15.4                | 52.1                | 24.2                 | 13.0                 | 43.0                 | 24.9                 | 13.4                 | 41.4                 |
|                       | asymptotic_bonf  | 26.8                | 12.9                | 48.4                | 21.6                 | 11.1                 | 38.7                 | 23.2                 | 11.9                 | 38.4                 |
|                       | permutation_bonf | 24.8                | 9.8                 | 46.3                | 20.1                 | 9.8                  | 38.0                 | 21.4                 | 10.4                 | 36.0                 |
| pwExp discrete        | asymptotic       | 34.9                | 18.9                | 60.6                | 29.5                 | 15.9                 | 50.0                 | 29.4                 | 16.6                 | 50.3                 |
|                       | asymptotic_bonf  | 32.7                | 16.3                | 57.1                | 26.0                 | 13.6                 | 47.0                 | 26.6                 | 15.0                 | 46.5                 |
|                       | permutation_bonf | 28.7                | 12.5                | 53.3                | 25.4                 | 12.4                 | 43.8                 | 25.1                 | 13.1                 | 44.1                 |
| Weib late continuous  | asymptotic       | 89.1                | 66.8                | 97.6                | 82.9                 | 57.9                 | 94.4                 | 80.8                 | 56.9                 | 94.9                 |
|                       | asymptotic_bonf  | 88.1                | 64.3                | 97.2                | 81.4                 | 54.7                 | 93.4                 | 79.8                 | 54.0                 | 93.5                 |
|                       | permutation_bonf | 83.9                | 56.3                | 96.1                | 78.4                 | 51.4                 | 92.3                 | 76.7                 | 48.8                 | 92.5                 |
| Weib late discrete    | asymptotic       | 93.3                | 75.9                | 98.9                | 88.5                 | 67.6                 | 97.3                 | 87.8                 | 66.7                 | 97.9                 |
|                       | asymptotic_bonf  | 92.6                | 73.3                | 98.7                | 87.1                 | 64.1                 | 96.6                 | 86.8                 | 64.4                 | 97.4                 |
|                       | permutation_bonf | 89.3                | 65.1                | 97.8                | 85.0                 | 59.9                 | 95.7                 | 83.8                 | 59.1                 | 96.1                 |
| Weib prop continuous  | asymptotic       | 85.4                | 63.8                | 96.4                | 79.4                 | 54.5                 | 92.4                 | 78.6                 | 53.6                 | 93.0                 |
|                       | asymptotic_bonf  | 83.9                | 60.5                | 95.4                | 77.4                 | 51.6                 | 91.3                 | 76.4                 | 49.7                 | 92.0                 |
|                       | permutation_bonf | 79.9                | 51.7                | 94.2                | 74.8                 | 47.5                 | 89.3                 | 73.5                 | 45.5                 | 89.9                 |
| Weib prop discrete    | asymptotic       | 92.1                | 73.5                | 98.7                | 86.9                 | 64.4                 | 96.4                 | 86.2                 | 64.7                 | 96.9                 |
|                       | asymptotic_bonf  | 90.4                | 70.1                | 98.2                | 85.1                 | 60.6                 | 96.0                 | 84.3                 | 61.4                 | 95.9                 |
|                       | permutation_bonf | 86.6                | 61.0                | 97.6                | 82.8                 | 56.4                 | 95.0                 | 80.7                 | 55.1                 | 95.0                 |
| Weib scale continuous | asymptotic       | 72.7                | 48.3                | 88.5                | 66.2                 | 42.2                 | 83.3                 | 65.6                 | 41.6                 | 83.7                 |
|                       | asymptotic_bonf  | 69.7                | 44.7                | 86.7                | 62.4                 | 38.7                 | 80.7                 | 63.1                 | 38.8                 | 81.6                 |
|                       | permutation_bonf | 64.8                | 35.9                | 83.7                | 57.8                 | 33.5                 | 77.3                 | 58.2                 | 32.1                 | 79.7                 |
| Weib scale discrete   | asymptotic       | 81.6                | 58.5                | 93.4                | 74.8                 | 51.2                 | 90.2                 | 74.7                 | 49.5                 | 90.1                 |
|                       | asymptotic_bonf  | 78.9                | 54.4                | 92.6                | 73.0                 | 48.2                 | 88.2                 | 72.3                 | 46.2                 | 89.0                 |
|                       | permutation_bonf | 72.7                | 43.8                | 89.2                | 68.8                 | 41.4                 | 86.6                 | 67.2                 | 40.8                 | 87.3                 |
| Weib shape continuous | asymptotic       | 53.6                | 30.1                | 72.3                | 47.0                 | 27.8                 | 66.4                 | 46.9                 | 28.5                 | 67.6                 |
|                       | asymptotic_bonf  | 48.5                | 25.9                | 68.7                | 43.2                 | 24.5                 | 62.6                 | 43.1                 | 24.2                 | 63.3                 |
|                       | permutation_bonf | 40.3                | 19.2                | 62.5                | 38.9                 | 21.4                 | 59.4                 | 38.2                 | 20.3                 | 59.6                 |
| Weib shape discrete   | asymptotic       | 65.3                | 40.0                | 82.6                | 57.4                 | 35.8                 | 76.0                 | 58.1                 | 36.1                 | 77.8                 |
|                       | asymptotic_bonf  | 61.5                | 35.3                | 79.7                | 54.2                 | 32.7                 | 72.6                 | 54.3                 | 33.2                 | 74.4                 |
|                       | permutation_bonf | 51.7                | 24.8                | 74.2                | 49.2                 | 27.4                 | 70.0                 | 49.8                 | 26.5                 | 71.1                 |

Table S89: Rejection rates in percent for the Tukey-type contrast matrix with  $\delta = 1.5$  and unbalanced medium sample sizes under unequal, low censoring.

| Distribution          | Method           | $\mathcal{H}_{0,7}$ | $\mathcal{H}_{0,8}$ | $\mathcal{H}_{0,9}$ | $\mathcal{H}_{0,13}$ | $\mathcal{H}_{0,14}$ | $\mathcal{H}_{0,15}$ | $\mathcal{H}_{0,16}$ | $\mathcal{H}_{0,17}$ | $\mathcal{H}_{0,18}$ |
|-----------------------|------------------|---------------------|---------------------|---------------------|----------------------|----------------------|----------------------|----------------------|----------------------|----------------------|
| exp early continuous  | asymptotic       | 1.8                 | 1.3                 | 3.9                 | 1.5                  | 1.1                  | 3.5                  | 2.3                  | 1.3                  | 3.9                  |
|                       | asymptotic_bonf  | 1.3                 | 0.8                 | 3.3                 | 1.1                  | 1.0                  | 3.2                  | 2.0                  | 0.9                  | 3.0                  |
|                       | permutation_bonf | 0.6                 | 0.2                 | 1.6                 | 0.5                  | 0.4                  | 2.3                  | 1.6                  | 0.5                  | 2.2                  |
| exp early discrete    | asymptotic       | 2.7                 | 1.4                 | 4.6                 | 1.9                  | 1.3                  | 4.2                  | 3.0                  | 1.3                  | 4.7                  |
|                       | asymptotic_bonf  | 1.8                 | 1.1                 | 4.0                 | 1.2                  | 1.1                  | 3.6                  | 2.5                  | 0.9                  | 3.8                  |
|                       | permutation_bonf | 0.6                 | 0.3                 | 2.3                 | 0.9                  | 0.5                  | 2.9                  | 1.3                  | 0.6                  | 2.6                  |
| exp late continuous   | asymptotic       | 2.6                 | 1.7                 | 4.7                 | 1.9                  | 1.4                  | 3.8                  | 2.9                  | 1.6                  | 4.3                  |
|                       | asymptotic_bonf  | 2.1                 | 1.5                 | 4.5                 | 1.2                  | 1.2                  | 3.3                  | 2.4                  | 1.2                  | 3.6                  |
|                       | permutation_bonf | 0.8                 | 0.2                 | 1.6                 | 0.8                  | 0.6                  | 2.8                  | 1.7                  | 0.3                  | 2.4                  |
| exp late discrete     | asymptotic       | 3.3                 | 2.0                 | 5.9                 | 2.6                  | 1.6                  | 4.3                  | 3.5                  | 2.0                  | 5.3                  |
|                       | asymptotic_bonf  | 2.4                 | 1.6                 | 5.0                 | 1.7                  | 1.3                  | 4.0                  | 2.5                  | 1.2                  | 4.2                  |
|                       | permutation_bonf | 1.0                 | 0.5                 | 2.7                 | 1.2                  | 1.1                  | 2.8                  | 1.7                  | 0.3                  | 3.2                  |
| exp prop continuous   | asymptotic       | 2.8                 | 1.3                 | 3.4                 | 2.8                  | 1.2                  | 3.8                  | 2.2                  | 1.9                  | 3.2                  |
|                       | asymptotic_bonf  | 2.3                 | 1.0                 | 2.7                 | 2.4                  | 1.1                  | 2.7                  | 1.9                  | 1.4                  | 2.7                  |
|                       | permutation_bonf | 1.3                 | 0.5                 | 1.5                 | 1.9                  | 0.4                  | 1.7                  | 0.9                  | 0.3                  | 2.2                  |
| exp prop discrete     | asymptotic       | 3.5                 | 1.7                 | 3.9                 | 3.2                  | 1.2                  | 4.3                  | 3.0                  | 2.0                  | 3.7                  |
|                       | asymptotic_bonf  | 2.8                 | 1.2                 | 3.5                 | 2.6                  | 1.1                  | 3.5                  | 2.2                  | 1.5                  | 3.3                  |
|                       | permutation_bonf | 1.5                 | 0.3                 | 1.6                 | 1.7                  | 0.2                  | 2.2                  | 1.5                  | 0.5                  | 1.9                  |
| logn continuous       | asymptotic       | 8.1                 | 5.2                 | 16.2                | 7.2                  | 5.3                  | 13.6                 | 7.0                  | 4.4                  | 13.7                 |
|                       | asymptotic_bonf  | 6.7                 | 4.4                 | 14.1                | 5.9                  | 4.7                  | 12.2                 | 5.6                  | 3.7                  | 12.4                 |
|                       | permutation_bonf | 1.3                 | 0.3                 | 4.7                 | 2.3                  | 0.8                  | 7.8                  | 2.2                  | 1.3                  | 6.7                  |
| logn discrete         | asymptotic       | 10.6                | 6.3                 | 19.8                | 9.1                  | 6.4                  | 16.7                 | 8.4                  | 5.2                  | 16.4                 |
|                       | asymptotic_bonf  | 8.7                 | 5.0                 | 17.7                | 7.9                  | 5.5                  | 14.8                 | 7.1                  | 4.3                  | 14.9                 |
|                       | permutation_bonf | 1.2                 | 0.2                 | 5.5                 | 3.5                  | 1.1                  | 10.4                 | 3.1                  | 1.0                  | 8.4                  |
| pwExp continuous      | asymptotic       | 2.0                 | 1.5                 | 3.6                 | 1.1                  | 1.3                  | 3.5                  | 1.8                  | 1.1                  | 2.9                  |
|                       | asymptotic_bonf  | 1.3                 | 1.3                 | 3.1                 | 0.6                  | 1.0                  | 3.0                  | 1.8                  | 0.9                  | 2.6                  |
|                       | permutation_bonf | 0.7                 | 0.4                 | 1.6                 | 0.4                  | 0.7                  | 2.2                  | 1.1                  | 0.3                  | 2.0                  |
| pwExp discrete        | asymptotic       | 2.5                 | 1.7                 | 4.3                 | 1.8                  | 1.4                  | 3.6                  | 2.3                  | 1.5                  | 4.0                  |
|                       | asymptotic_bonf  | 1.7                 | 1.4                 | 3.7                 | 0.8                  | 1.0                  | 3.2                  | 1.9                  | 1.1                  | 3.1                  |
|                       | permutation_bonf | 0.5                 | 0.4                 | 1.7                 | 0.4                  | 0.6                  | 2.6                  | 1.3                  | 0.1                  | 2.6                  |
| Weib late continuous  | asymptotic       | 10.3                | 4.2                 | 20.4                | 9.1                  | 4.8                  | 16.5                 | 9.7                  | 4.5                  | 18.2                 |
|                       | asymptotic_bonf  | 8.8                 | 3.4                 | 18.0                | 7.8                  | 3.7                  | 14.1                 | 8.3                  | 3.6                  | 15.5                 |
|                       | permutation_bonf | 2.4                 | 0.0                 | 8.0                 | 4.3                  | 1.3                  | 8.7                  | 3.2                  | 0.6                  | 8.1                  |
| Weib late discrete    | asymptotic       | 12.8                | 5.3                 | 25.0                | 10.6                 | 5.4                  | 20.2                 | 12.1                 | 5.6                  | 21.4                 |
|                       | asymptotic_bonf  | 11.5                | 4.2                 | 22.8                | 9.5                  | 4.6                  | 18.0                 | 9.8                  | 4.3                  | 18.8                 |
|                       | permutation_bonf | 2.4                 | 0.3                 | 8.4                 | 5.8                  | 1.6                  | 11.2                 | 4.1                  | 0.7                  | 11.4                 |
| Weib prop continuous  | asymptotic       | 8.2                 | 2.9                 | 16.9                | 7.9                  | 3.6                  | 14.2                 | 8.9                  | 3.5                  | 14.4                 |
|                       | asymptotic_bonf  | 7.0                 | 2.4                 | 13.9                | 6.6                  | 2.6                  | 11.6                 | 7.0                  | 2.9                  | 11.8                 |
|                       | permutation_bonf | 1.6                 | 0.0                 | 5.9                 | 3.6                  | 1.1                  | 7.0                  | 2.8                  | 0.5                  | 6.4                  |
| Weib prop discrete    | asymptotic       | 11.6                | 4.4                 | 20.8                | 9.5                  | 4.6                  | 17.4                 | 10.6                 | 4.4                  | 17.8                 |
|                       | asymptotic_bonf  | 9.6                 | 2.9                 | 17.7                | 8.2                  | 3.5                  | 15.5                 | 8.6                  | 3.3                  | 15.2                 |
|                       | permutation_bonf | 1.9                 | 0.0                 | 6.3                 | 4.7                  | 0.9                  | 8.7                  | 3.6                  | 0.4                  | 8.3                  |
| Weib scale continuous | asymptotic       | 5.3                 | 1.4                 | 8.7                 | 4.6                  | 1.7                  | 7.9                  | 4.7                  | 1.7                  | 6.9                  |
|                       | asymptotic_bonf  | 4.1                 | 0.8                 | 6.5                 | 3.9                  | 1.2                  | 6.4                  | 3.4                  | 1.2                  | 5.7                  |
|                       | permutation_bonf | 0.5                 | 0.0                 | 2.6                 | 2.0                  | 0.5                  | 4.0                  | 1.4                  | 0.1                  | 3.0                  |
| Weib scale discrete   | asymptotic       | 5.9                 | 2.4                 | 10.9                | 6.2                  | 2.4                  | 10.4                 | 6.2                  | 2.8                  | 10.2                 |
|                       | asymptotic_bonf  | 5.1                 | 1.2                 | 9.1                 | 5.2                  | 1.5                  | 8.1                  | 4.6                  | 1.8                  | 7.4                  |
|                       | permutation_bonf | 0.7                 | 0.0                 | 2.7                 | 2.1                  | 0.5                  | 4.3                  | 1.4                  | 0.1                  | 3.6                  |
| Weib shape continuous | asymptotic       | 2.2                 | 0.9                 | 4.2                 | 3.1                  | 0.8                  | 3.6                  | 2.8                  | 0.9                  | 3.9                  |
|                       | asymptotic_bonf  | 1.8                 | 0.5                 | 3.4                 | 2.4                  | 0.6                  | 3.2                  | 1.5                  | 0.4                  | 2.7                  |
|                       | permutation_bonf | 0.2                 | 0.0                 | 1.1                 | 1.1                  | 0.2                  | 1.9                  | 0.4                  | 0.0                  | 1.4                  |
| Weib shape discrete   | asymptotic       | 3.4                 | 1.1                 | 5.3                 | 3.3                  | 1.0                  | 5.1                  | 3.9                  | 1.2                  | 5.2                  |
|                       | asymptotic_bonf  | 1.9                 | 0.9                 | 4.4                 | 2.8                  | 0.7                  | 4.2                  | 2.7                  | 0.9                  | 3.9                  |
|                       | permutation_bonf | 0.2                 | 0.0                 | 1.0                 | 1.2                  | 0.2                  | 2.6                  | 0.5                  | 0.0                  | 1.7                  |



Table S90: Rejection rates in percent for the Tukey-type contrast matrix with  $\delta = 1.5$  and unbalanced small sample sizes under unequal, low censoring.

| Distribution          | Method           | $\mathcal{H}_{0,7}$ | $\mathcal{H}_{0,8}$ | $\mathcal{H}_{0,9}$ | $\mathcal{H}_{0,13}$ | $\mathcal{H}_{0,14}$ | $\mathcal{H}_{0,15}$ | $\mathcal{H}_{0,16}$ | $\mathcal{H}_{0,17}$ | $\mathcal{H}_{0,18}$ |
|-----------------------|------------------|---------------------|---------------------|---------------------|----------------------|----------------------|----------------------|----------------------|----------------------|----------------------|
| exp early continuous  | asymptotic       | 0.8                 | 3.0                 | 2.0                 | 0.8                  | 1.5                  | 1.5                  | 0.8                  | 2.2                  | 1.3                  |
|                       | asymptotic_bonf  | 0.6                 | 2.9                 | 1.6                 | 0.7                  | 1.5                  | 1.3                  | 0.6                  | 1.9                  | 1.0                  |
|                       | permutation_bonf | 0.1                 | 0.0                 | 0.1                 | 0.1                  | 0.1                  | 0.1                  | 0.0                  | 0.3                  | 0.3                  |
| exp early discrete    | asymptotic       | 0.7                 | 3.0                 | 1.9                 | 0.8                  | 1.4                  | 1.5                  | 0.9                  | 1.9                  | 1.4                  |
|                       | asymptotic_bonf  | 0.7                 | 2.9                 | 1.8                 | 0.7                  | 1.4                  | 1.5                  | 0.6                  | 1.7                  | 1.0                  |
|                       | permutation_bonf | 0.1                 | 0.0                 | 0.1                 | 0.1                  | 0.2                  | 0.2                  | 0.0                  | 0.3                  | 0.2                  |
| exp late continuous   | asymptotic       | 1.0                 | 1.9                 | 1.9                 | 0.7                  | 1.0                  | 1.8                  | 0.7                  | 1.6                  | 1.4                  |
|                       | asymptotic_bonf  | 0.7                 | 1.7                 | 1.7                 | 0.6                  | 1.0                  | 1.5                  | 0.5                  | 1.5                  | 1.1                  |
|                       | permutation_bonf | 0.0                 | 0.0                 | 0.0                 | 0.0                  | 0.1                  | 0.0                  | 0.0                  | 0.2                  | 0.0                  |
| exp late discrete     | asymptotic       | 0.8                 | 1.8                 | 2.0                 | 1.0                  | 1.0                  | 2.3                  | 0.9                  | 1.6                  | 1.8                  |
|                       | asymptotic_bonf  | 0.7                 | 1.7                 | 1.7                 | 0.6                  | 0.9                  | 1.8                  | 0.7                  | 1.4                  | 1.3                  |
|                       | permutation_bonf | 0.0                 | 0.0                 | 0.0                 | 0.0                  | 0.3                  | 0.1                  | 0.0                  | 0.1                  | 0.1                  |
| exp prop continuous   | asymptotic       | 1.1                 | 2.0                 | 1.7                 | 1.3                  | 1.1                  | 1.5                  | 0.8                  | 0.9                  | 1.8                  |
|                       | asymptotic_bonf  | 1.1                 | 1.9                 | 1.7                 | 0.9                  | 0.9                  | 1.4                  | 0.6                  | 0.9                  | 1.6                  |
|                       | permutation_bonf | 0.0                 | 0.3                 | 0.2                 | 0.0                  | 0.1                  | 0.2                  | 0.2                  | 0.0                  | 0.2                  |
| exp prop discrete     | asymptotic       | 1.2                 | 2.1                 | 1.9                 | 1.2                  | 1.5                  | 1.8                  | 0.8                  | 1.1                  | 1.7                  |
|                       | asymptotic_bonf  | 1.2                 | 2.0                 | 1.9                 | 1.0                  | 1.1                  | 1.5                  | 0.6                  | 0.8                  | 1.6                  |
|                       | permutation_bonf | 0.0                 | 0.2                 | 0.1                 | 0.0                  | 0.1                  | 0.2                  | 0.0                  | 0.0                  | 0.2                  |
| logn continuous       | asymptotic       | 1.7                 | 3.1                 | 2.2                 | 1.3                  | 0.7                  | 1.8                  | 0.9                  | 1.0                  | 1.9                  |
|                       | asymptotic_bonf  | 1.5                 | 3.0                 | 1.8                 | 0.8                  | 0.6                  | 1.6                  | 0.8                  | 0.8                  | 1.5                  |
|                       | permutation_bonf | 0.2                 | 0.1                 | 0.1                 | 0.0                  | 0.2                  | 0.0                  | 0.0                  | 0.0                  | 0.0                  |
| logn discrete         | asymptotic       | 1.9                 | 3.2                 | 2.3                 | 1.3                  | 0.8                  | 1.6                  | 1.1                  | 0.9                  | 1.8                  |
|                       | asymptotic_bonf  | 1.5                 | 3.1                 | 2.0                 | 1.2                  | 0.7                  | 1.5                  | 0.8                  | 0.7                  | 1.6                  |
|                       | permutation_bonf | 0.2                 | 0.1                 | 0.1                 | 0.0                  | 0.1                  | 0.0                  | 0.1                  | 0.0                  | 0.0                  |
| pwExp continuous      | asymptotic       | 1.0                 | 2.3                 | 1.6                 | 0.7                  | 1.3                  | 1.5                  | 0.6                  | 1.8                  | 1.5                  |
|                       | asymptotic_bonf  | 0.9                 | 2.3                 | 1.3                 | 0.6                  | 1.2                  | 1.1                  | 0.5                  | 1.6                  | 1.1                  |
|                       | permutation_bonf | 0.0                 | 0.0                 | 0.1                 | 0.0                  | 0.1                  | 0.3                  | 0.0                  | 0.2                  | 0.2                  |
| pwExp discrete        | asymptotic       | 1.2                 | 2.4                 | 1.6                 | 0.7                  | 1.2                  | 1.8                  | 0.5                  | 1.4                  | 1.5                  |
|                       | asymptotic_bonf  | 1.1                 | 2.4                 | 1.5                 | 0.6                  | 1.0                  | 1.4                  | 0.5                  | 1.2                  | 1.2                  |
|                       | permutation_bonf | 0.0                 | 0.0                 | 0.1                 | 0.0                  | 0.2                  | 0.3                  | 0.0                  | 0.2                  | 0.2                  |
| Weib late continuous  | asymptotic       | 1.7                 | 1.6                 | 2.7                 | 1.3                  | 0.6                  | 2.5                  | 1.3                  | 0.8                  | 2.1                  |
|                       | asymptotic_bonf  | 1.3                 | 1.5                 | 2.0                 | 1.0                  | 0.4                  | 2.1                  | 1.2                  | 0.6                  | 2.0                  |
|                       | permutation_bonf | 0.0                 | 0.0                 | 0.0                 | 0.1                  | 0.0                  | 0.4                  | 0.1                  | 0.0                  | 0.0                  |
| Weib late discrete    | asymptotic       | 1.5                 | 2.0                 | 3.2                 | 1.3                  | 0.6                  | 2.9                  | 1.5                  | 0.9                  | 2.1                  |
|                       | asymptotic_bonf  | 1.4                 | 1.6                 | 2.4                 | 1.0                  | 0.5                  | 2.3                  | 1.2                  | 0.7                  | 1.9                  |
|                       | permutation_bonf | 0.0                 | 0.0                 | 0.0                 | 0.1                  | 0.0                  | 0.3                  | 0.1                  | 0.0                  | 0.1                  |
| Weib prop continuous  | asymptotic       | 1.4                 | 2.2                 | 2.0                 | 1.2                  | 0.6                  | 2.4                  | 1.1                  | 0.7                  | 2.0                  |
|                       | asymptotic_bonf  | 1.2                 | 2.1                 | 1.7                 | 1.0                  | 0.6                  | 2.0                  | 1.0                  | 0.6                  | 1.7                  |
|                       | permutation_bonf | 0.0                 | 0.0                 | 0.0                 | 0.1                  | 0.0                  | 0.1                  | 0.1                  | 0.0                  | 0.0                  |
| Weib prop discrete    | asymptotic       | 1.2                 | 2.3                 | 2.4                 | 0.8                  | 0.6                  | 2.6                  | 1.2                  | 0.9                  | 1.9                  |
|                       | asymptotic_bonf  | 1.1                 | 2.3                 | 2.1                 | 0.6                  | 0.5                  | 2.1                  | 0.9                  | 0.7                  | 1.7                  |
|                       | permutation_bonf | 0.0                 | 0.0                 | 0.0                 | 0.1                  | 0.0                  | 0.1                  | 0.1                  | 0.0                  | 0.0                  |
| Weib scale continuous | asymptotic       | 2.7                 | 3.5                 | 2.5                 | 1.6                  | 0.9                  | 1.1                  | 1.2                  | 1.2                  | 1.6                  |
|                       | asymptotic_bonf  | 2.6                 | 3.4                 | 2.1                 | 1.3                  | 0.9                  | 1.0                  | 0.8                  | 0.7                  | 1.1                  |
|                       | permutation_bonf | 0.0                 | 0.0                 | 0.1                 | 0.1                  | 0.3                  | 0.0                  | 0.0                  | 0.0                  | 0.0                  |
| Weib scale discrete   | asymptotic       | 2.9                 | 3.8                 | 2.5                 | 1.5                  | 0.8                  | 1.6                  | 0.9                  | 1.2                  | 1.7                  |
|                       | asymptotic_bonf  | 2.7                 | 3.7                 | 2.3                 | 0.9                  | 0.8                  | 1.0                  | 0.6                  | 0.7                  | 1.4                  |
|                       | permutation_bonf | 0.0                 | 0.0                 | 0.0                 | 0.1                  | 0.2                  | 0.0                  | 0.0                  | 0.0                  | 0.0                  |
| Weib shape continuous | asymptotic       | 6.0                 | 8.7                 | 3.2                 | 4.7                  | 3.0                  | 2.7                  | 4.0                  | 3.2                  | 2.7                  |
|                       | asymptotic_bonf  | 5.9                 | 8.5                 | 2.7                 | 4.0                  | 2.6                  | 2.3                  | 3.4                  | 2.7                  | 2.0                  |
|                       | permutation_bonf | 0.6                 | 0.2                 | 0.4                 | 0.8                  | 0.8                  | 0.2                  | 0.0                  | 0.1                  | 0.3                  |
| Weib shape discrete   | asymptotic       | 6.1                 | 9.0                 | 3.2                 | 4.0                  | 2.5                  | 2.4                  | 3.2                  | 2.6                  | 2.4                  |
|                       | asymptotic_bonf  | 6.0                 | 8.7                 | 2.9                 | 3.3                  | 2.1                  | 2.1                  | 2.8                  | 2.0                  | 2.0                  |
|                       | permutation_bonf | 0.3                 | 0.2                 | 0.4                 | 1.0                  | 0.5                  | 0.2                  | 0.0                  | 0.2                  | 0.3                  |

## References

- [1] P. J. Bickel and P. W. Millar. Uniform convergence of probability measures on classes of functions. *Statistica Sinica*, 2(1):1–15, 1992.
- [2] M. Ditzhaus, M. Yu, and J. Xu. Studentized permutation method for comparing two restricted mean survival times with small sample from randomized trials. *Statistics in Medicine*, 42(13):2226–2240, 2023.
- [3] D. Dobler. A discontinuity adjustment for subdistribution function confidence bands applied to right-censored competing risks data. *Electronic Journal of Statistics*, 11(2):3673 – 3702, 2017.
- [4] D. Dobler and M. Munko. A discontinuity adjustment for subdistribution function confidence bands applied to right-censored competing risks data with erratum, 2024.
- [5] M. Munko, M. Ditzhaus, D. Dobler, and J. Genuneit. RMST-based multiple contrast tests in general factorial designs. *Statistics in Medicine*, 43(10):1849–1866, 2024.
- [6] M. Munko, M. Ditzhaus, M. Pauly, and Ł. Smaga. Multiple comparison procedures for simultaneous inference in functional MANOVA. *arXiv preprint arXiv:2406.01242*, 2024.
- [7] M. Munko and D. Dobler. Conditional delta-method for resampling empirical processes in multiple sample problems. *arXiv preprint arXiv:2408.10856*, 2024.
- [8] C. Rao and S. K. Mitra. *Generalized Inverse of Matrices and Its Applications*. New York-London-Sydney: John Wiley & Sons, 1971.
- [9] A. v. d. Vaart and J. Wellner. *Weak Convergence and Empirical Processes: With Applications to Statistics*. Springer, Cham, Switzerland, 2023.
- [10] A. van der Vaart and J. Wellner. *Weak convergence and empirical processes: With applications to statistics*. Springer Series in Statistics. Springer, New York, 1996.
